# Supplementary material for: The complement of a $\sigma$-compact subset of a space with a $\pi$-tree also has a $\pi$-tree
Source: arXiv:1512.02458 ancillary file (2016-11-20)
Supplement: Supplementary file 1 [file The_foliage_hybrid_operation__slides_from_talk_.pdf]

Mikhail Patrakeev

# The foliage hybrid operation

slides from the talk

Alexandroff Readings, May 22–26, 2016

Moscow, Russia

# HYBRID OPERATION

$G$  is a graft for  $T$  iff

$$(1) \quad G \cap T = \{0_G\} \cup \max G$$

$$(2) \quad <_G \upharpoonright (G \cap T) = <_T \upharpoonright (G \cap T)$$

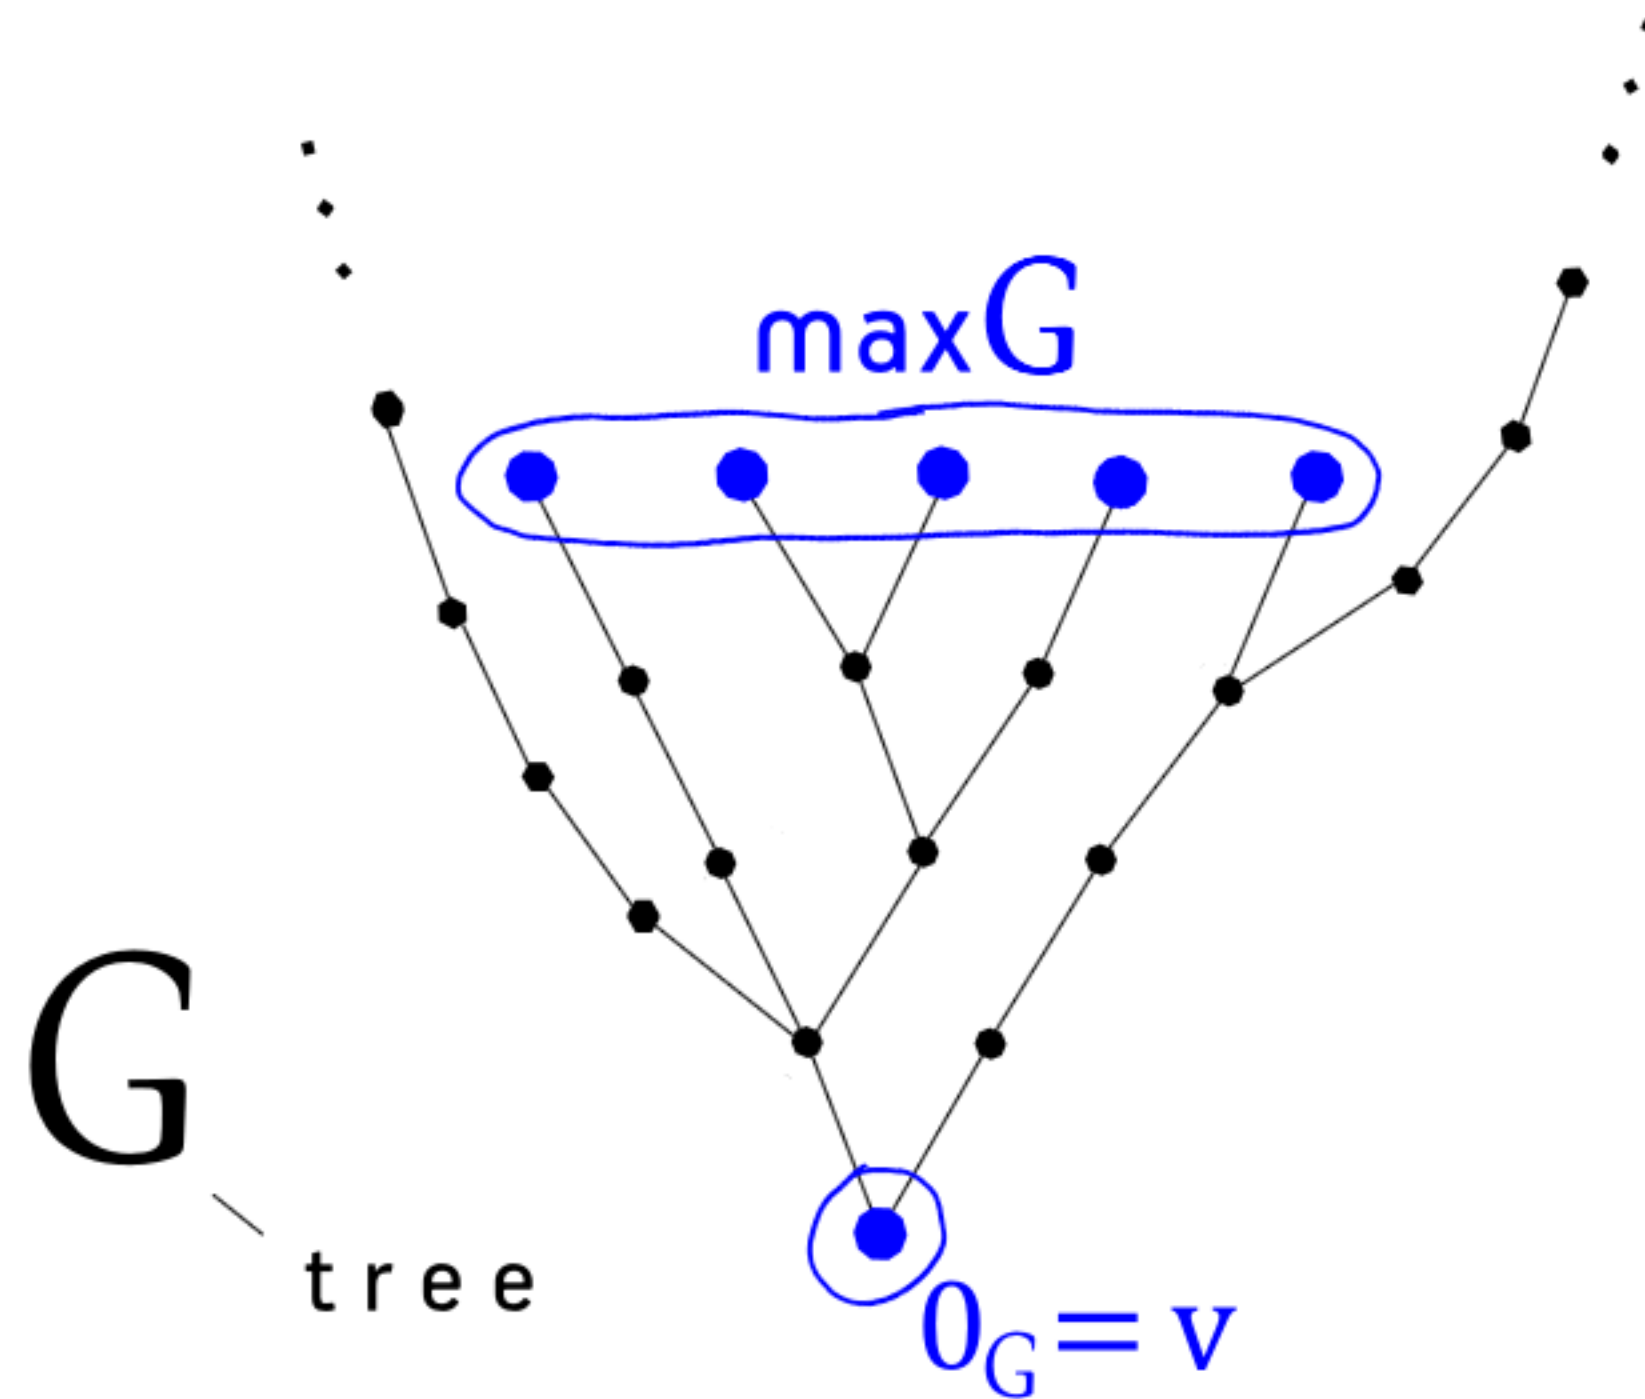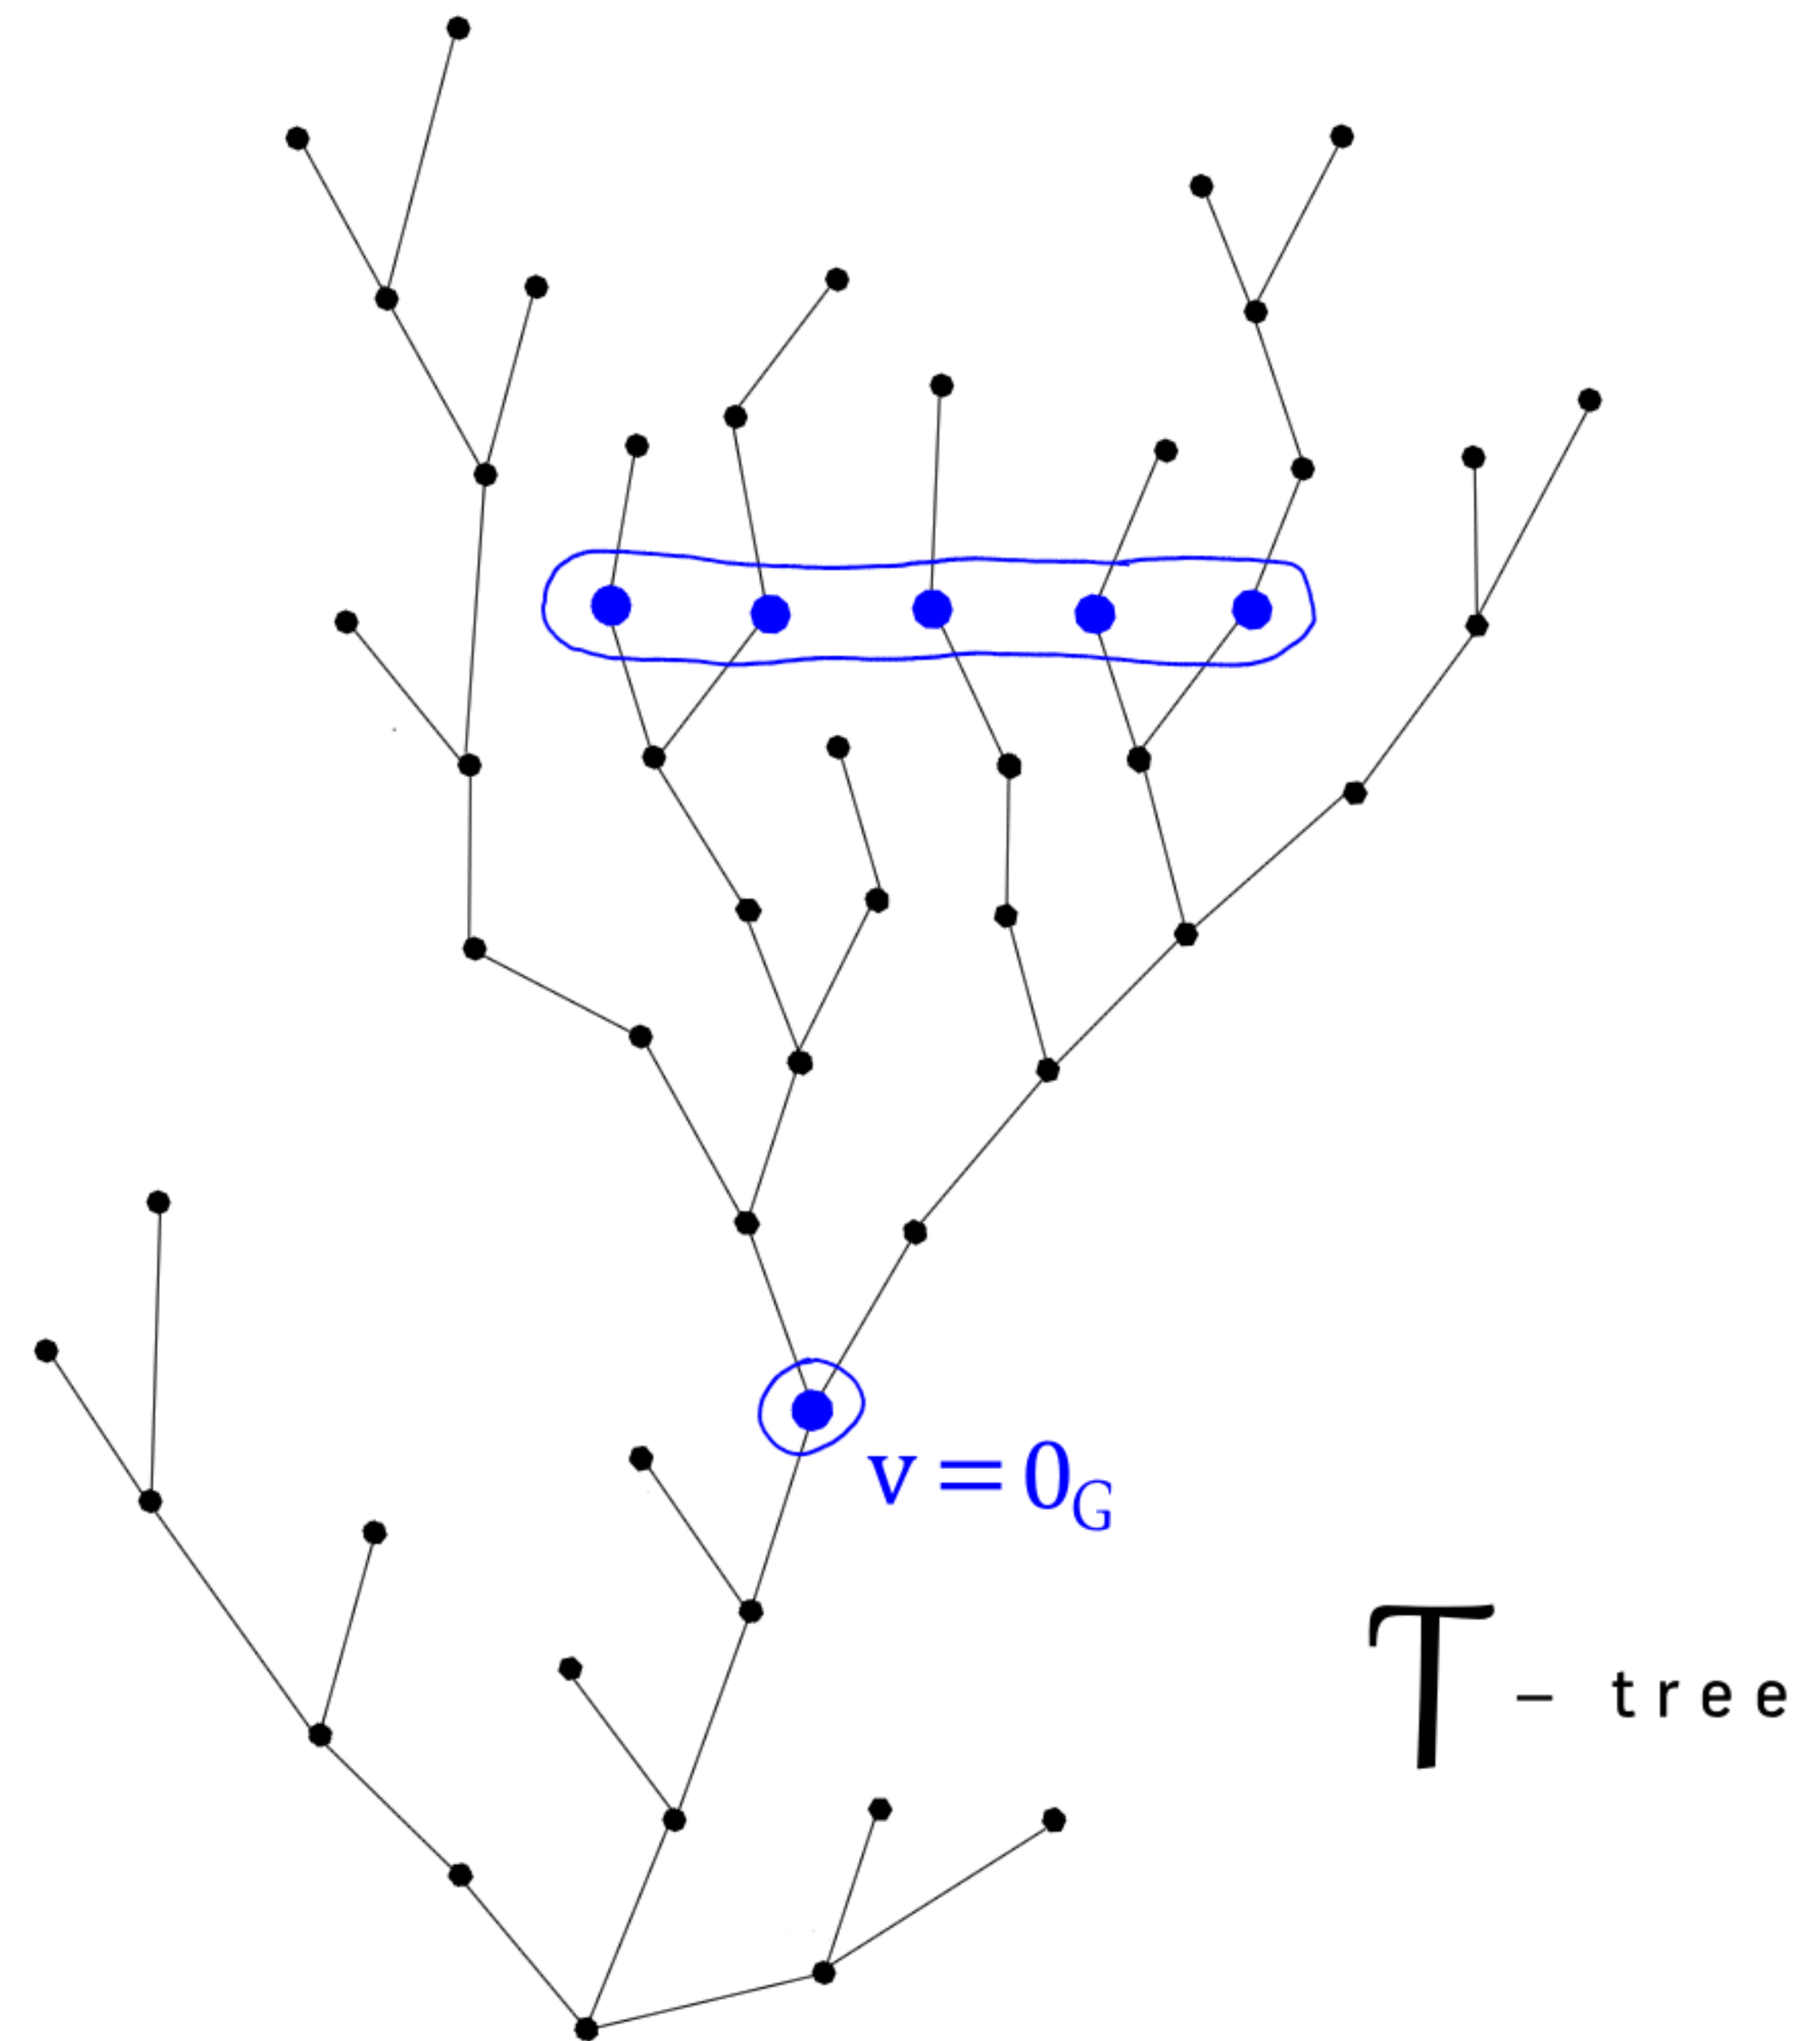

# HYBRID OPERATION

$G$  is a graft for  $T$  iff

$$(1) \quad G \cap T = \{0_G\} \cup \max G$$

$$(2) \quad <_G \upharpoonright (G \cap T) = <_T \upharpoonright (G \cap T)$$

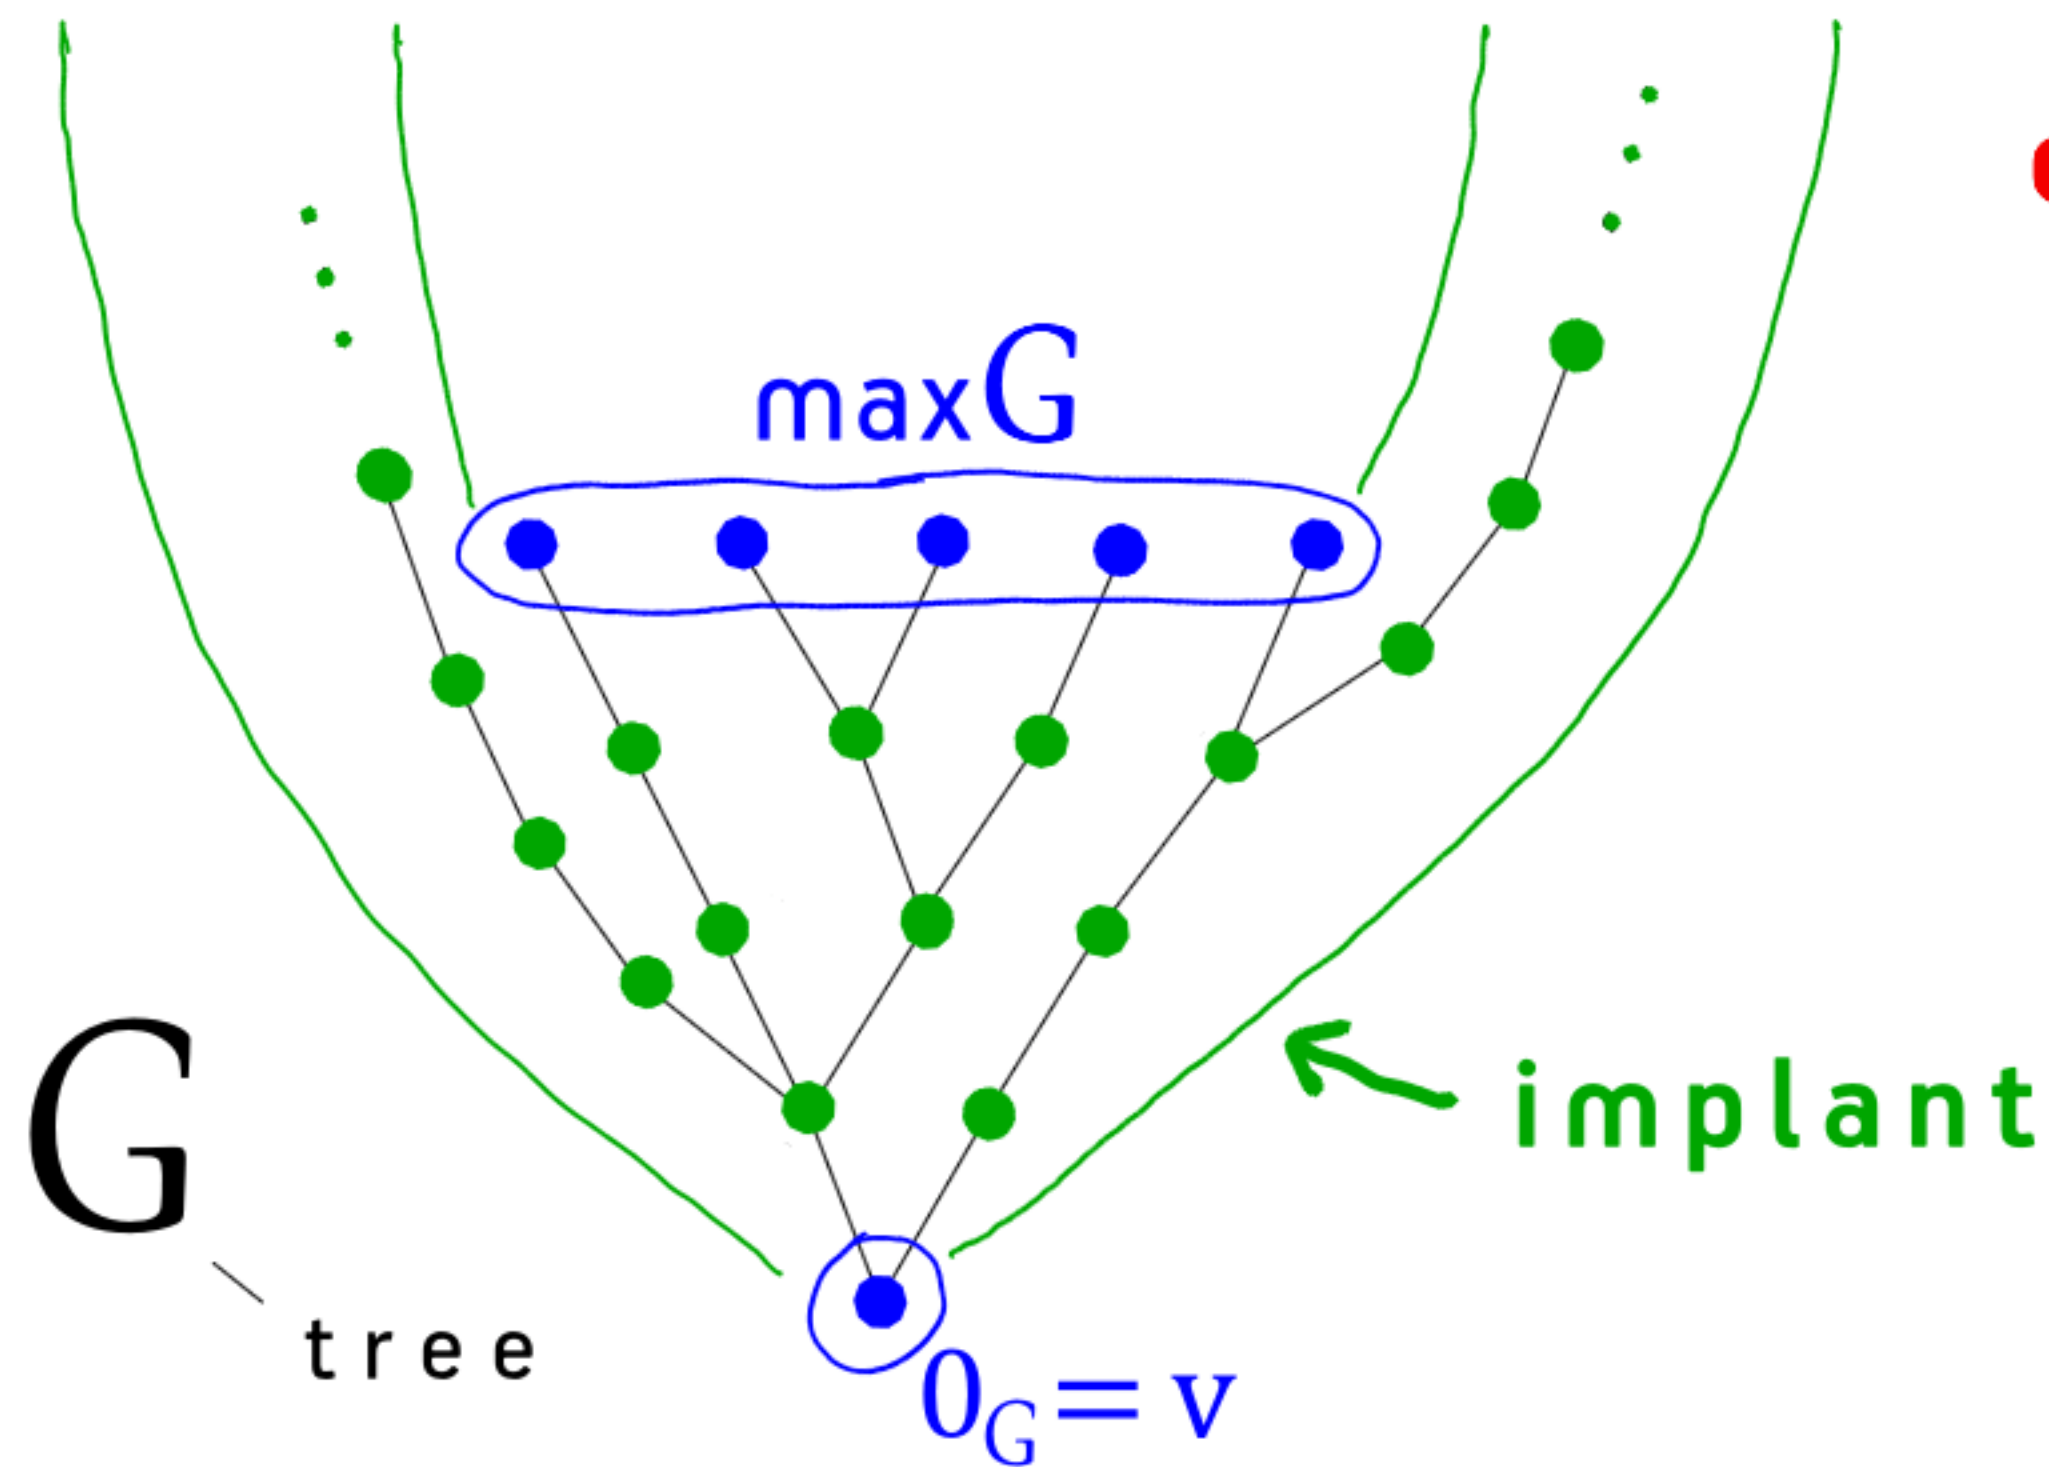

**explant** →

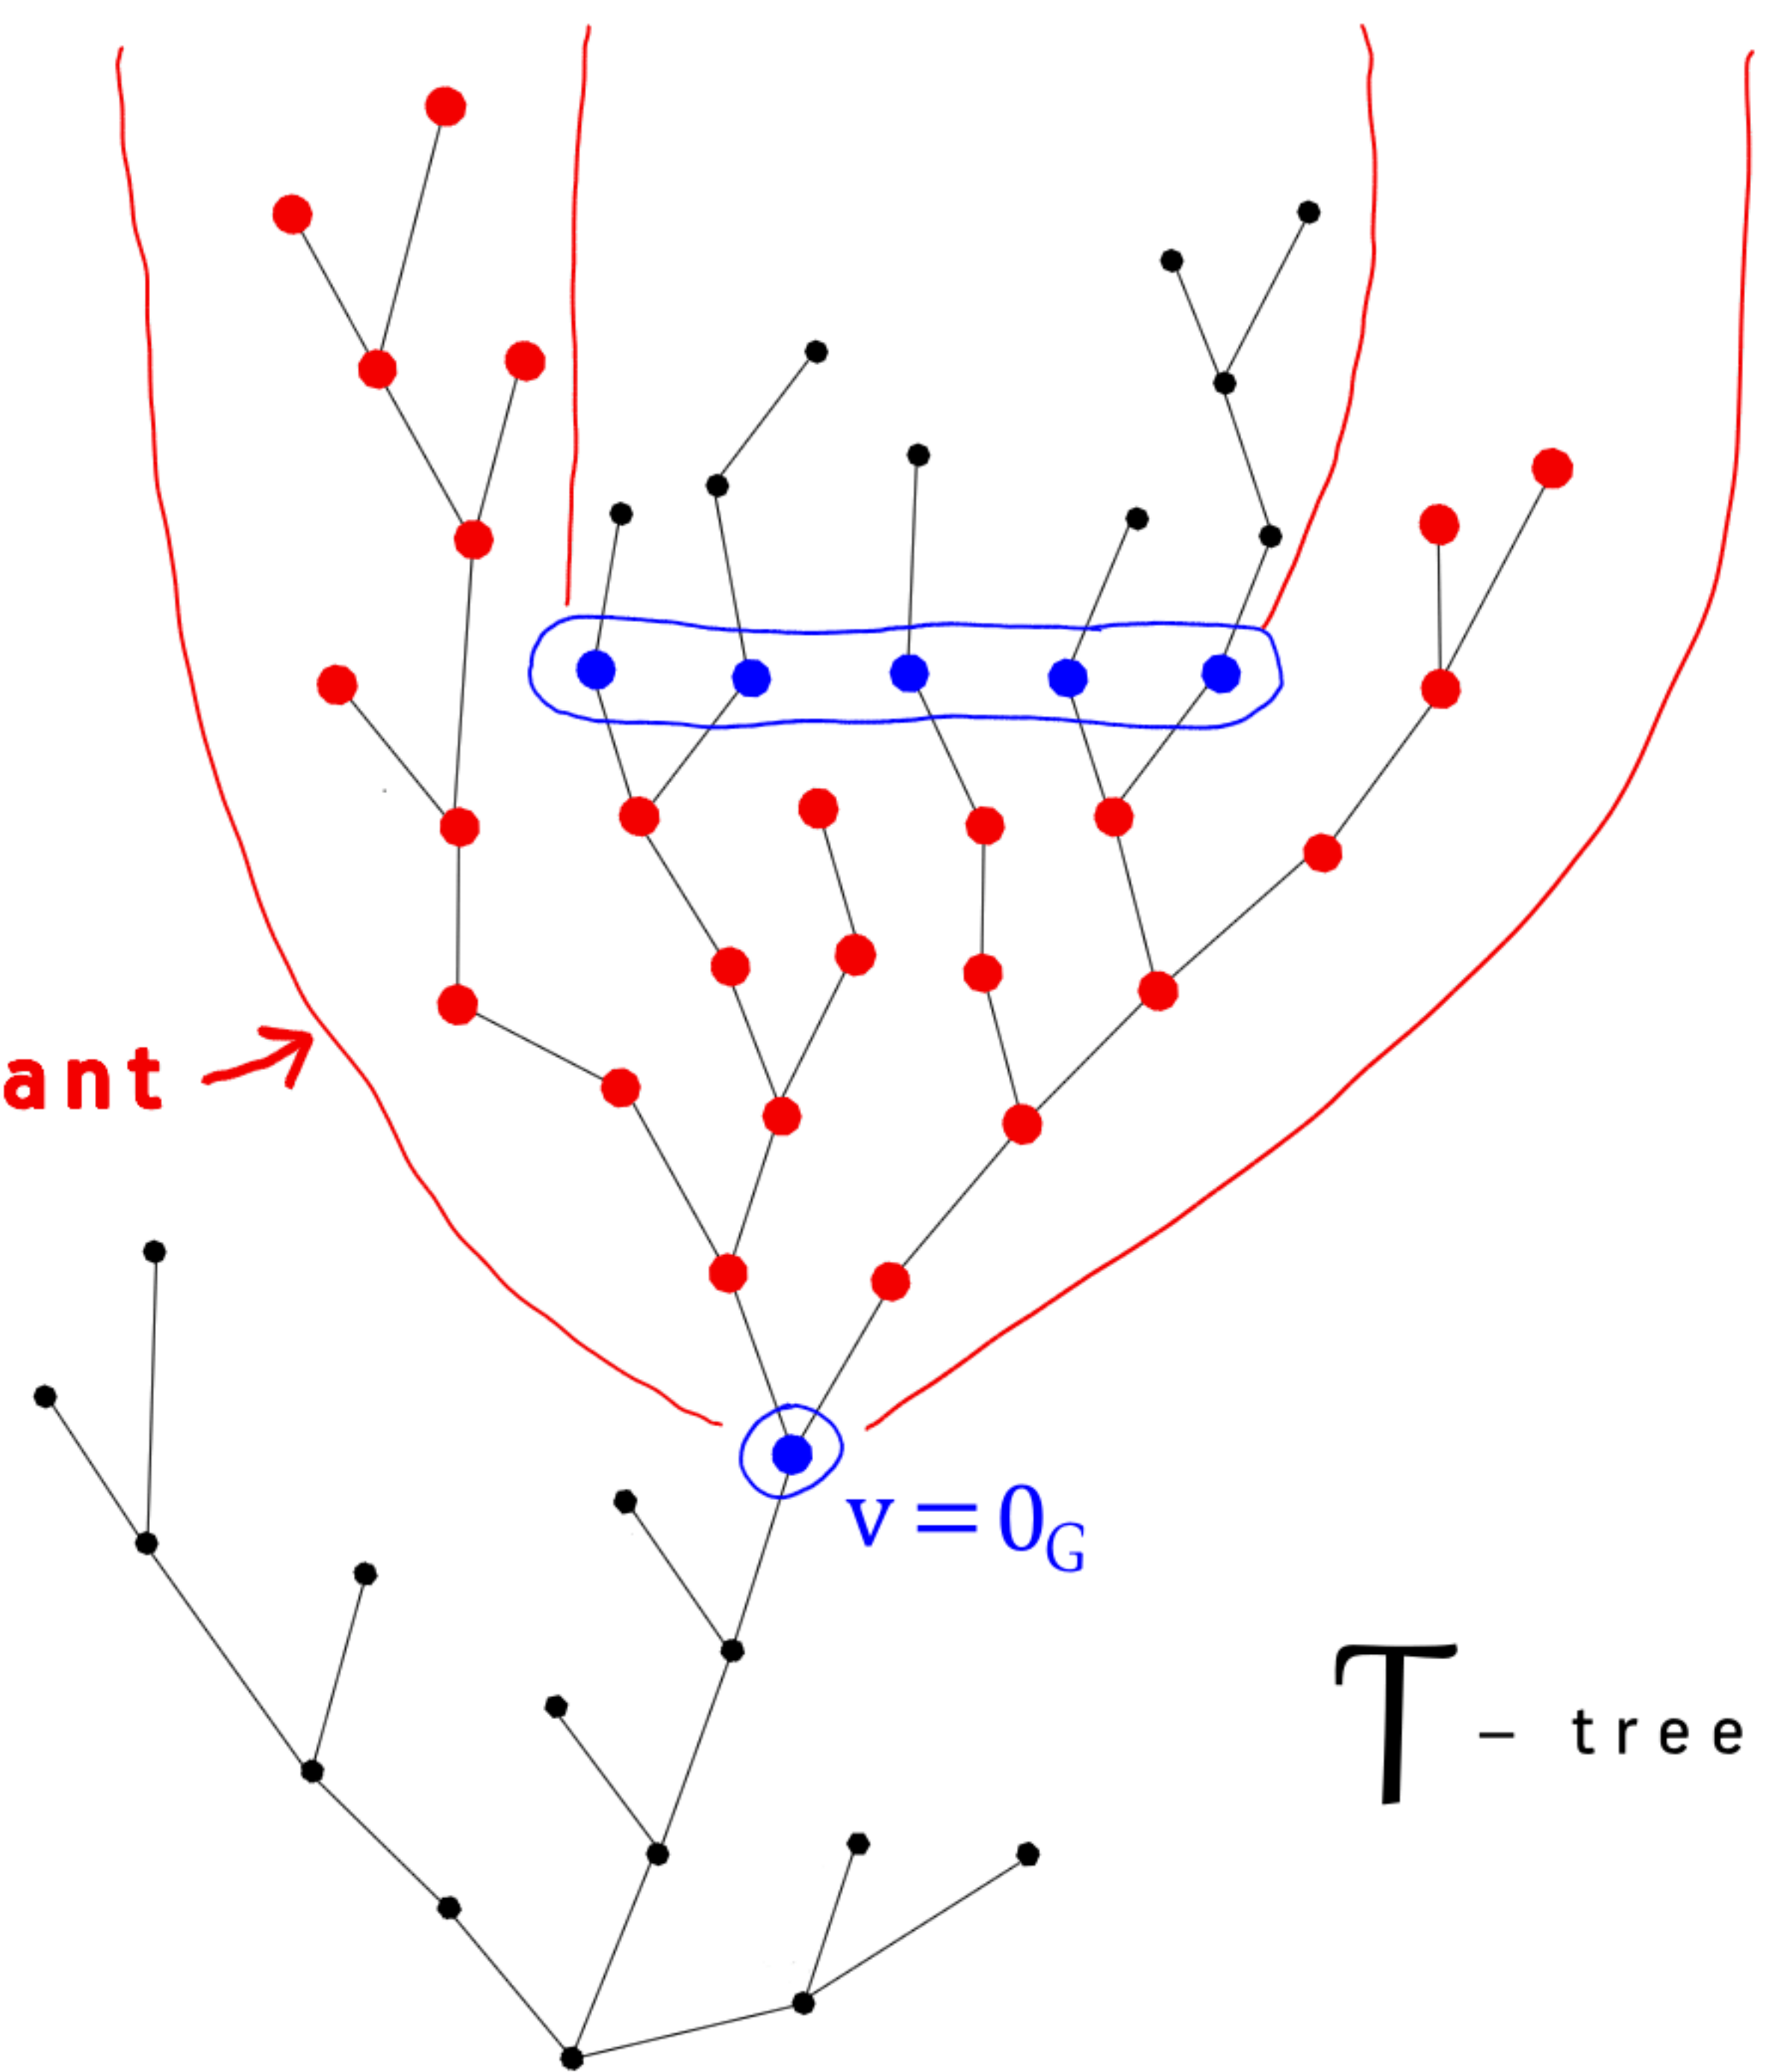

# HYBRID OPERATION

$G$  is a graft for  $T$  iff

$$(1) \quad G \cap T = \{0_G\} \cup \text{max}G$$

$$(2) \quad <_G \upharpoonright (G \cap T) = <_T \upharpoonright (G \cap T)$$

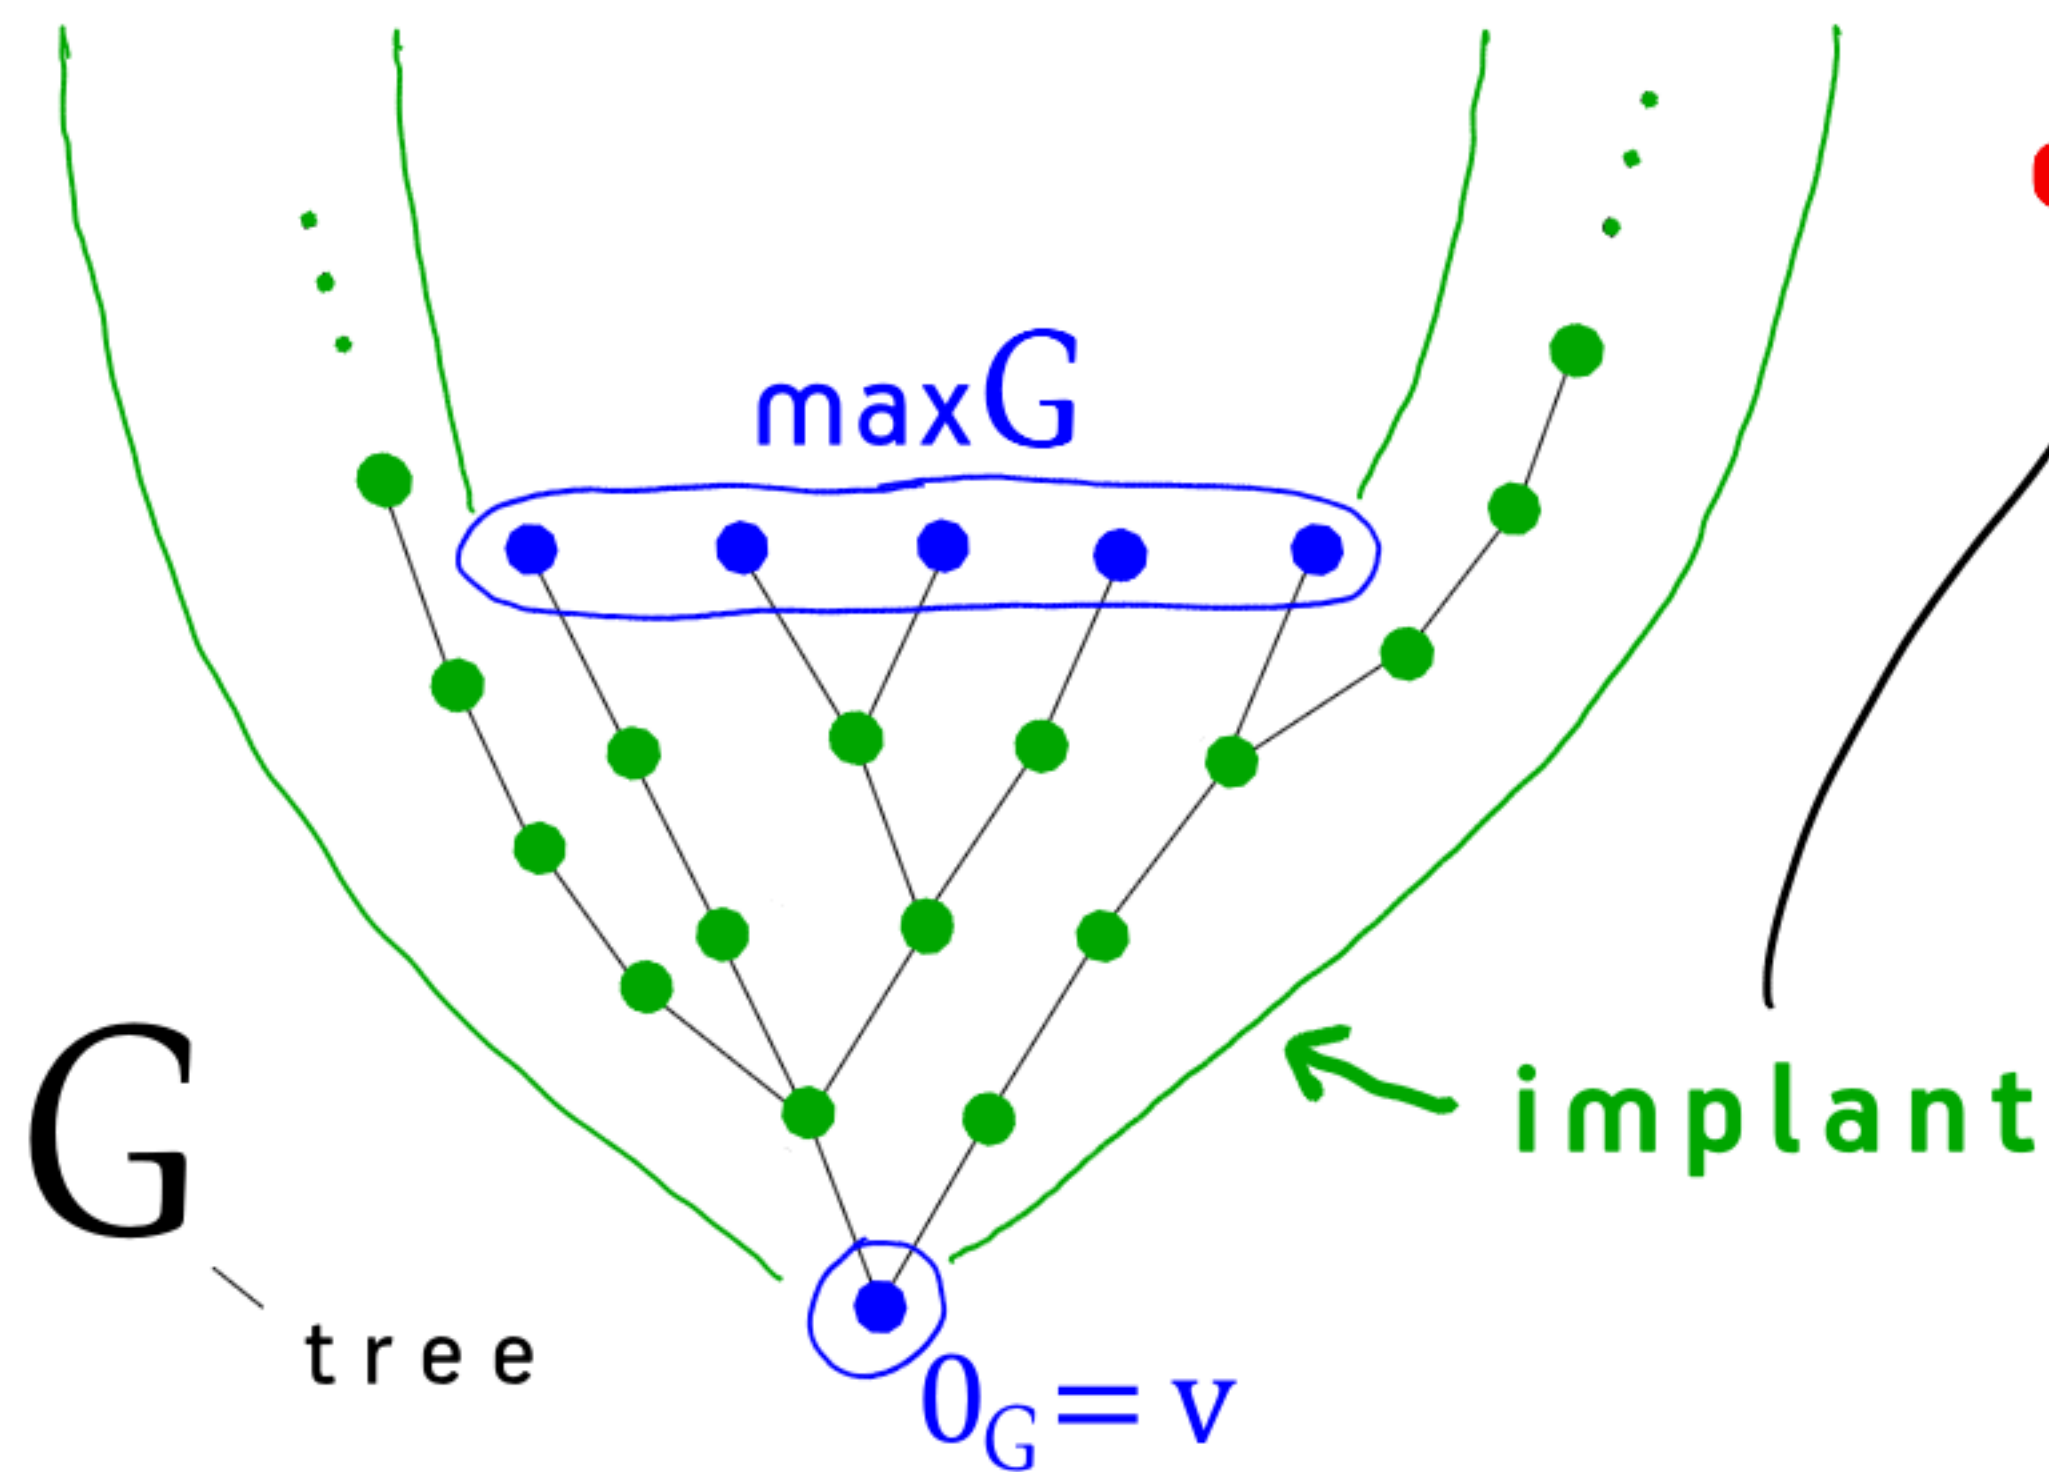

~~explant~~ →

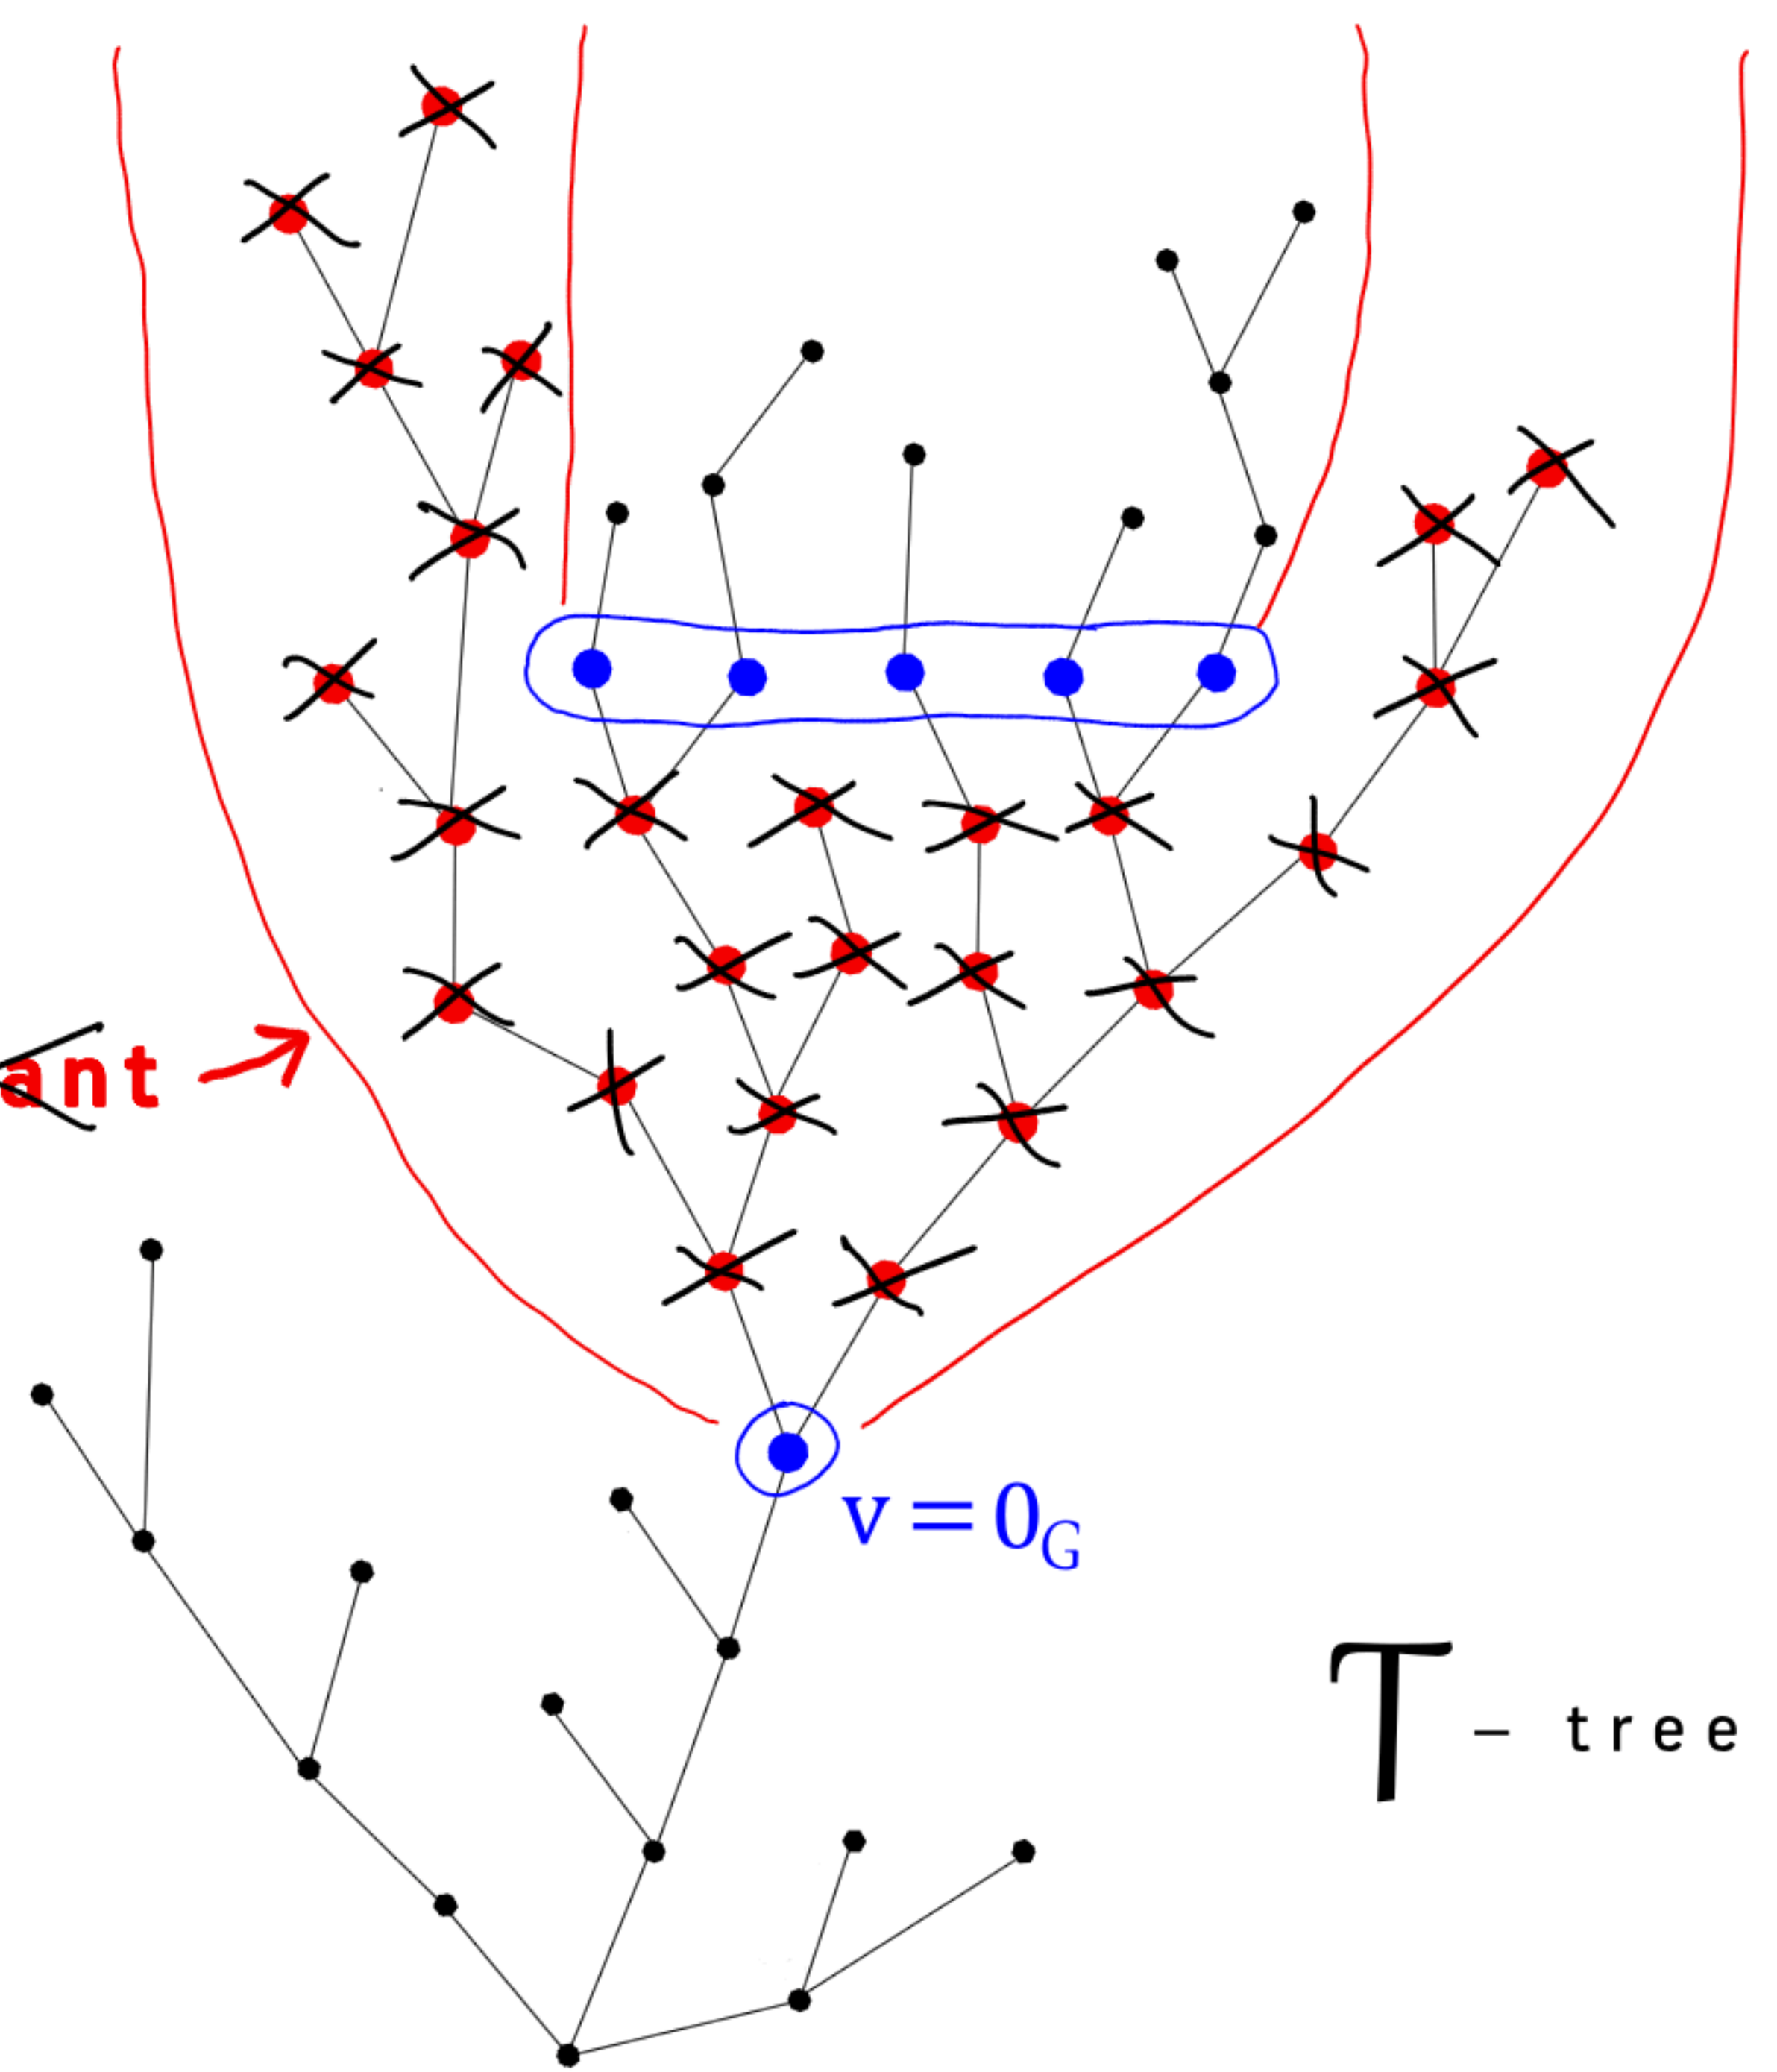



# HYBRID OPERATION

$G$  is a graft for  $T$  iff

$$(1) \quad G \cap T = \{0_G\} \cup \max G$$

$$(2) \quad <_G \upharpoonright (G \cap T) = <_T \upharpoonright (G \cap T)$$

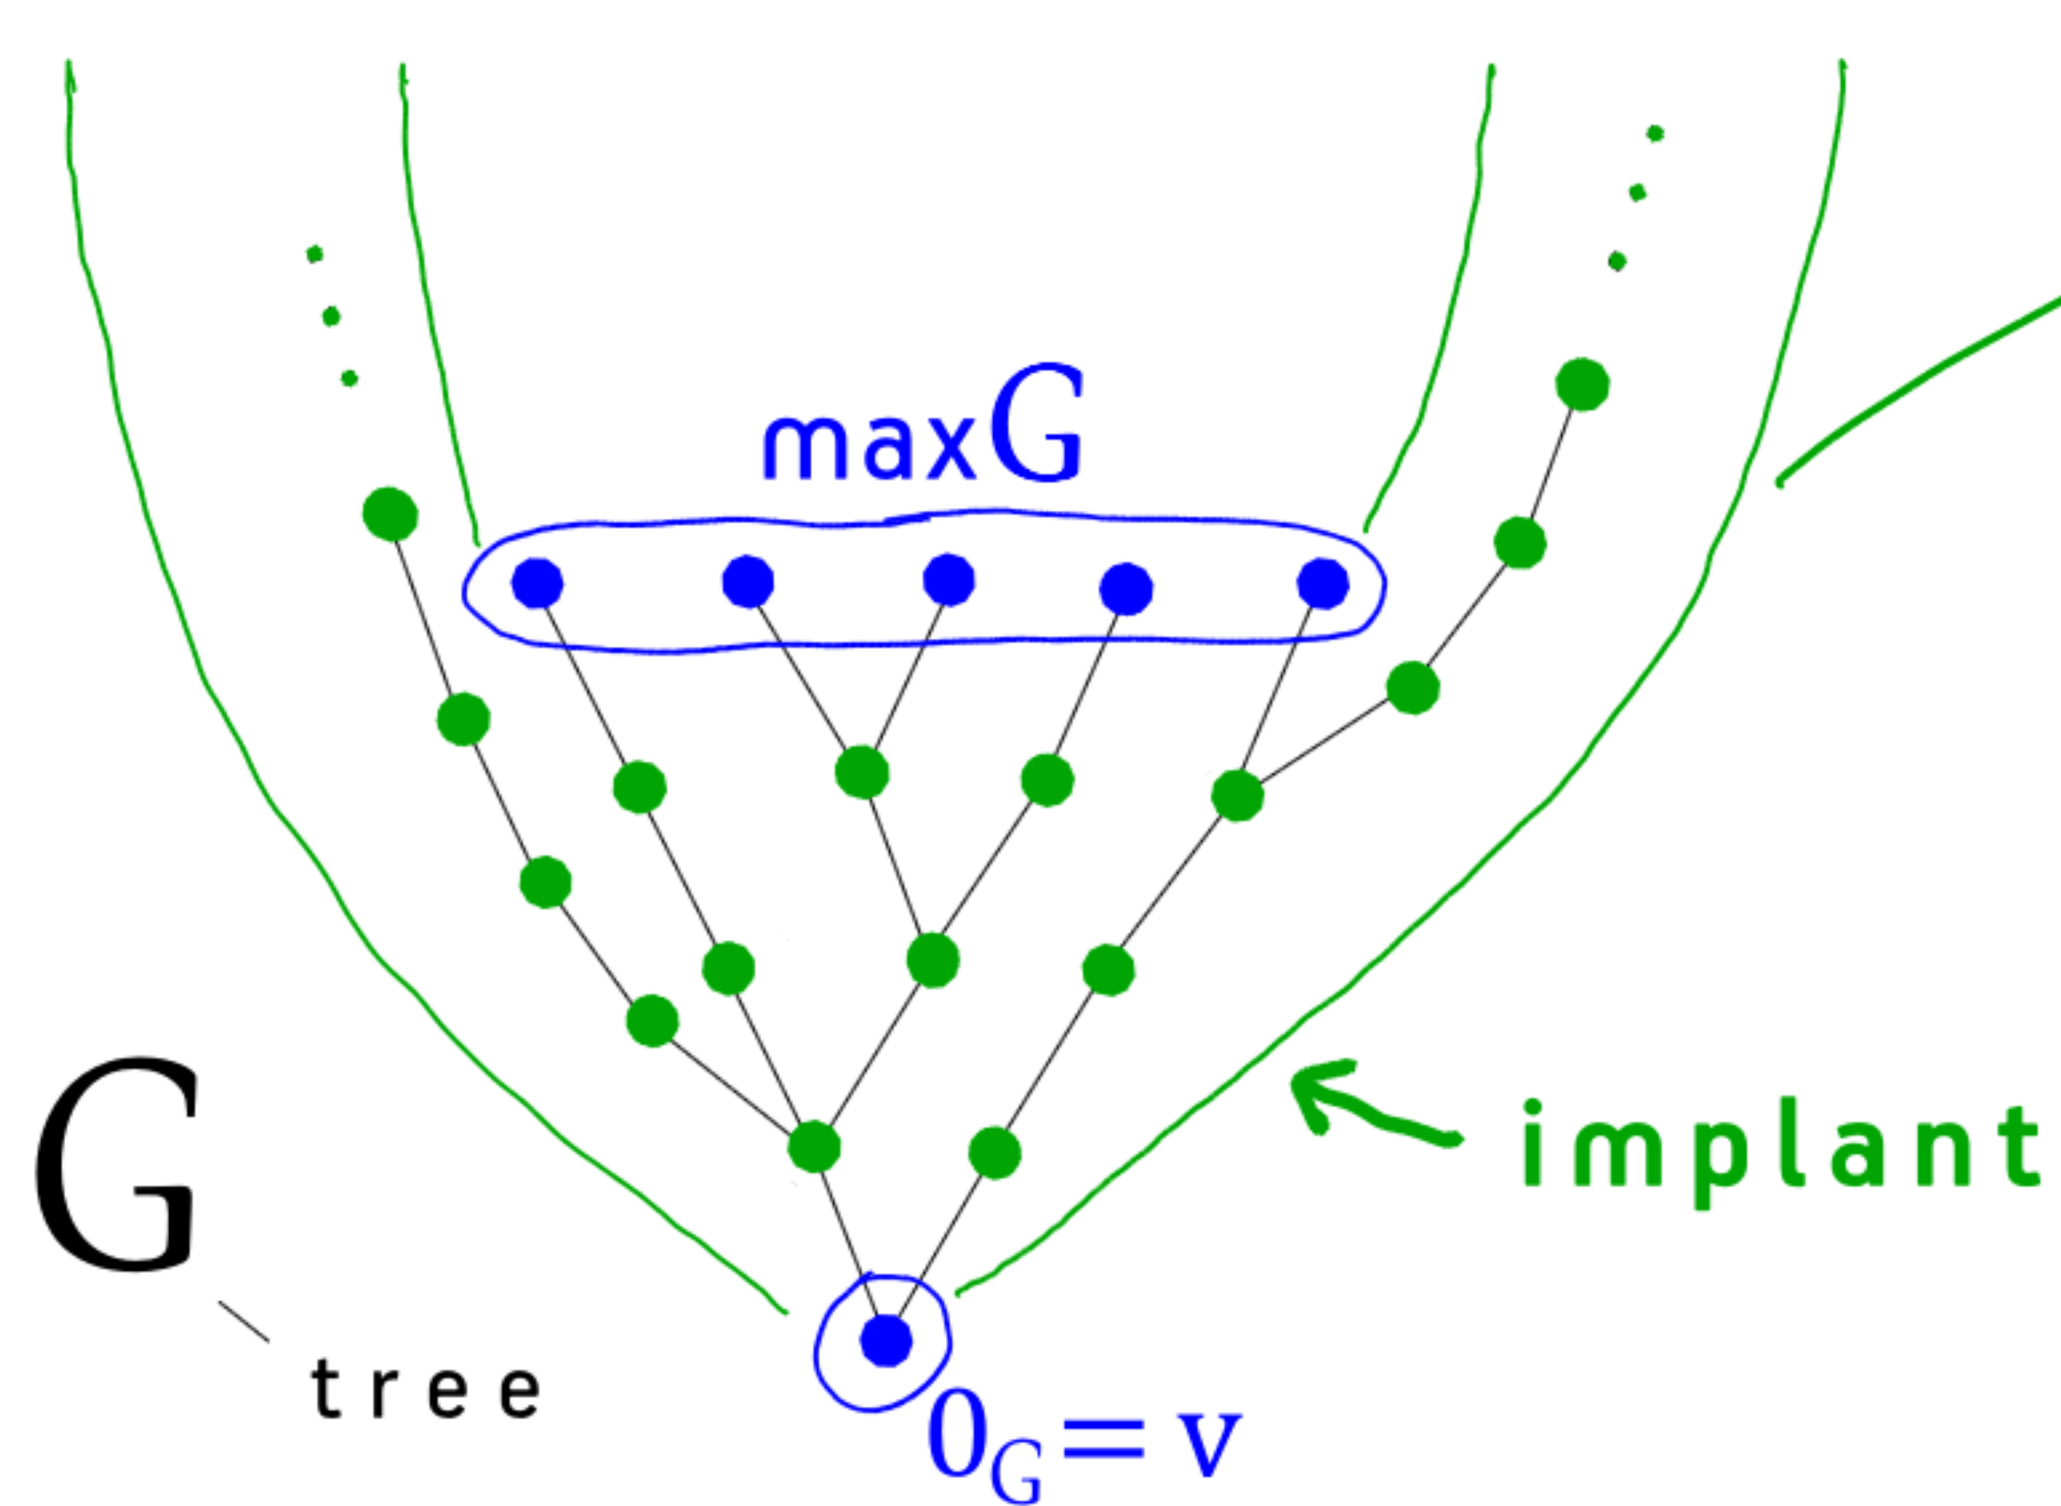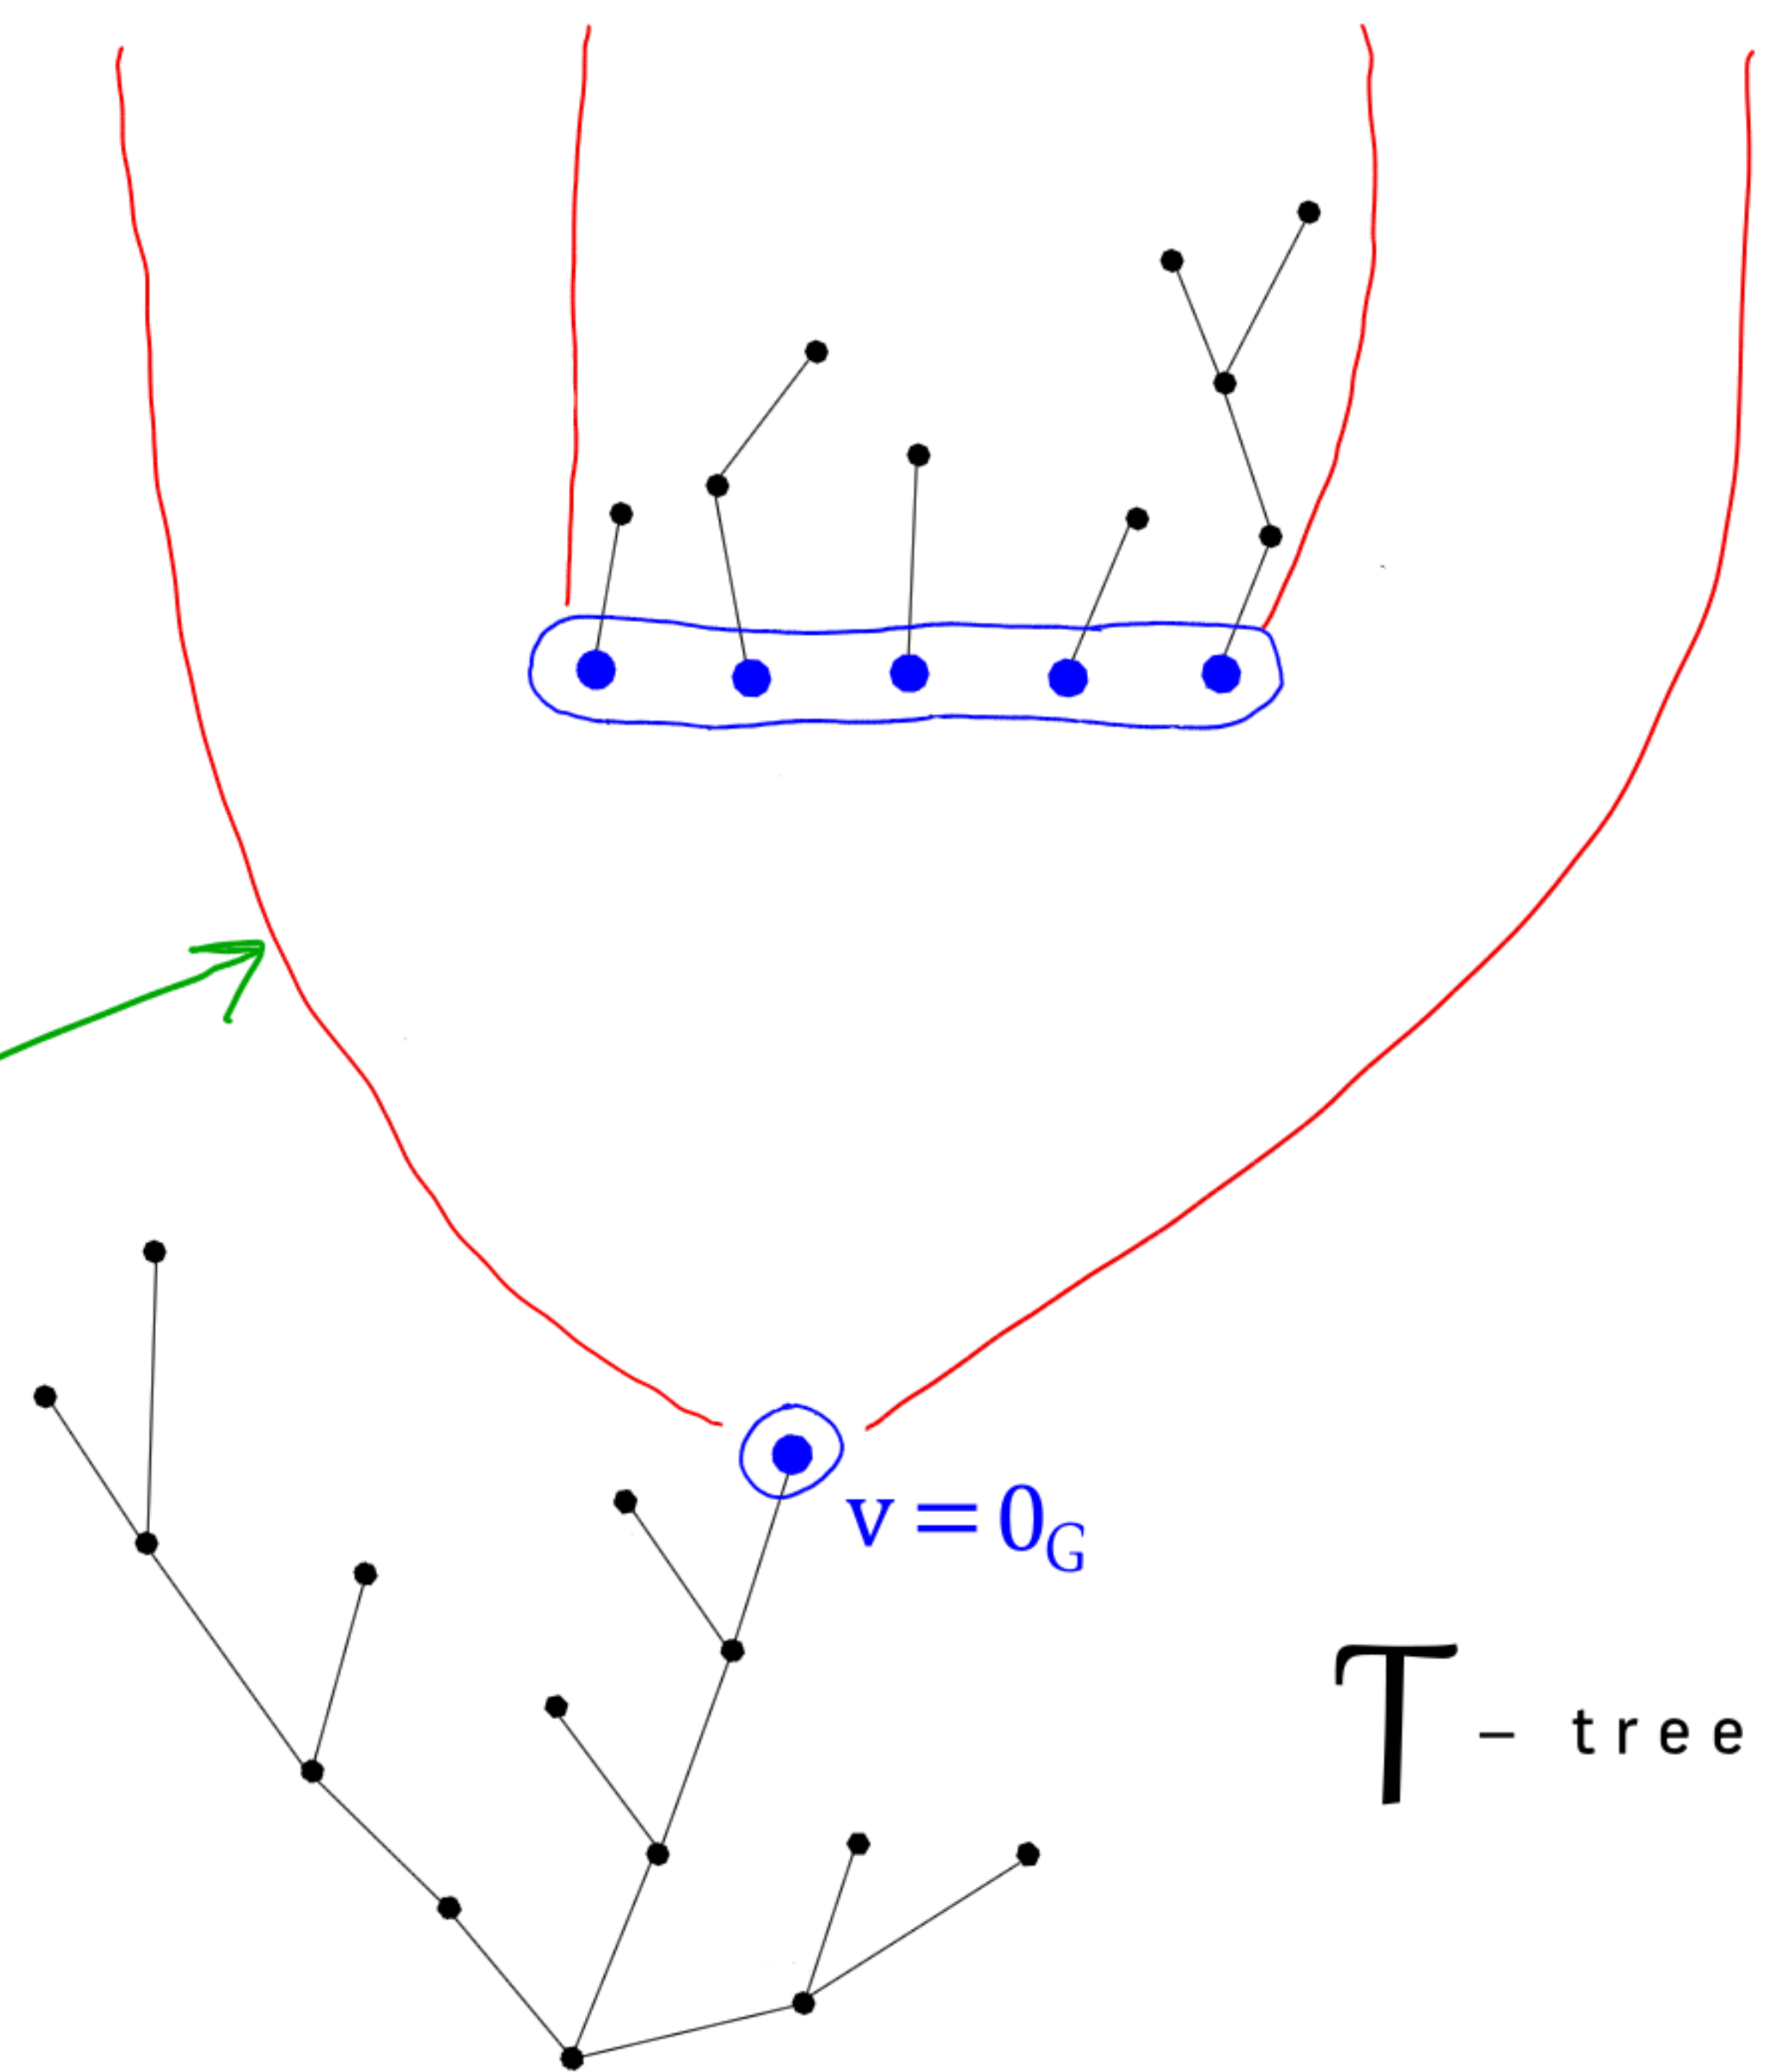

# HYBRID OPERATION

$G$  is a graft for  $T$  iff

$$(1) \quad G \cap T = \{0_G\} \cup \max G$$

$$(2) \quad <_G \upharpoonright (G \cap T) = <_T \upharpoonright (G \cap T)$$

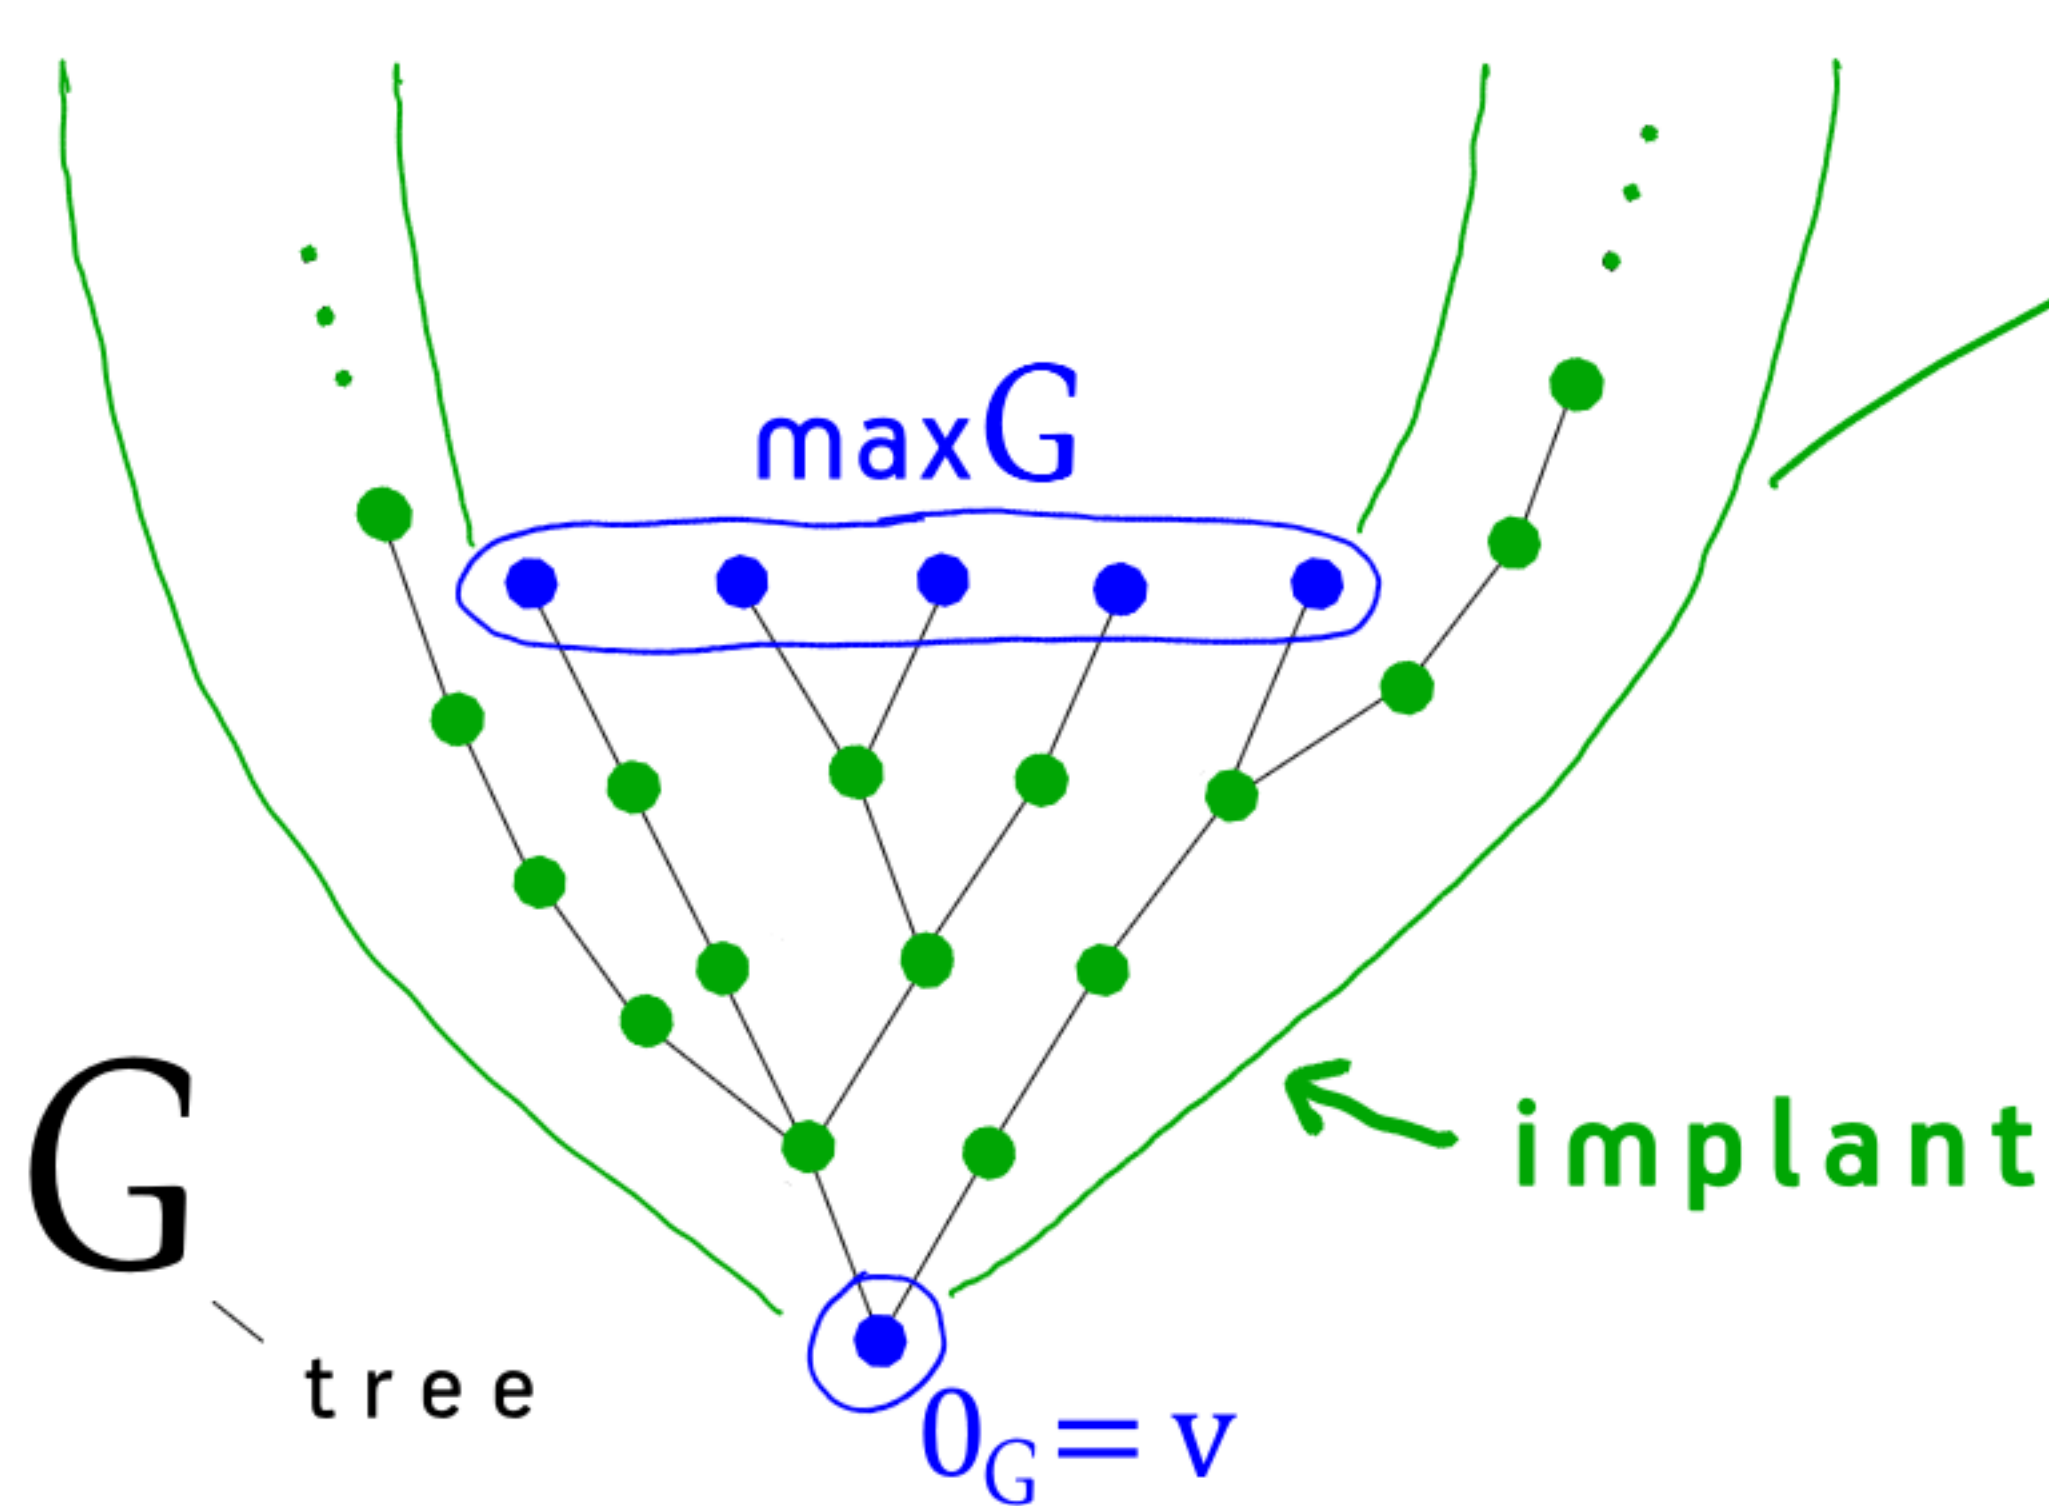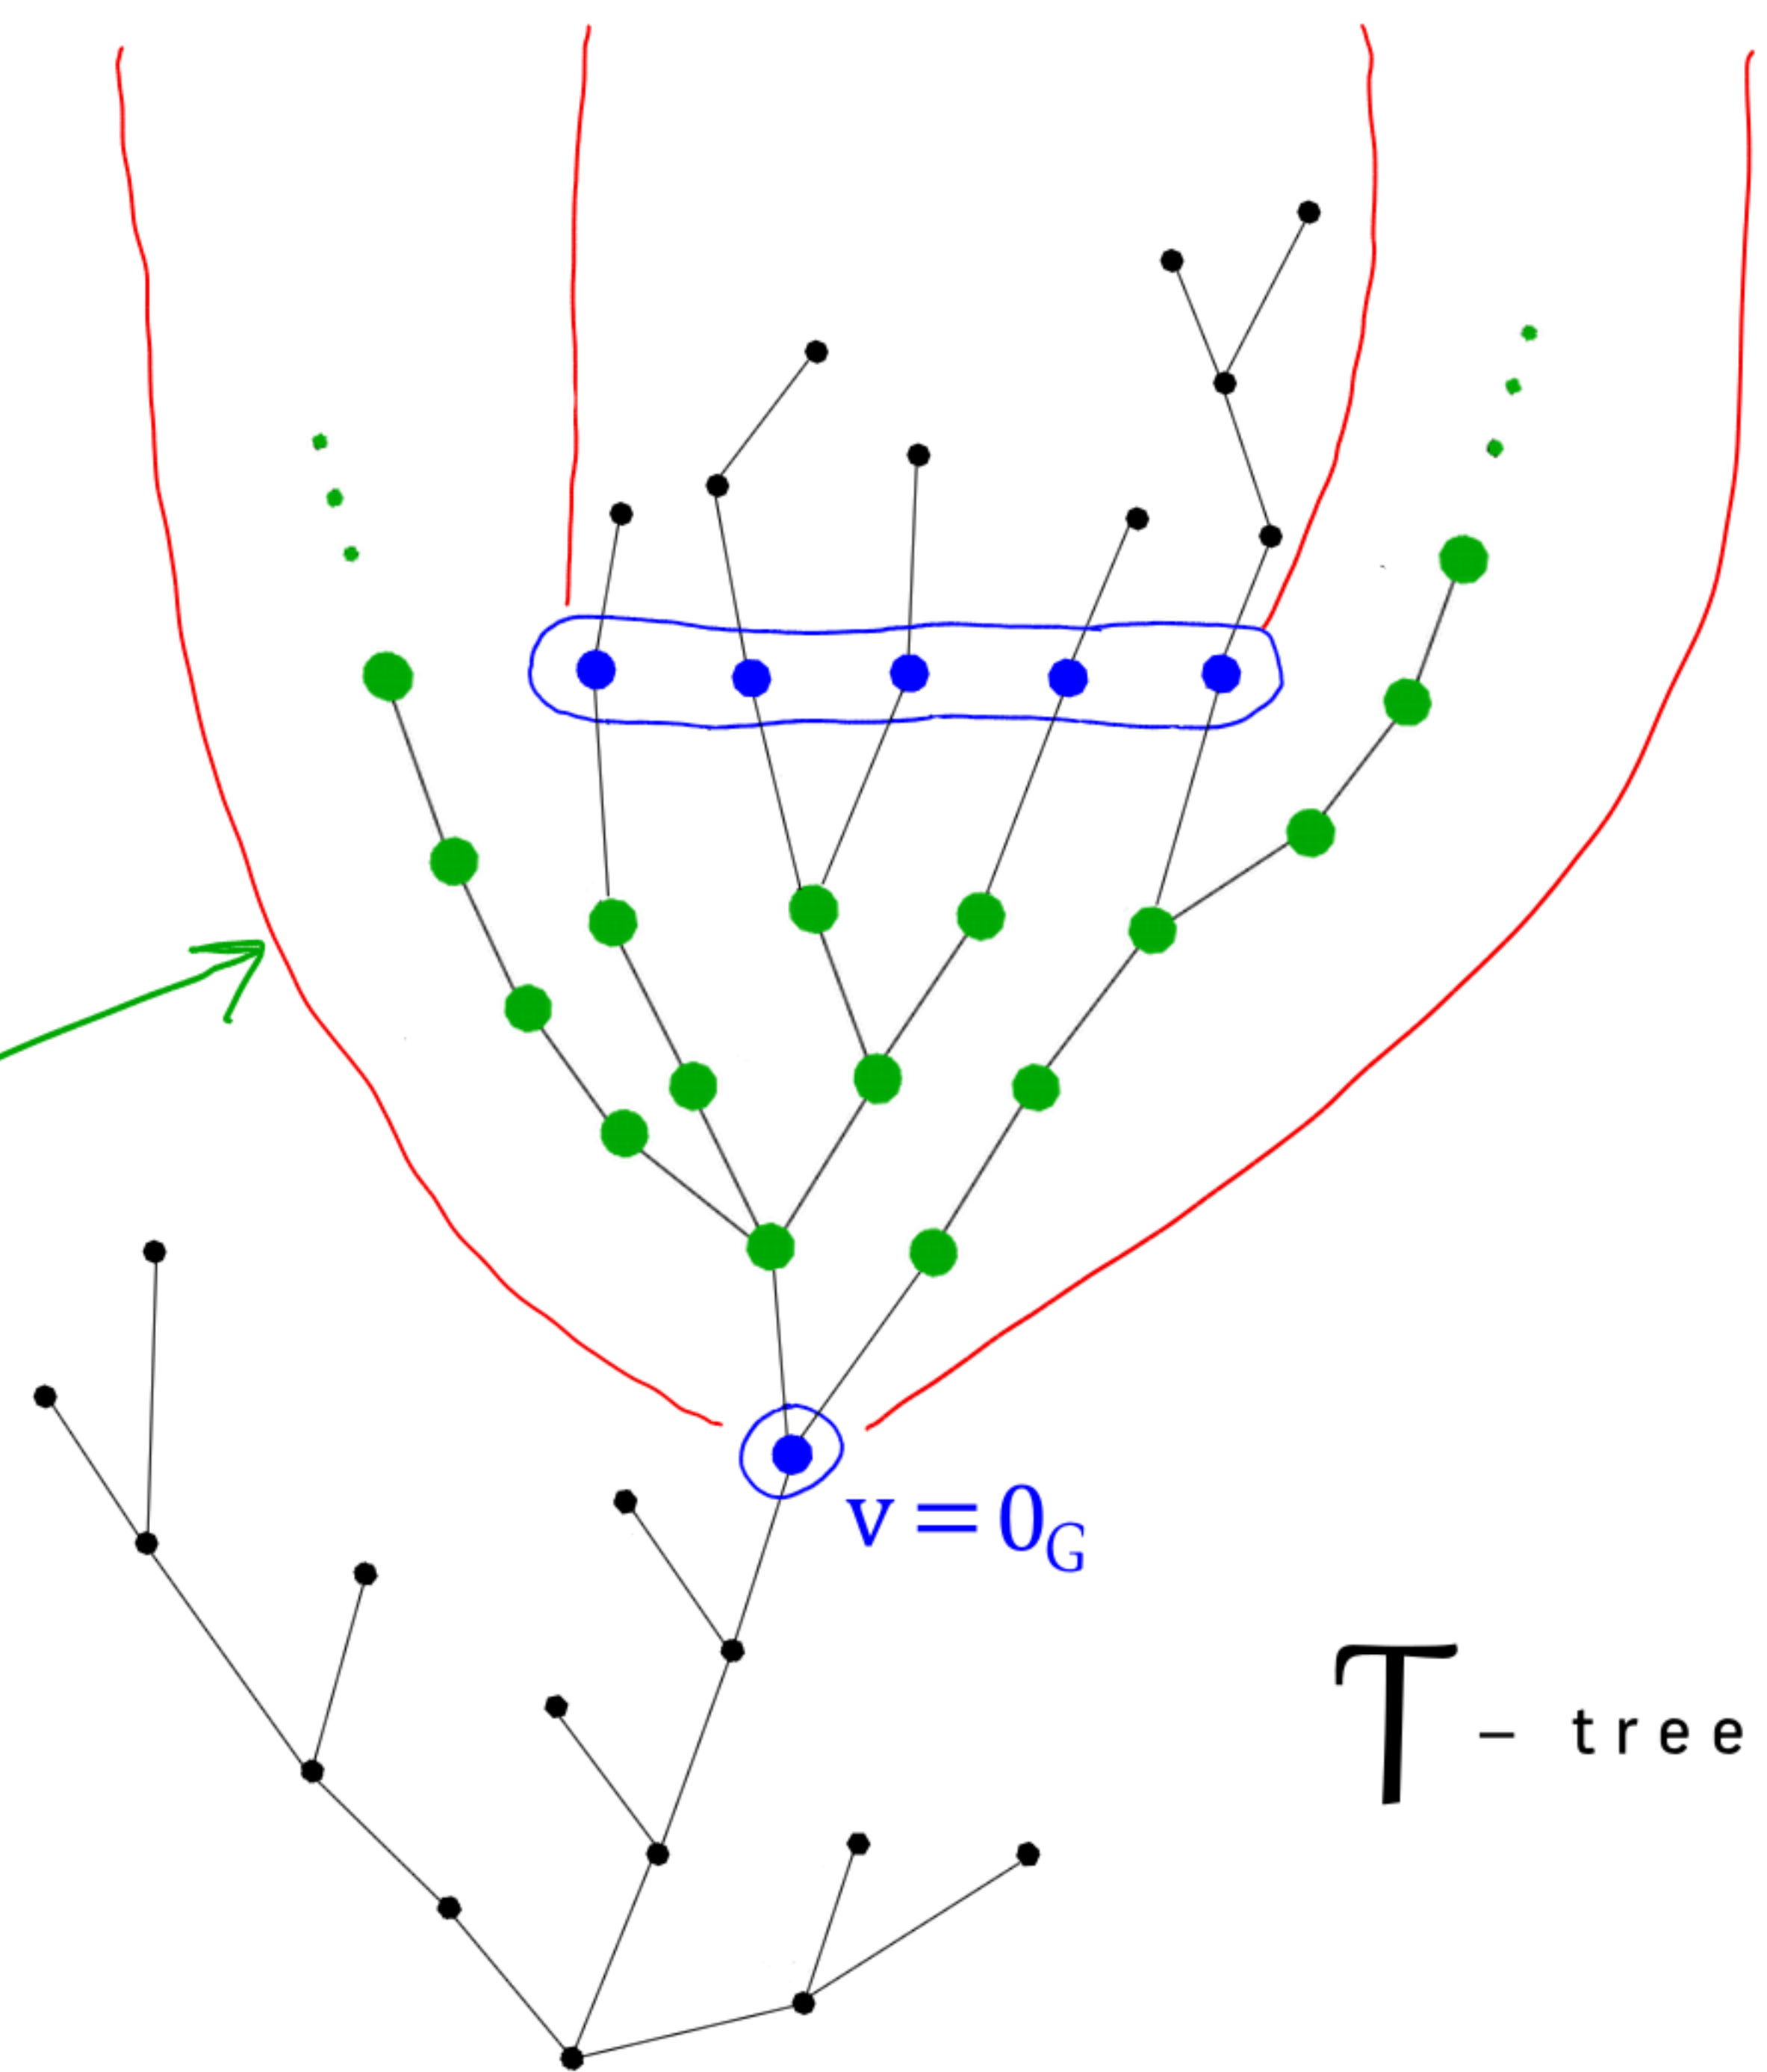

# HYBRID OPERATION

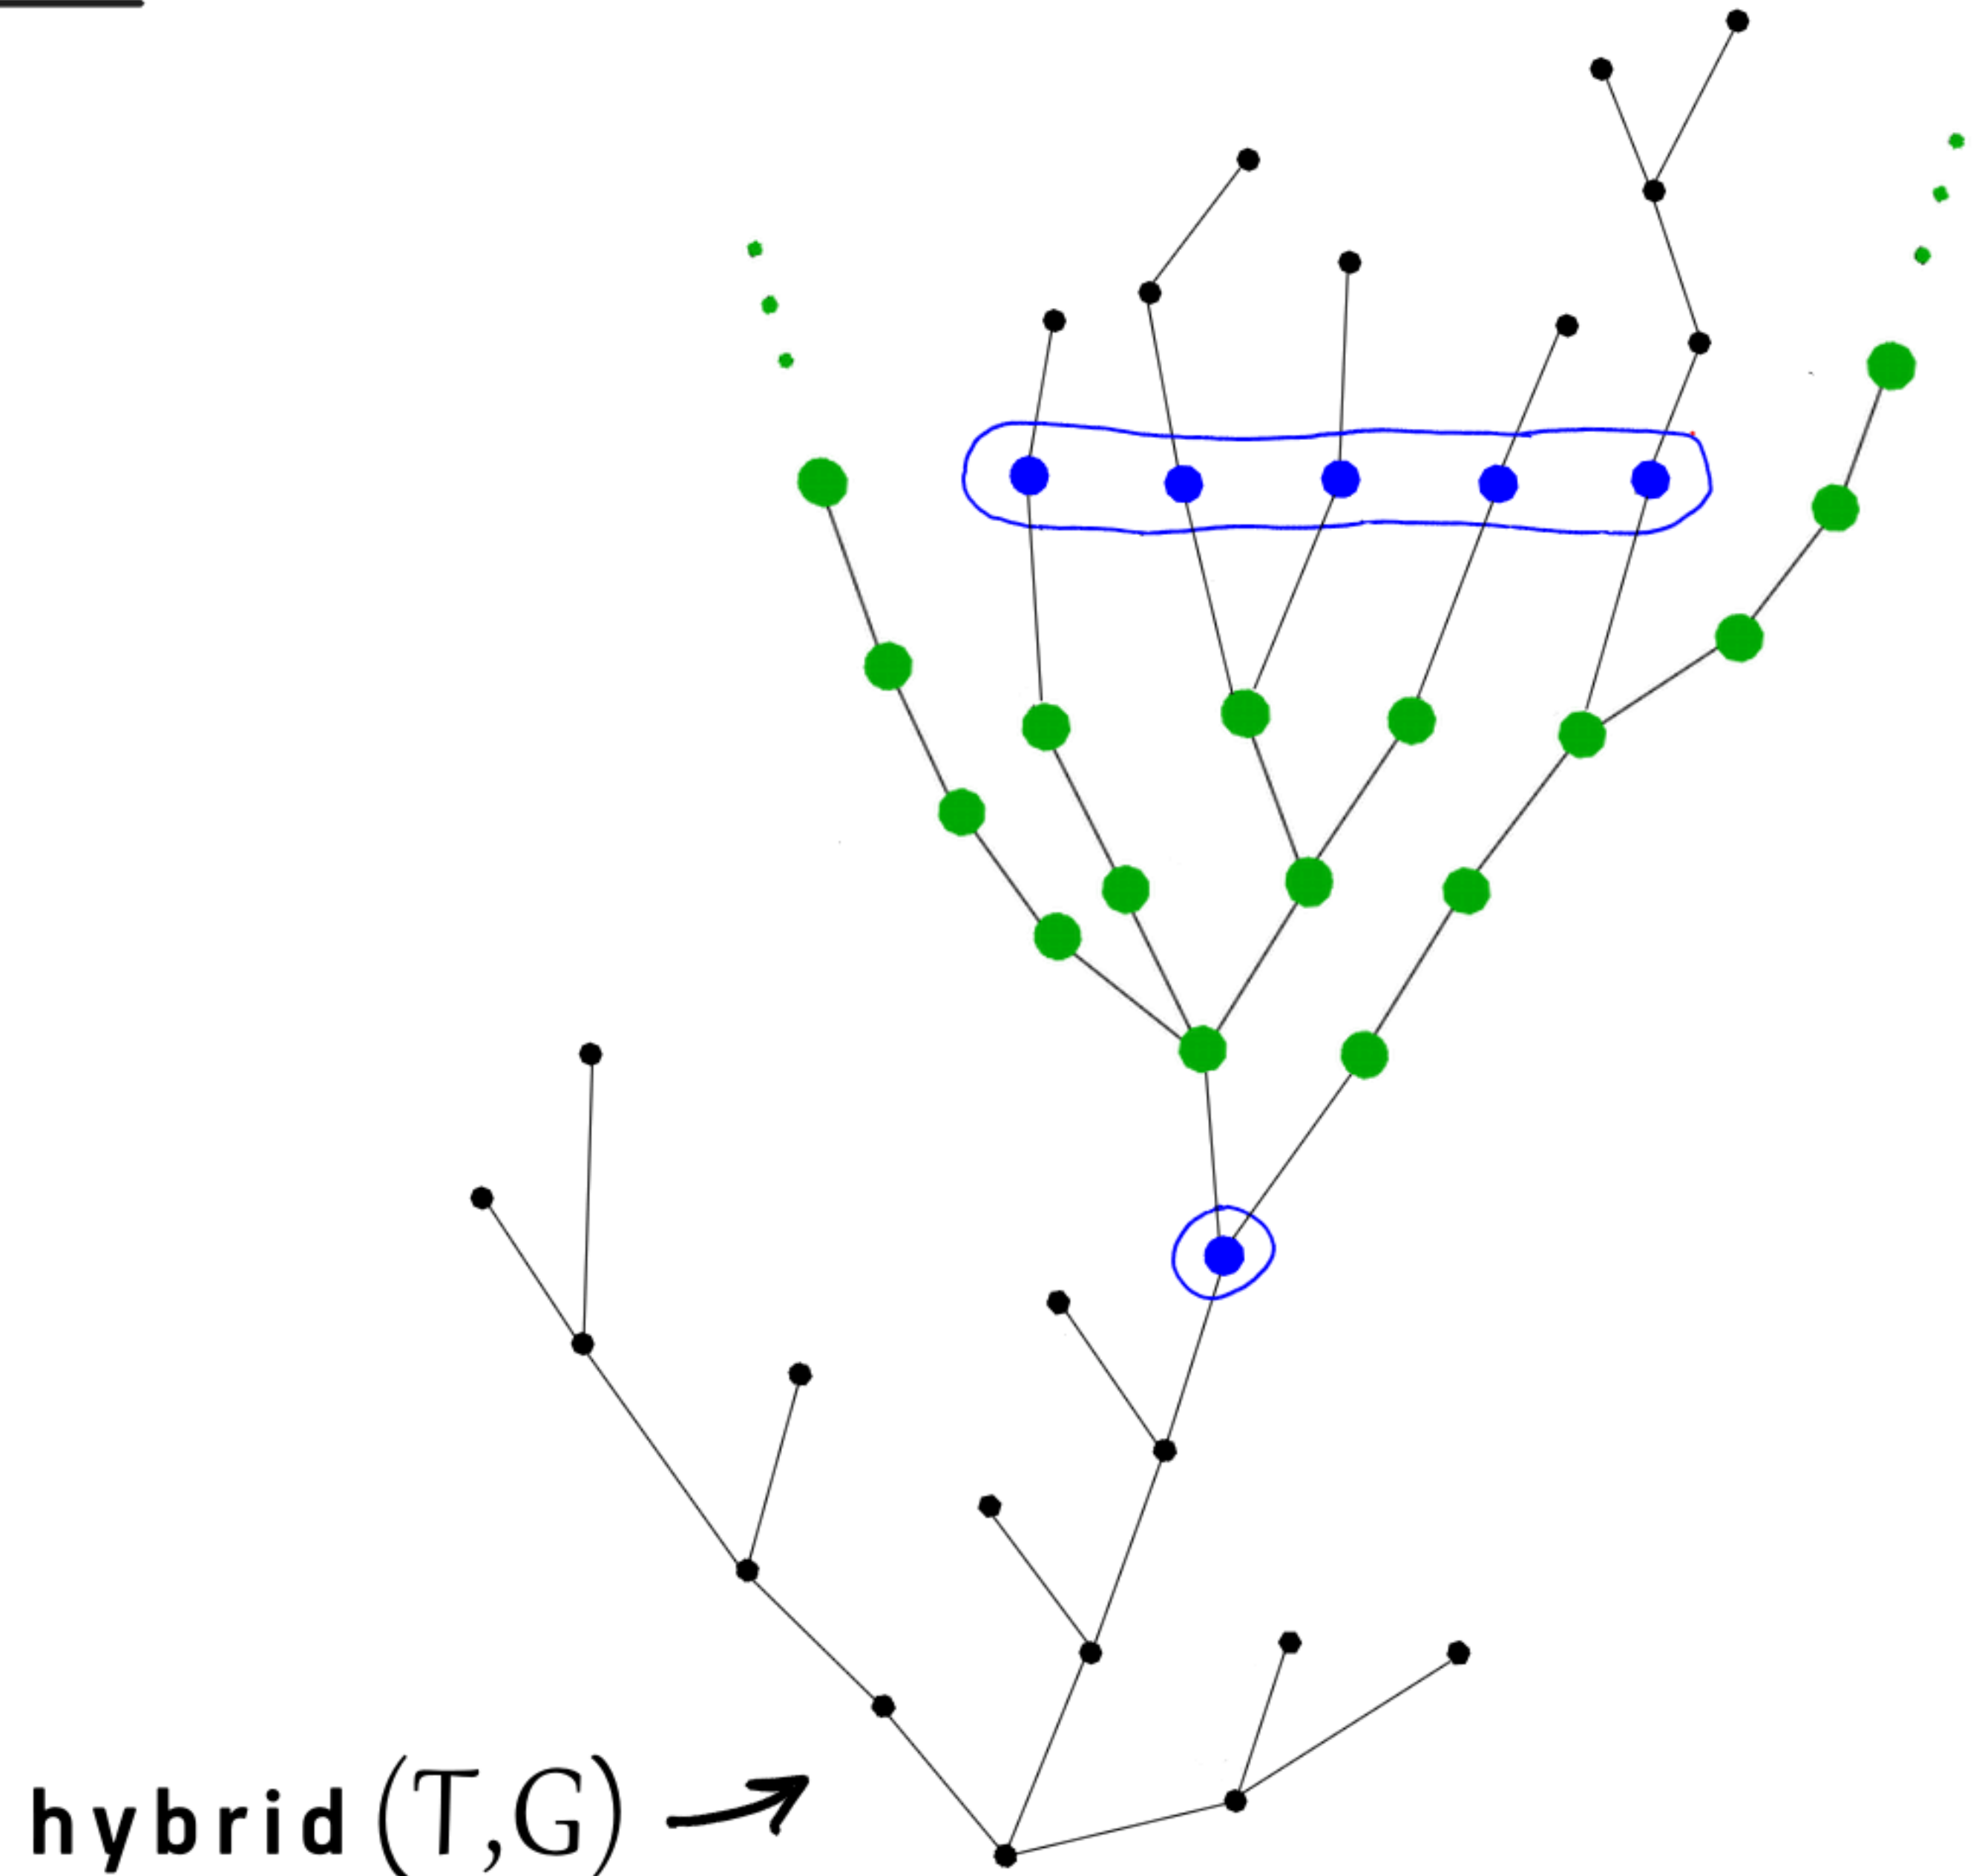

# HYBRID OPERATION

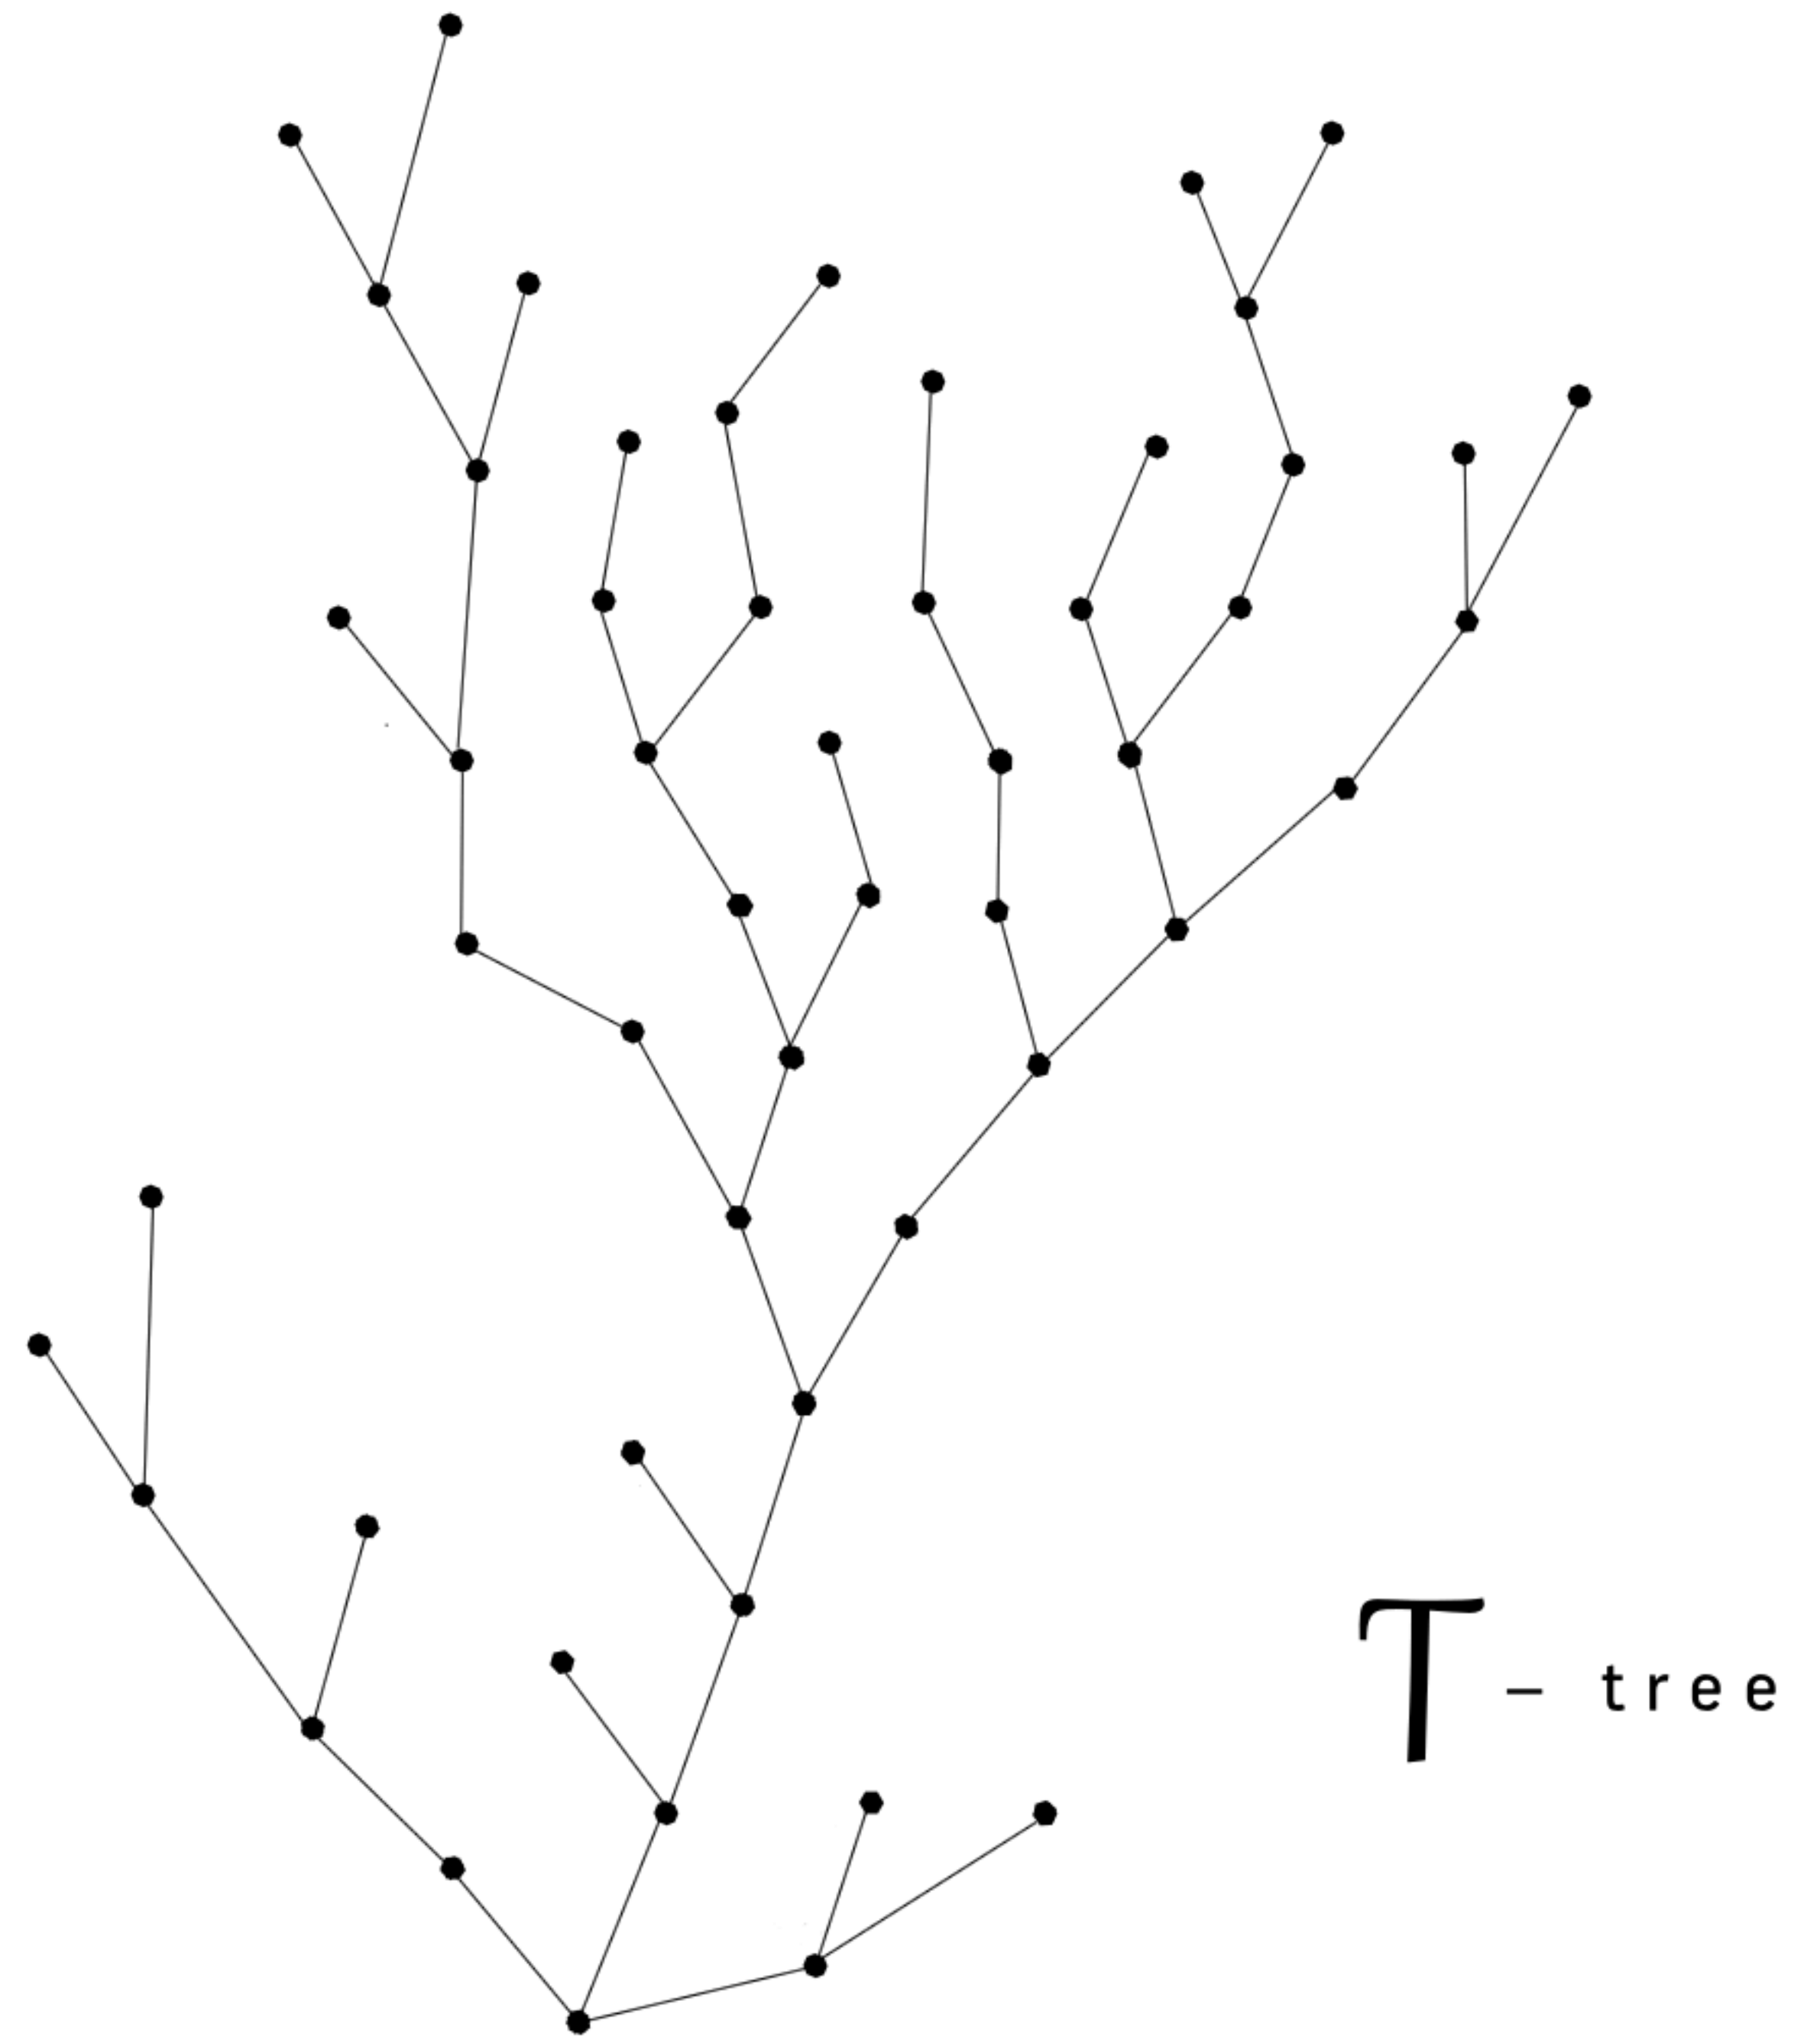



# HYBRID OPERATION

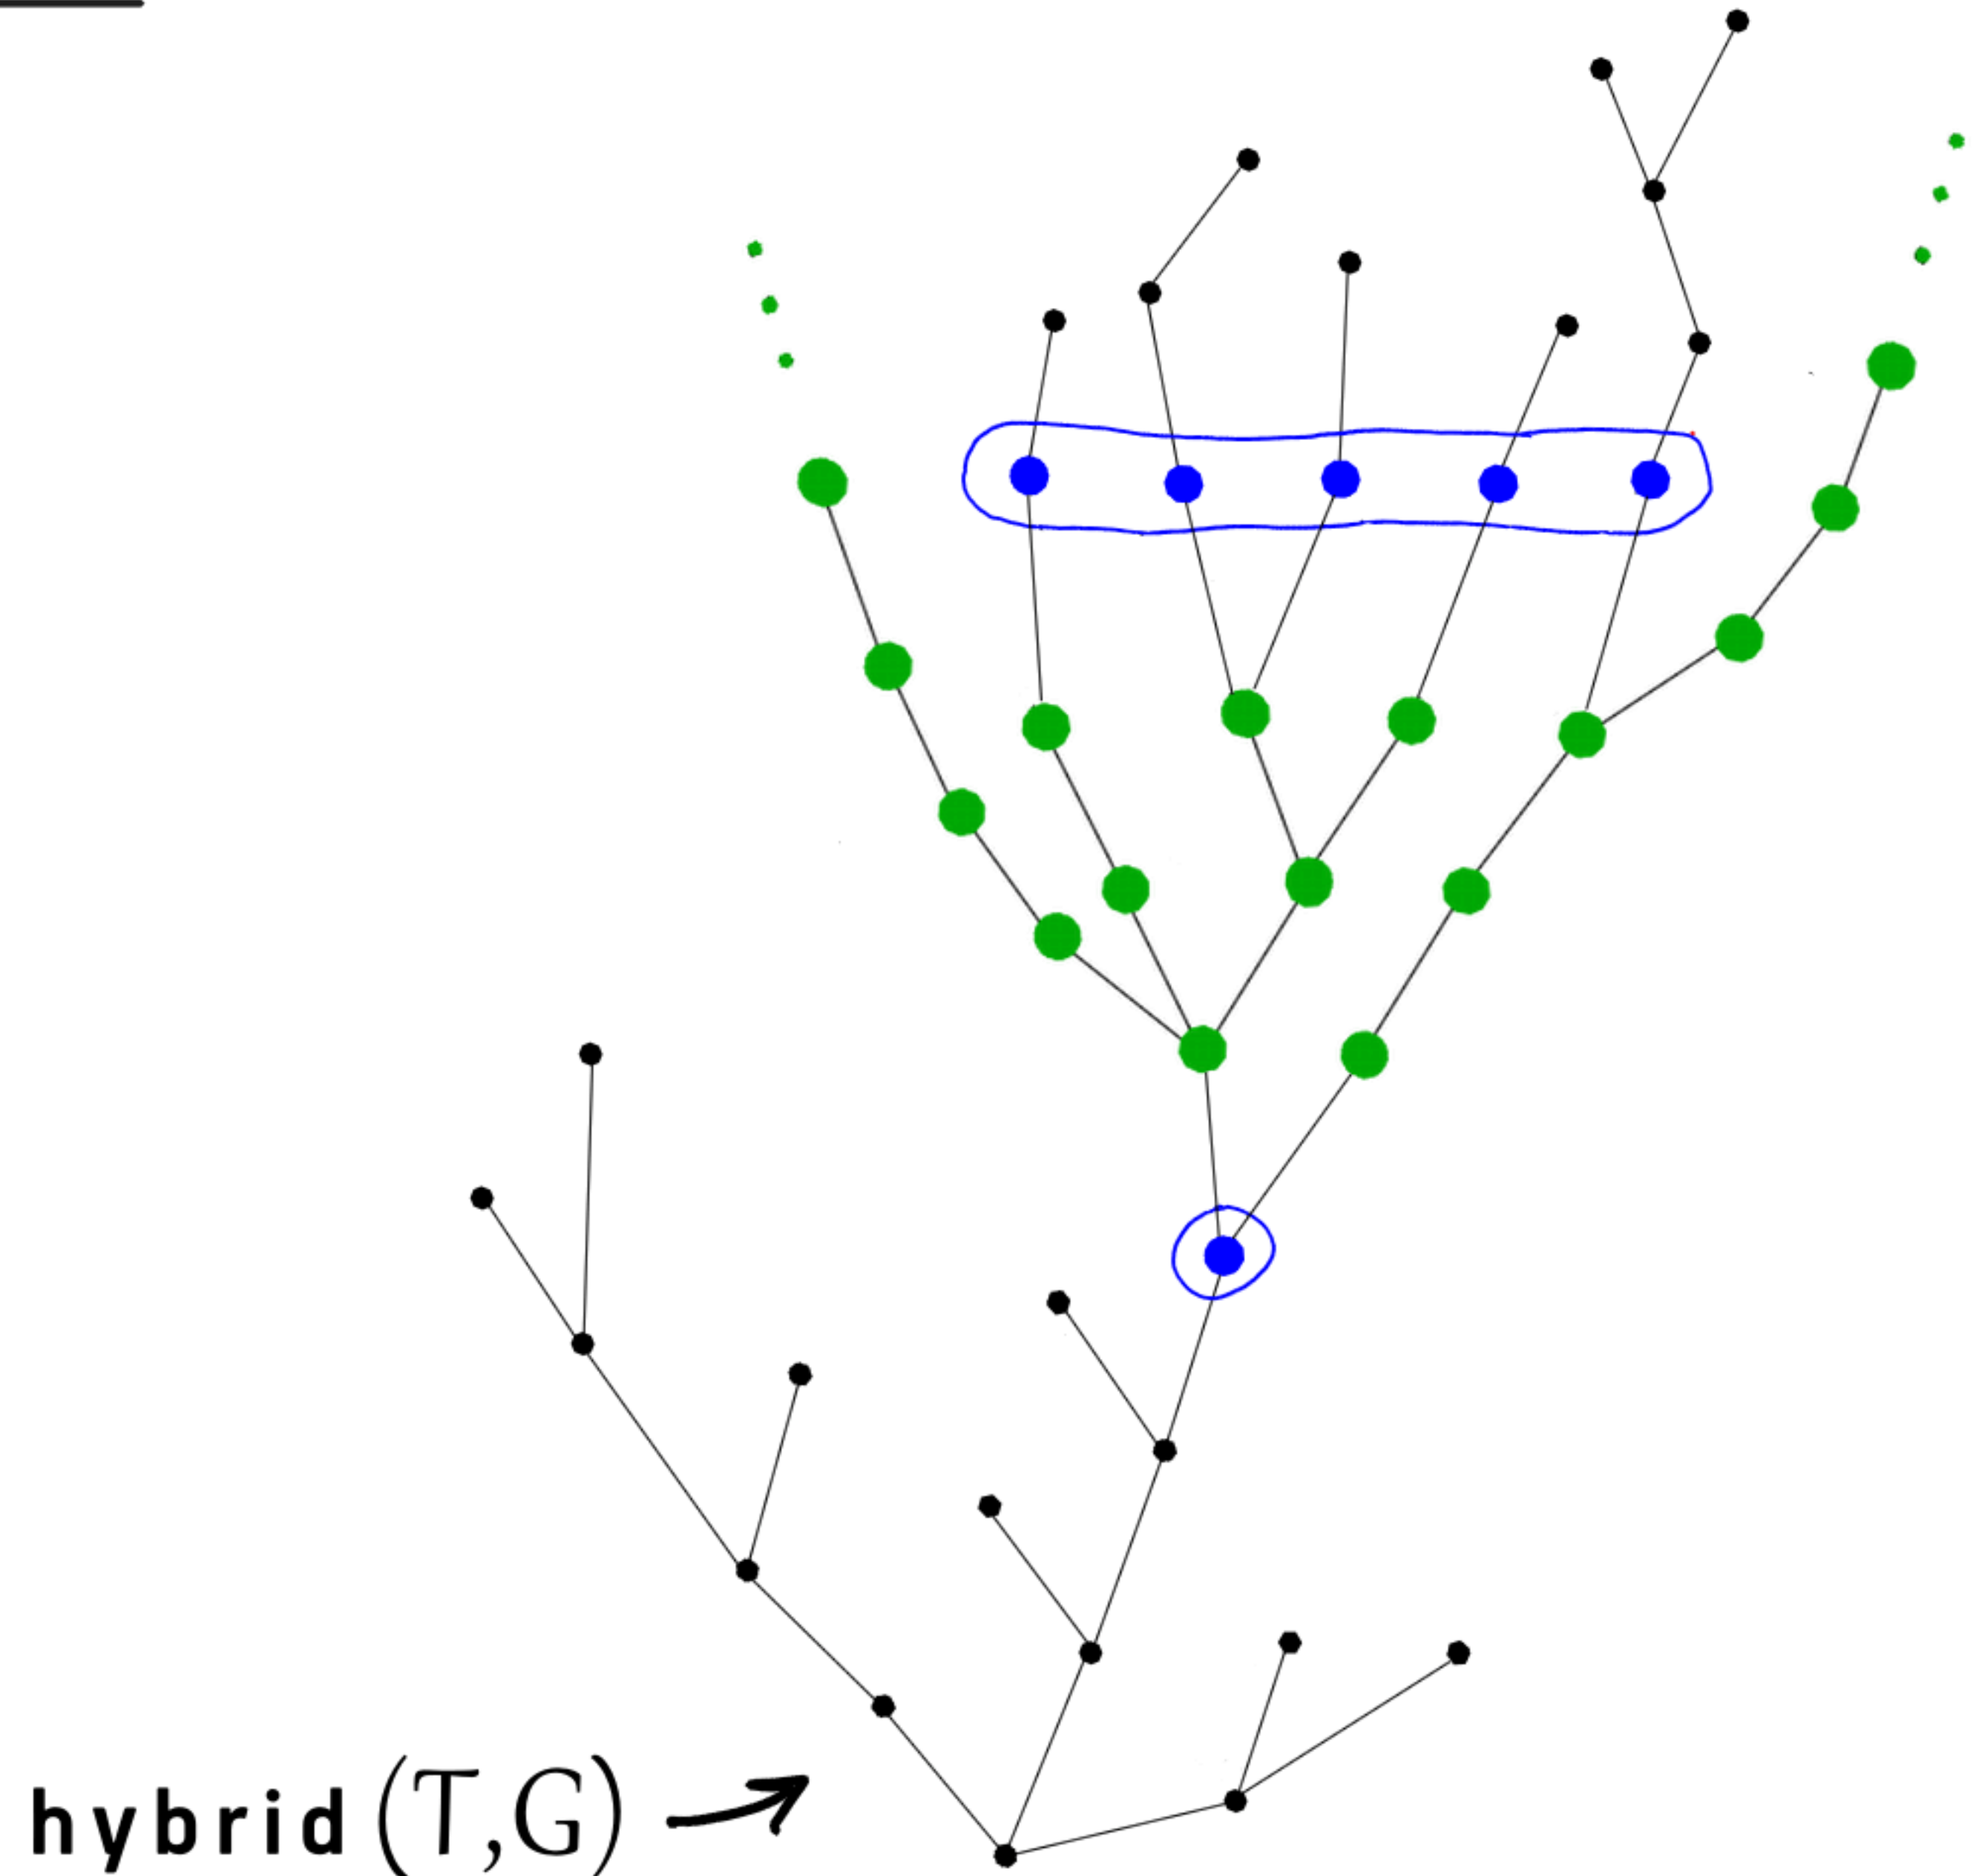

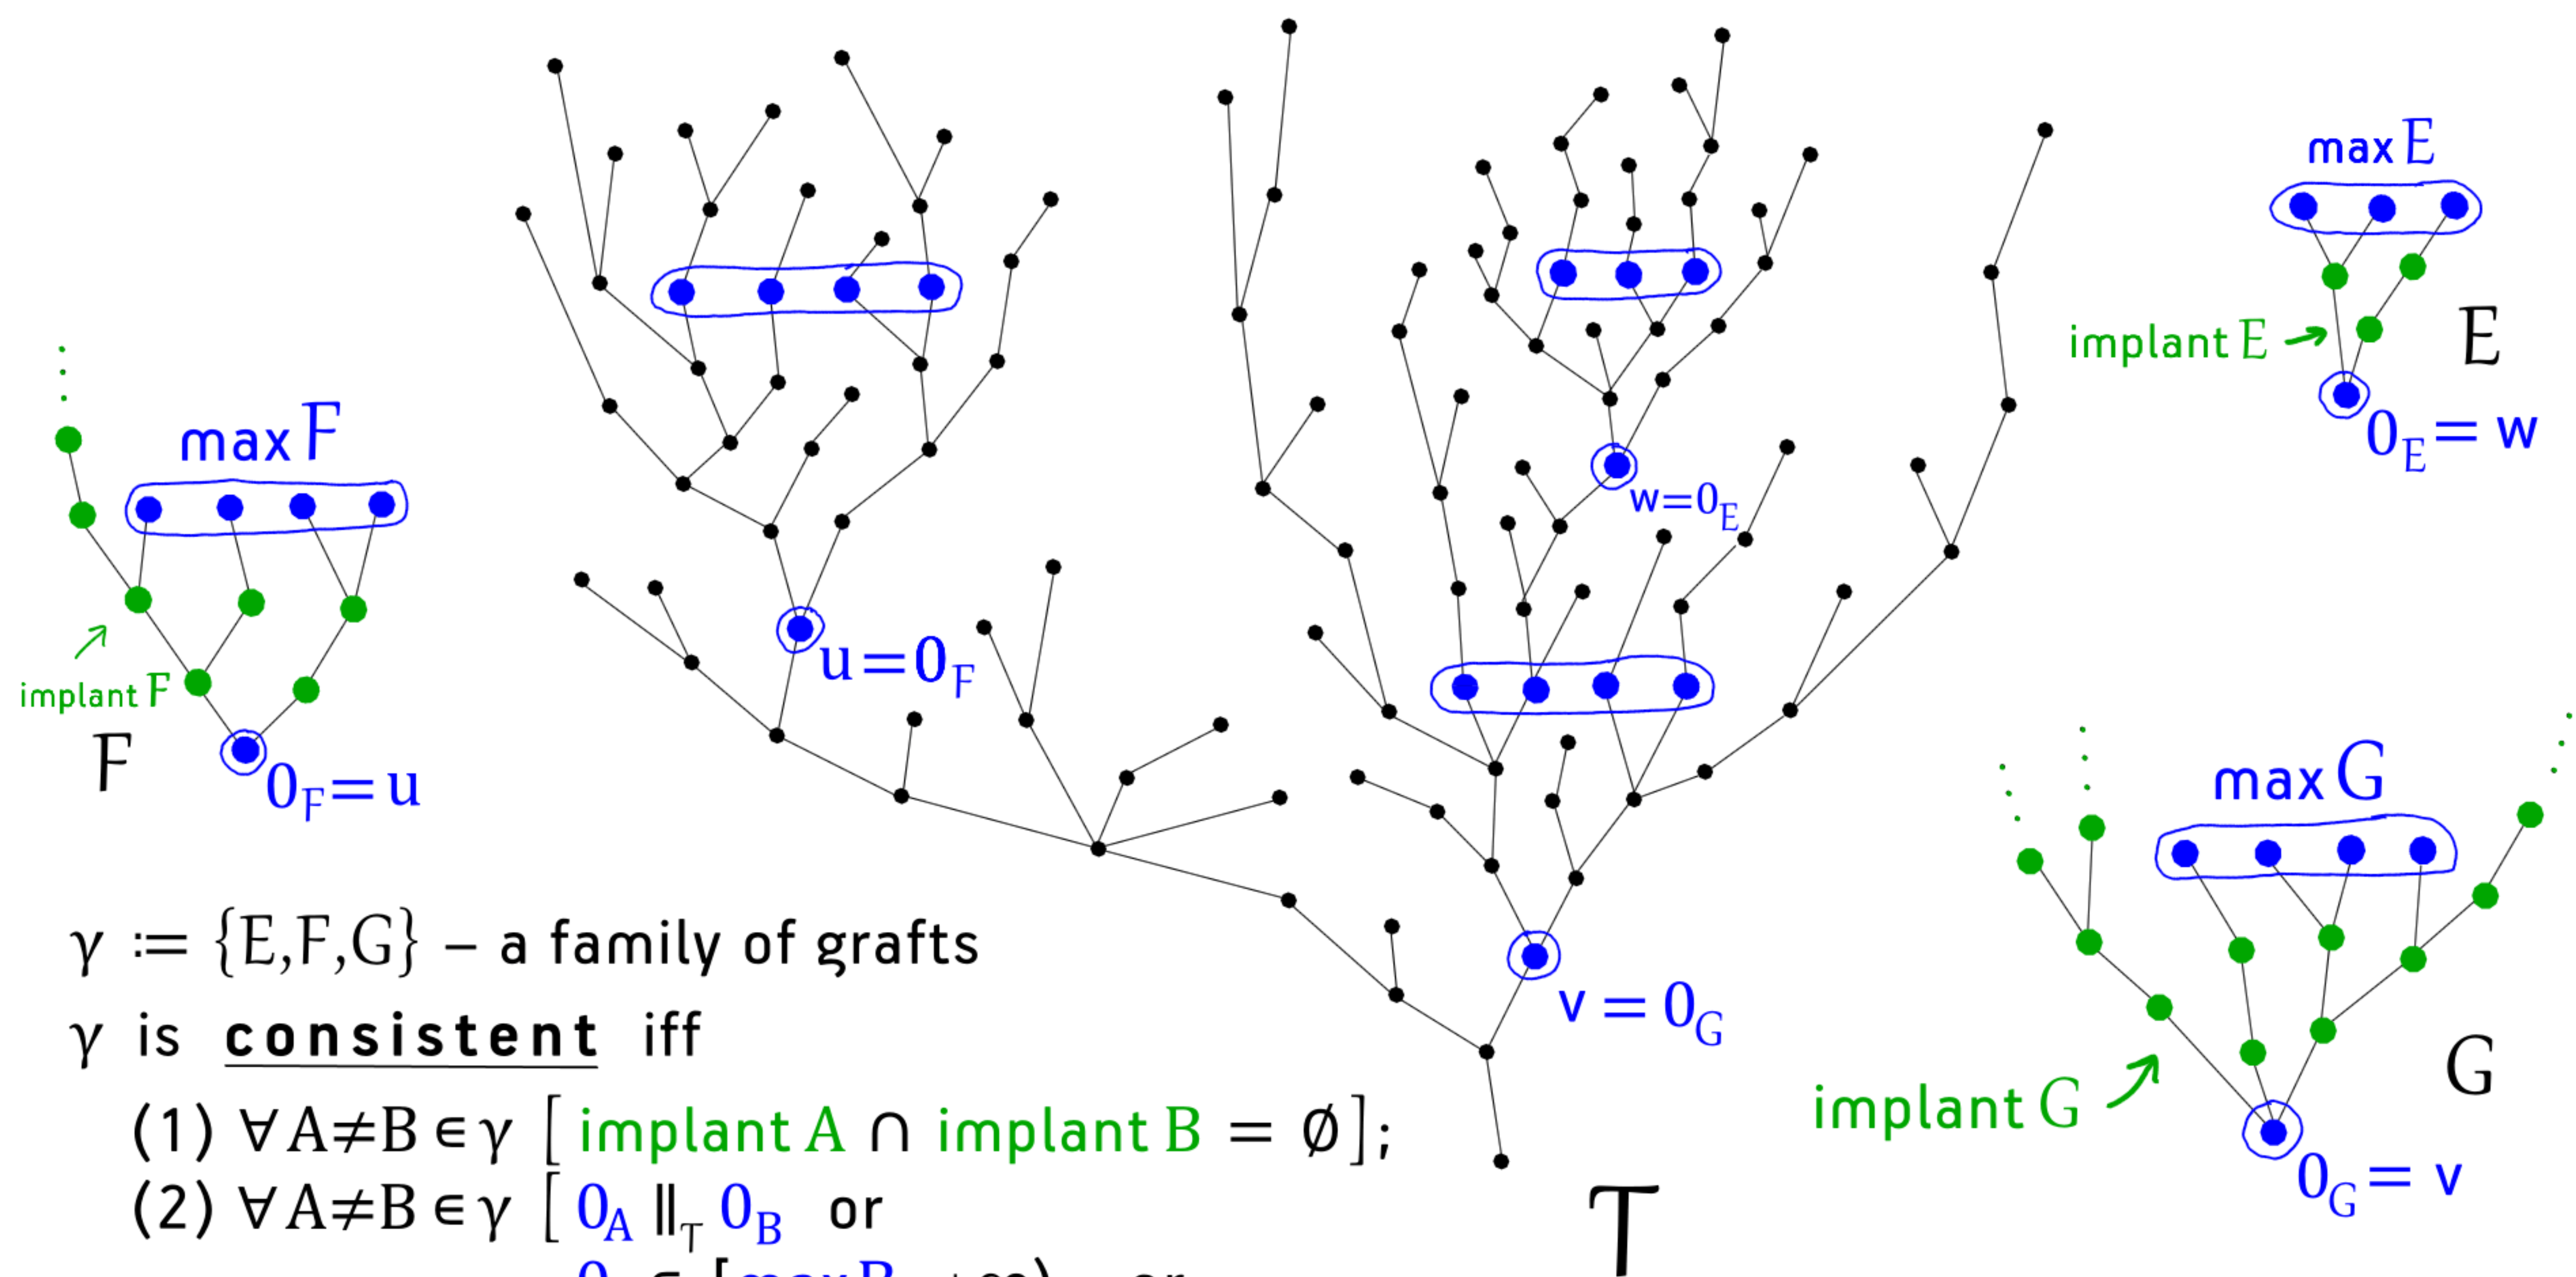



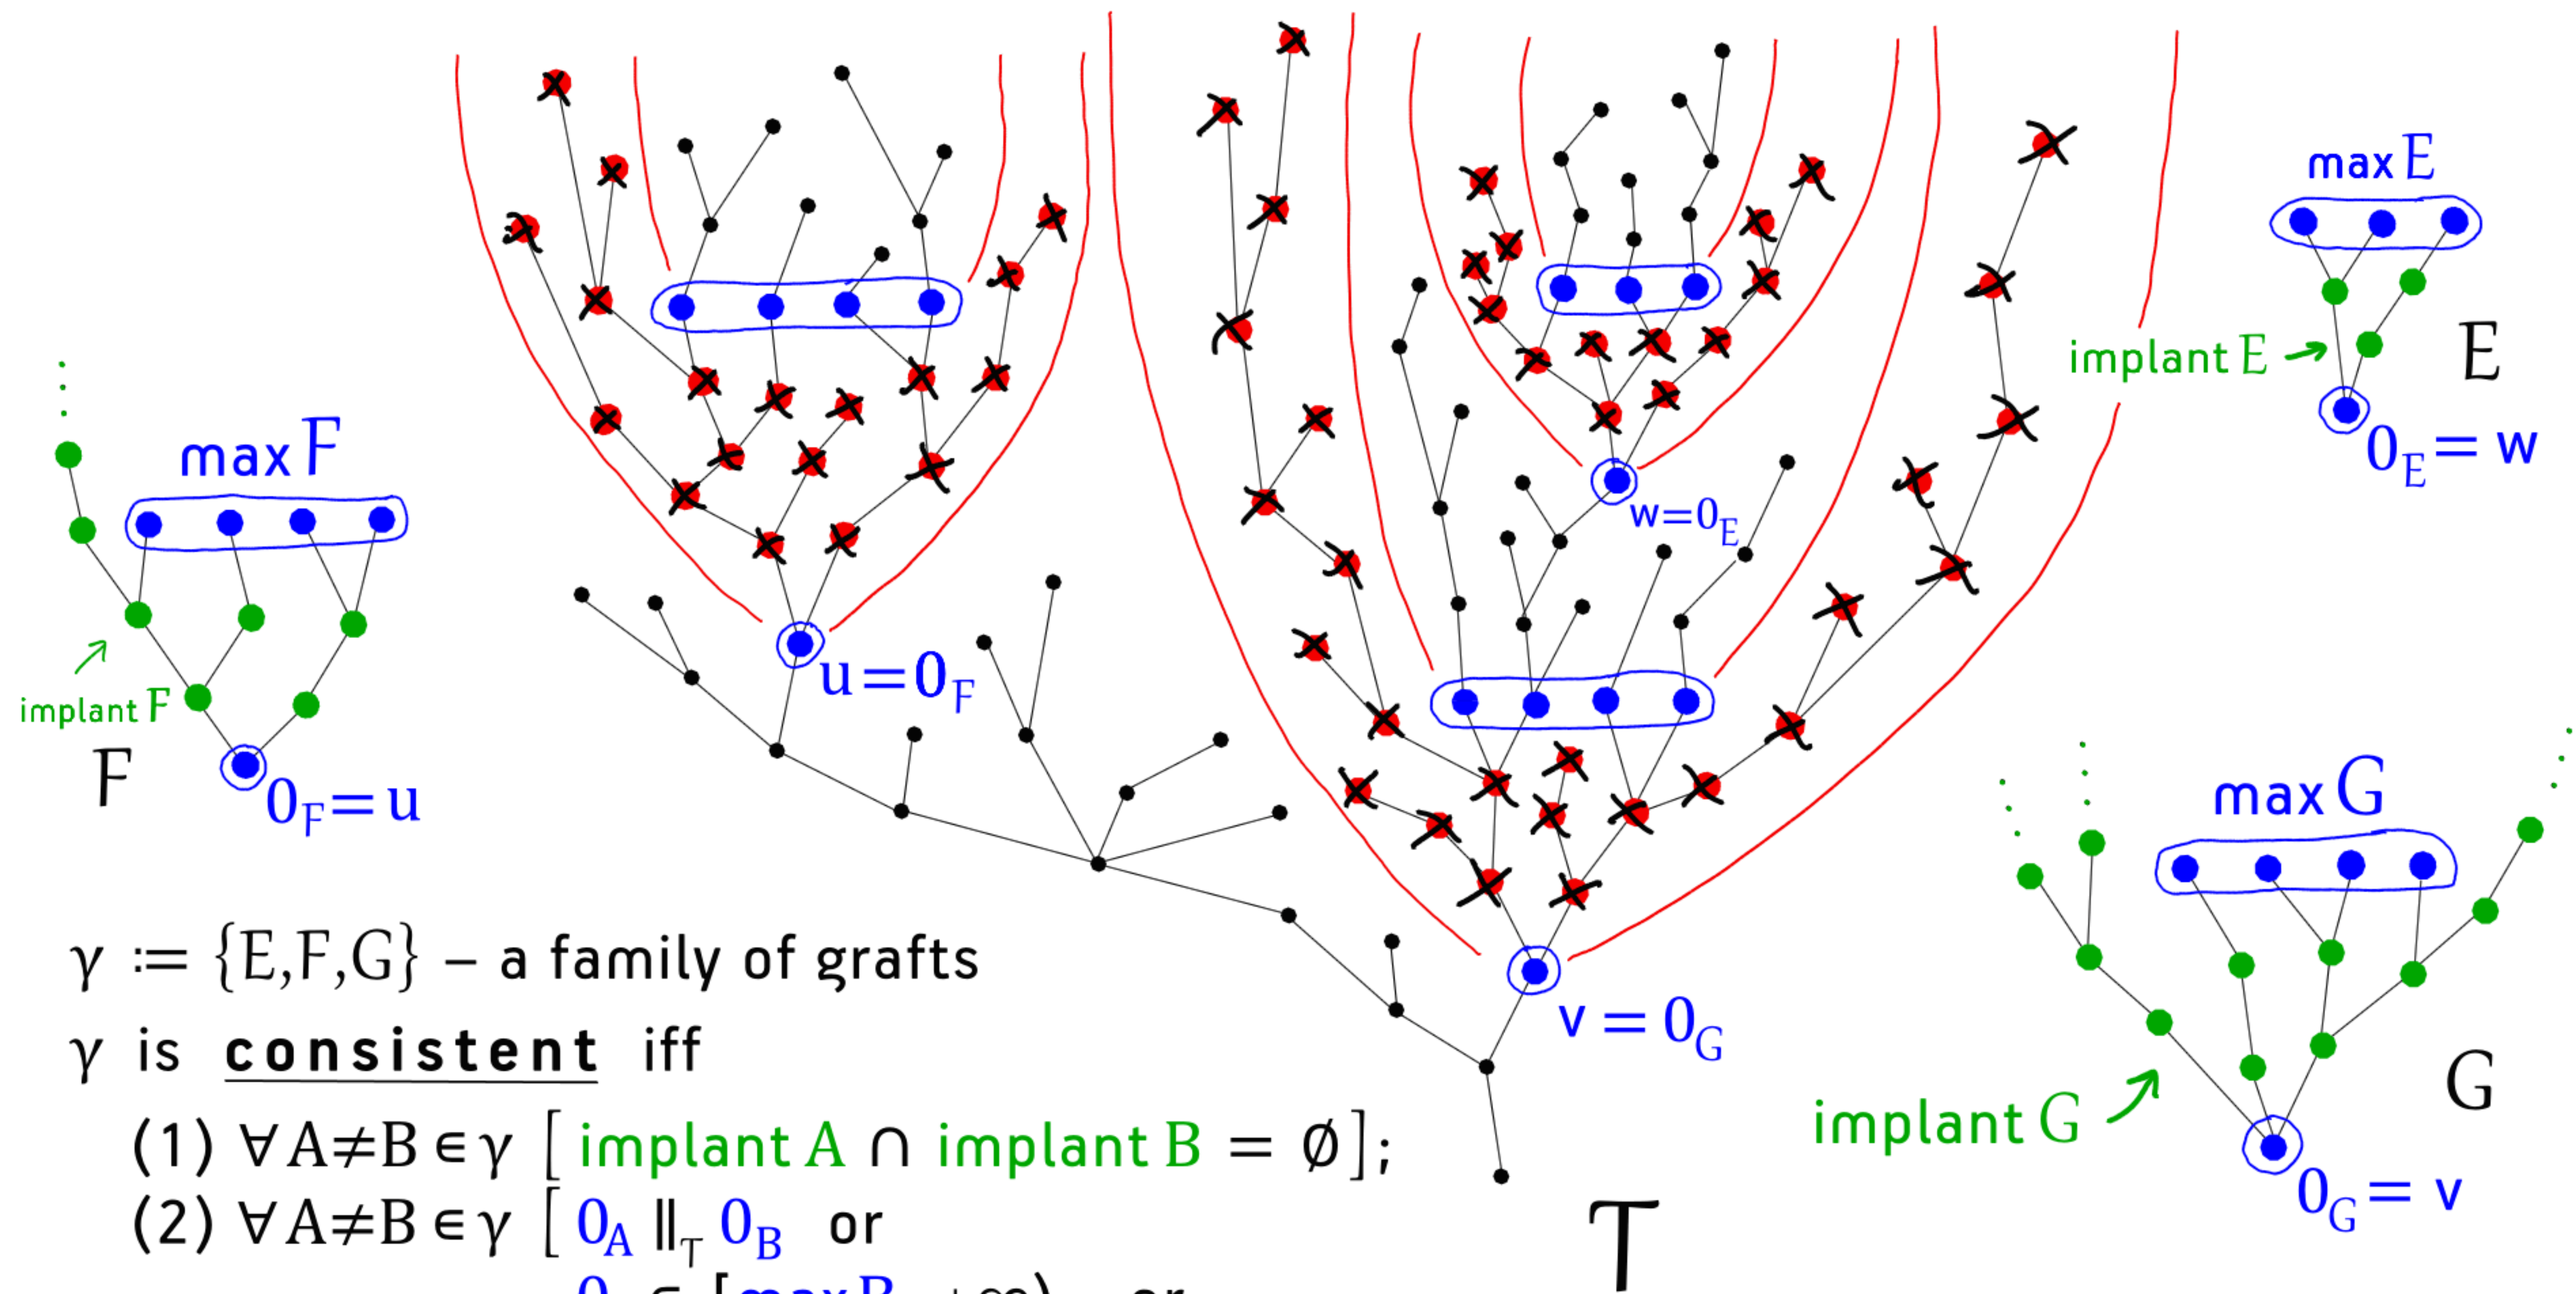



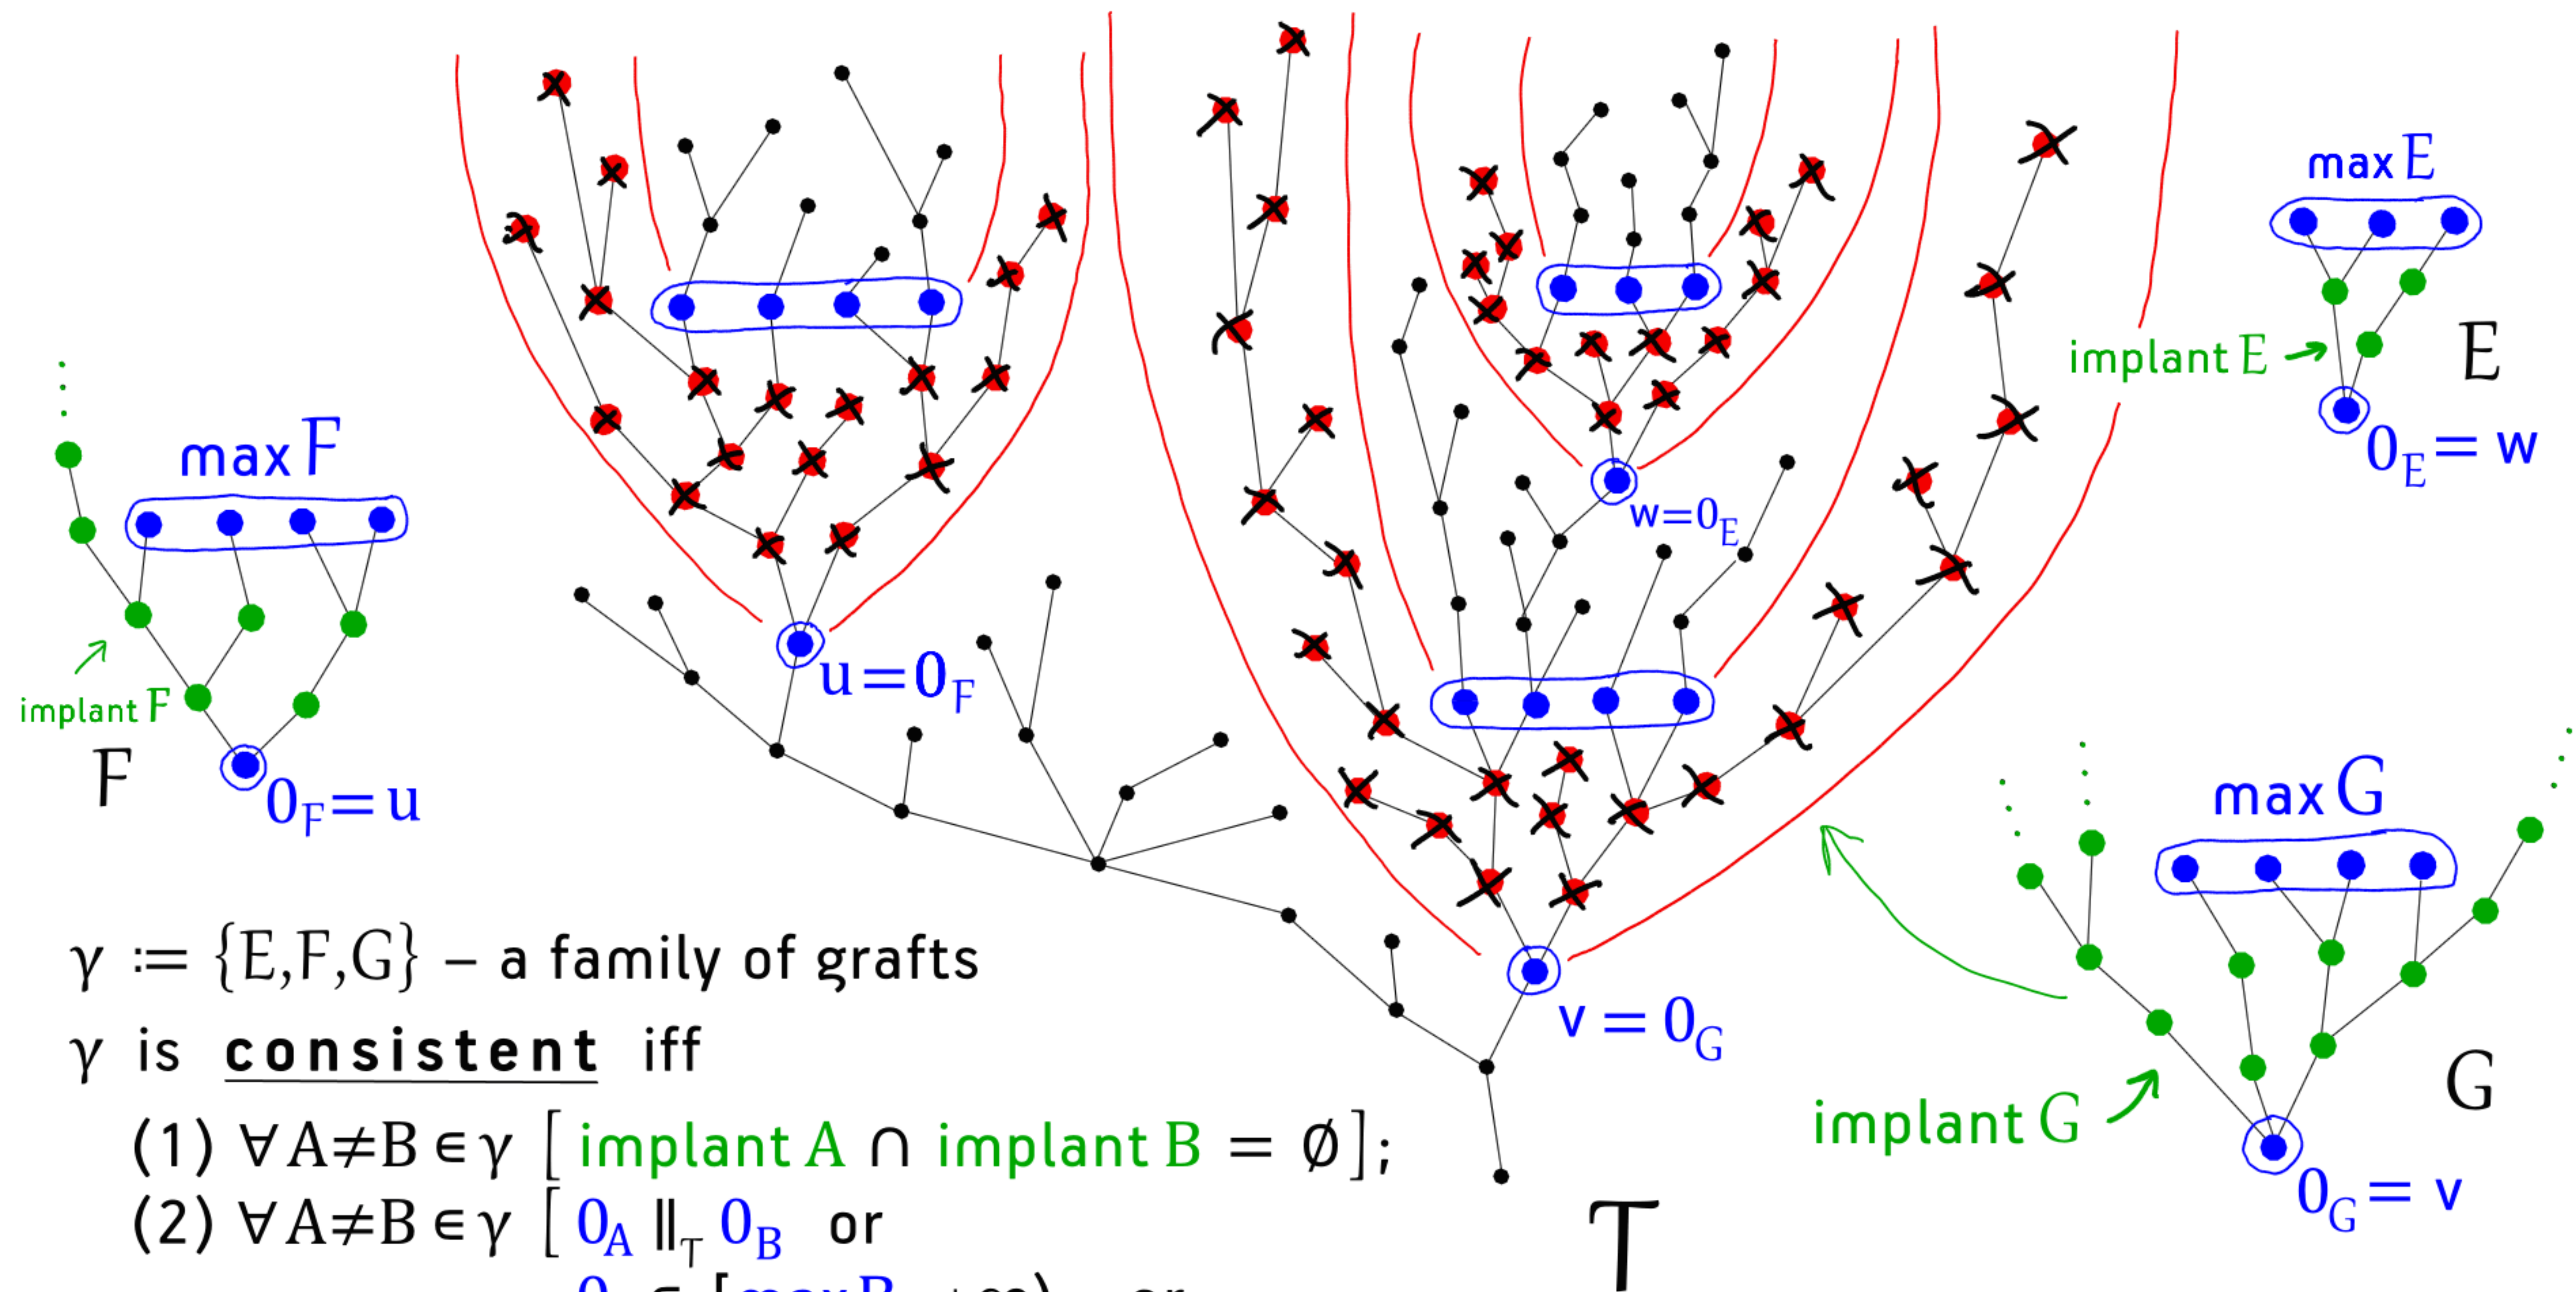



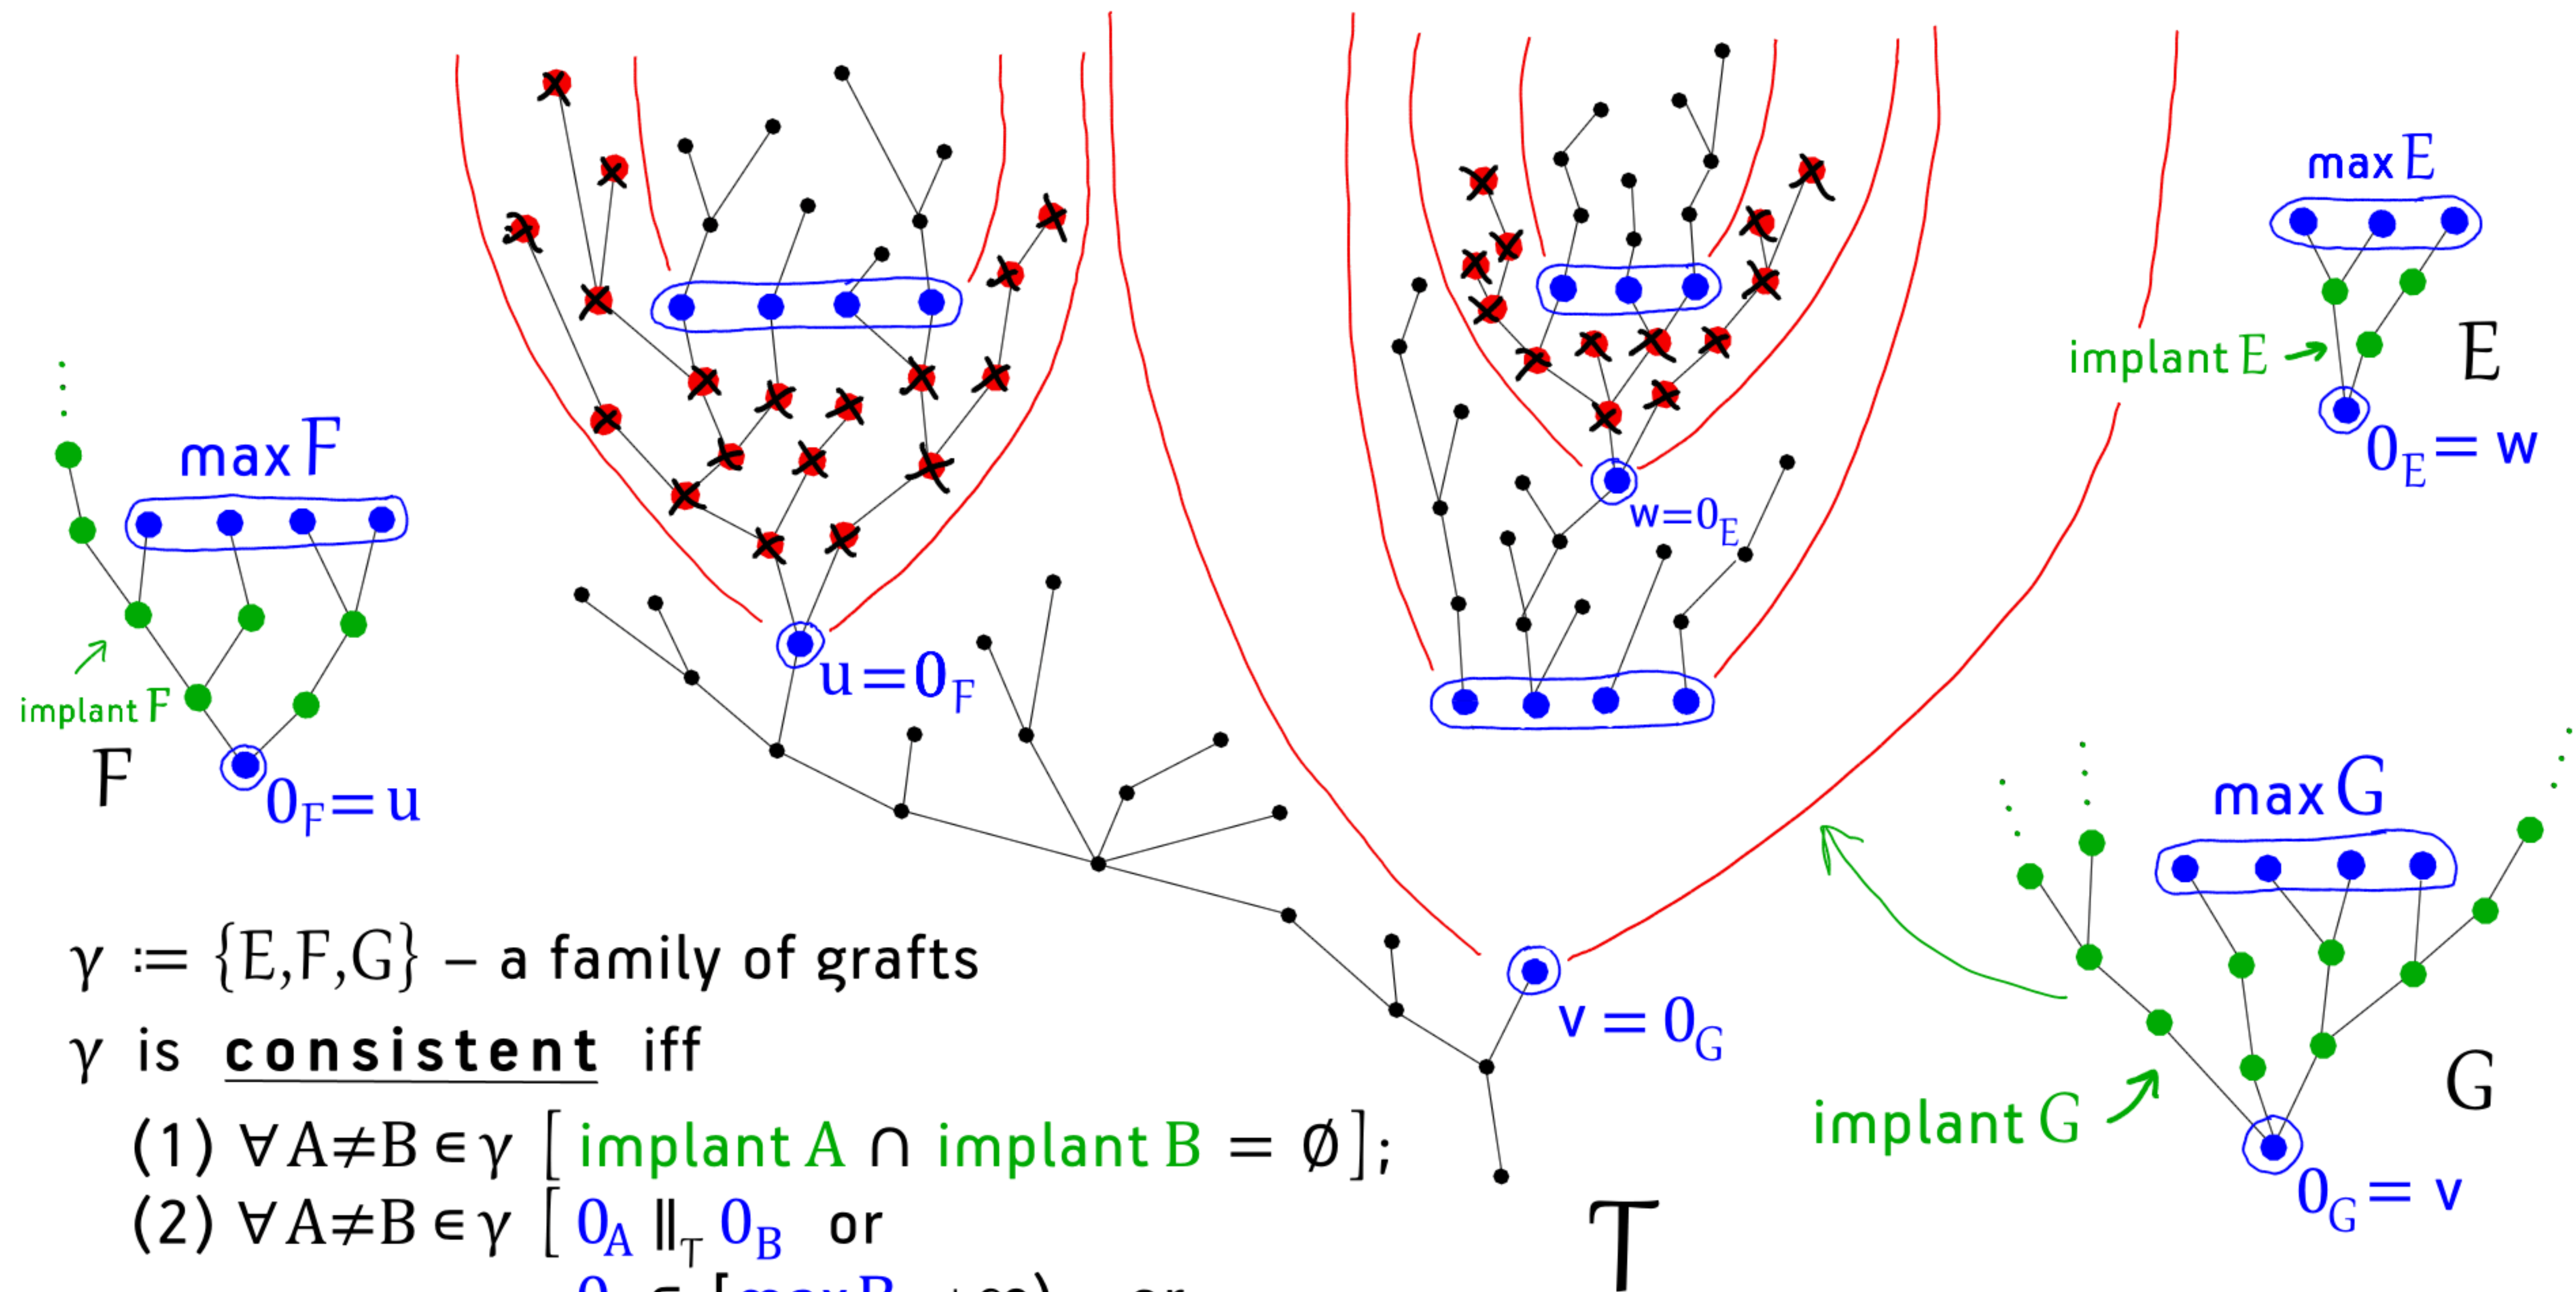

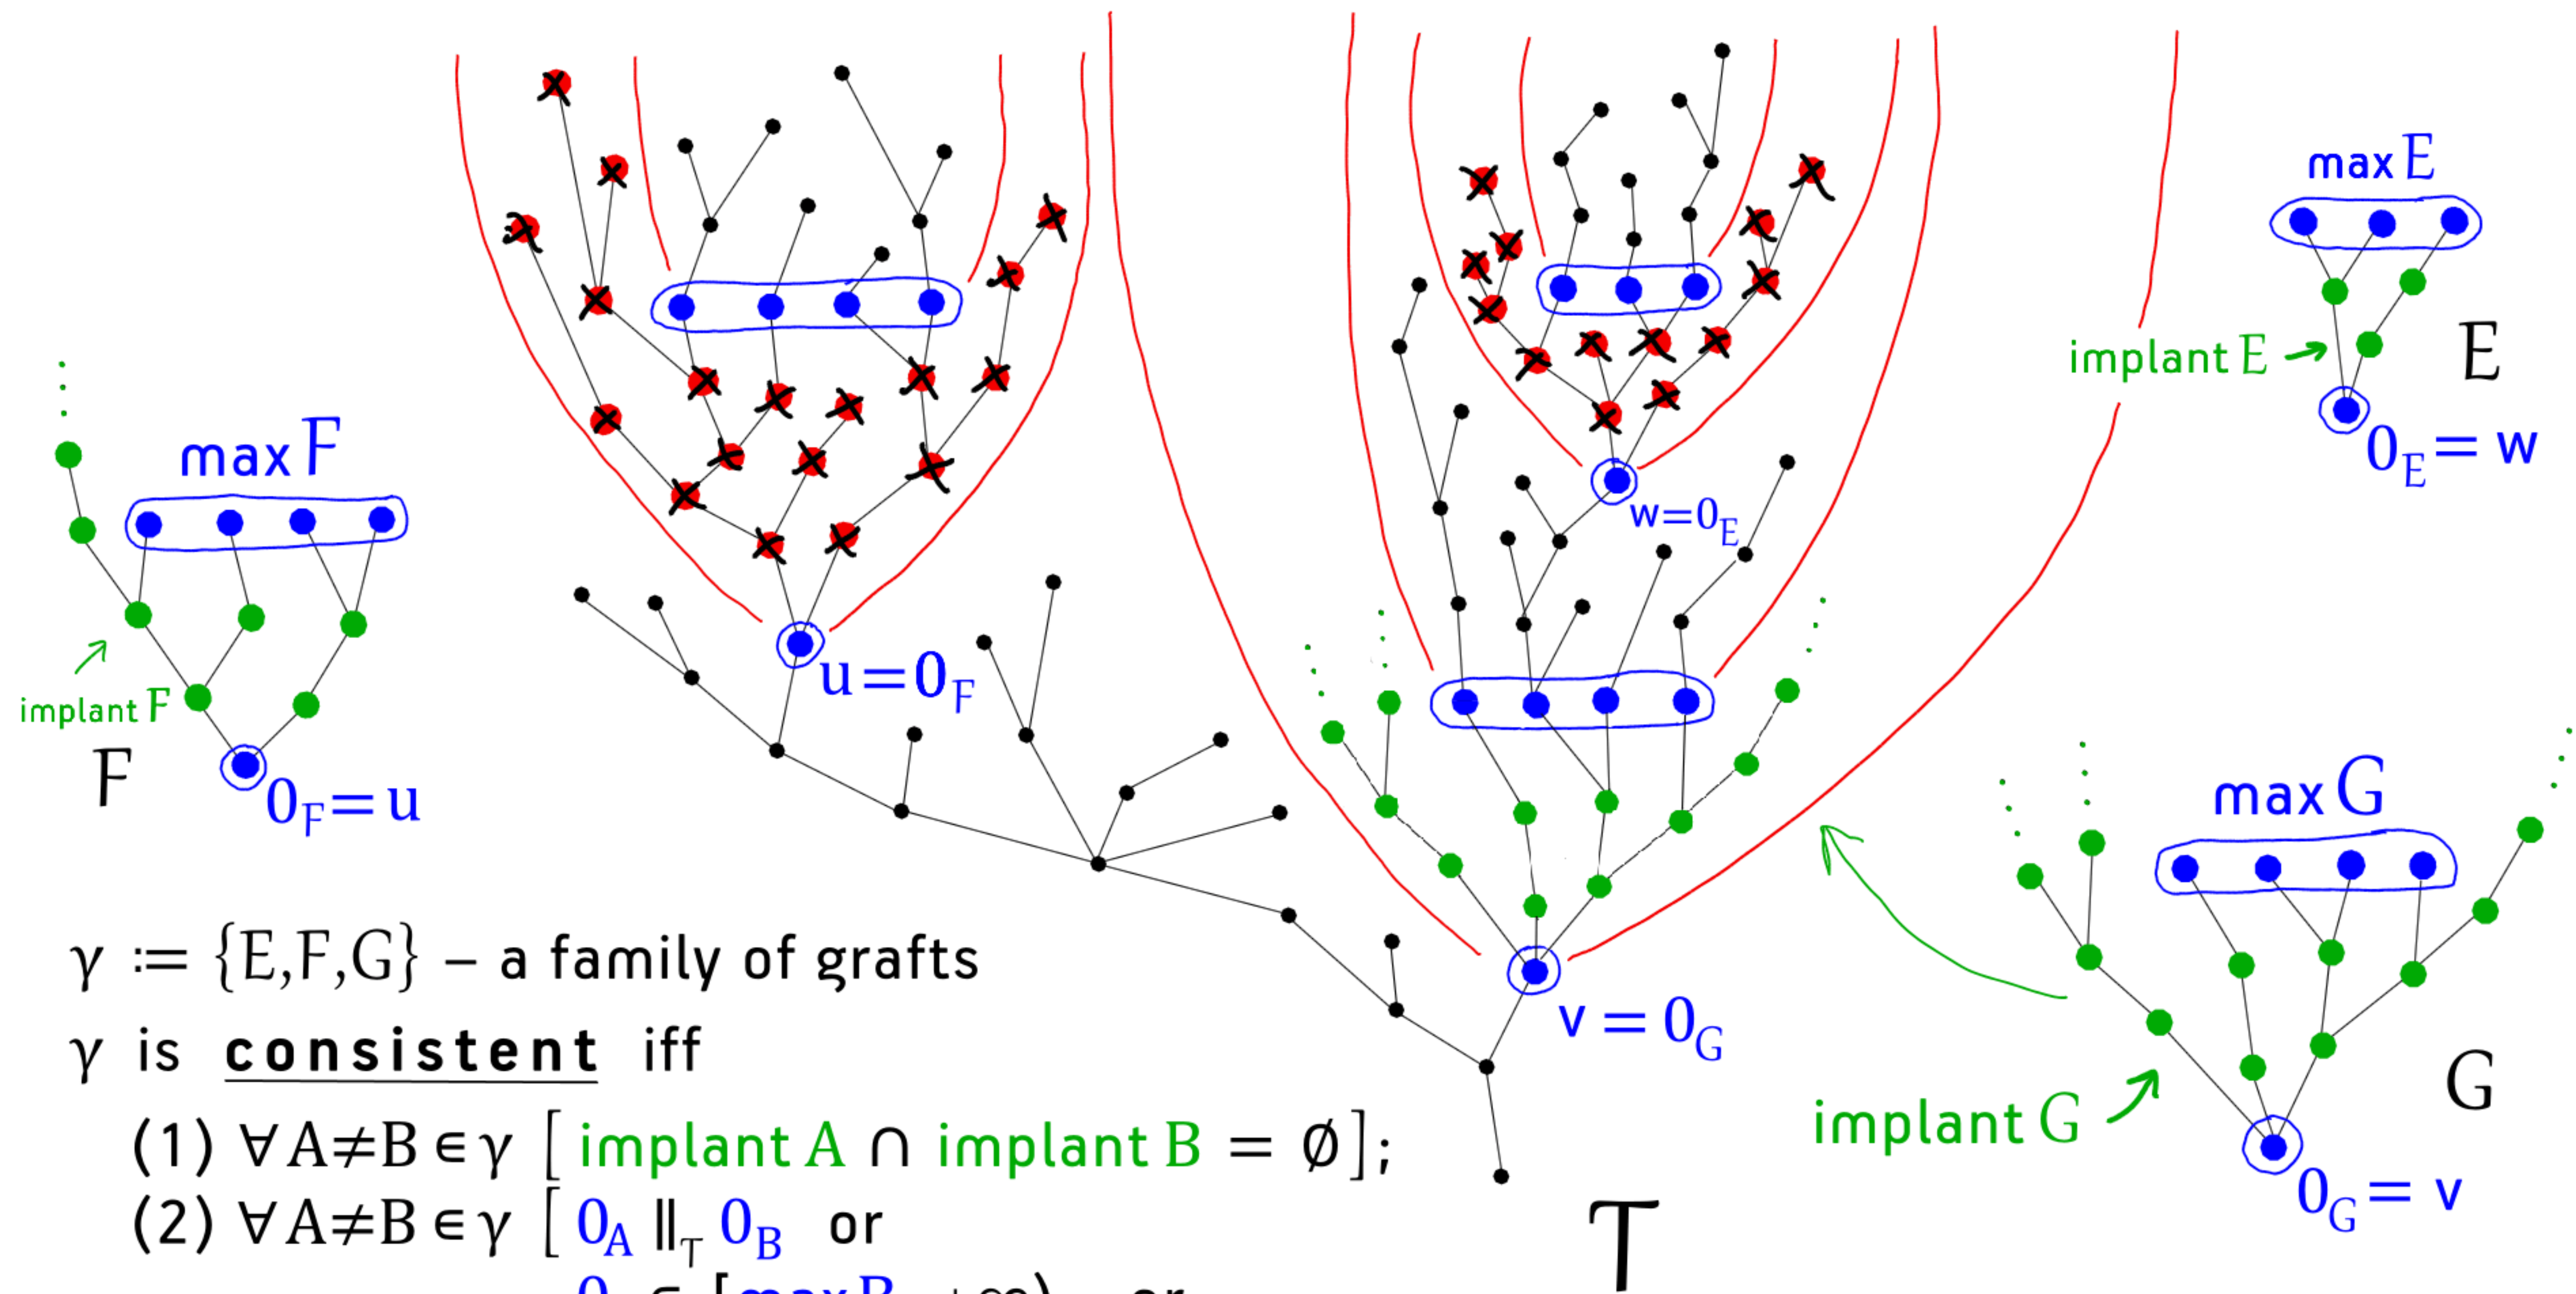



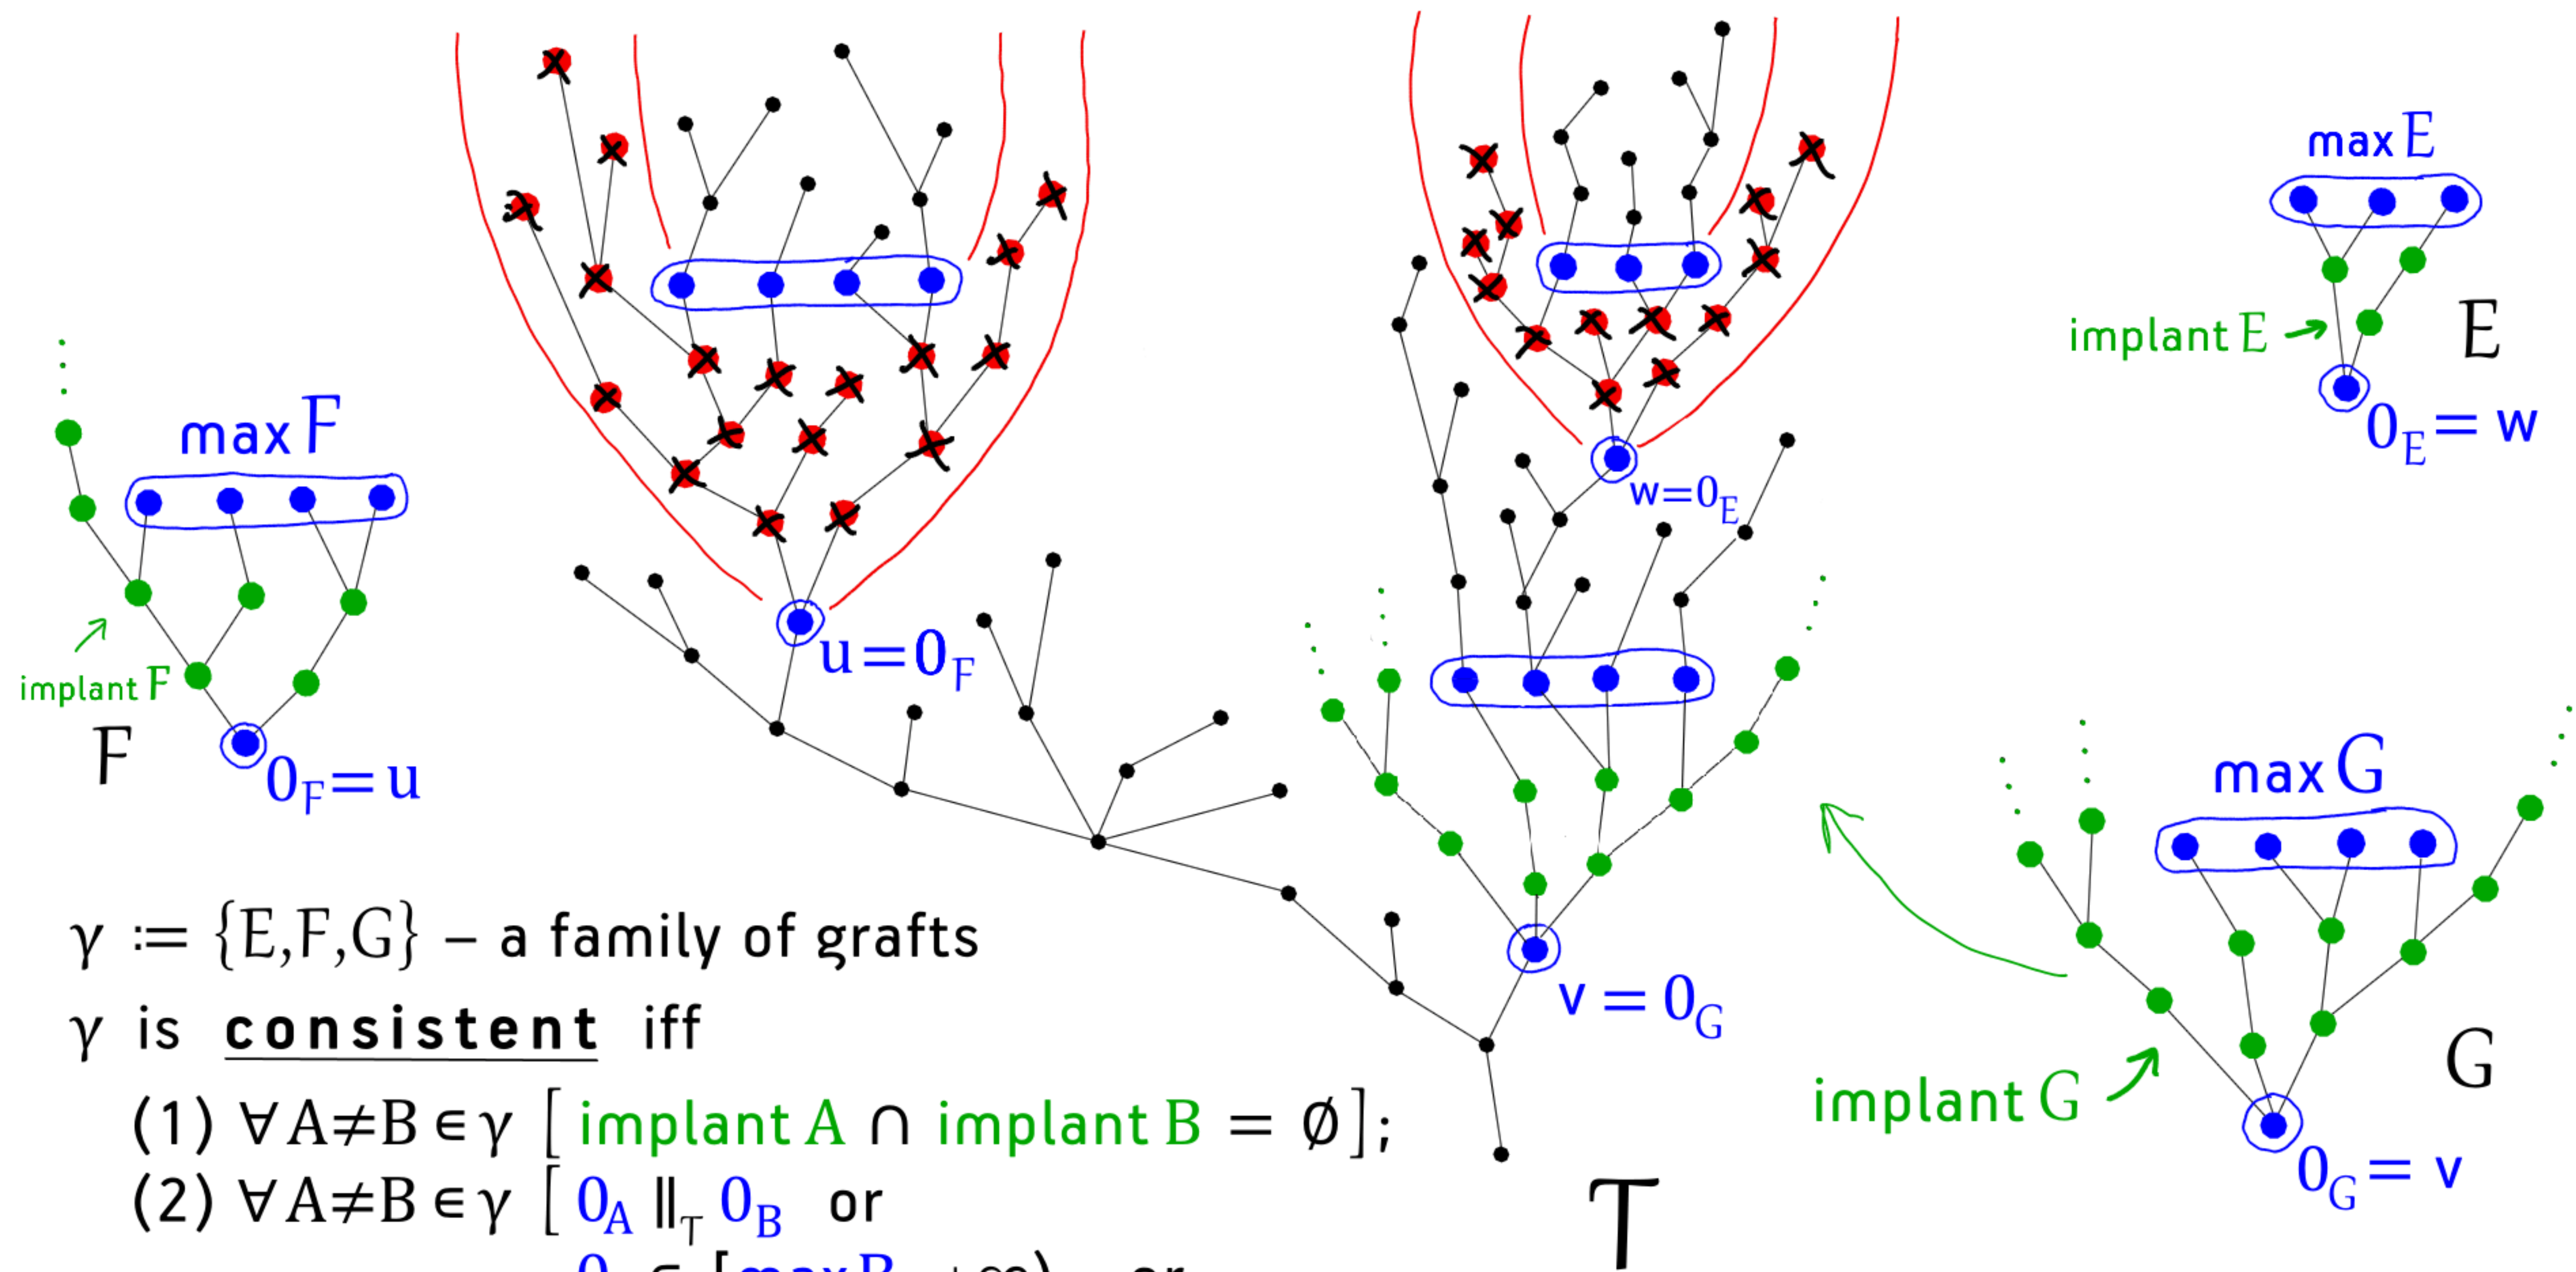

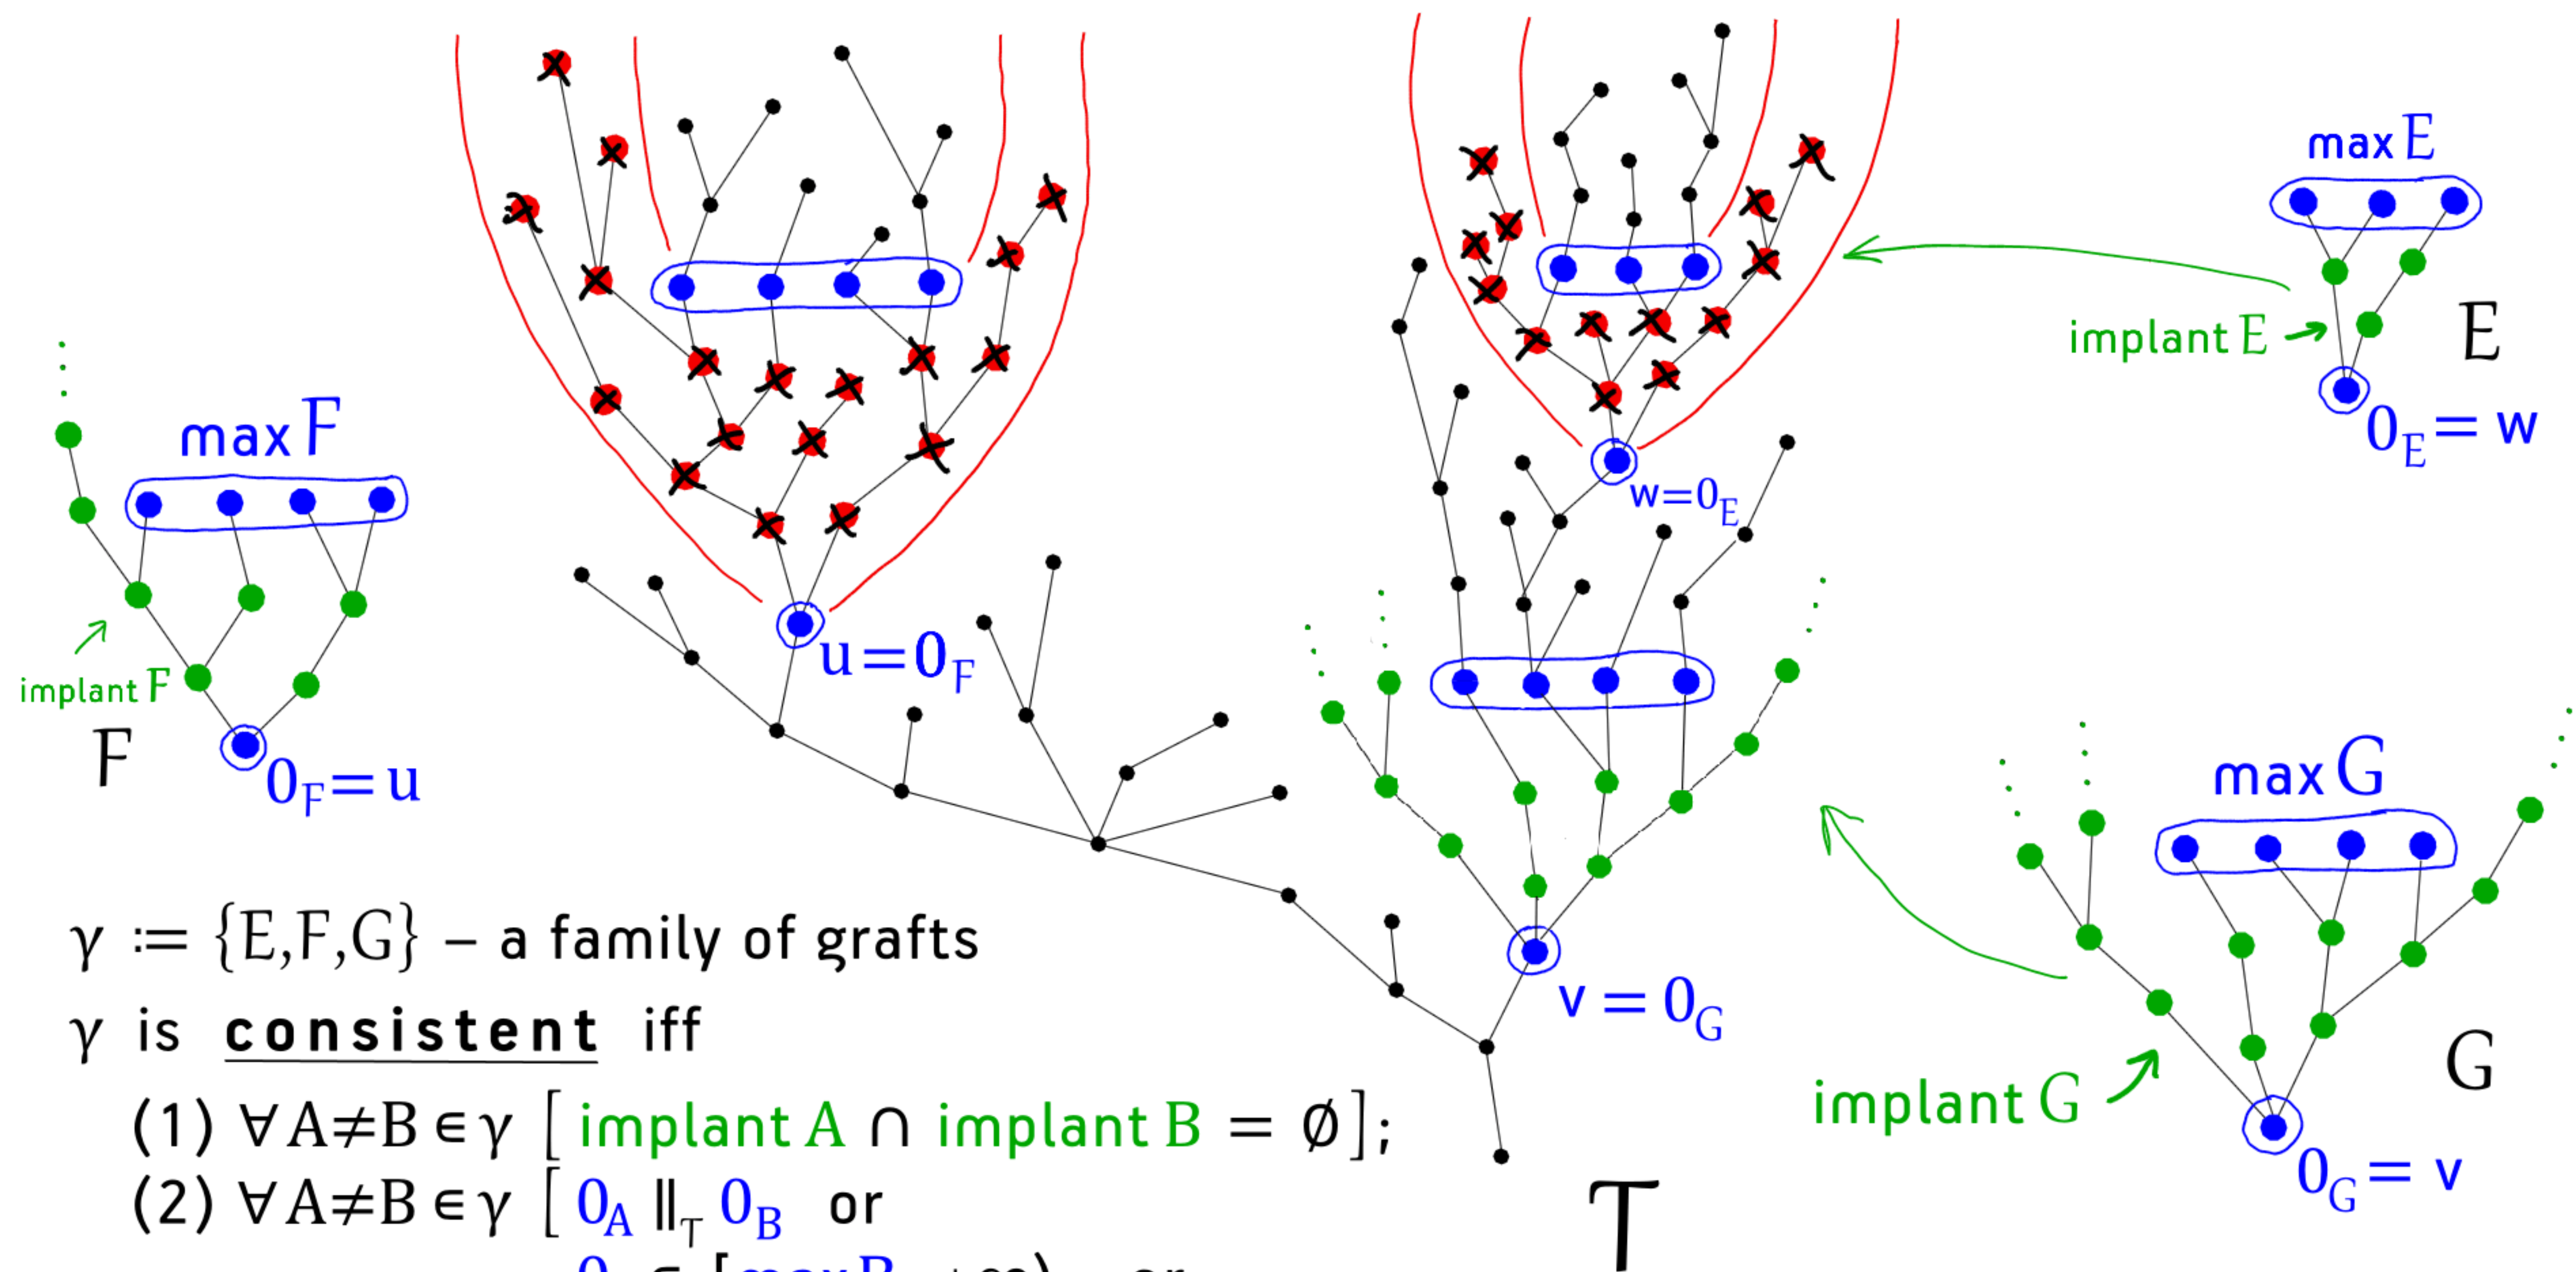

$\gamma := \{E, F, G\}$  – a family of grafts

$\gamma$  is **consistent** iff

(1)  $\forall A \neq B \in \gamma$  [  $\text{implant } A \cap \text{implant } B = \emptyset$  ];

(2)  $\forall A \neq B \in \gamma$  [  $0_A \parallel_T 0_B$  or  
 $0_A \in [\max B, +\infty)_T$  or  
 $0_B \in [\max A, +\infty)_T$  ].



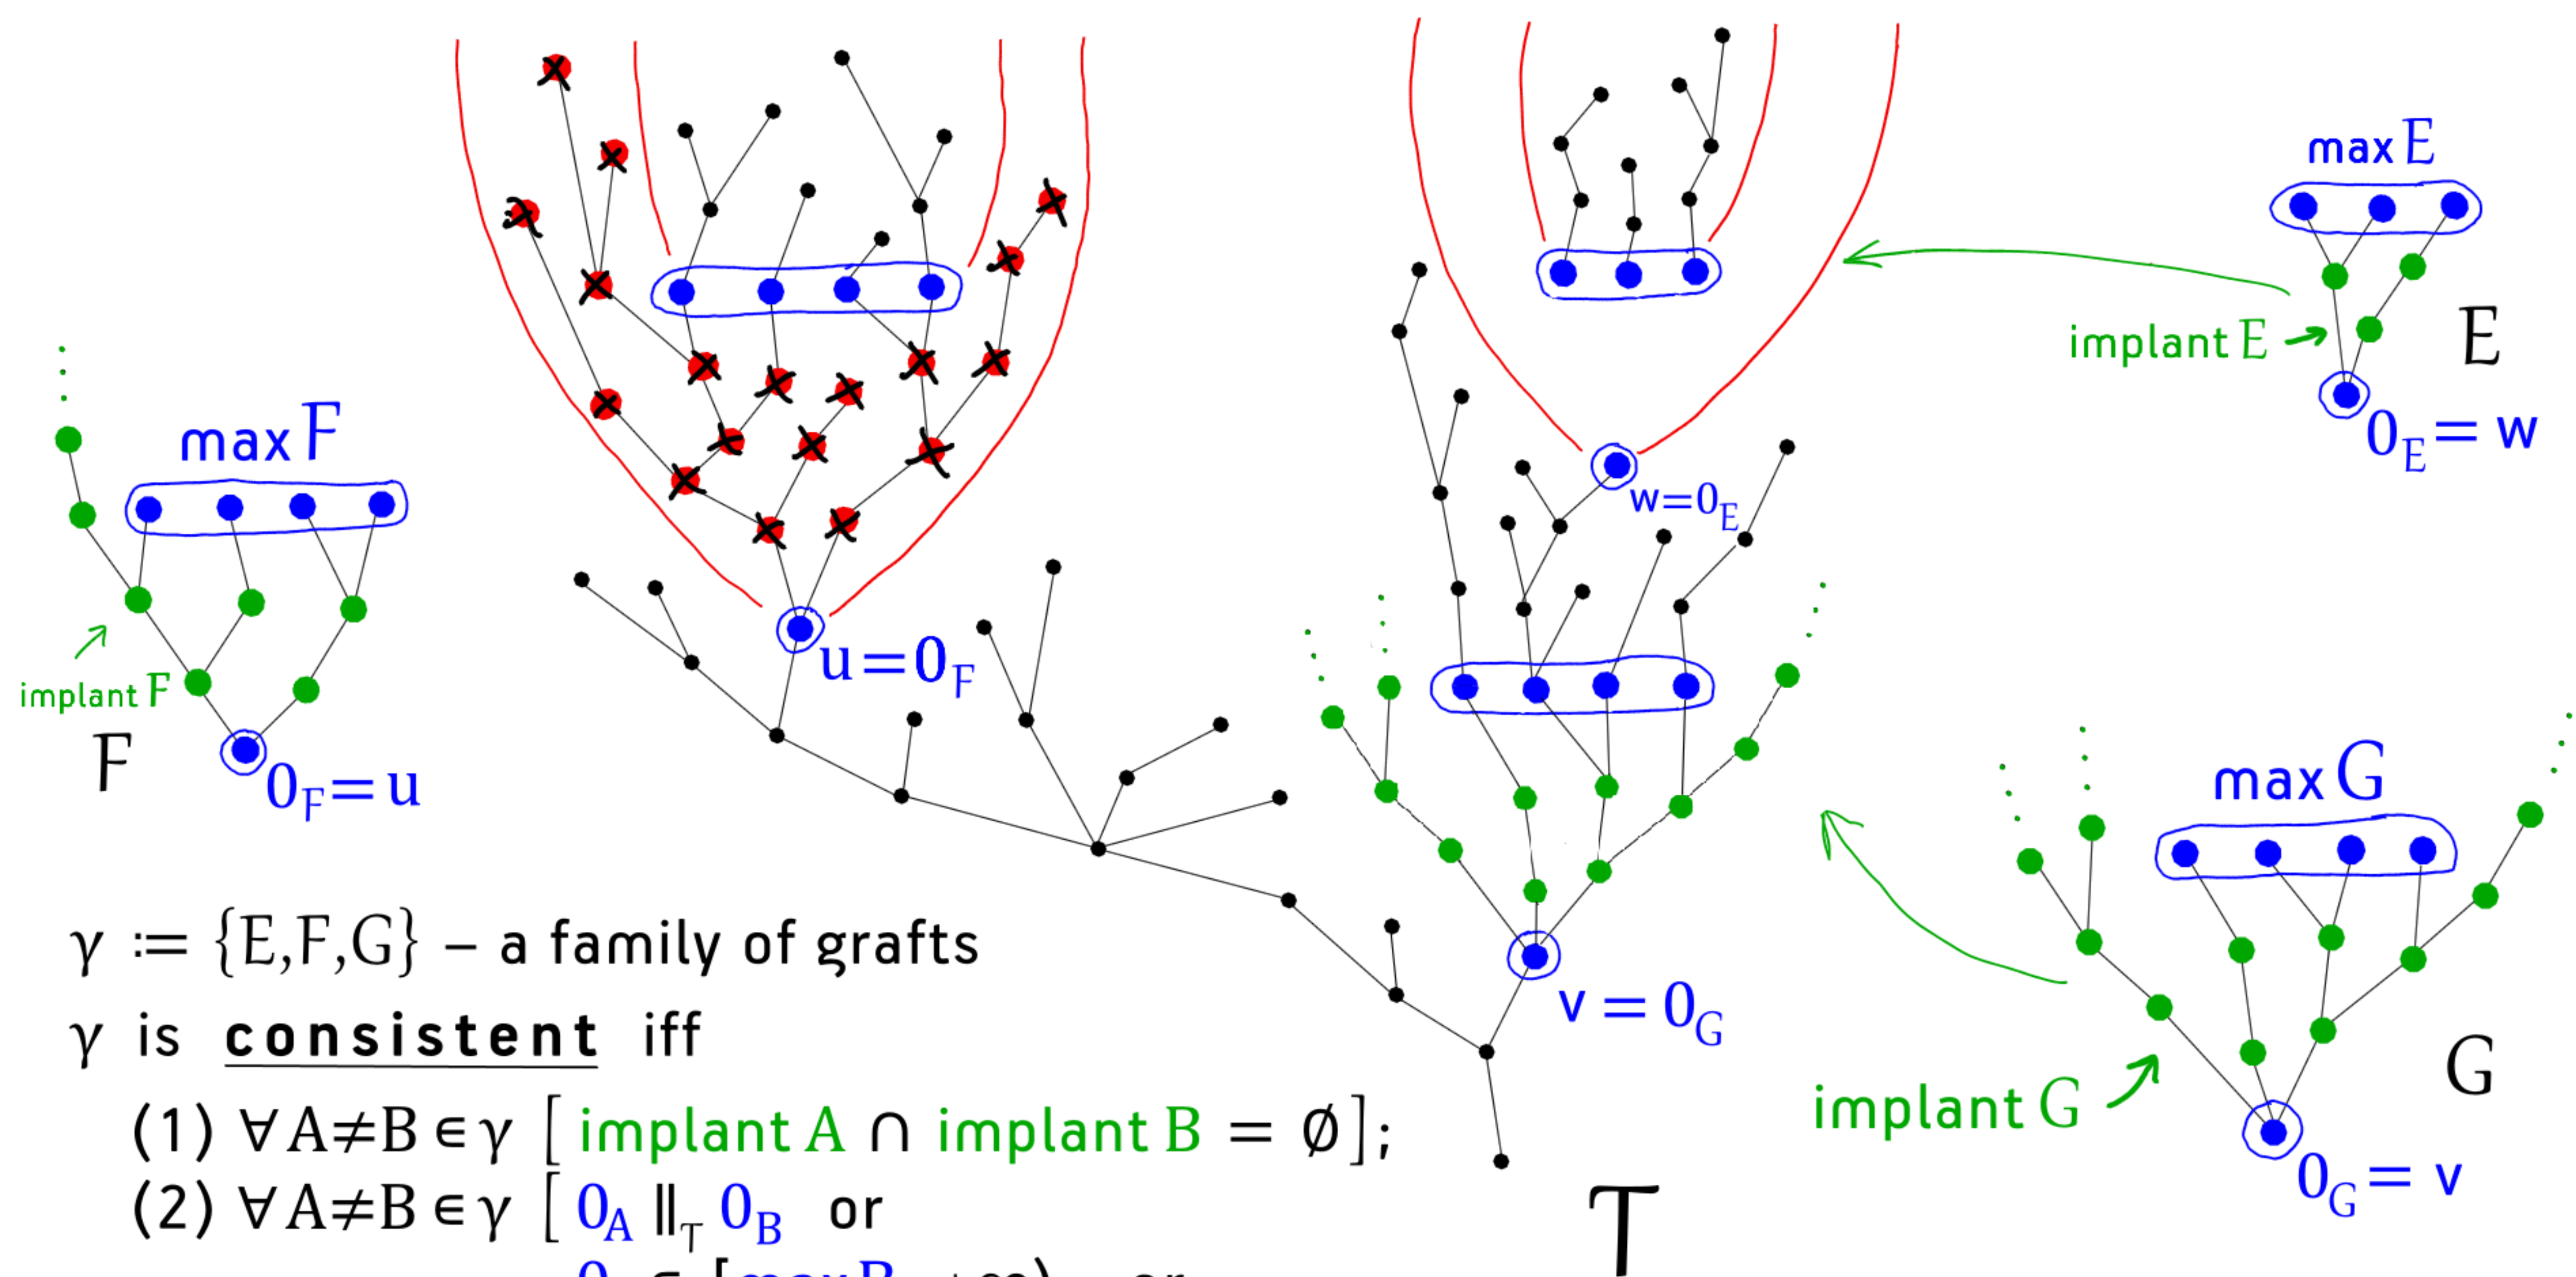

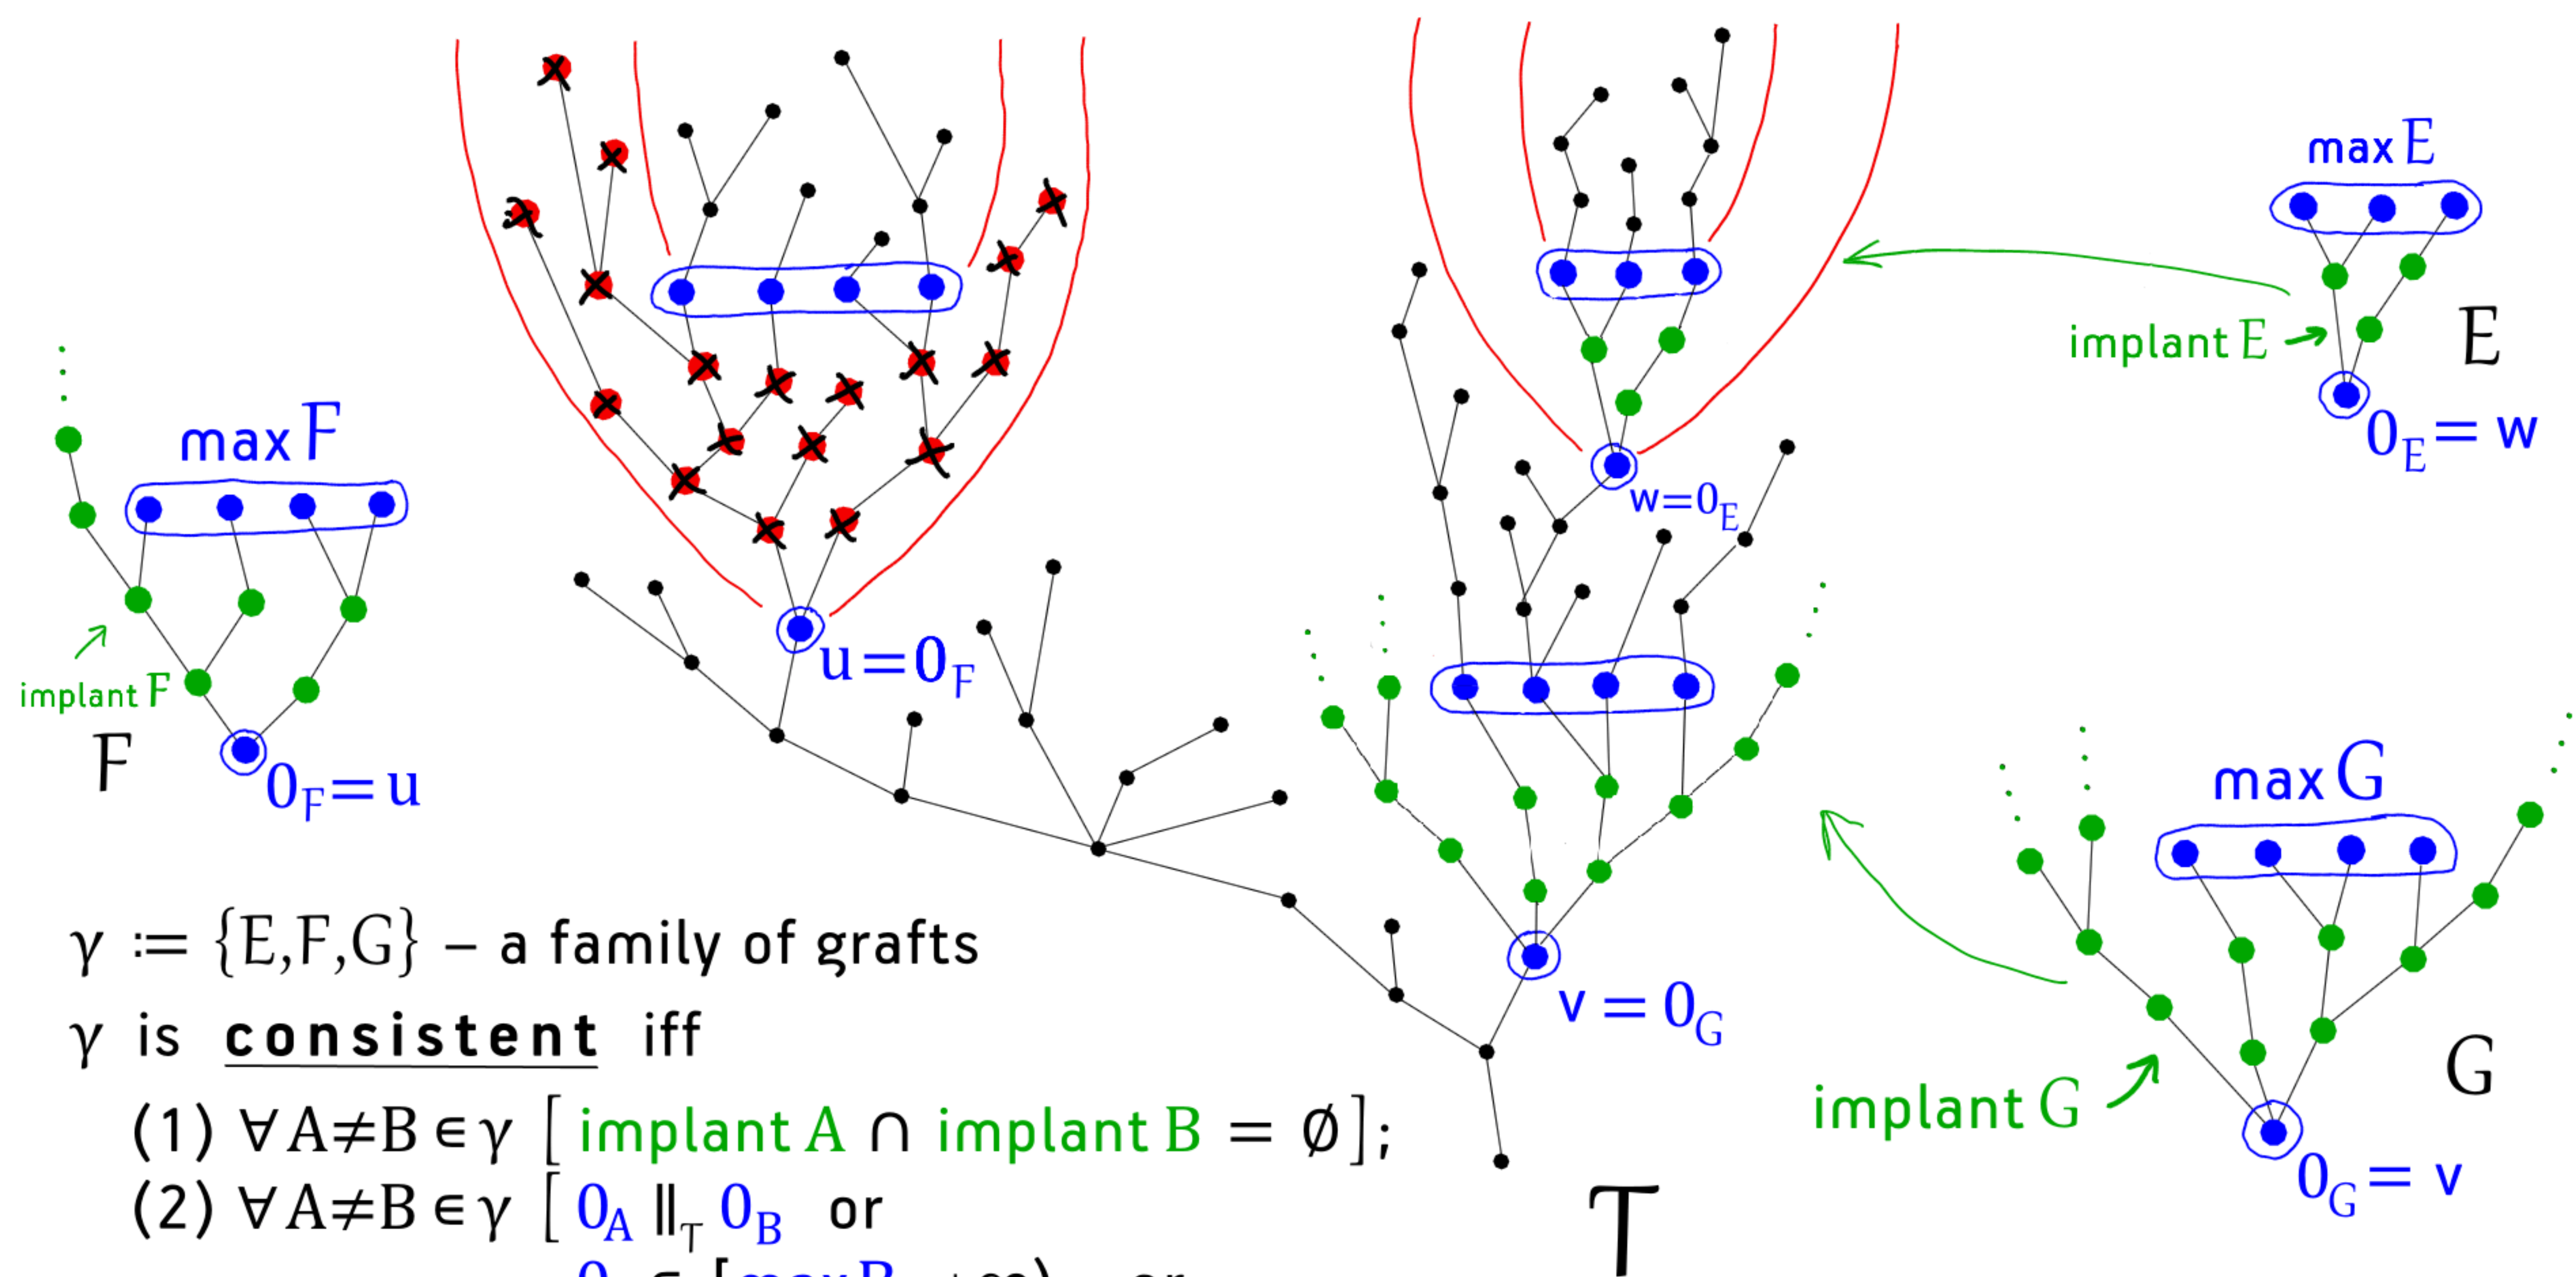



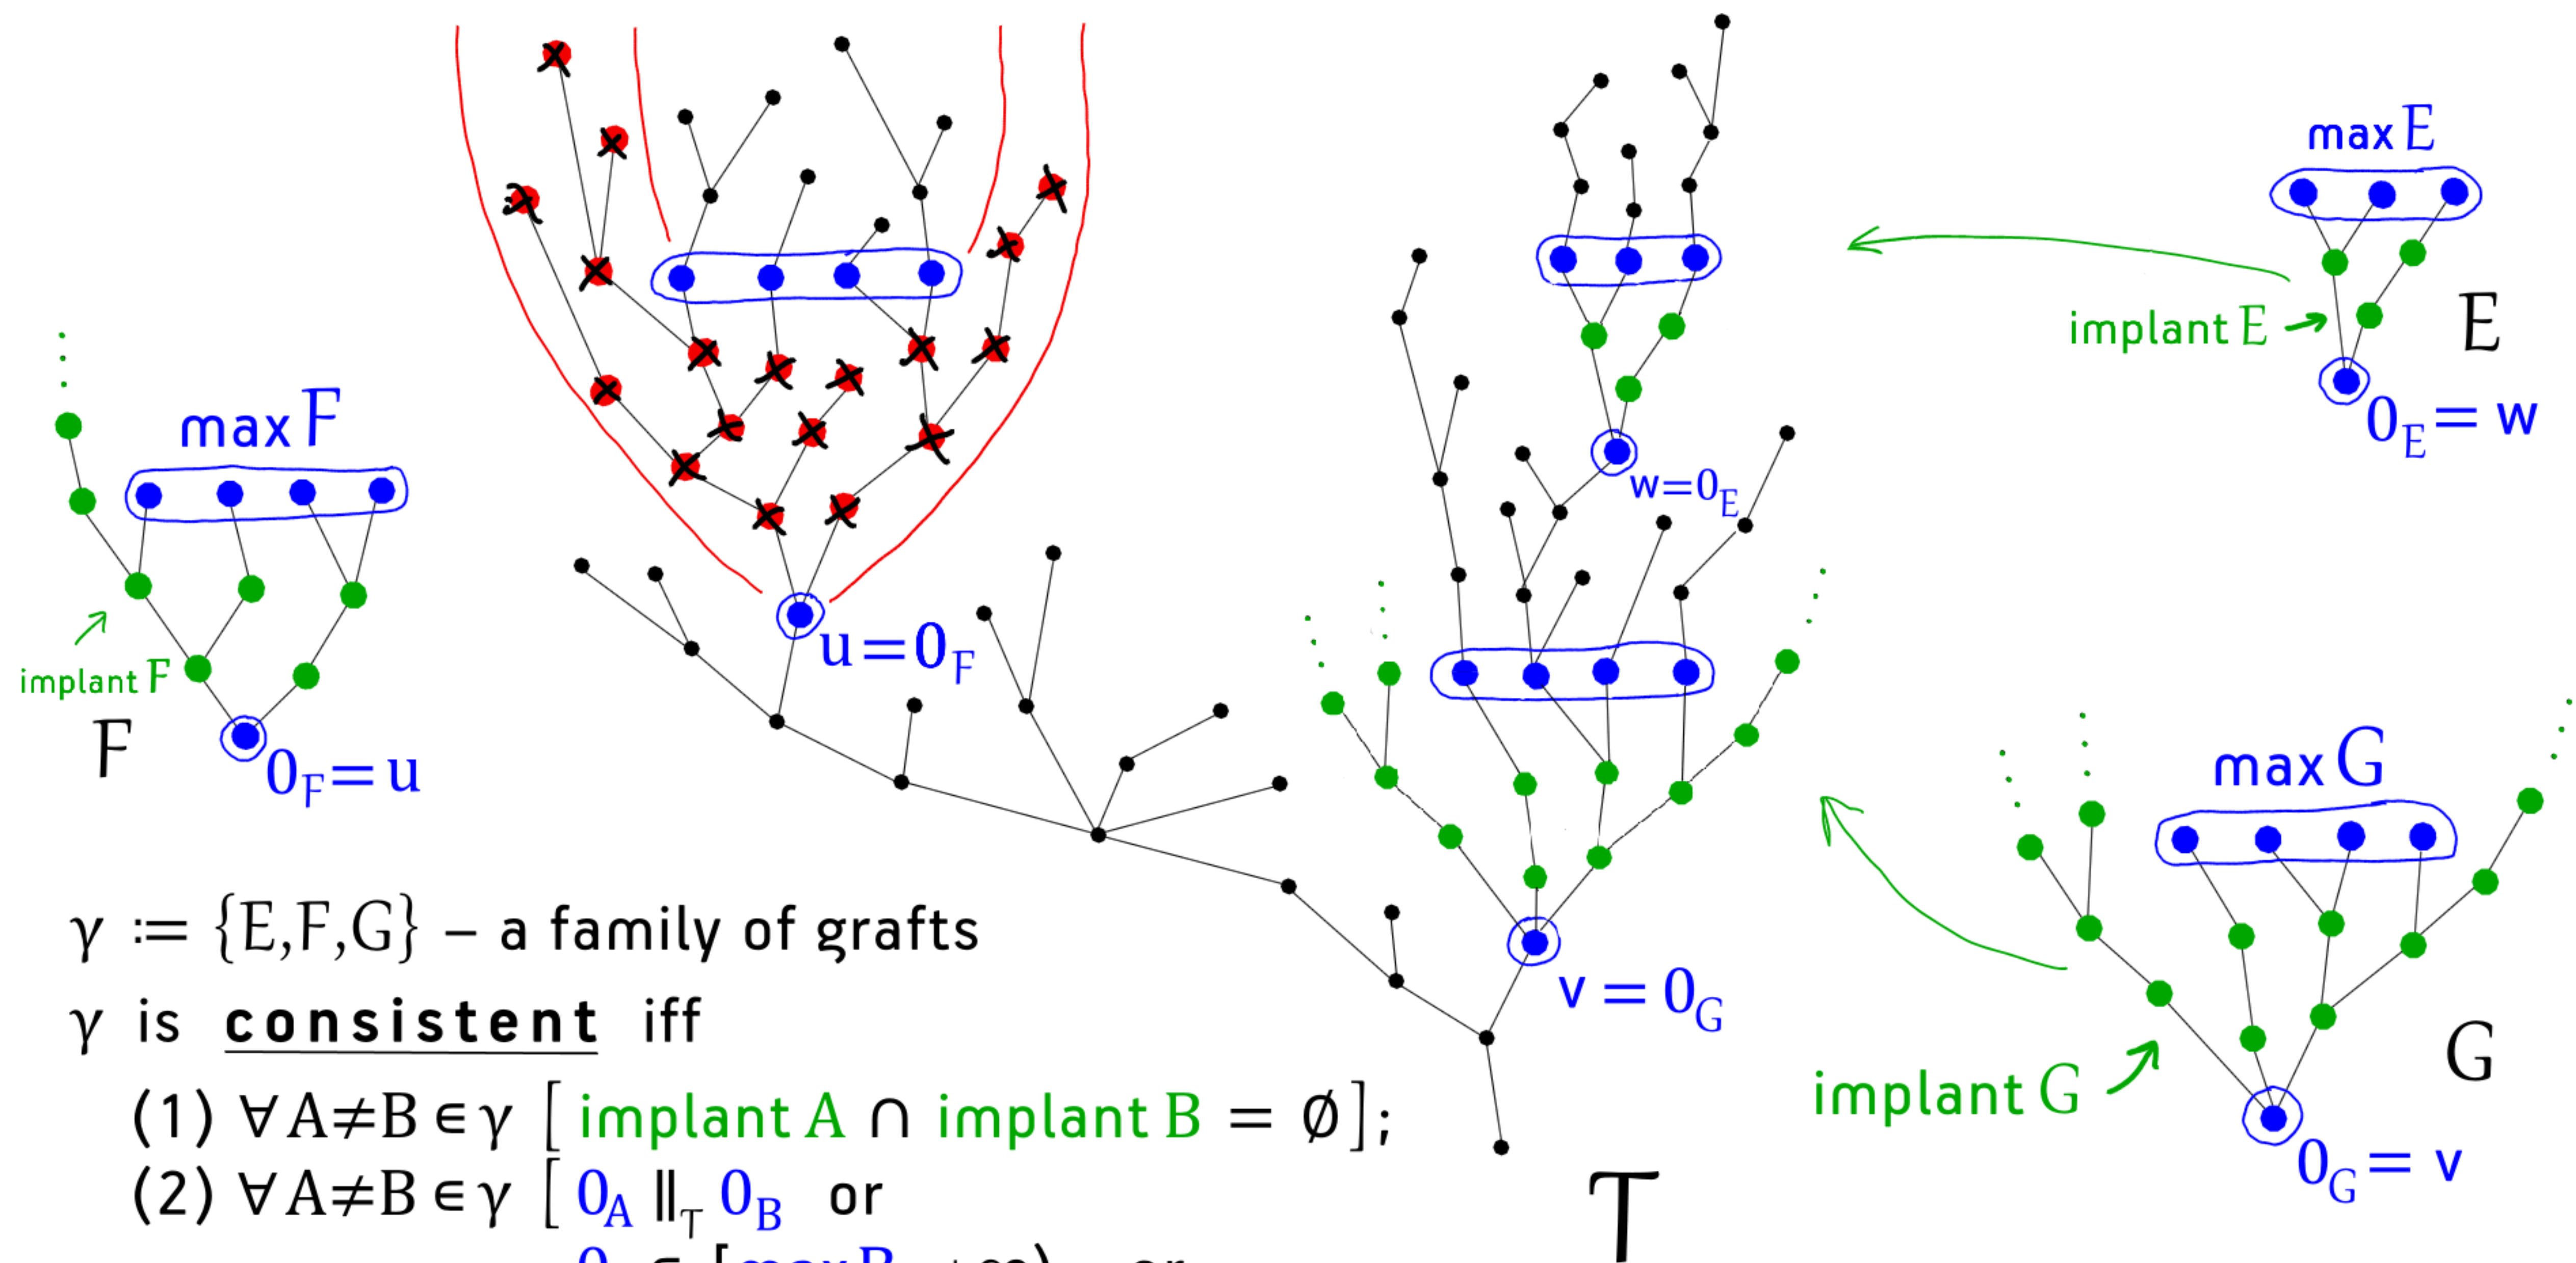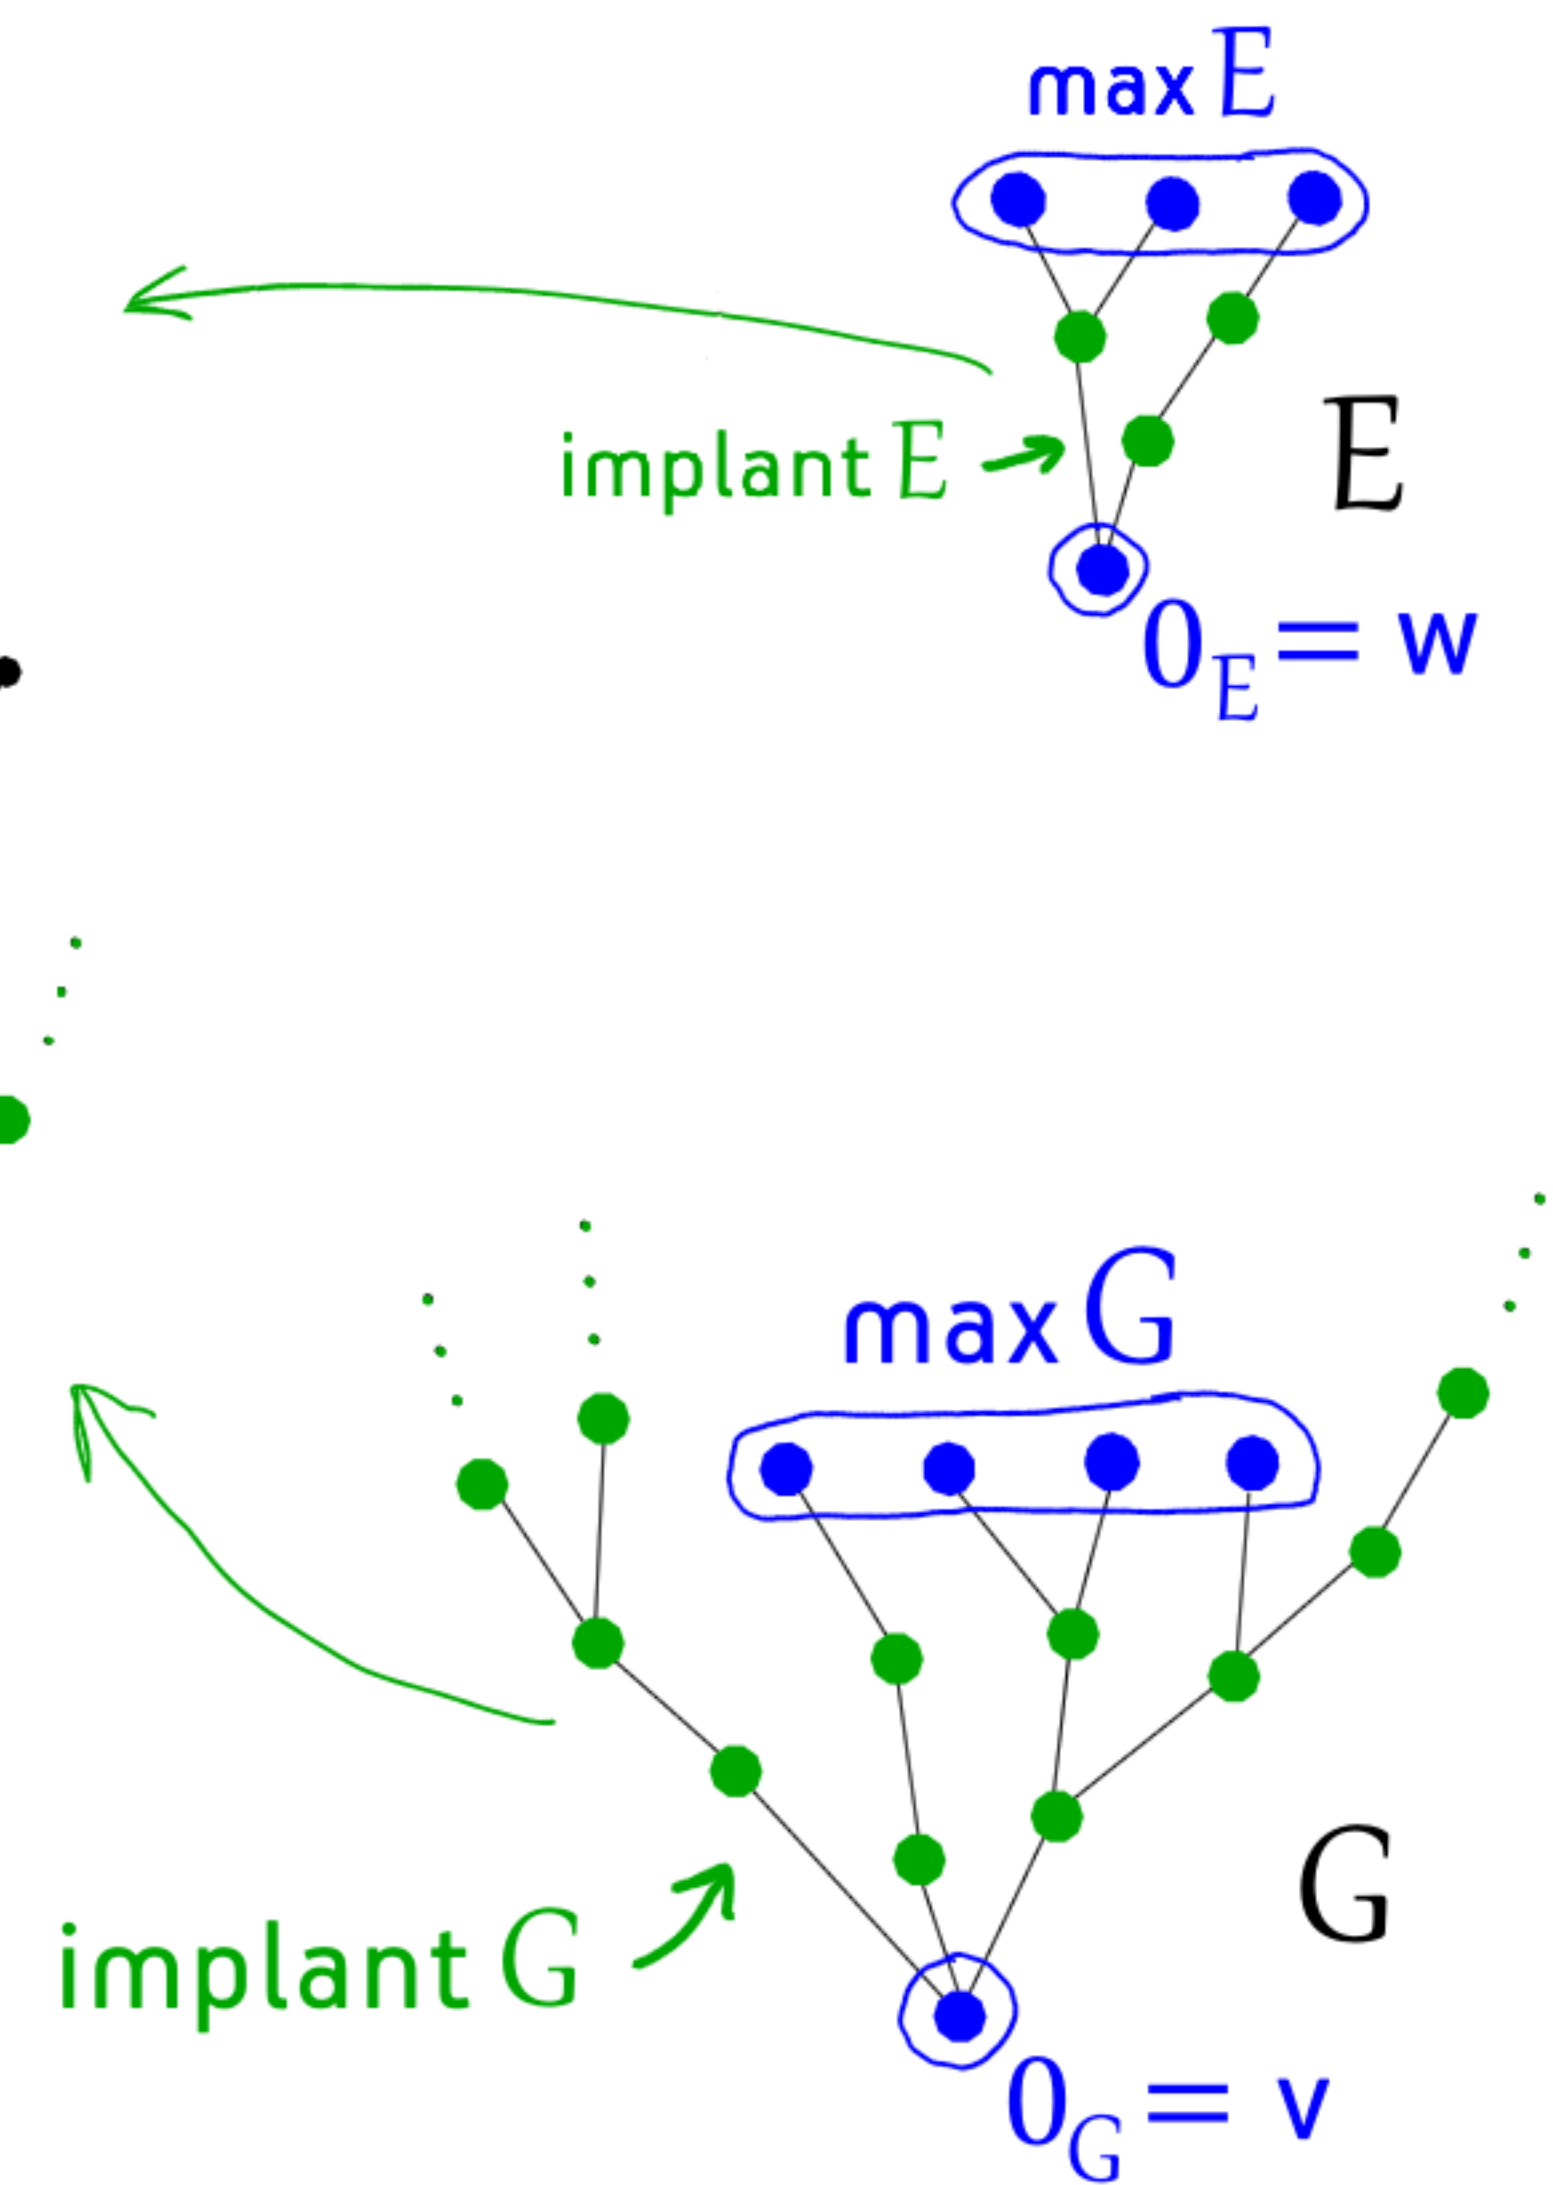

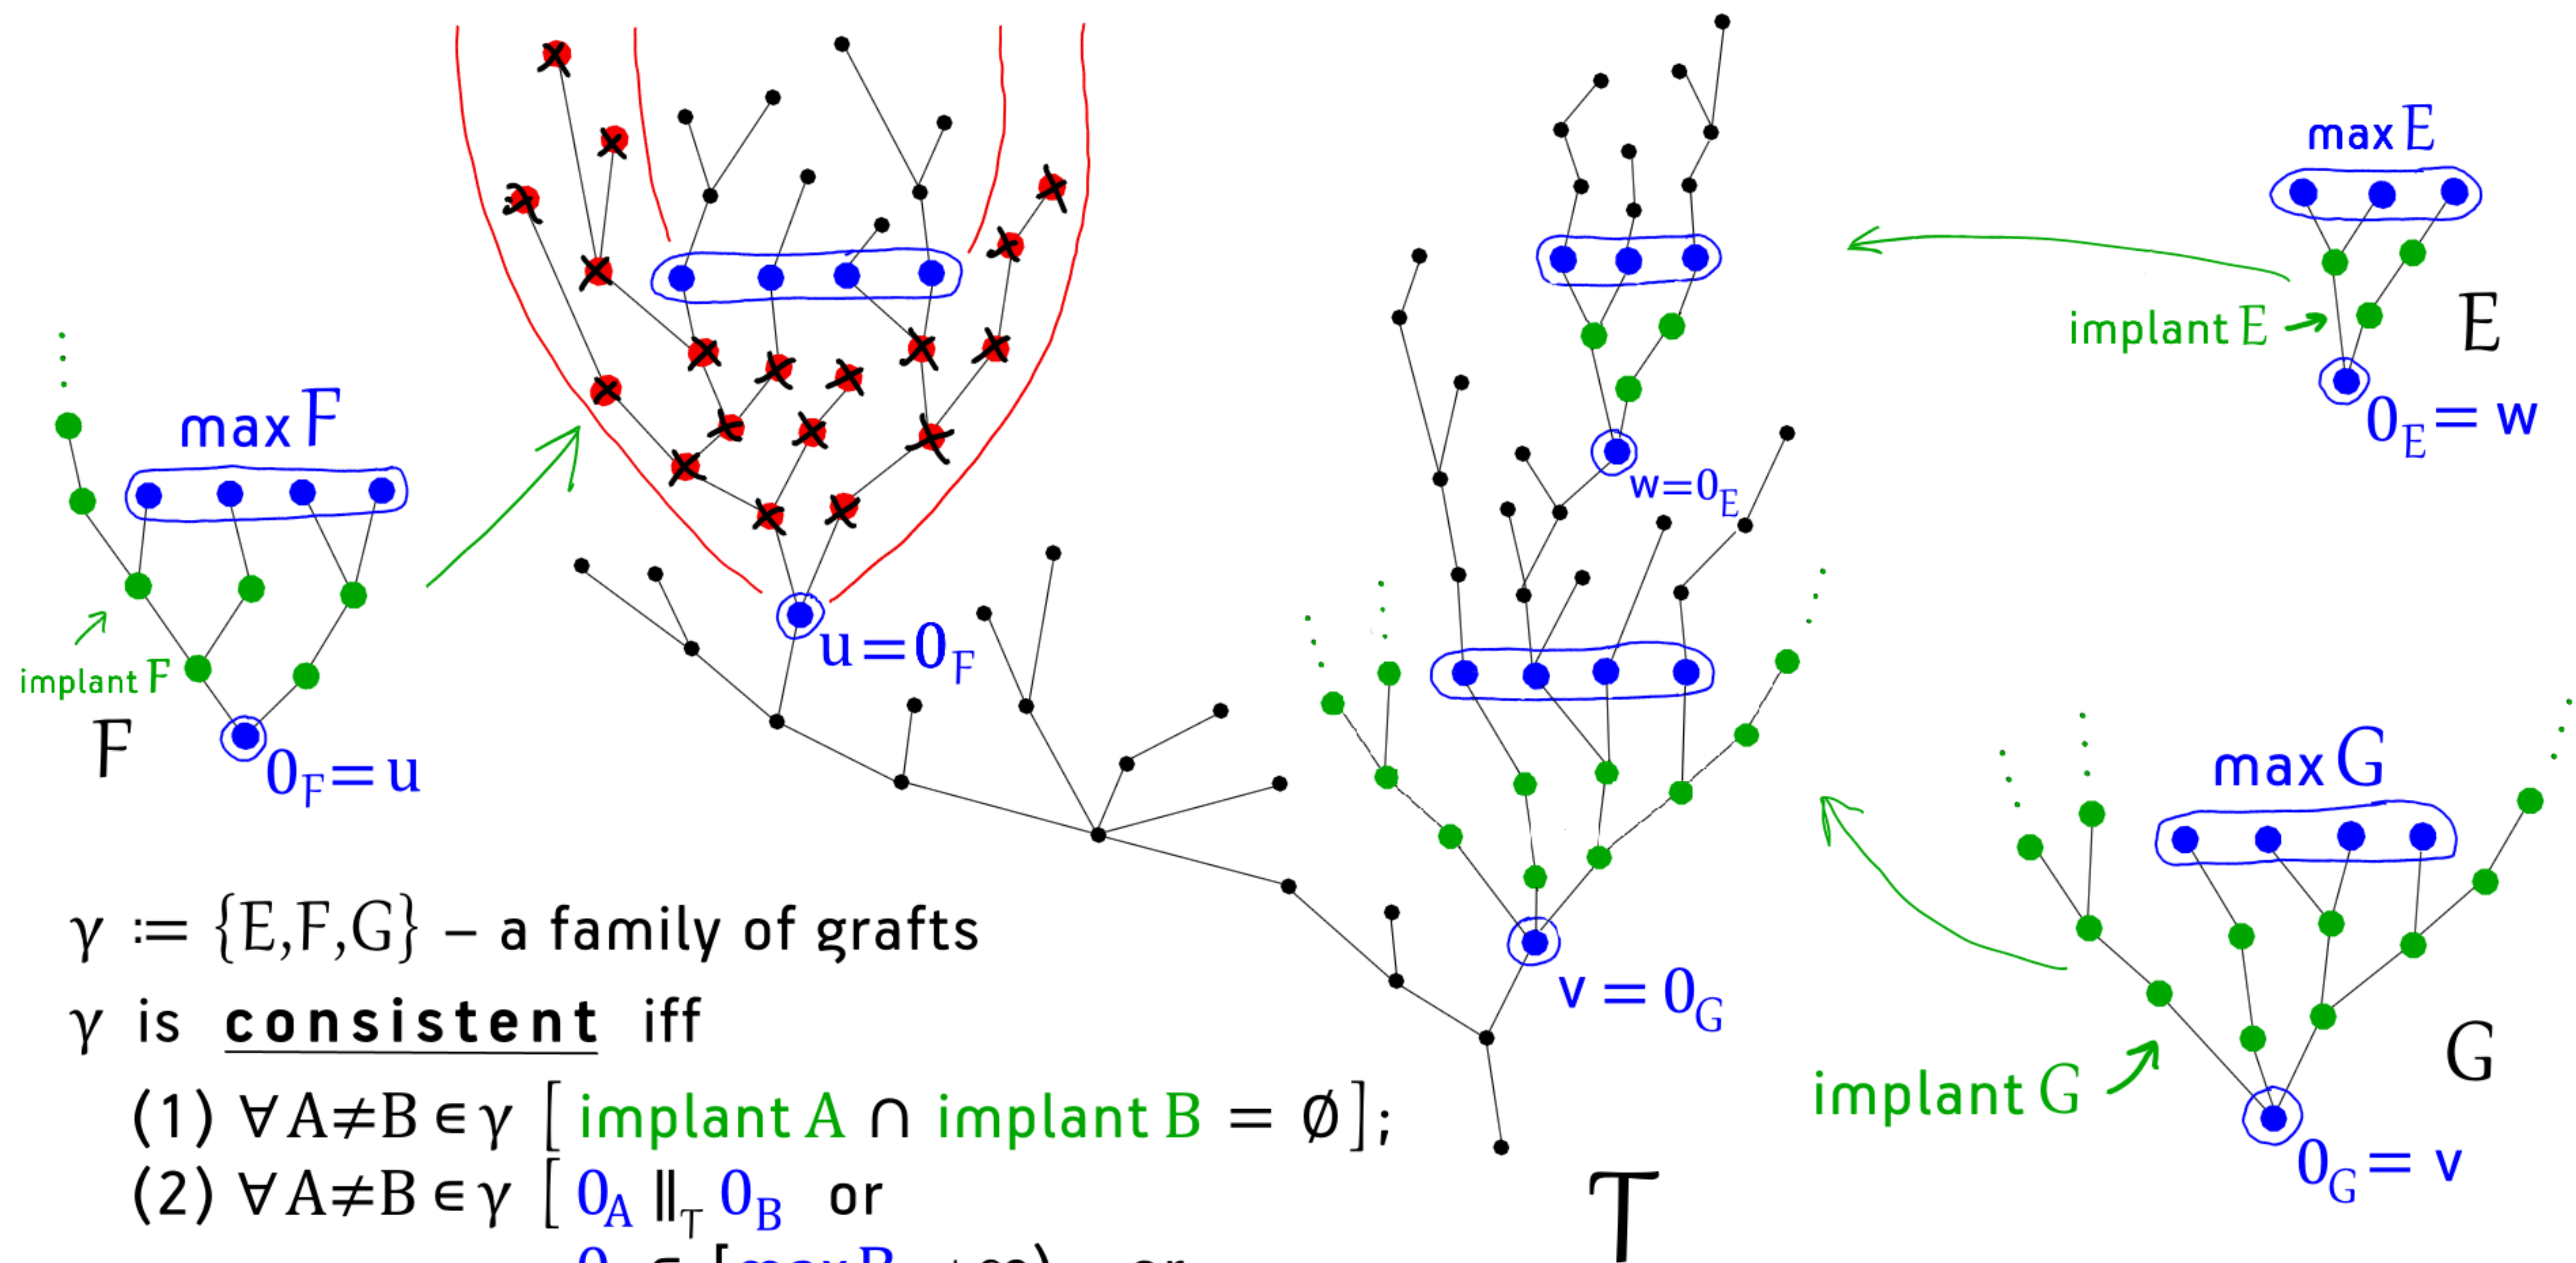



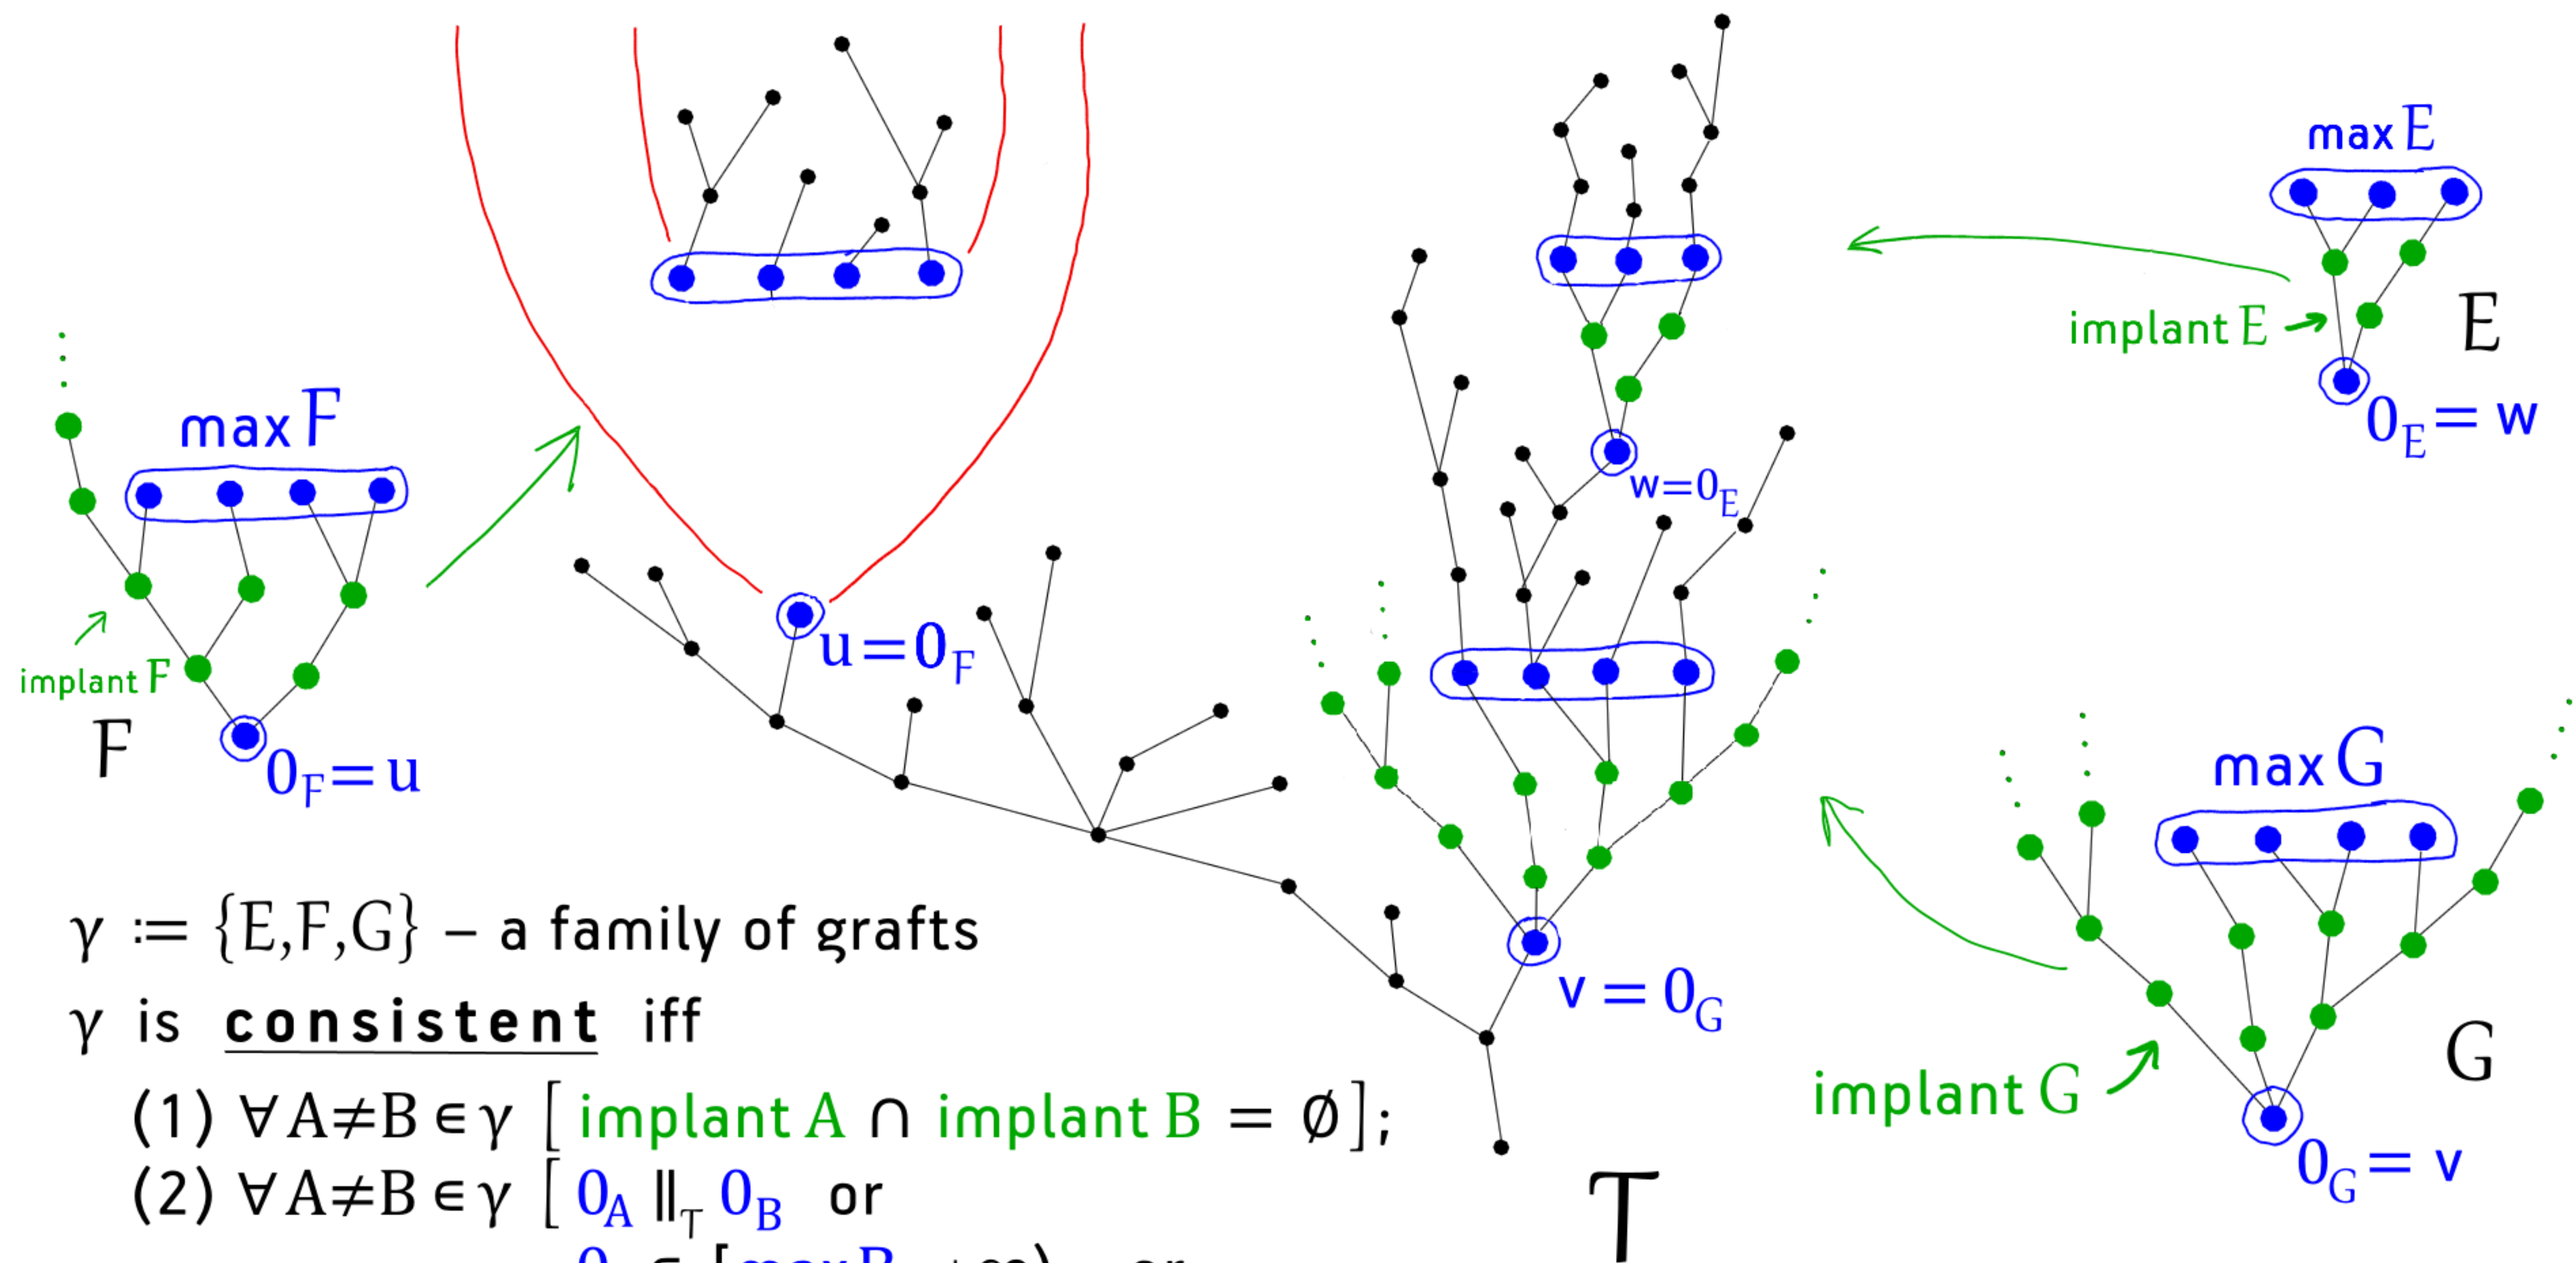

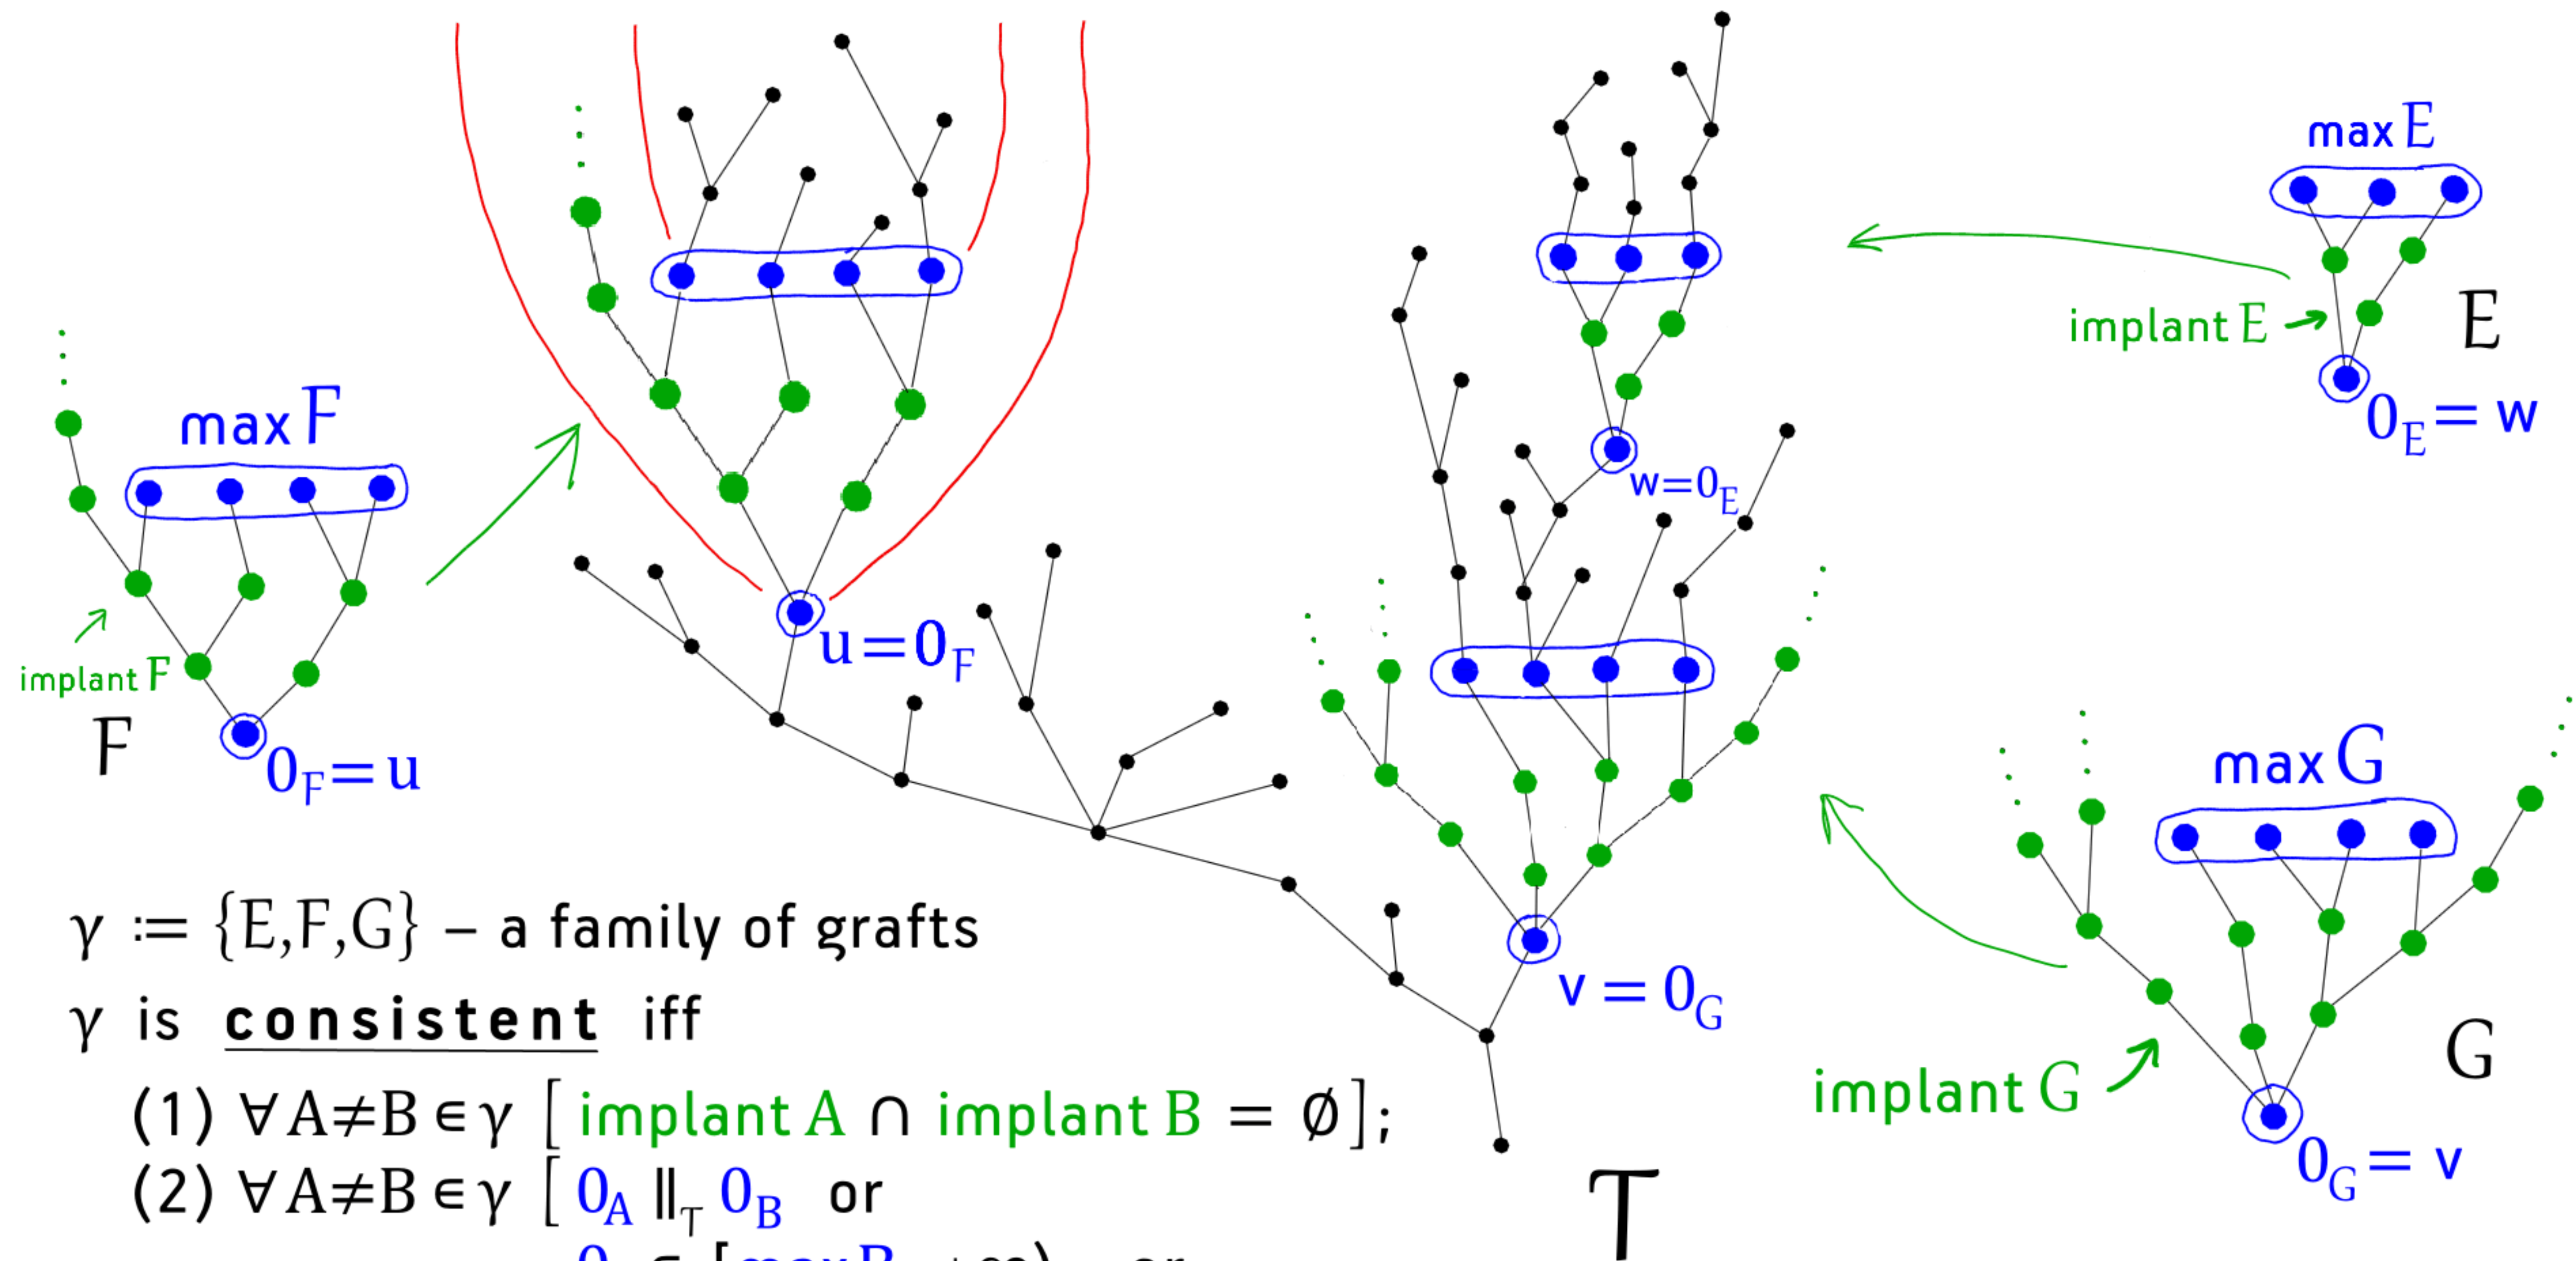



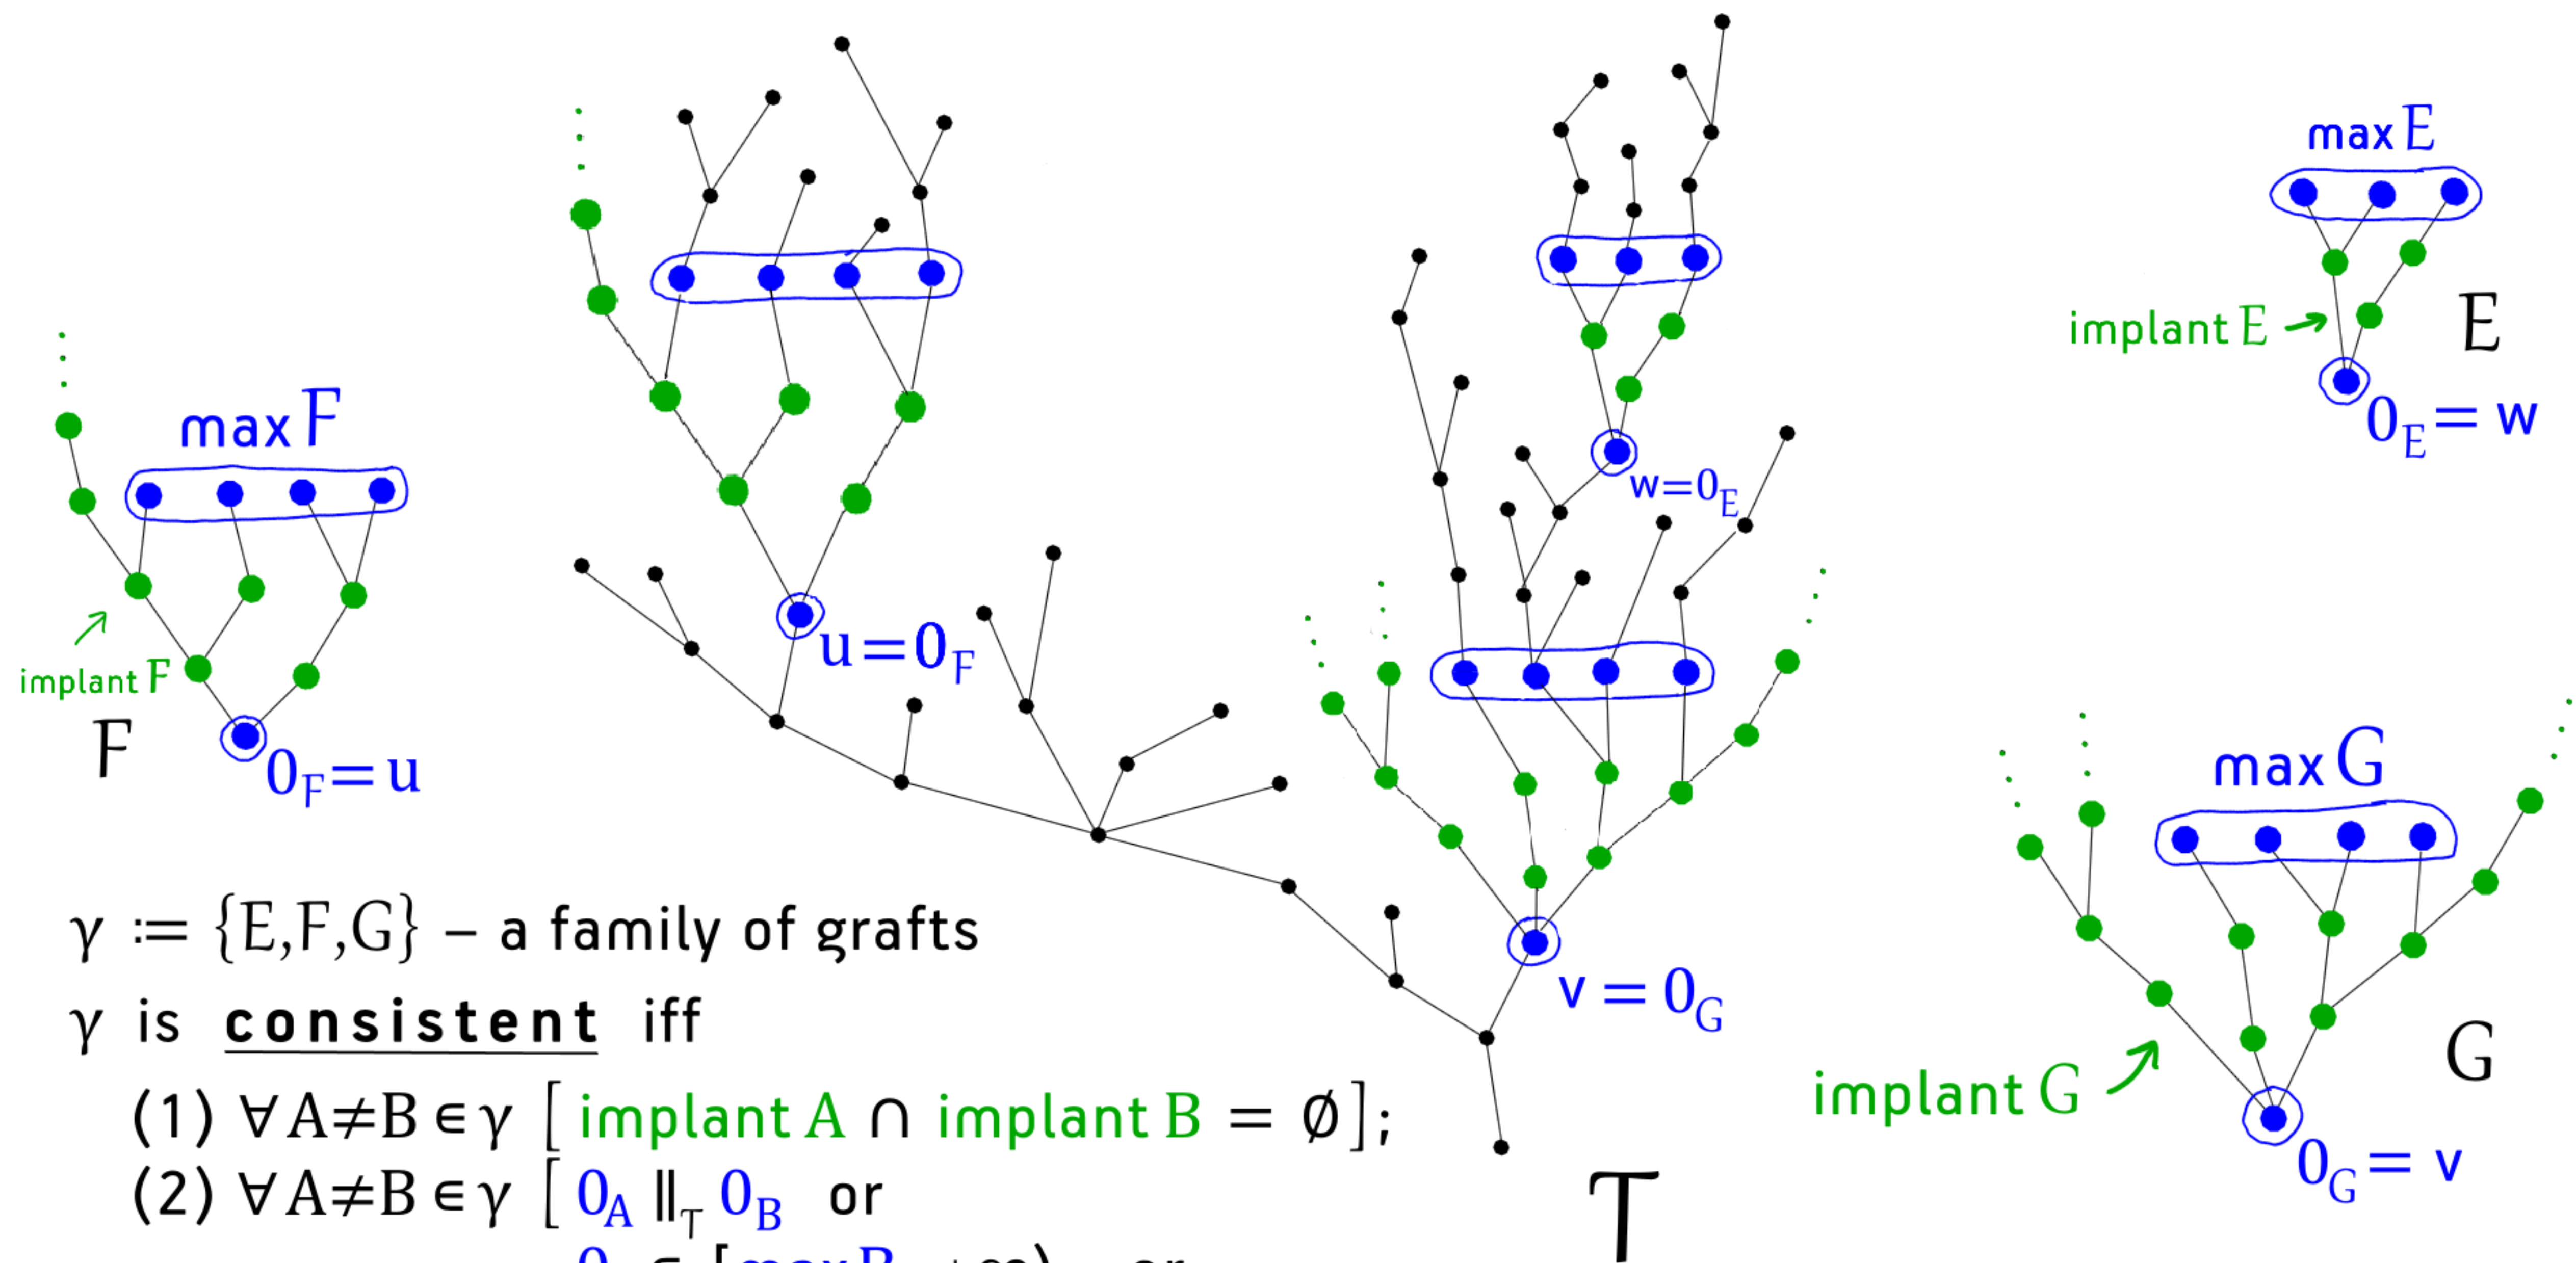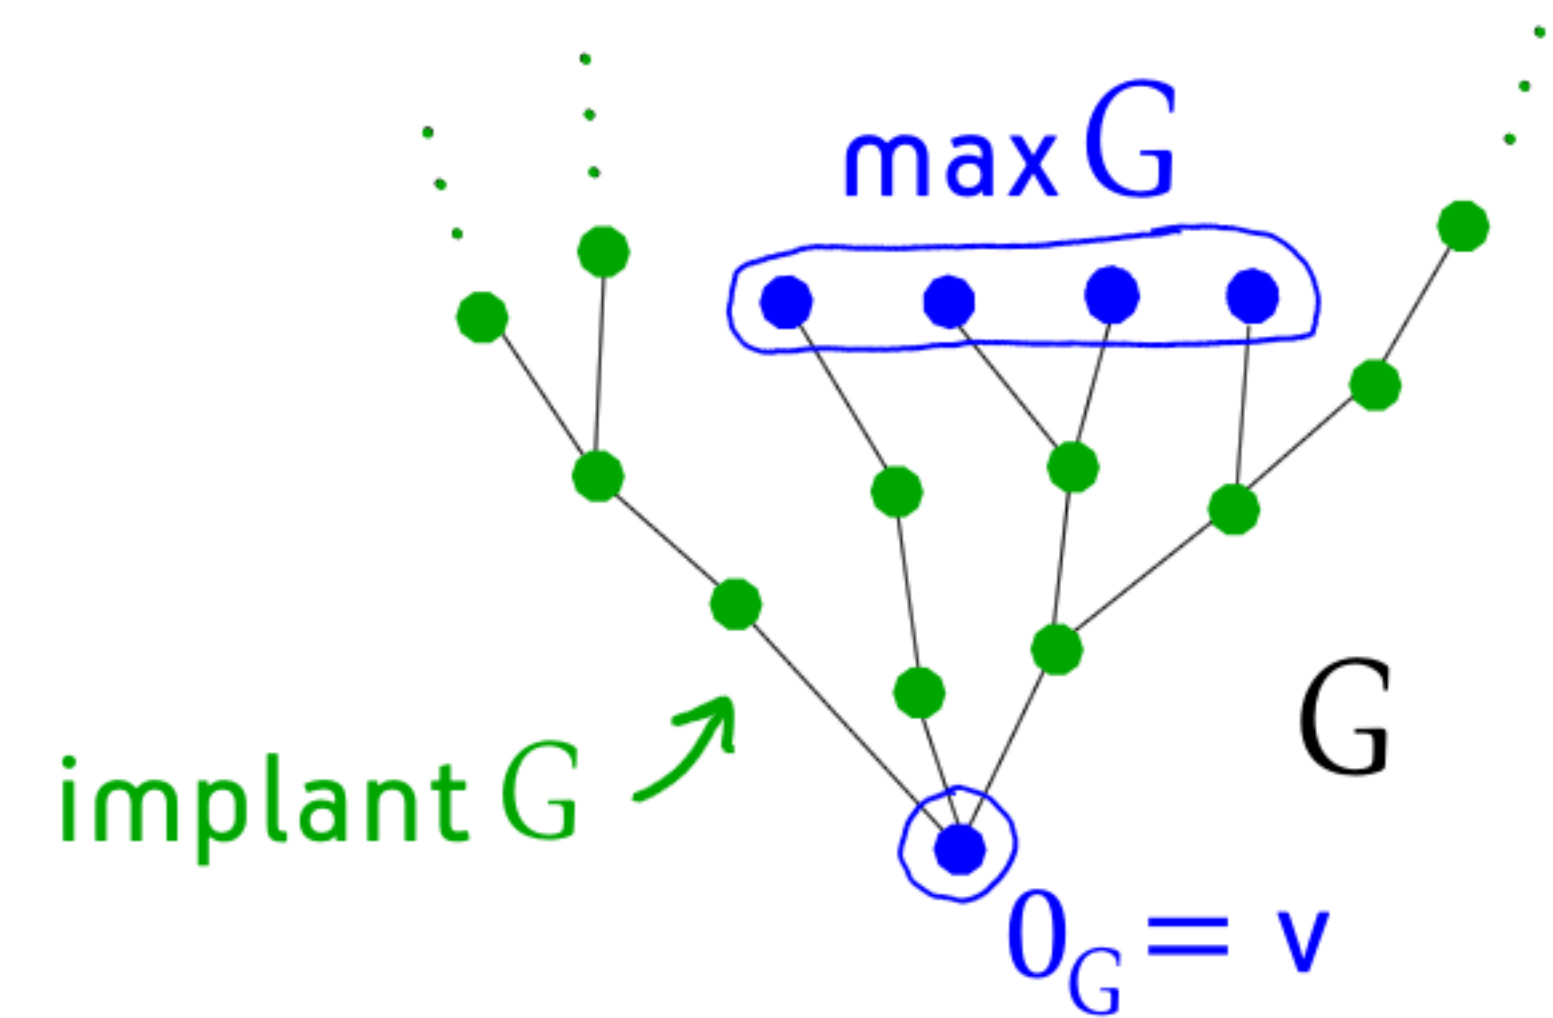

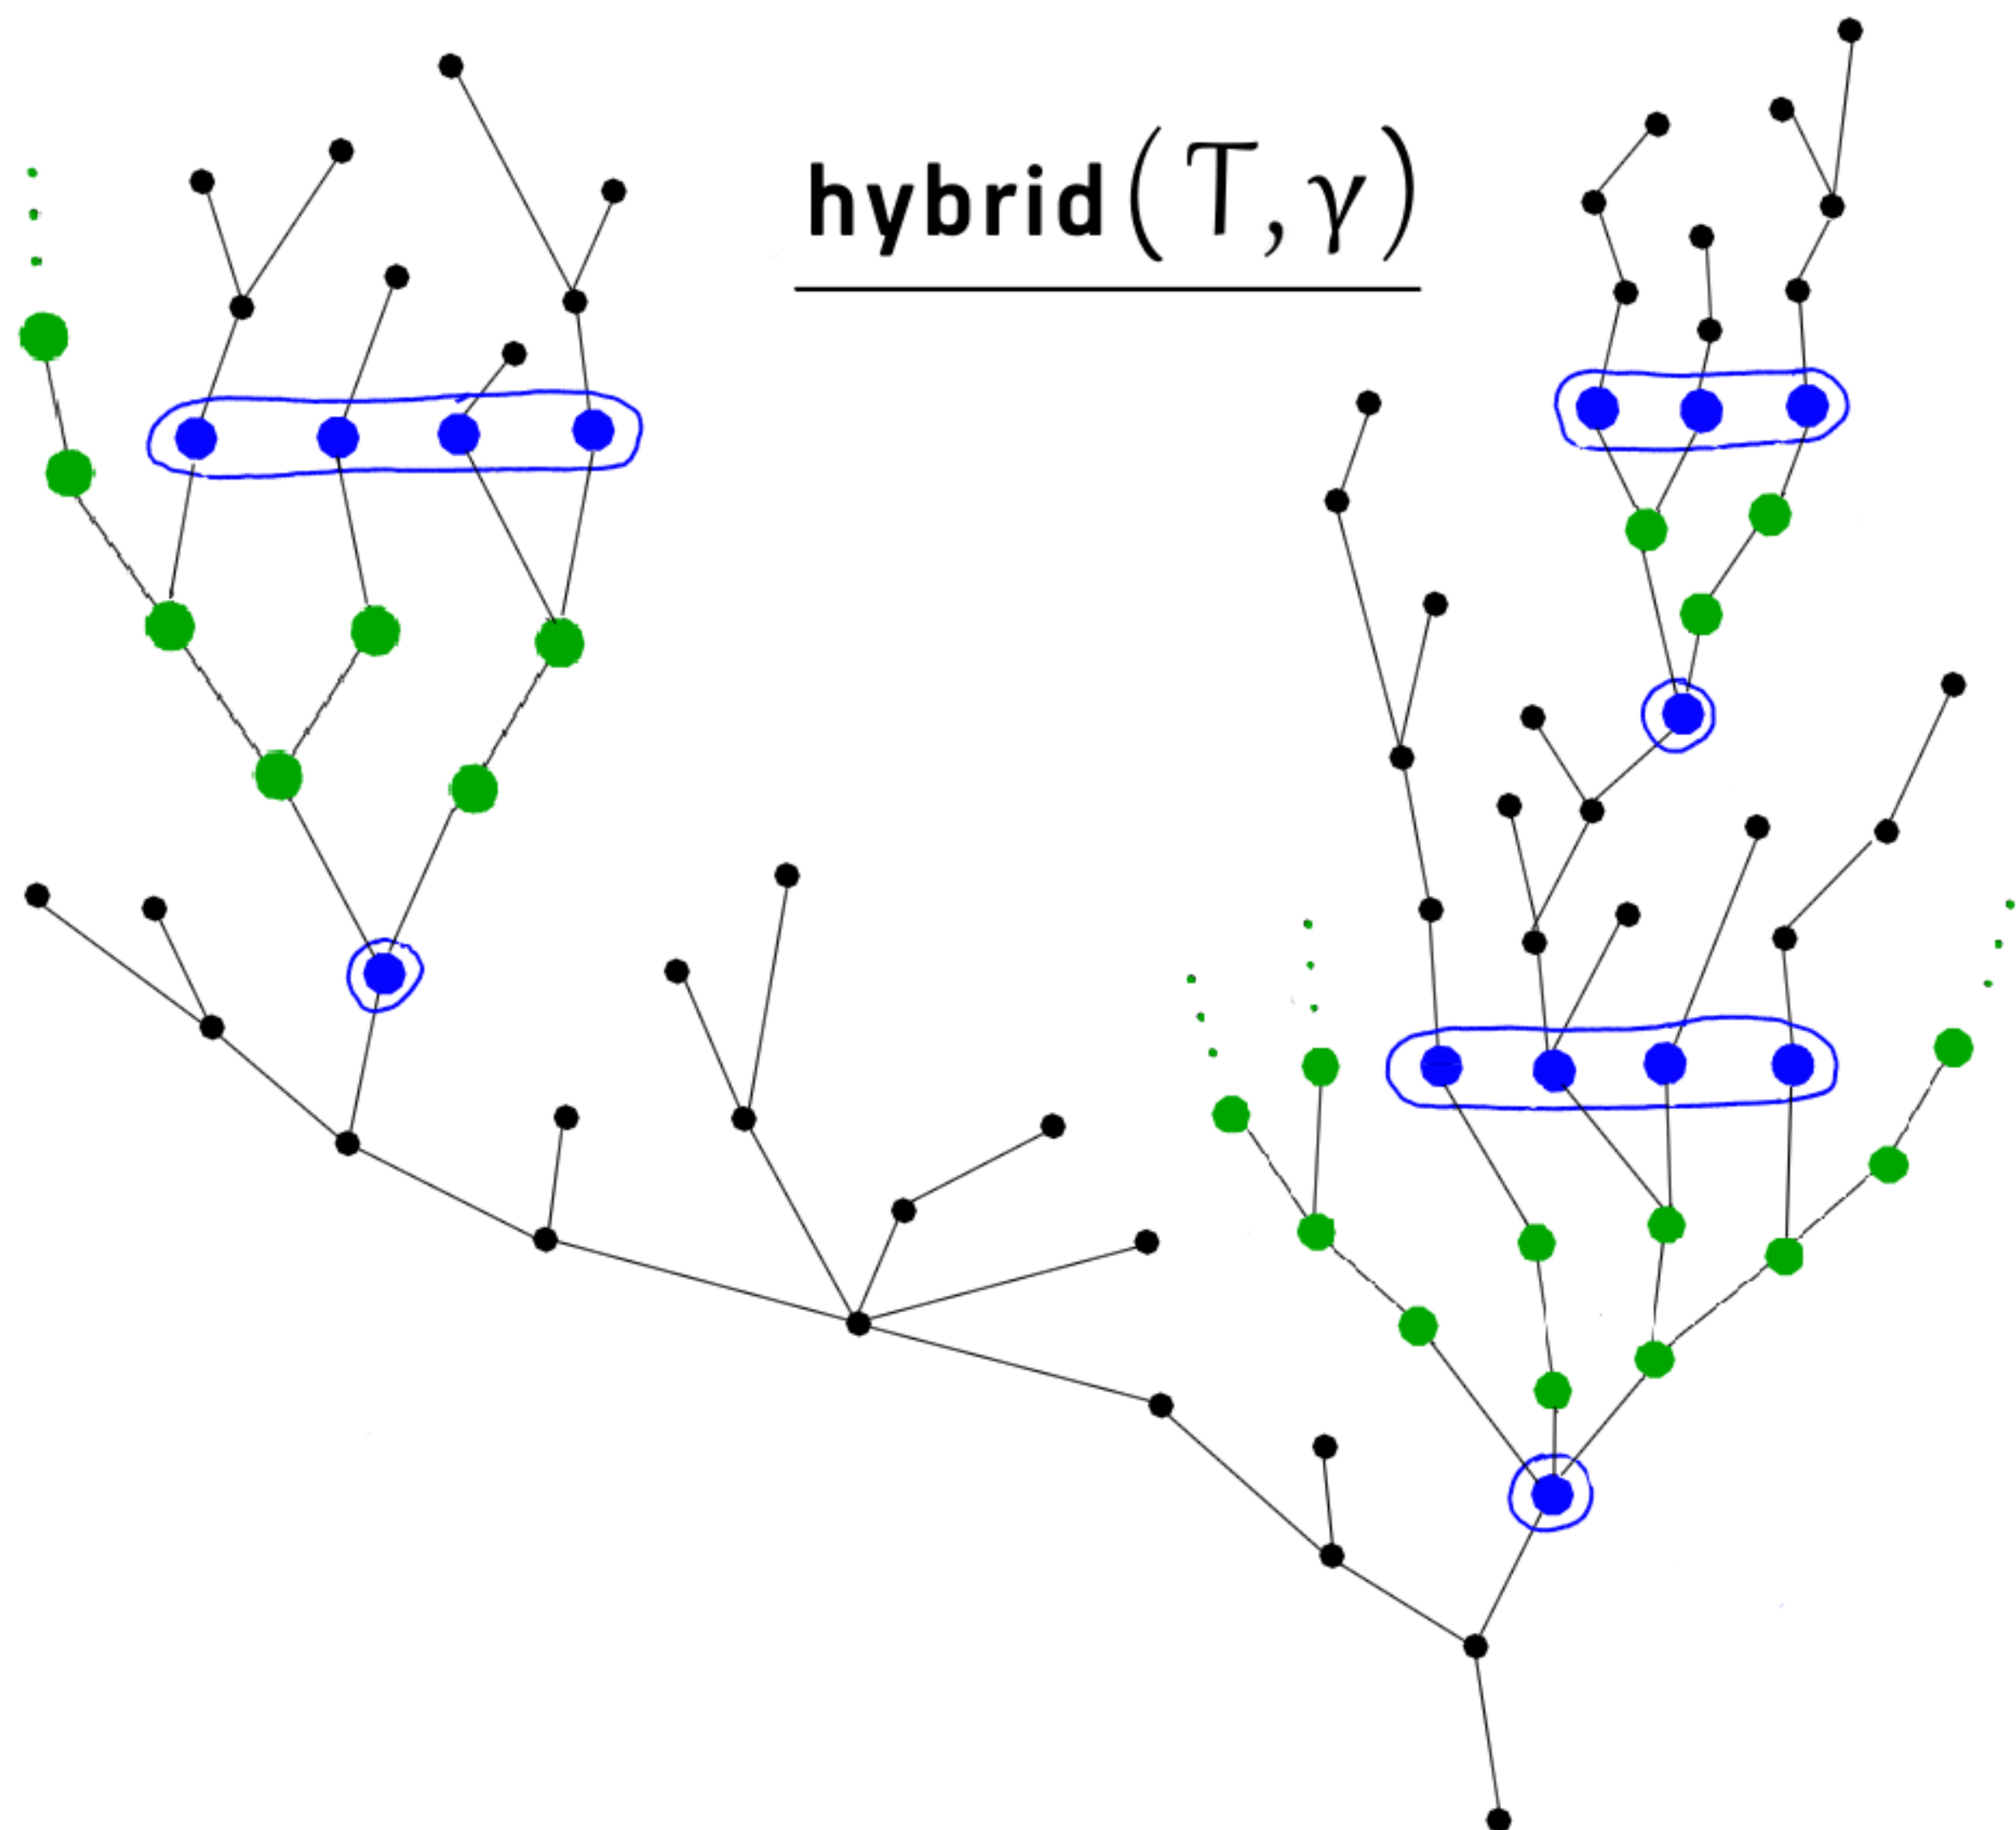



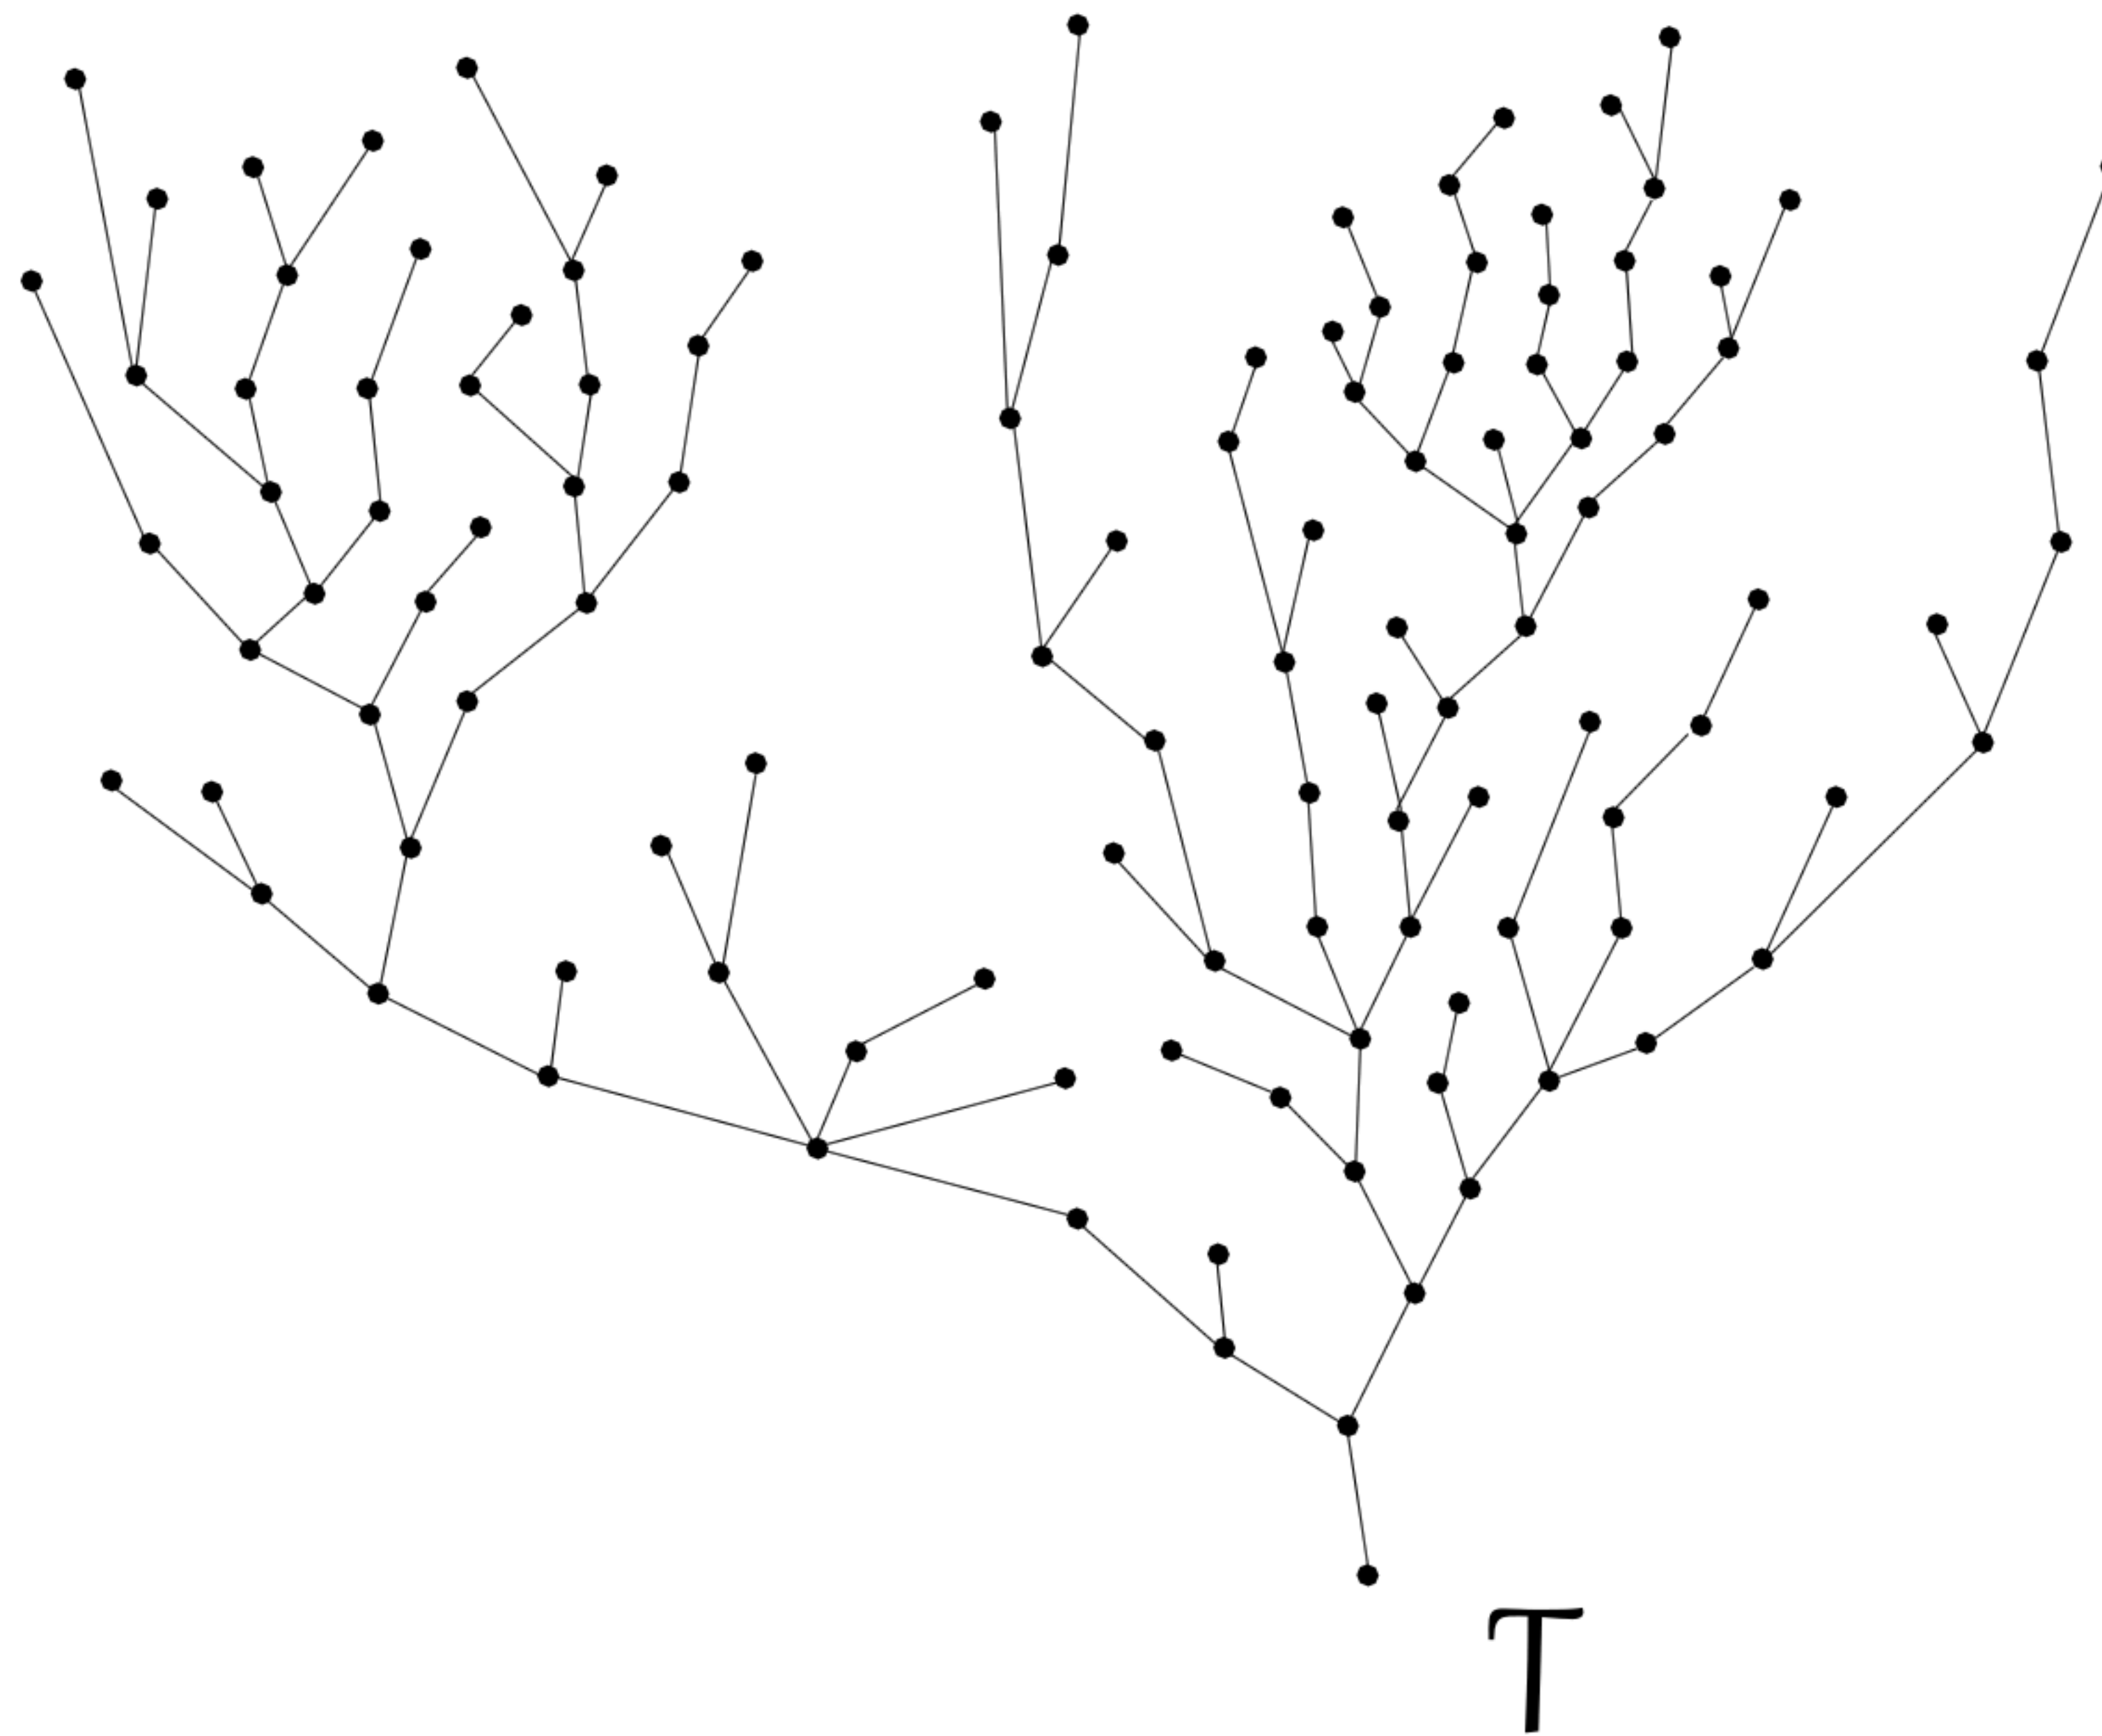

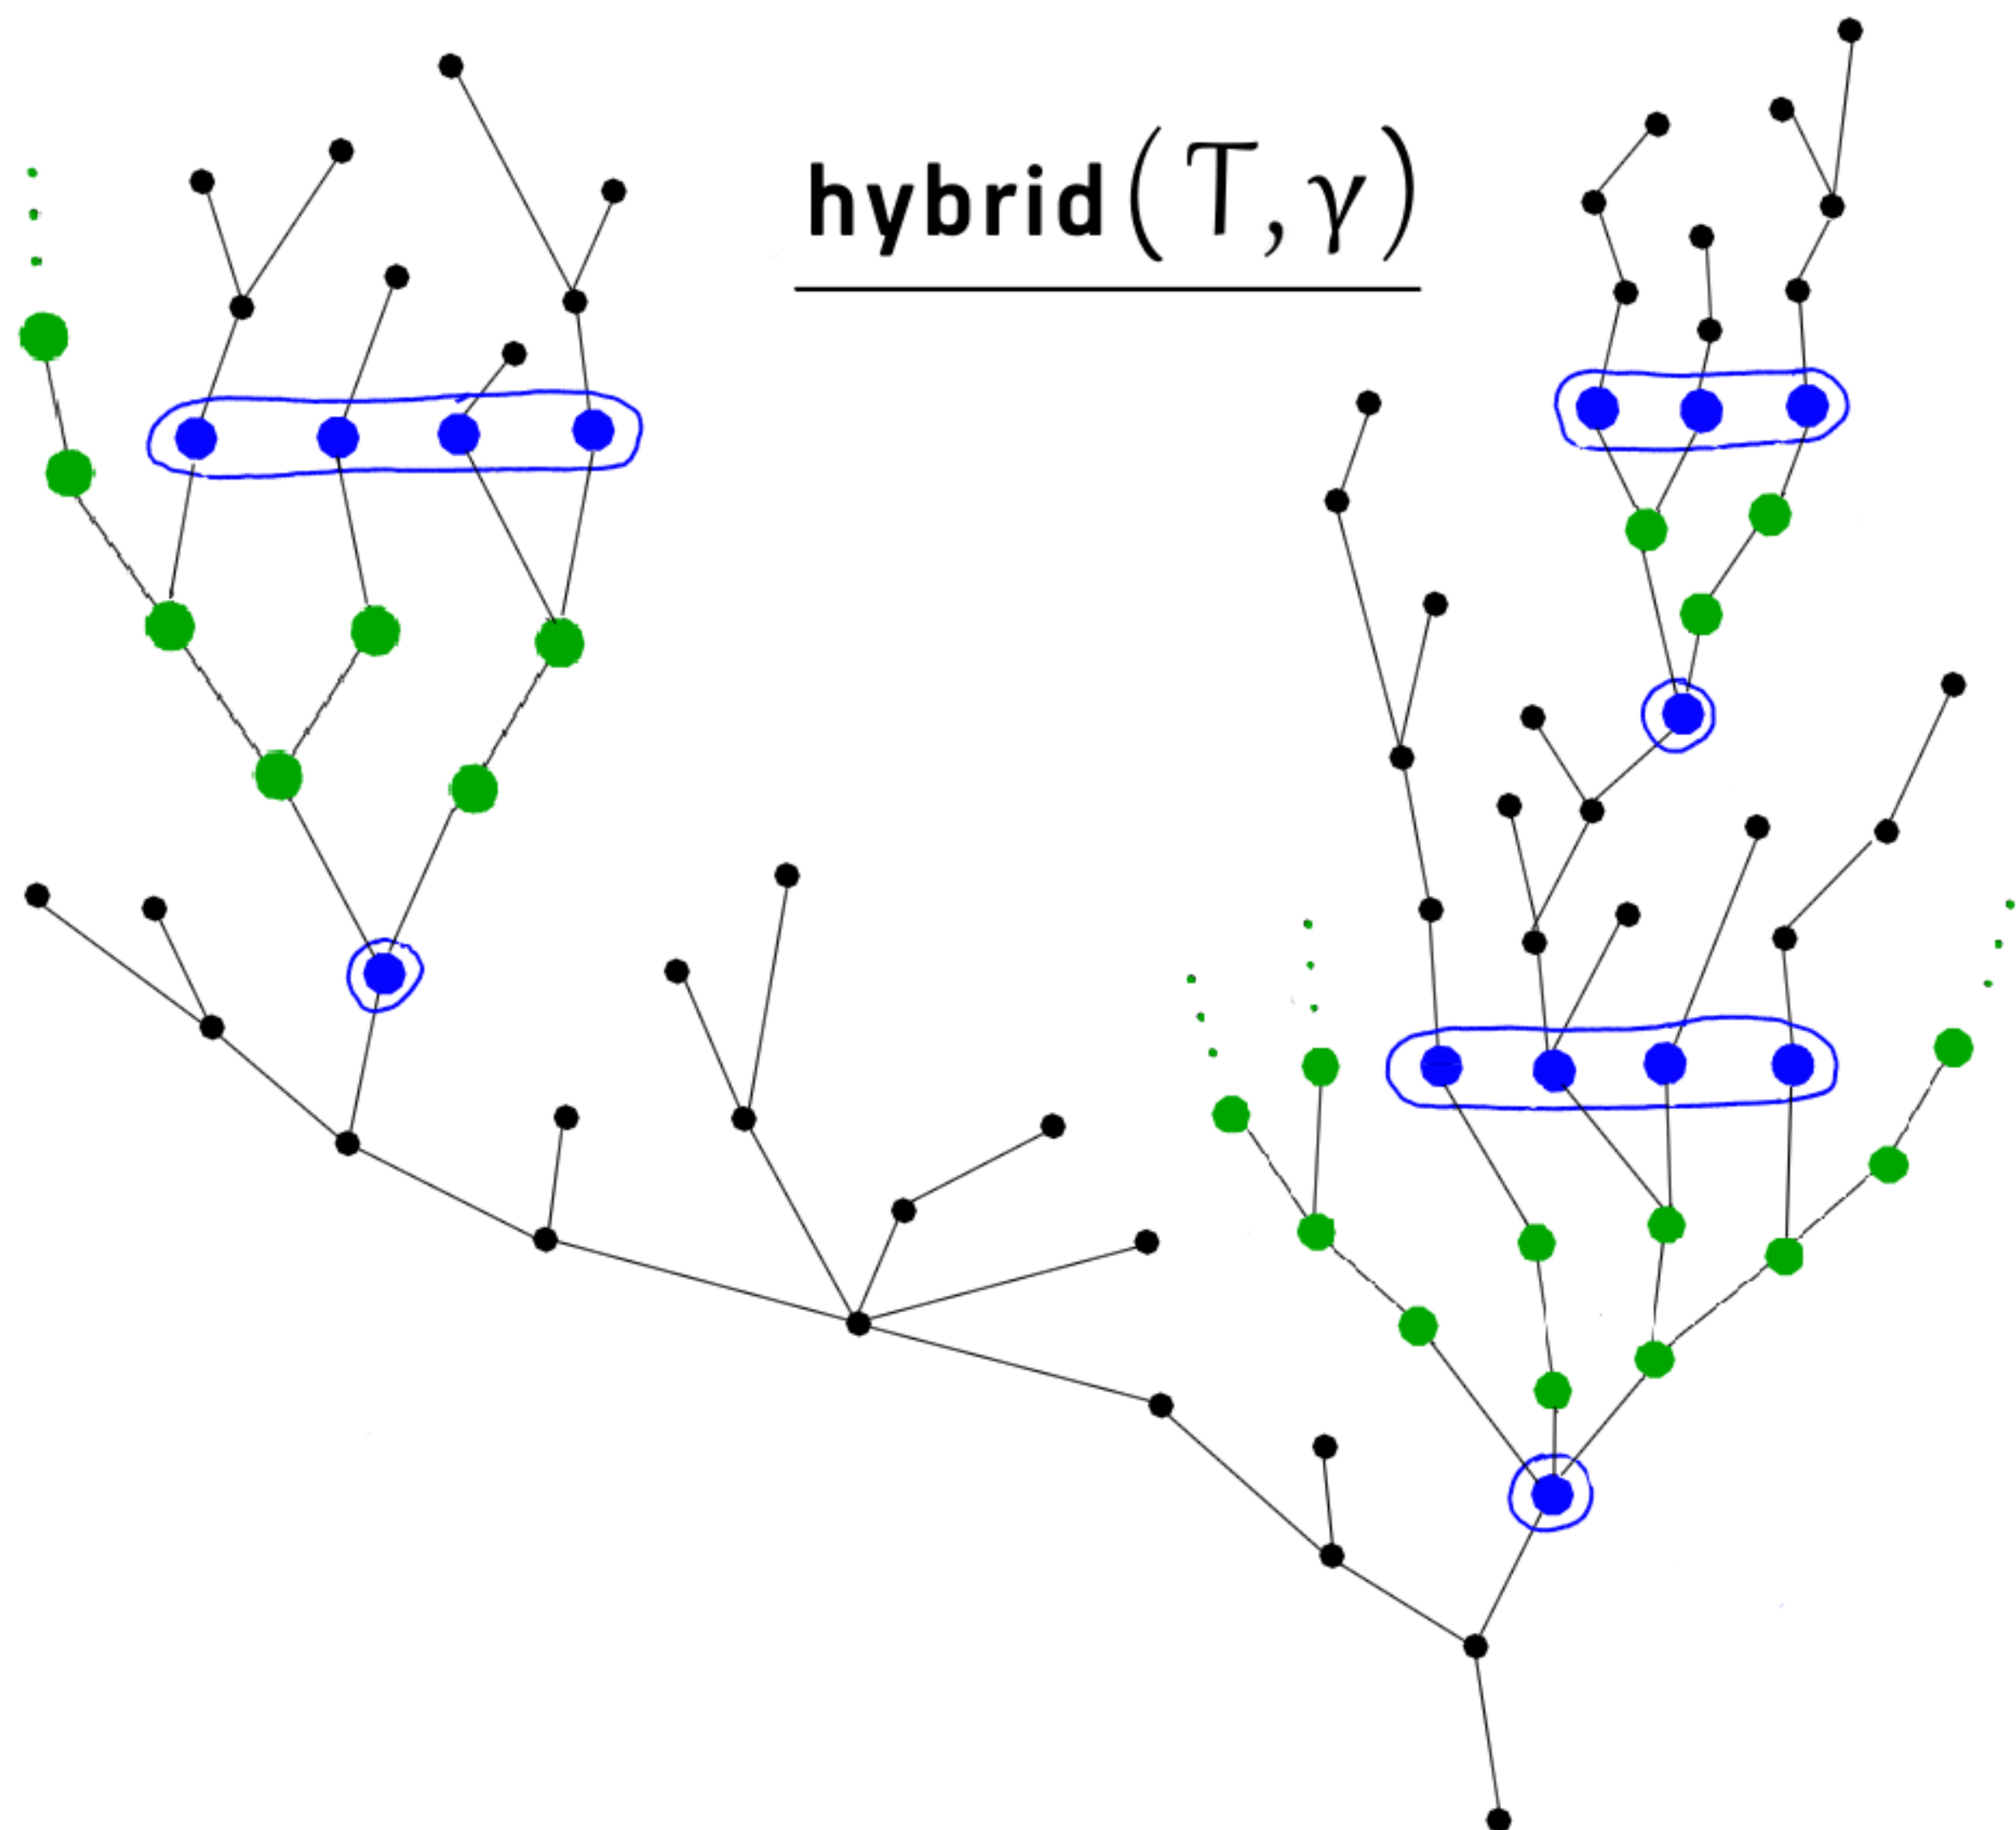

# FOLIAGE HYBRID OPERATION

We consider non-increasing foliage trees (i.e.,  $w > v \rightarrow \mathbf{F}_w \subseteq \mathbf{F}_v$ ).

**A** is a foliage graft for **F** iff

- (1)  $G$  is a graft for  $T$ ;
- (2)  $\mathbf{A}_{0_G} \subseteq \mathbf{F}_{0_G}$ ;
- (3)  $\forall m \in \max G \ [ \mathbf{A}_m = \mathbf{F}_m ]$ .

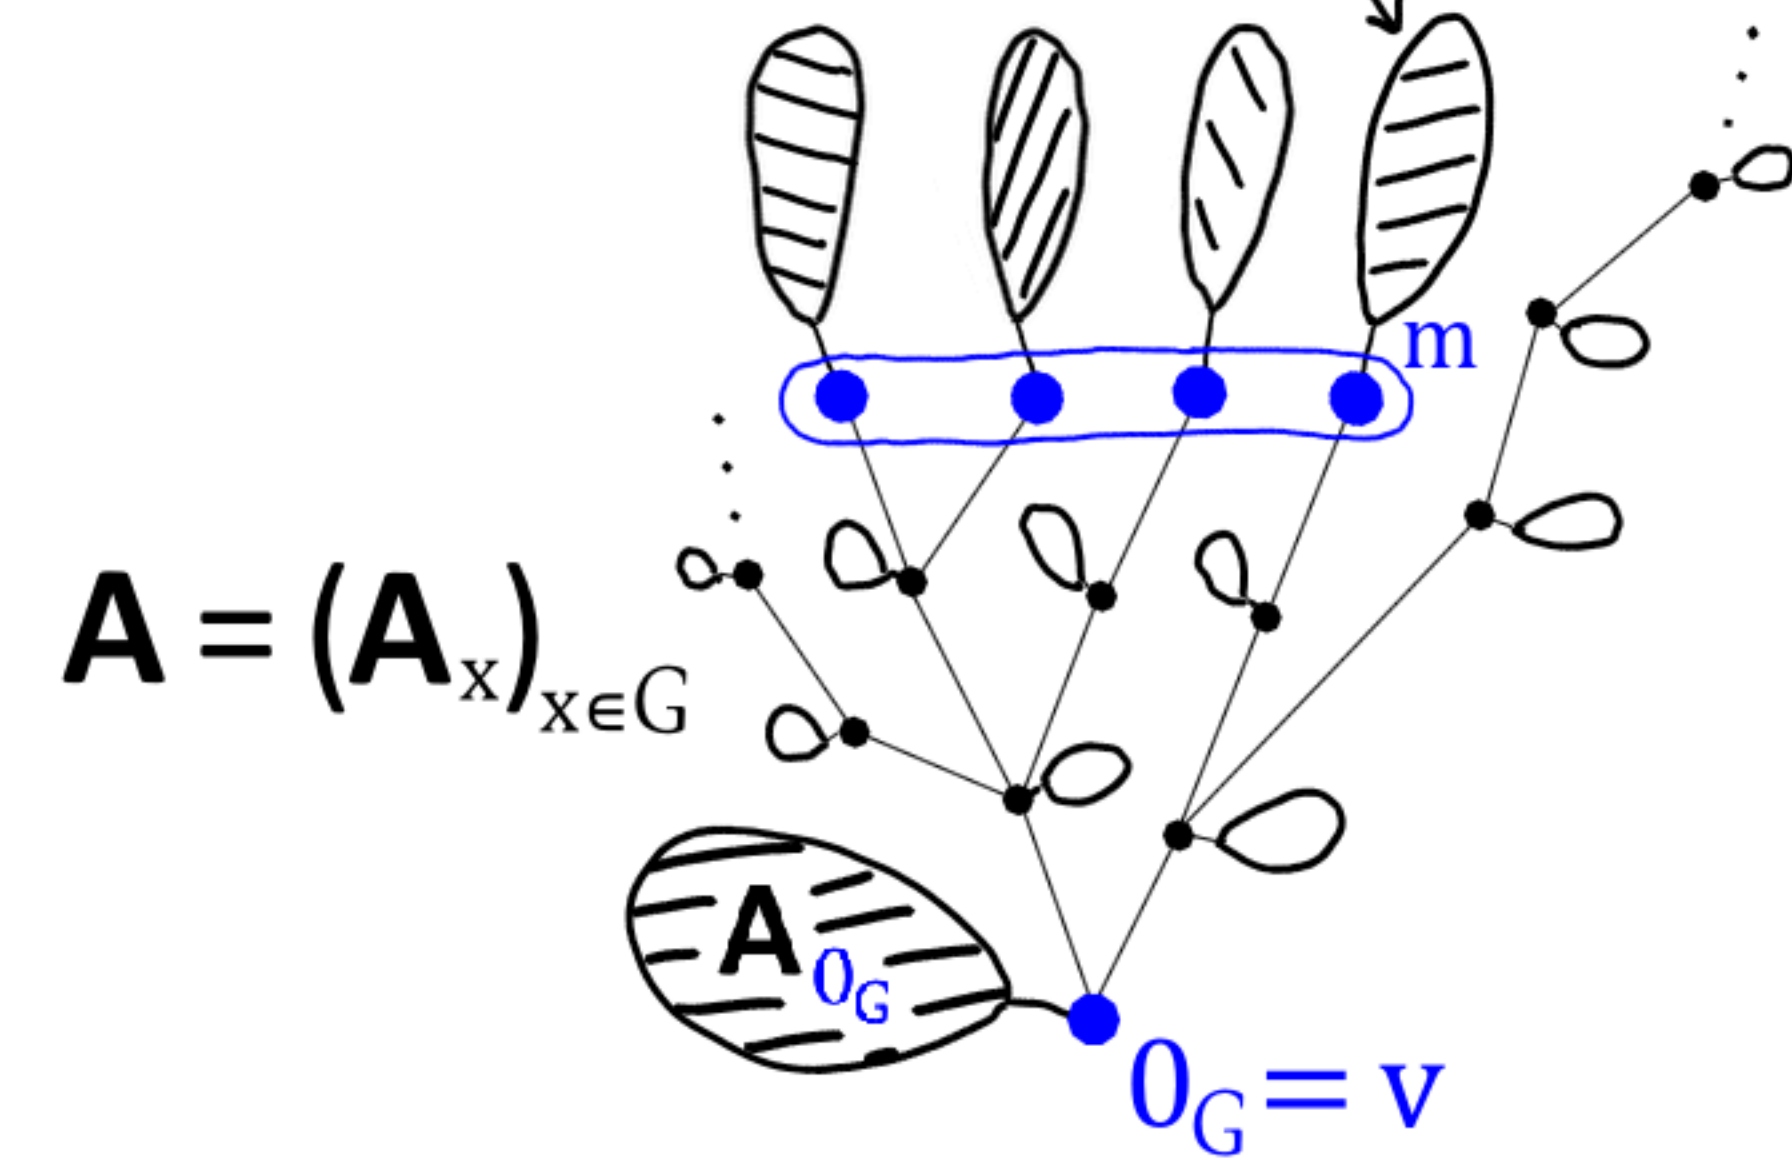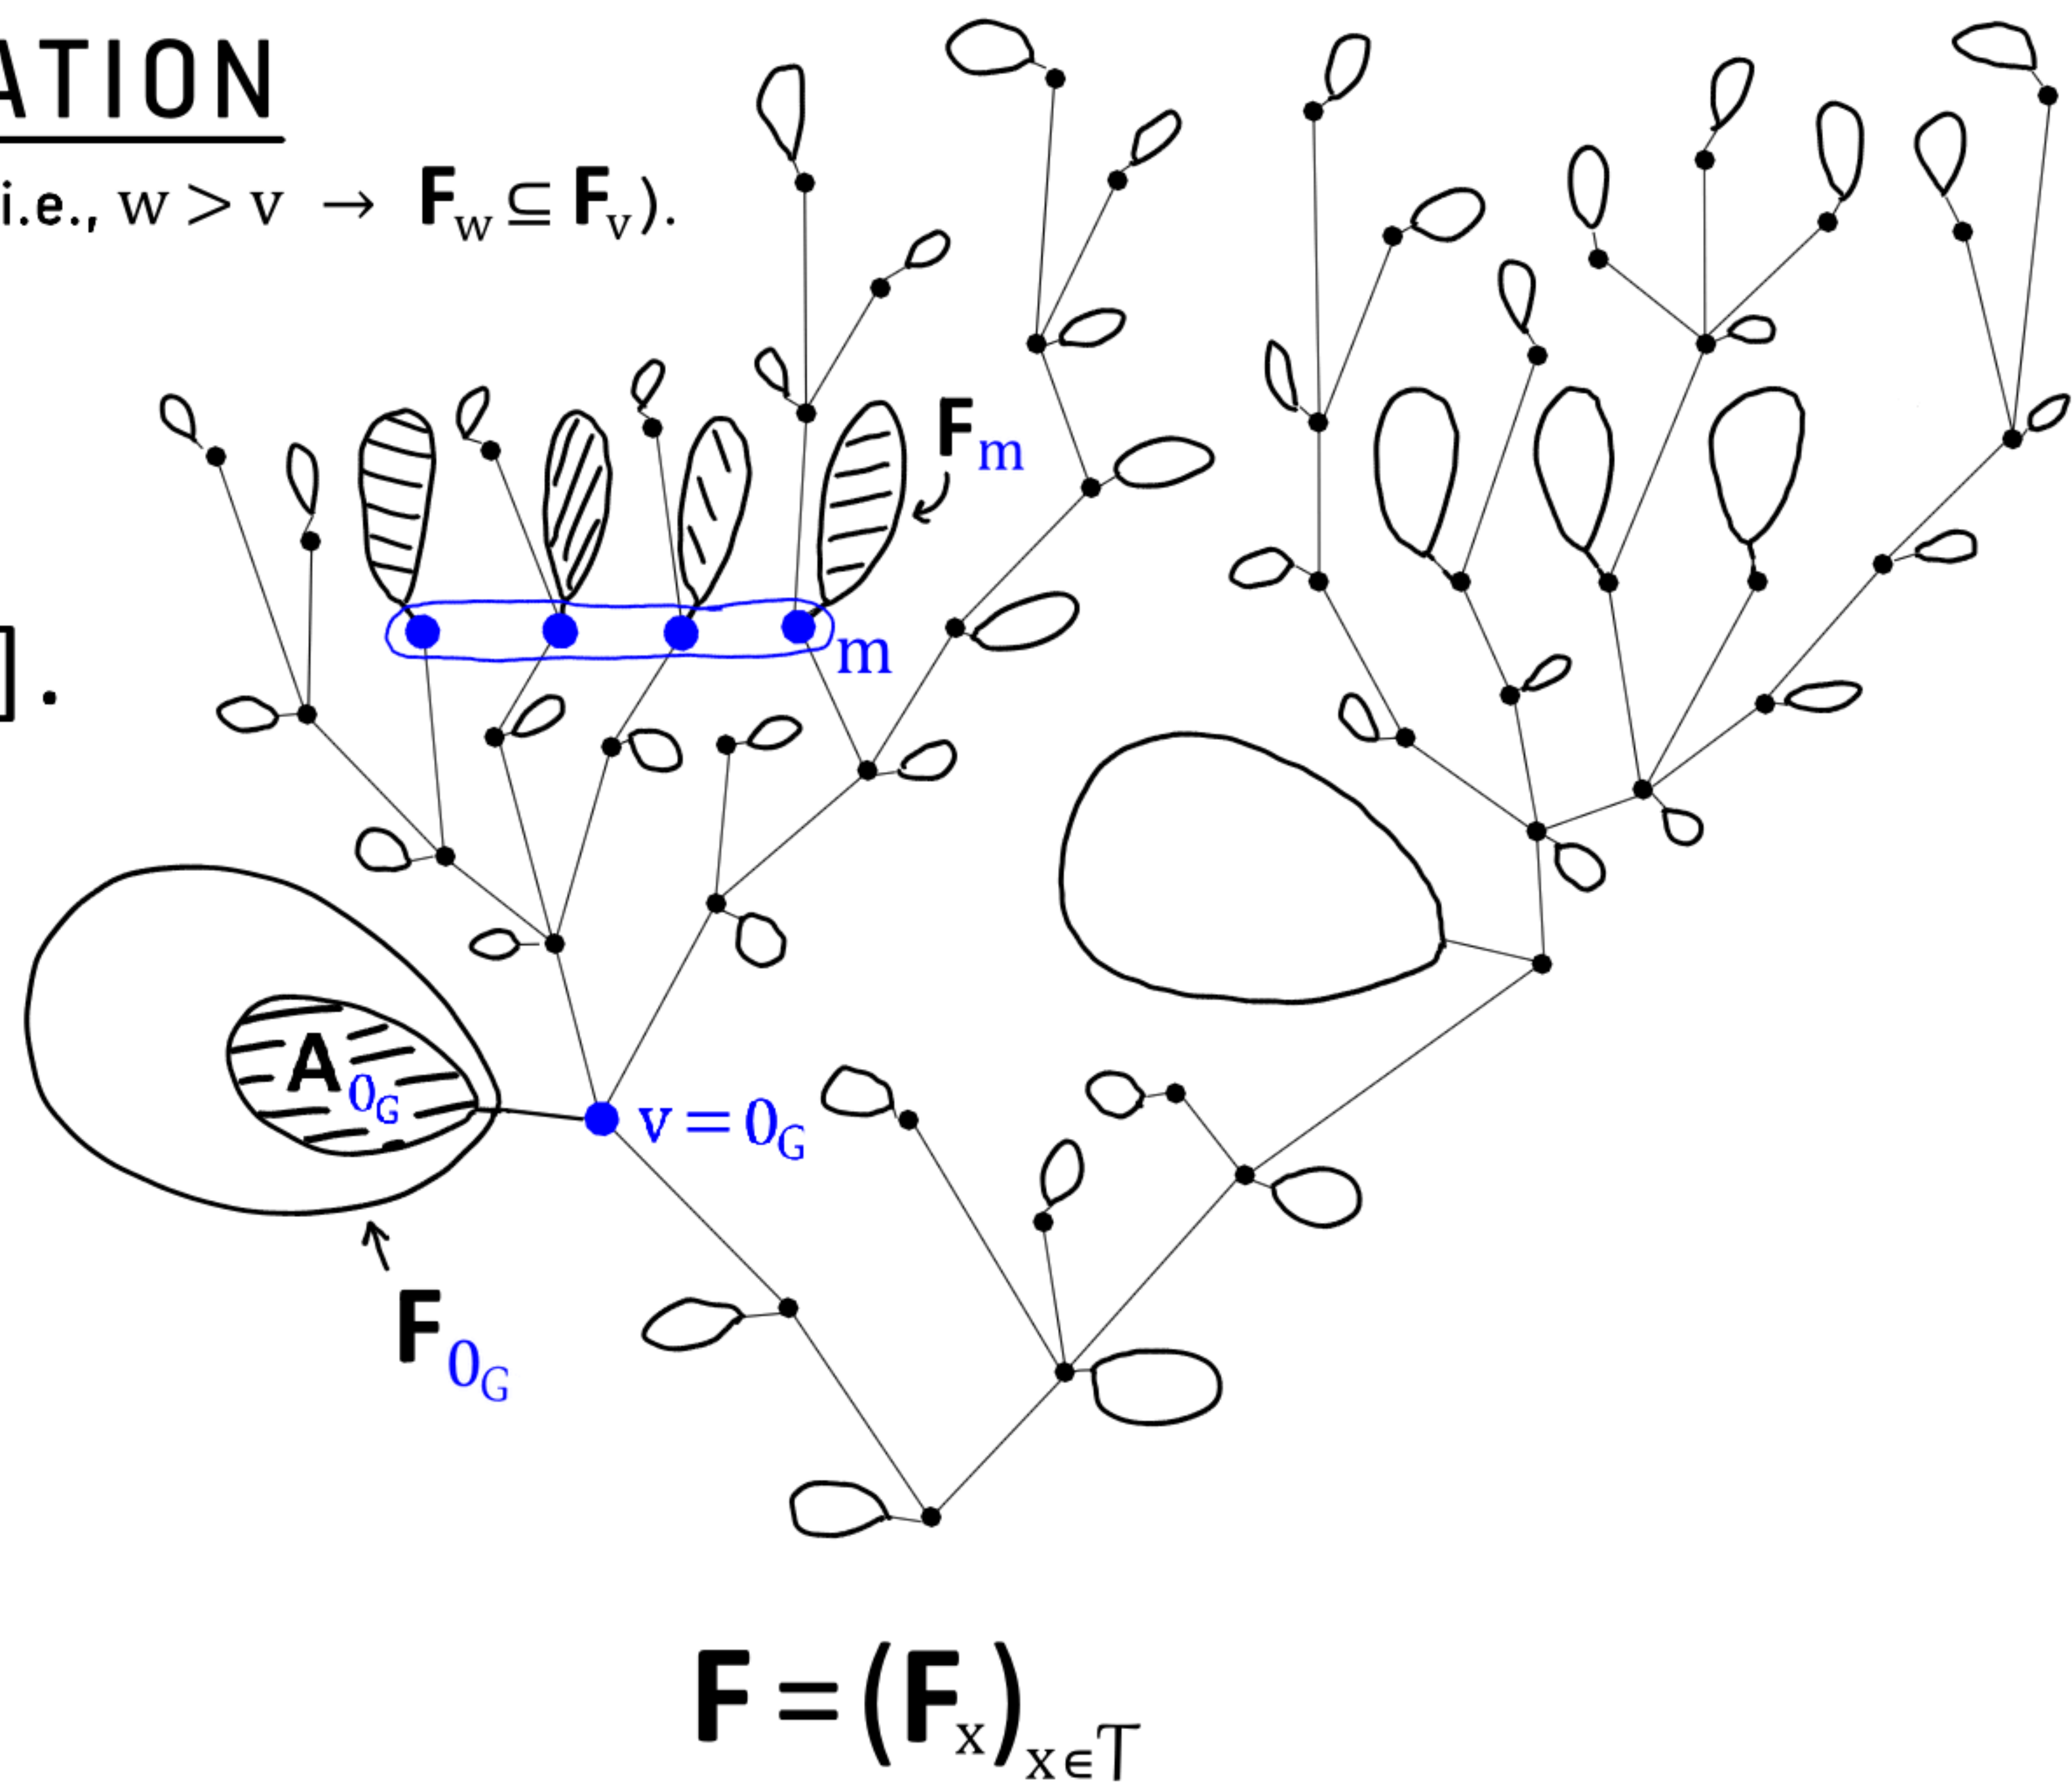



# FOLIAGE HYBRID OPERATION

We consider non-increasing foliage trees (i.e.,  $w > v \rightarrow \mathbf{F}_w \subseteq \mathbf{F}_v$ ).

**A** is a foliage graft for **F** iff

- (1)  $G$  is a graft for  $T$ ;
- (2)  $\mathbf{A}_{0_G} \subseteq \mathbf{F}_{0_G}$ ;
- (3)  $\forall m \in \max G \ [ \mathbf{A}_m = \mathbf{F}_m ]$ .

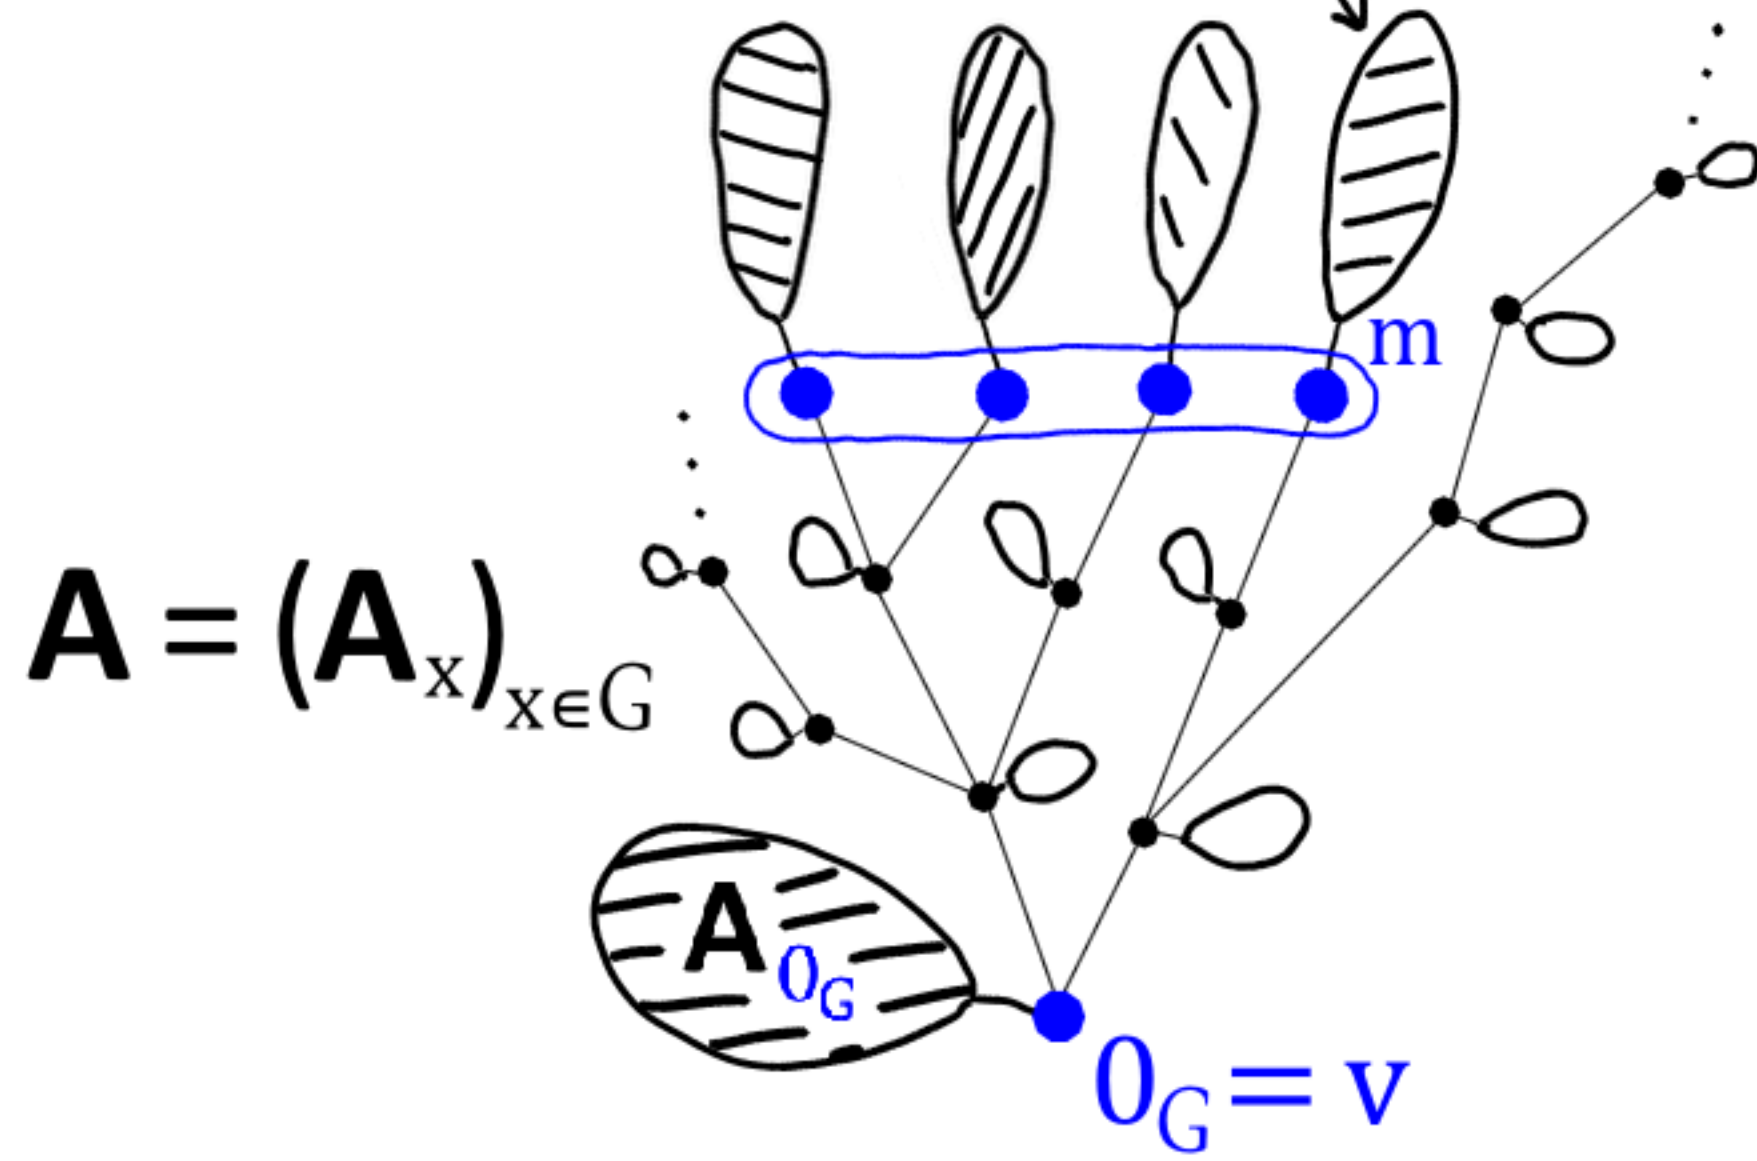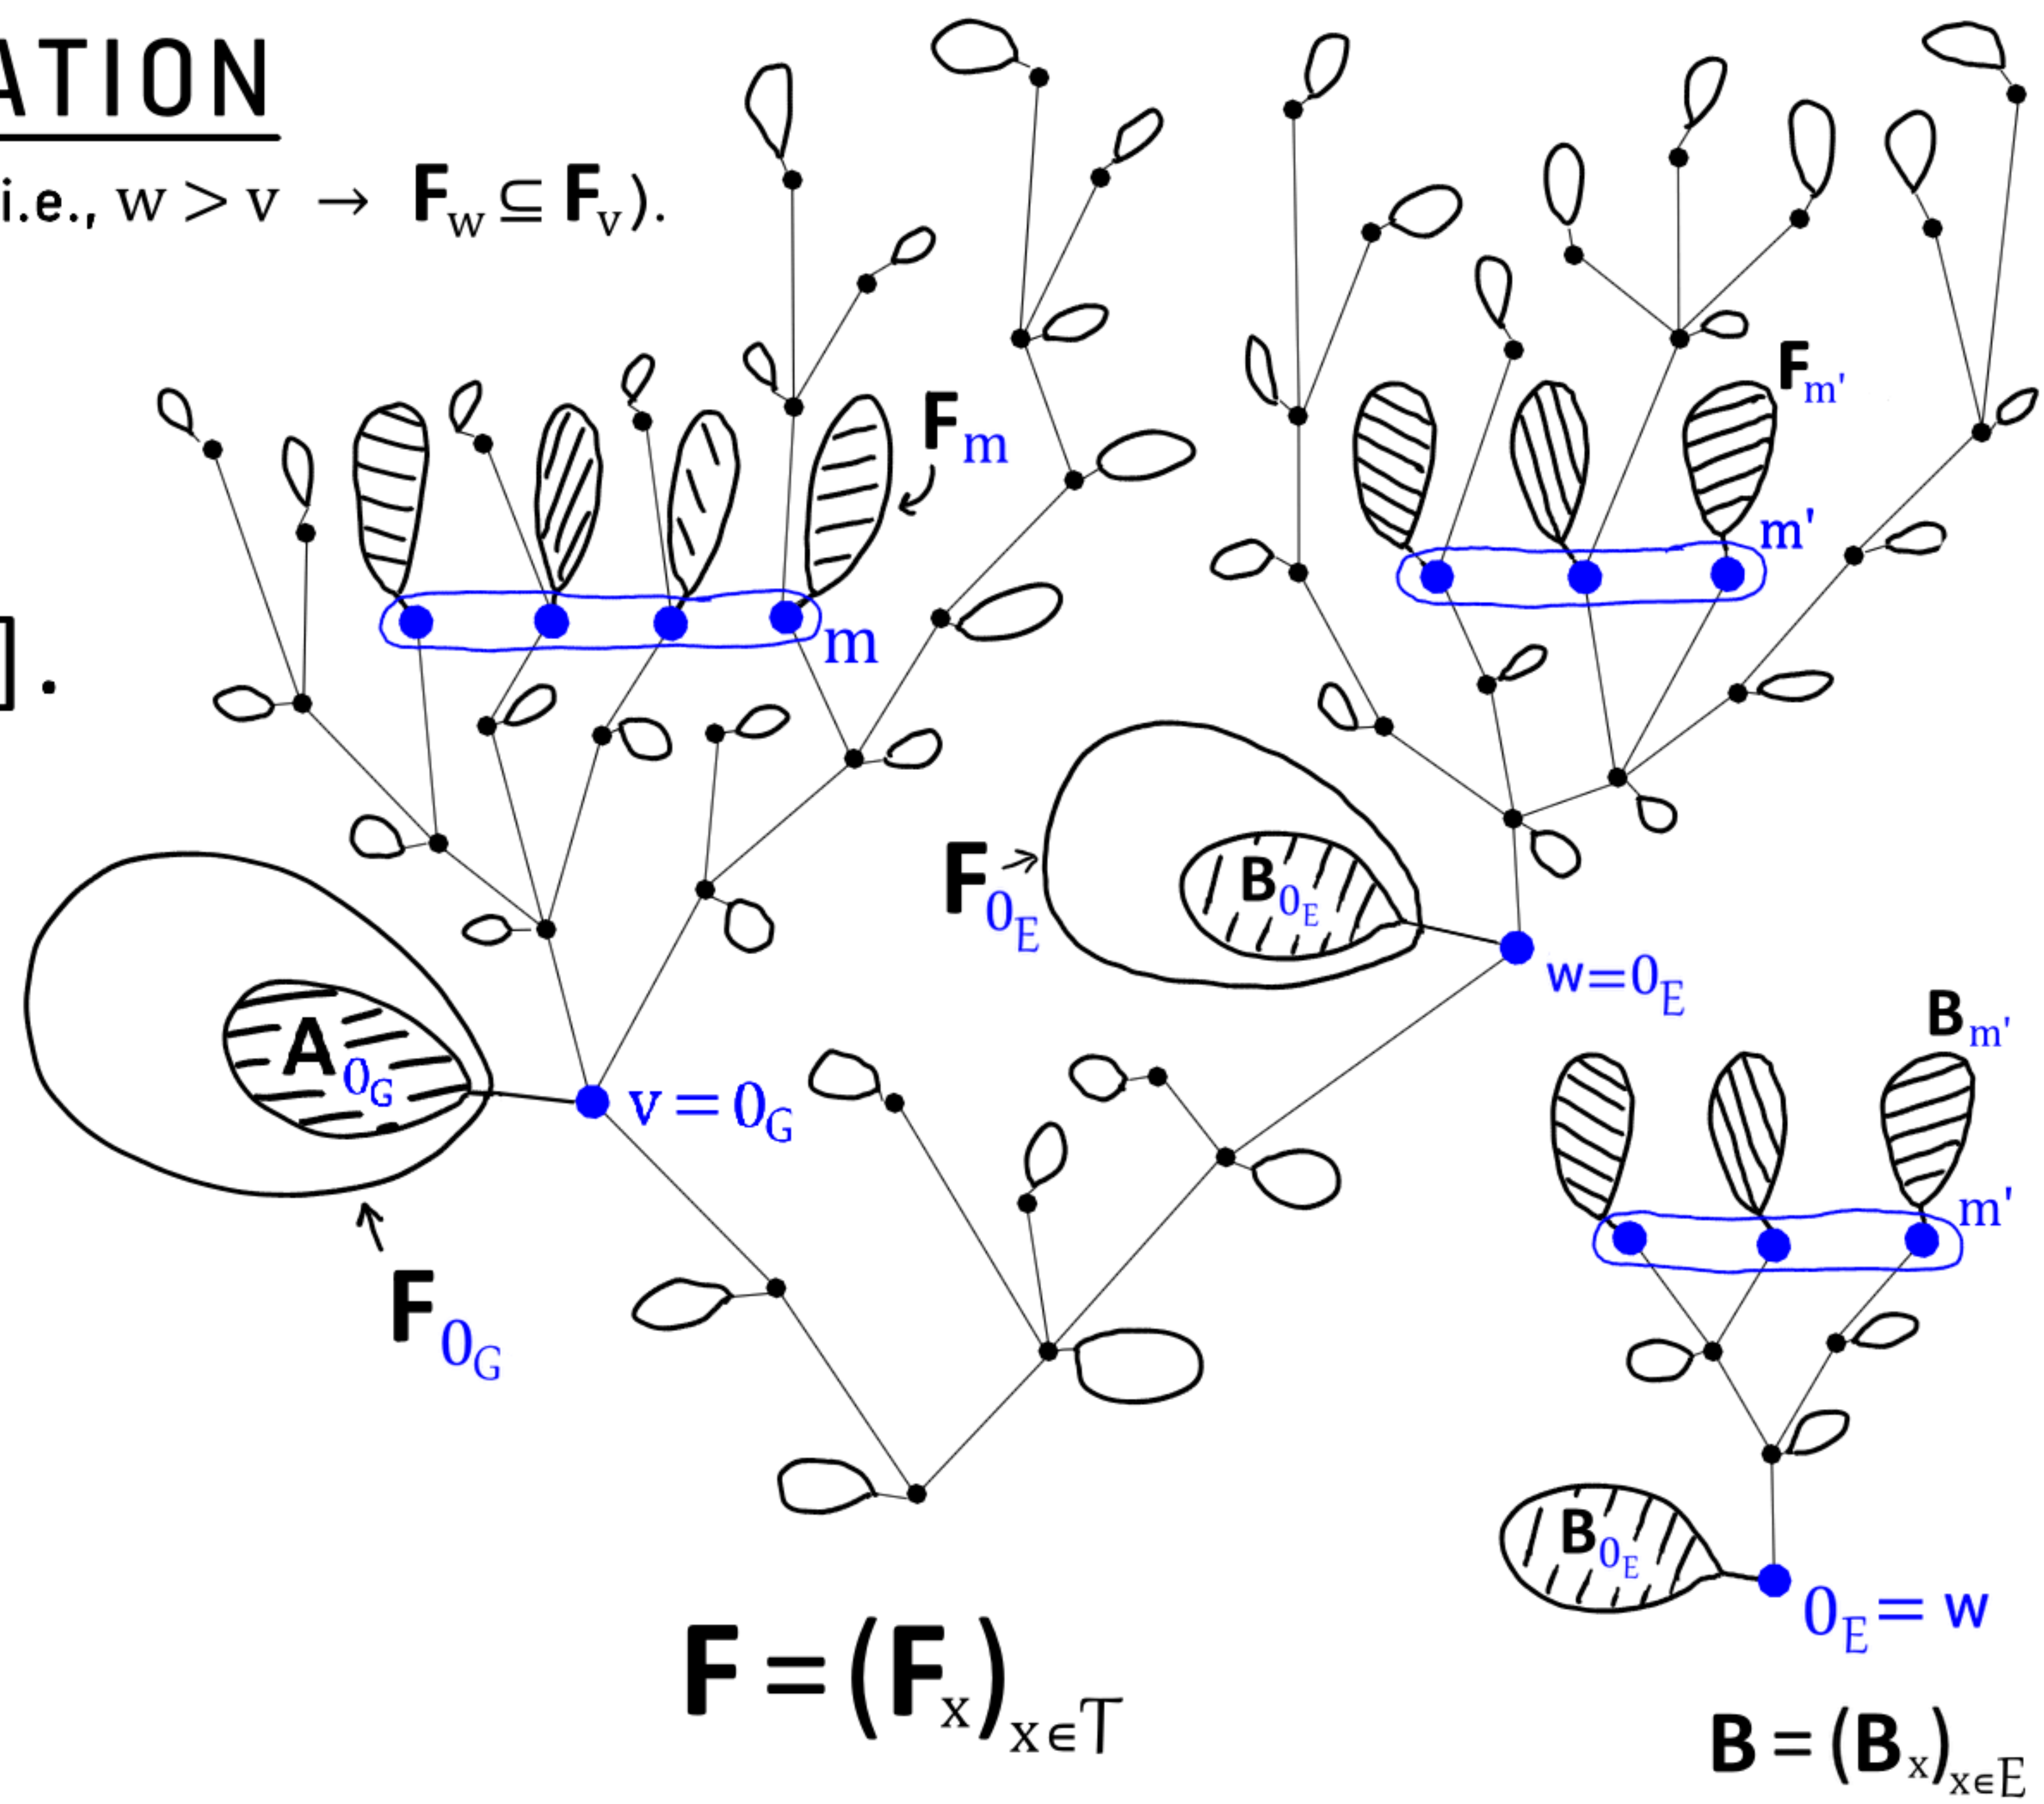



# FOLIAGE HYBRID OPERATION

We consider non-increasing foliage trees (i.e.,  $w > v \rightarrow \mathbf{F}_w \subseteq \mathbf{F}_v$ ).

**A** is a foliage graft for **F** iff

- (1)  $G$  is a graft for  $T$ ;
- (2)  $\mathbf{A}_{0_G} \subseteq \mathbf{F}_{0_G}$ ;
- (3)  $\forall m \in \max G \ [ \mathbf{A}_m = \mathbf{F}_m ]$ .

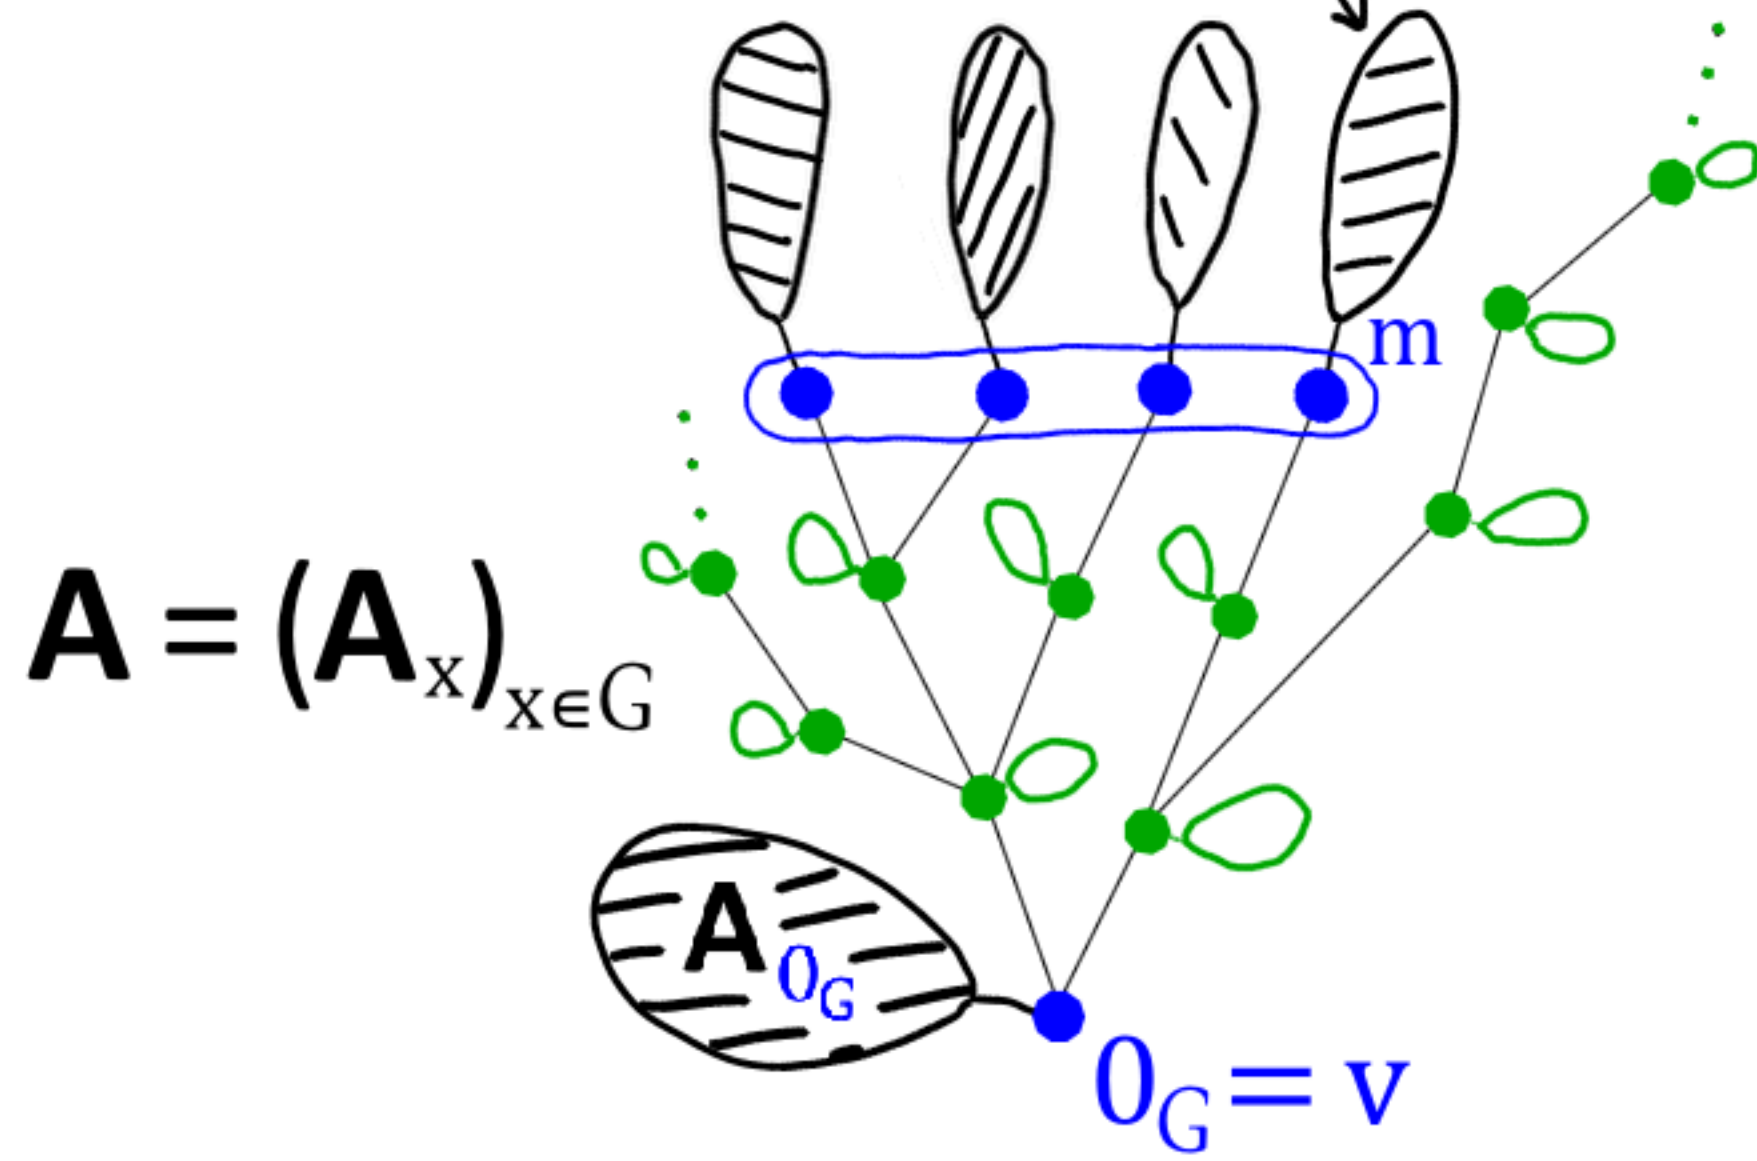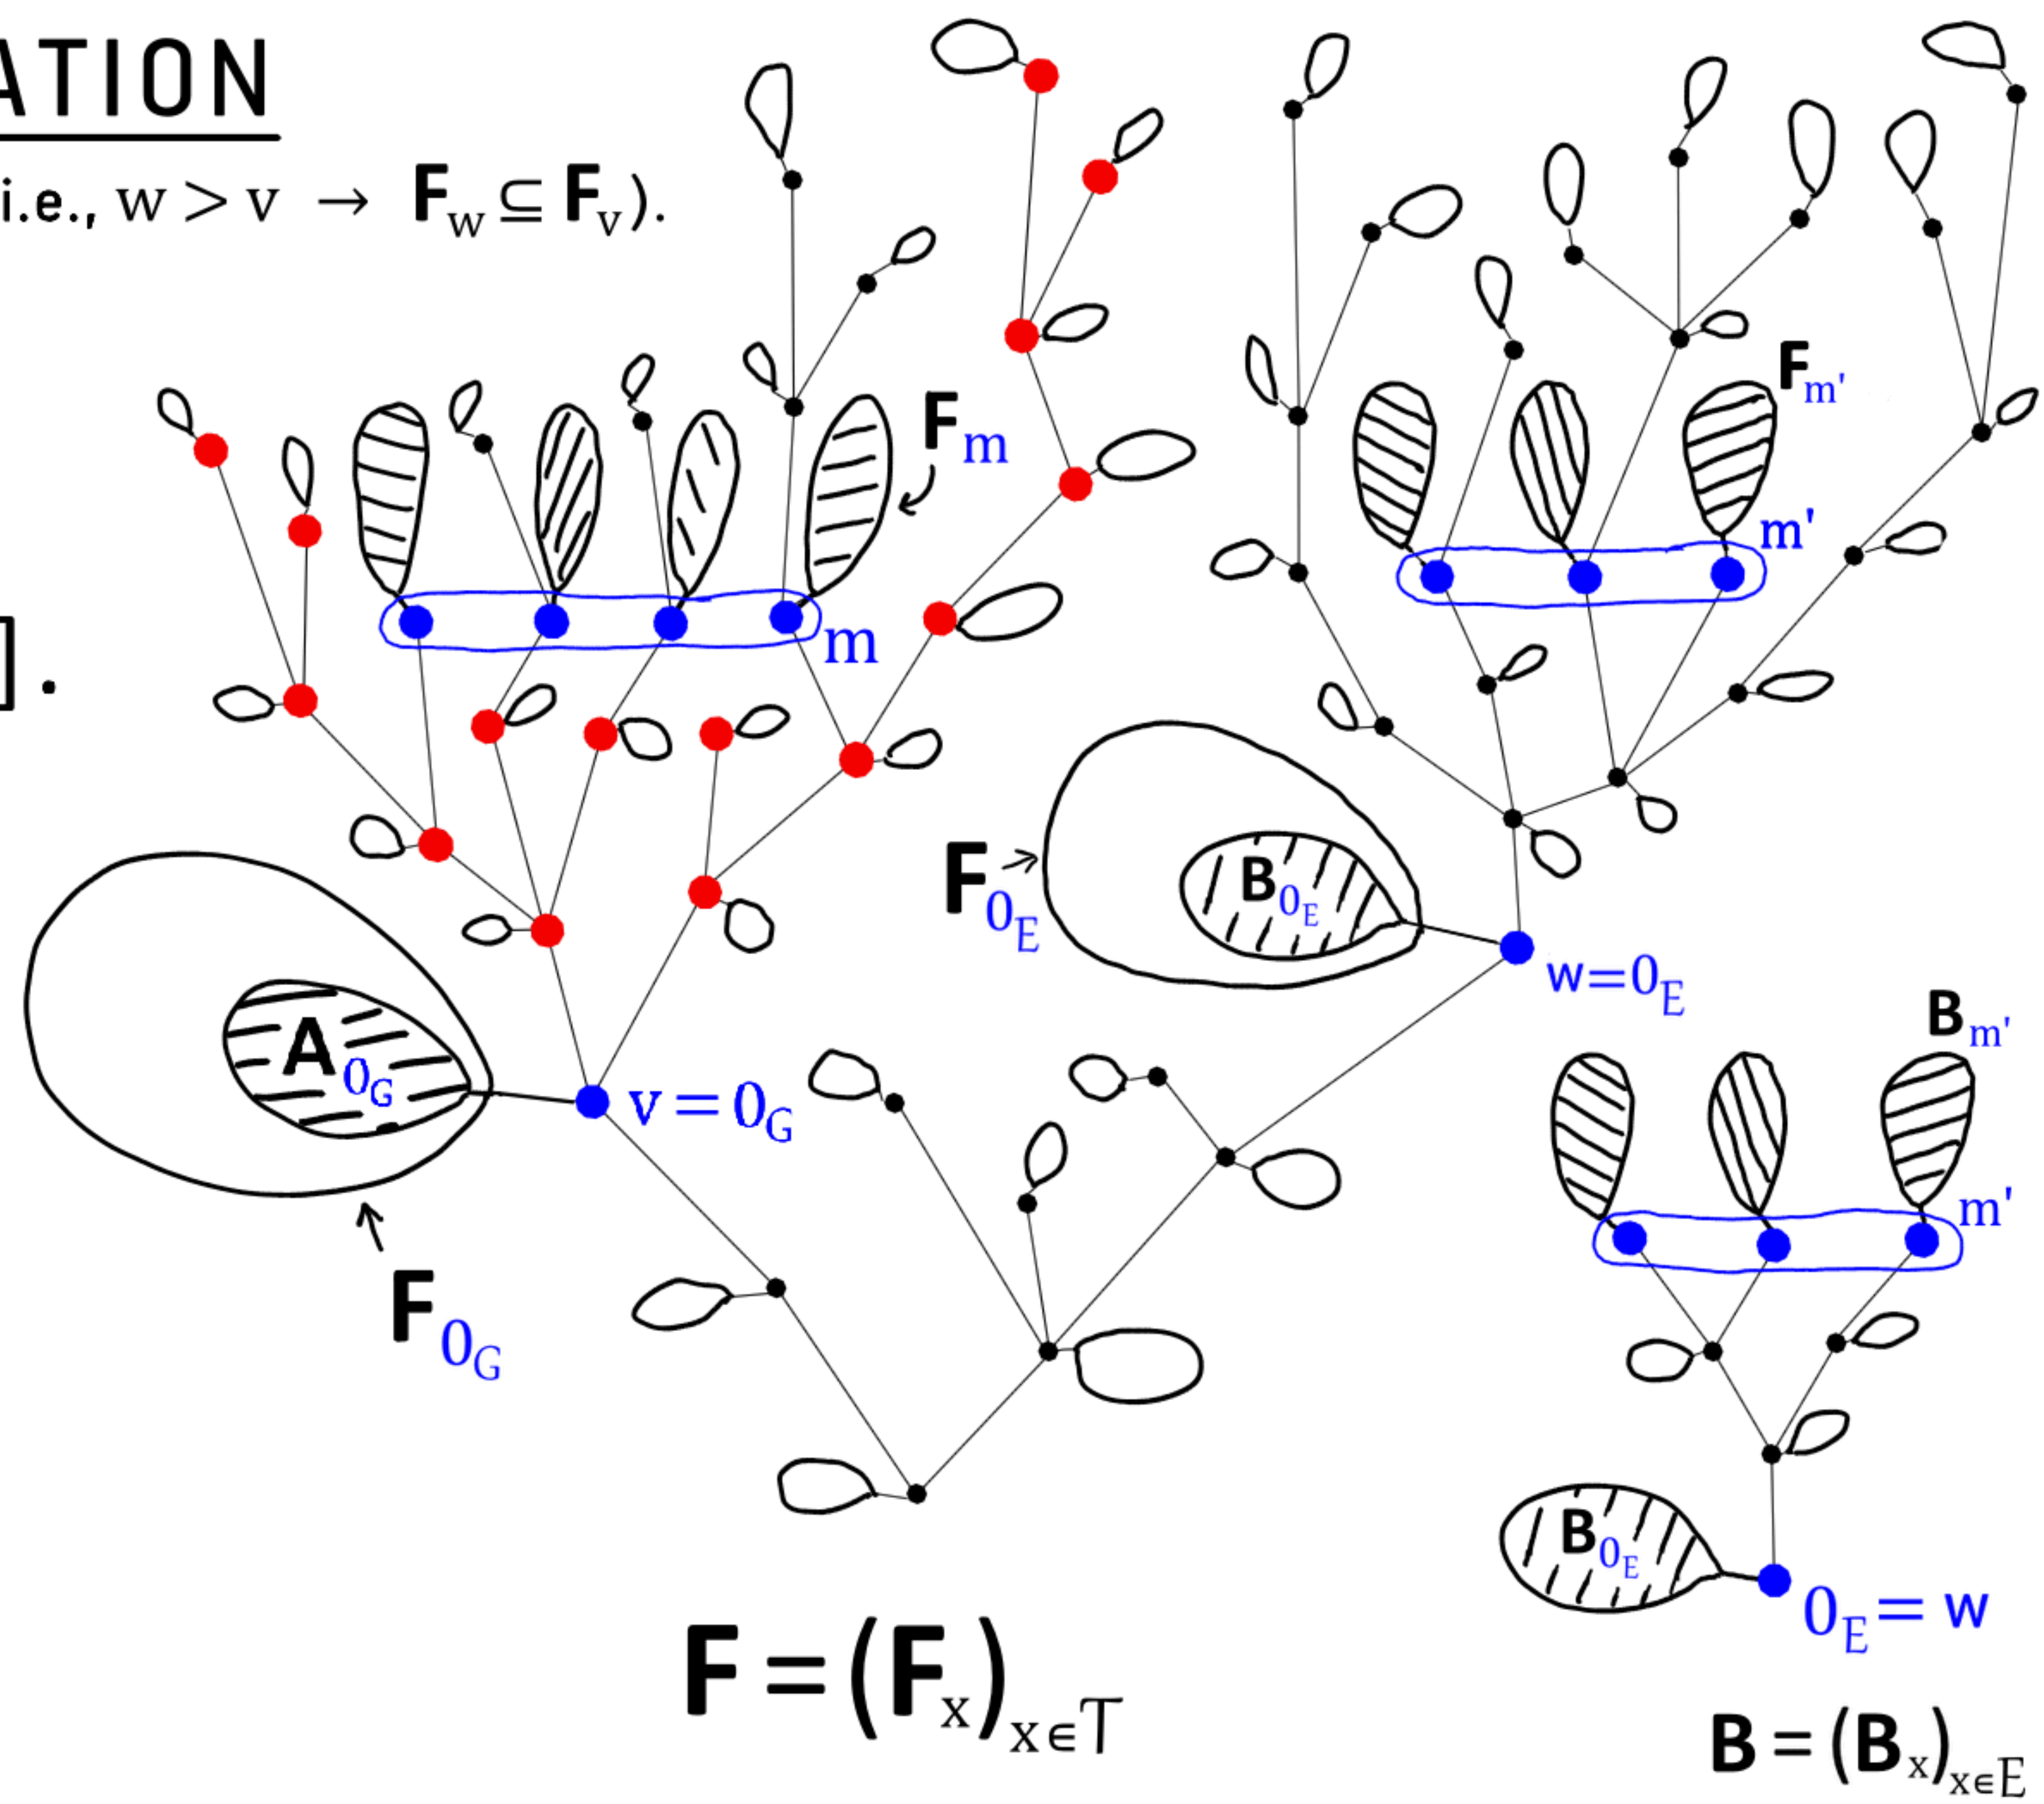



# FOLIAGE HYBRID OPERATION

We consider non-increasing foliage trees (i.e.,  $w > v \rightarrow \mathbf{F}_w \subseteq \mathbf{F}_v$ ).

**A** is a foliage graft for **F** iff

- (1)  $G$  is a graft for  $T$ ;
- (2)  $\mathbf{A}_{0_G} \subseteq \mathbf{F}_{0_G}$ ;
- (3)  $\forall m \in \max G \ [ \mathbf{A}_m = \mathbf{F}_m ]$ .

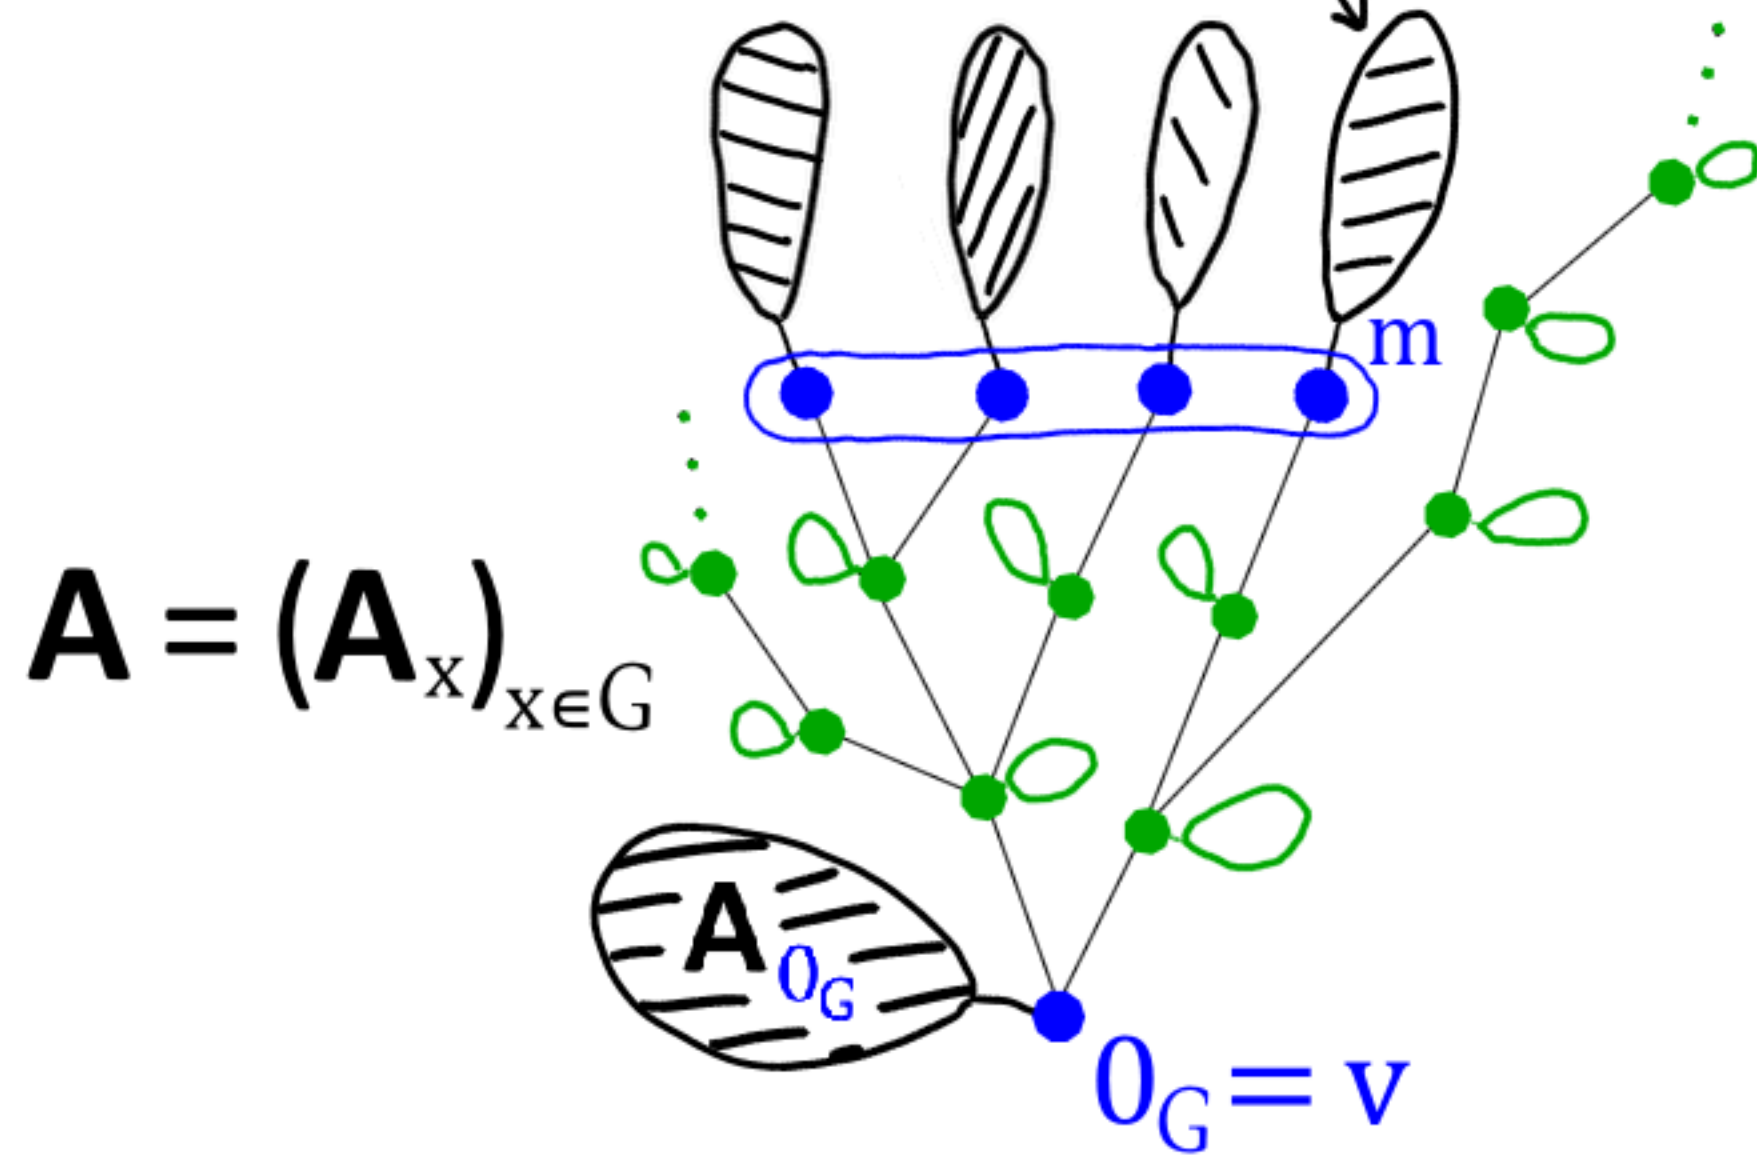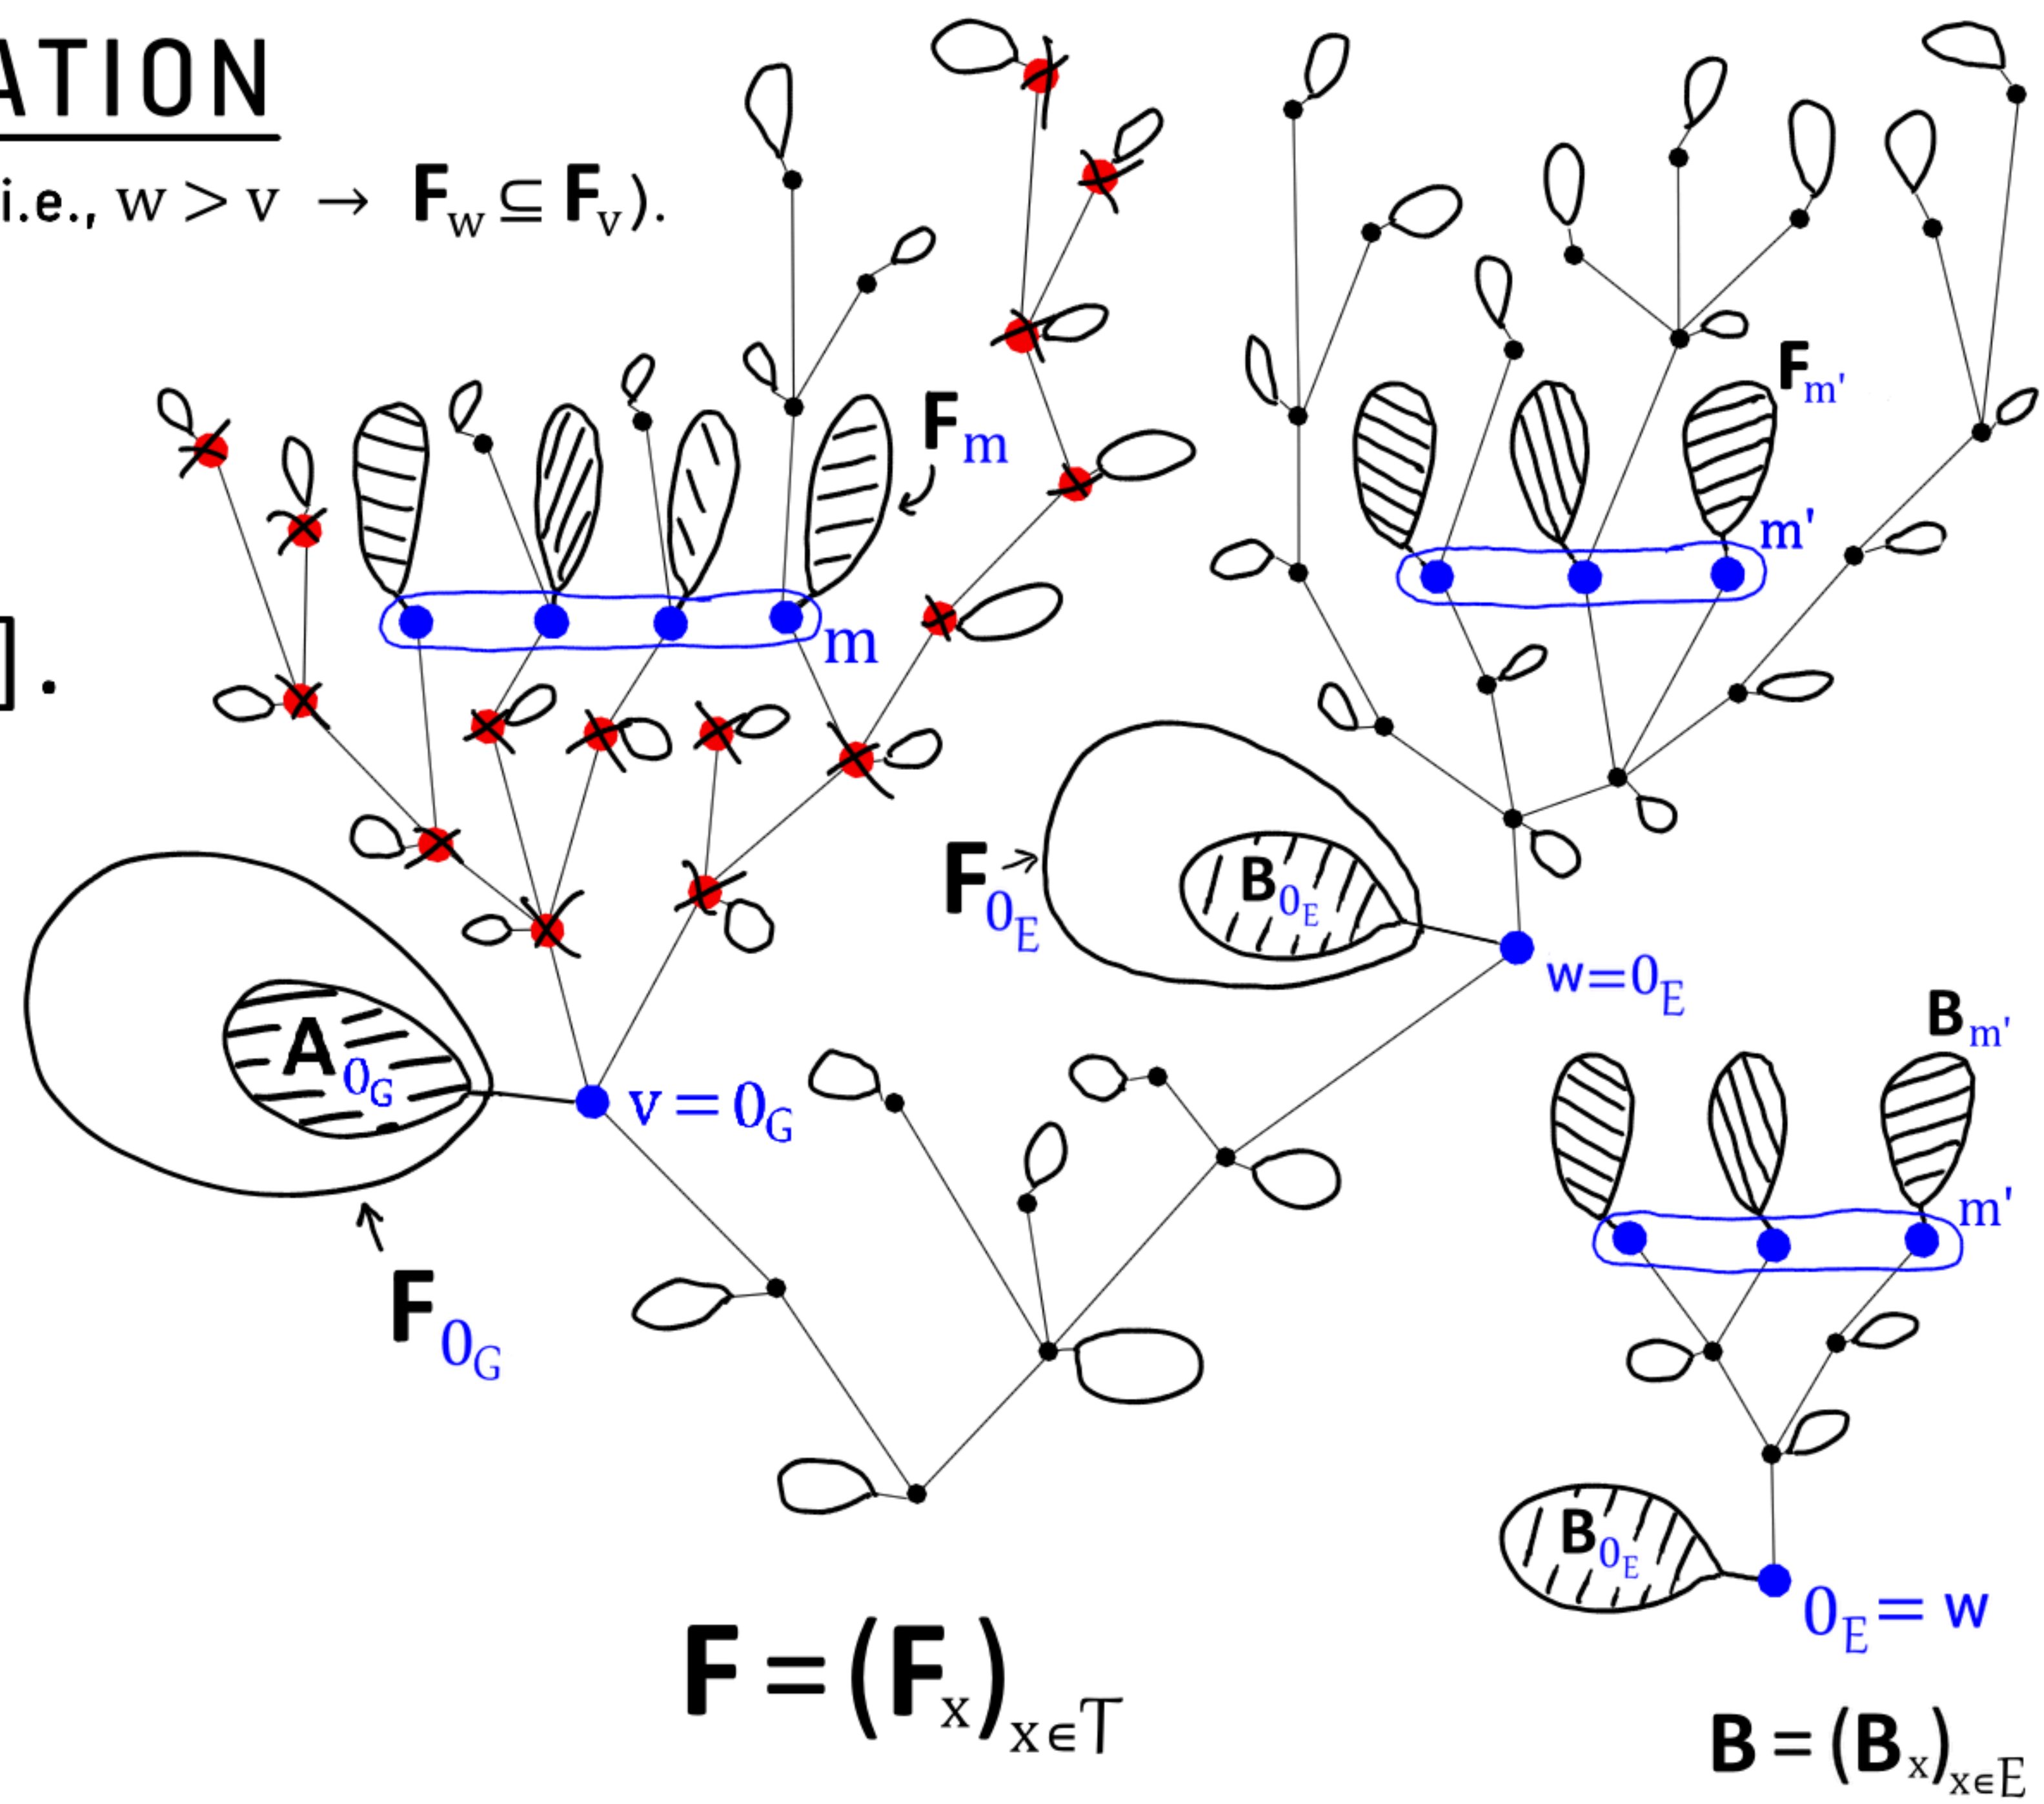



# FOLIAGE HYBRID OPERATION

We consider non-increasing foliage trees (i.e.,  $w > v \rightarrow \mathbf{F}_w \subseteq \mathbf{F}_v$ ).

**A** is a foliage graft for **F** iff

- (1)  $G$  is a graft for  $T$ ;
- (2)  $\mathbf{A}_{0_G} \subseteq \mathbf{F}_{0_G}$ ;
- (3)  $\forall m \in \max G \ [ \mathbf{A}_m = \mathbf{F}_m ]$ .

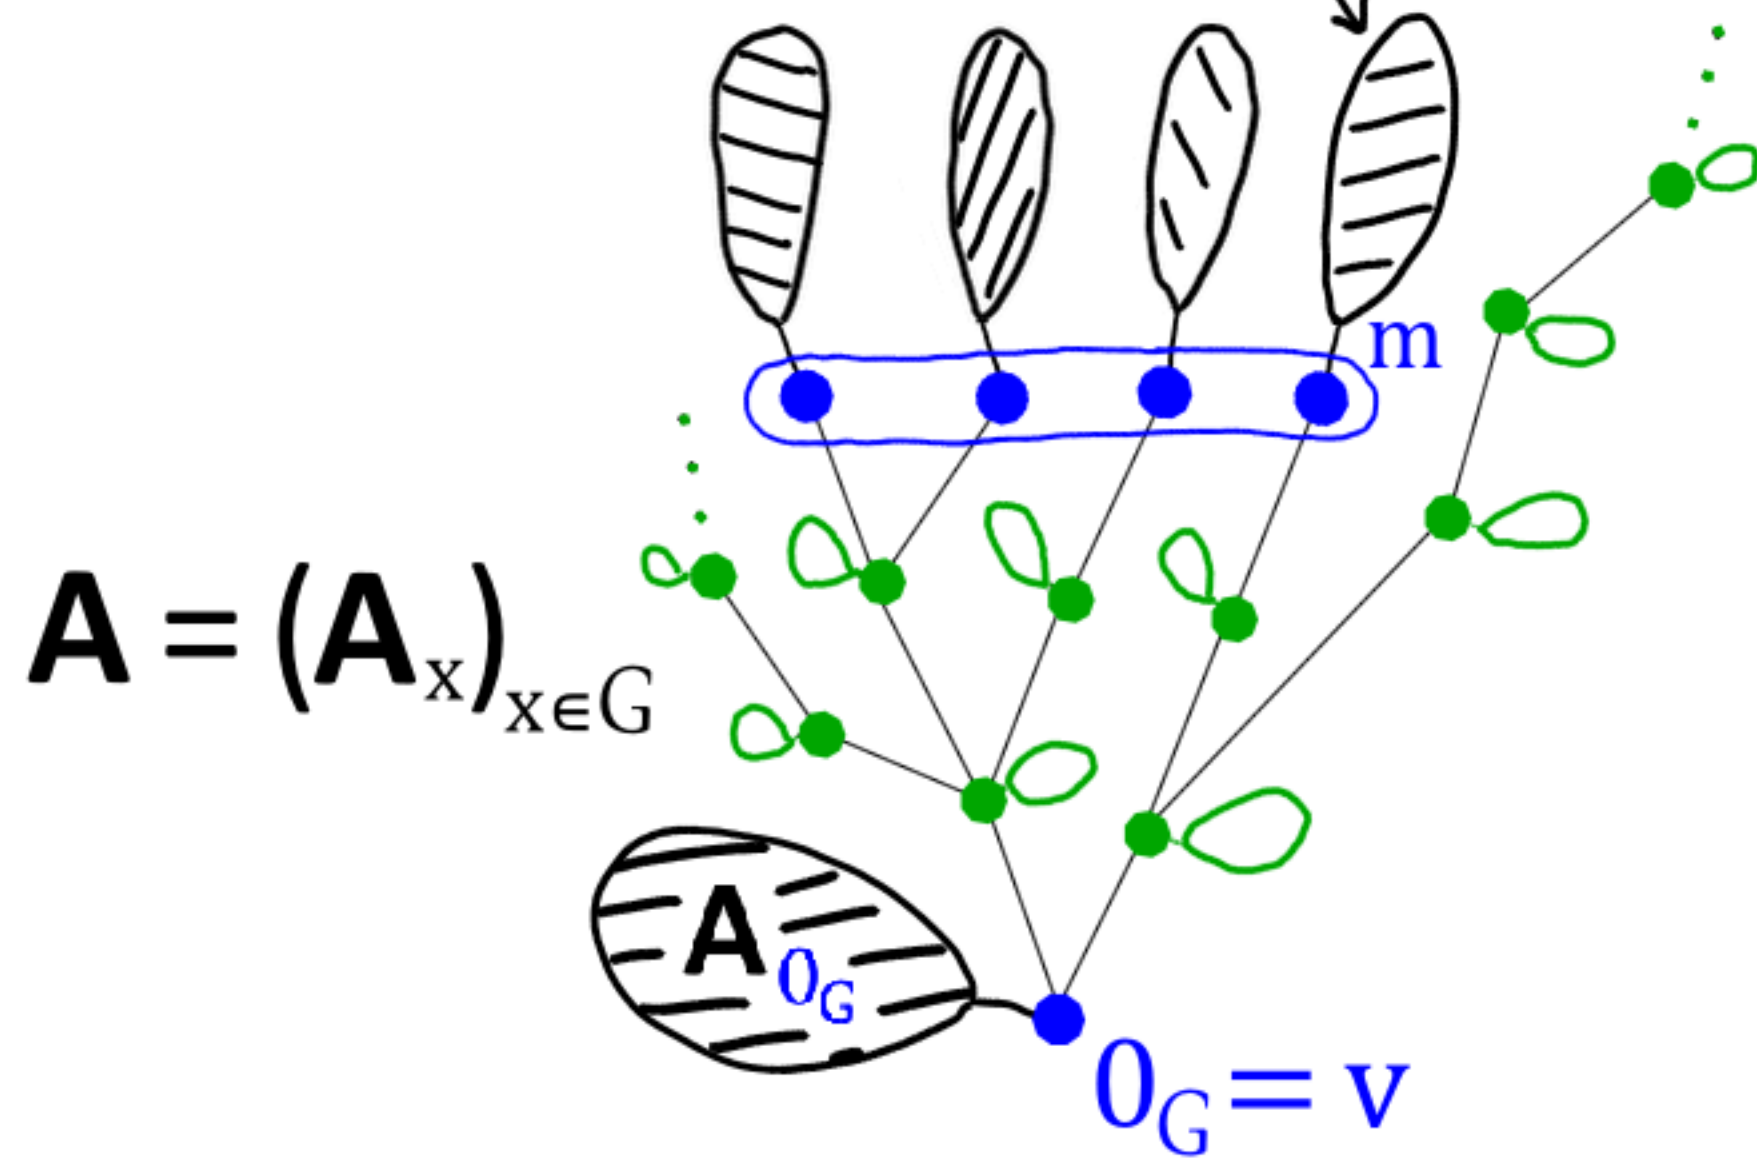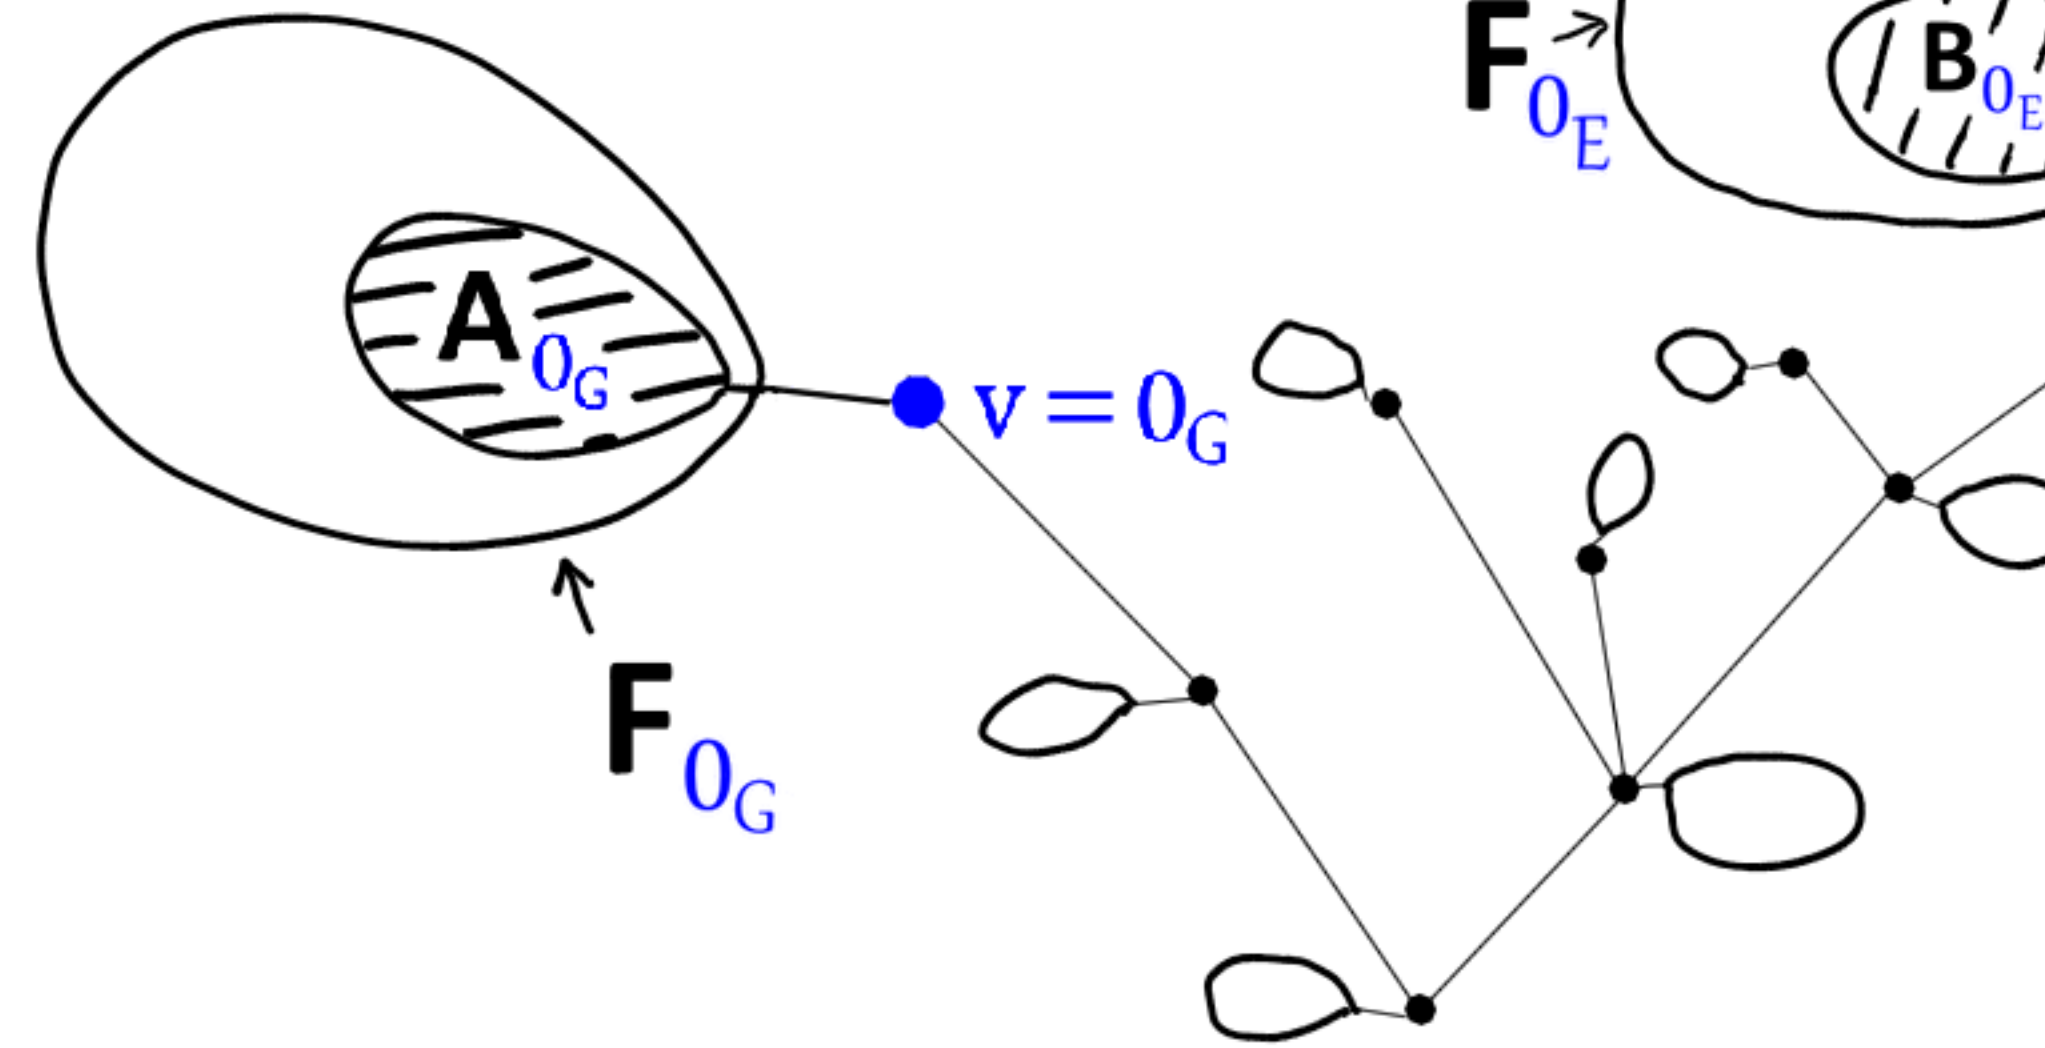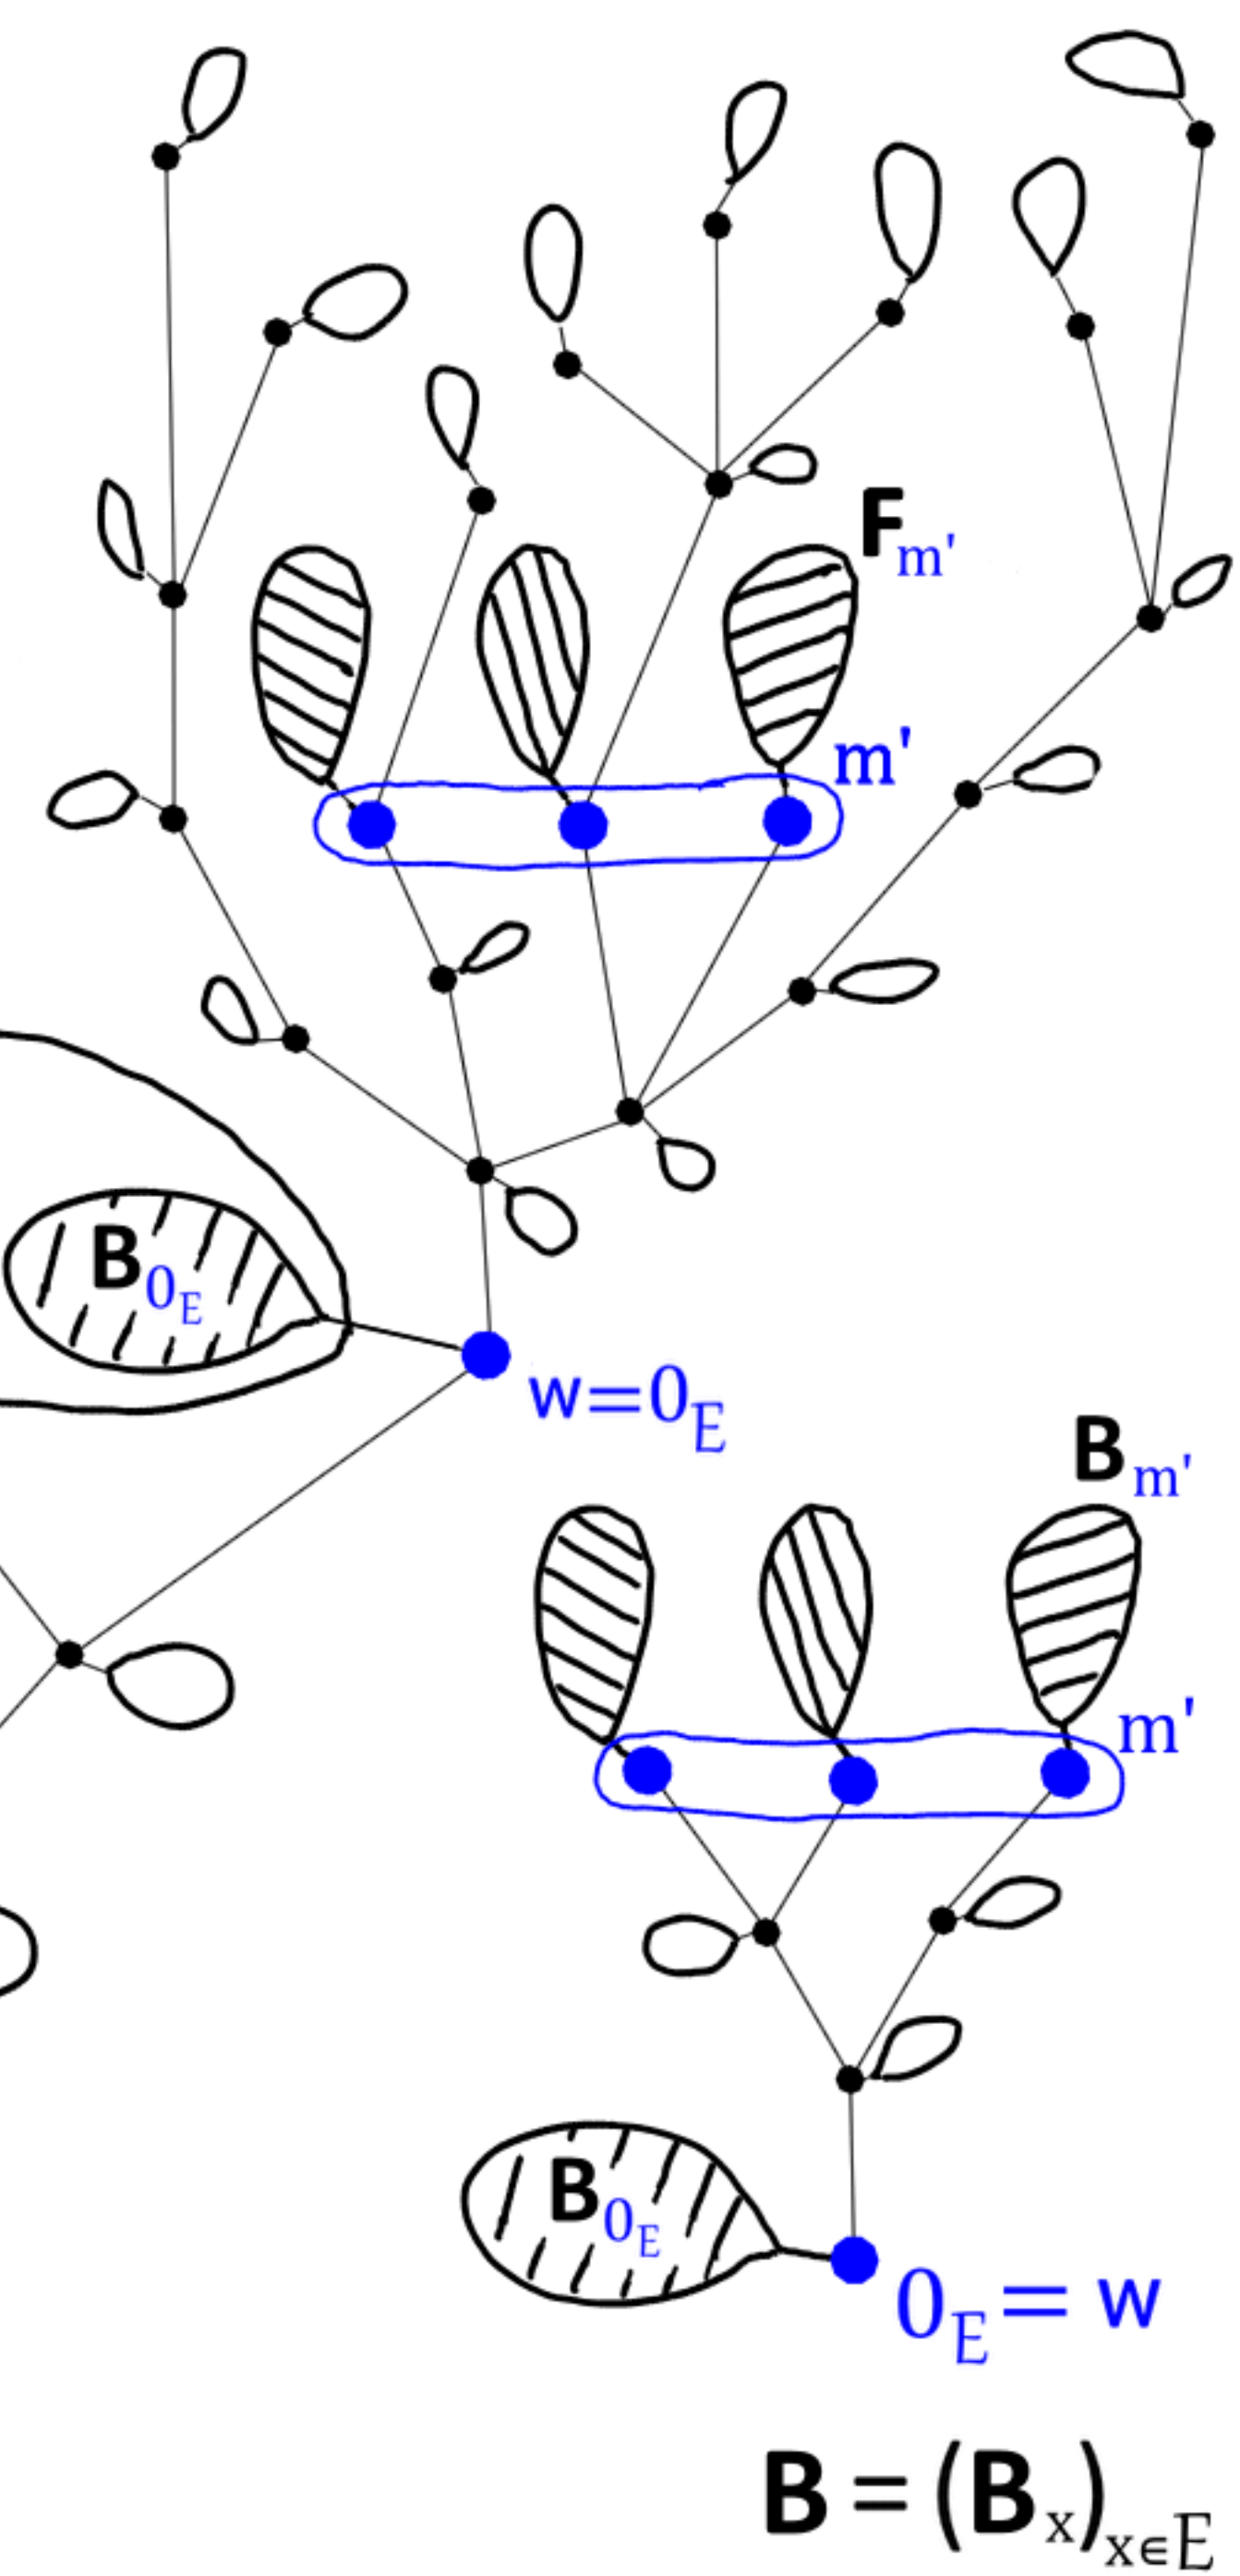



# FOLIAGE HYBRID OPERATION

We consider non-increasing foliage trees (i.e.,  $w > v \rightarrow \mathbf{F}_w \subseteq \mathbf{F}_v$ ).

**A** is a foliage graft for **F** iff

- (1)  $G$  is a graft for  $T$ ;
- (2)  $\mathbf{A}_{0_G} \subseteq \mathbf{F}_{0_G}$ ;
- (3)  $\forall m \in \max G \ [ \mathbf{A}_m = \mathbf{F}_m ]$ .

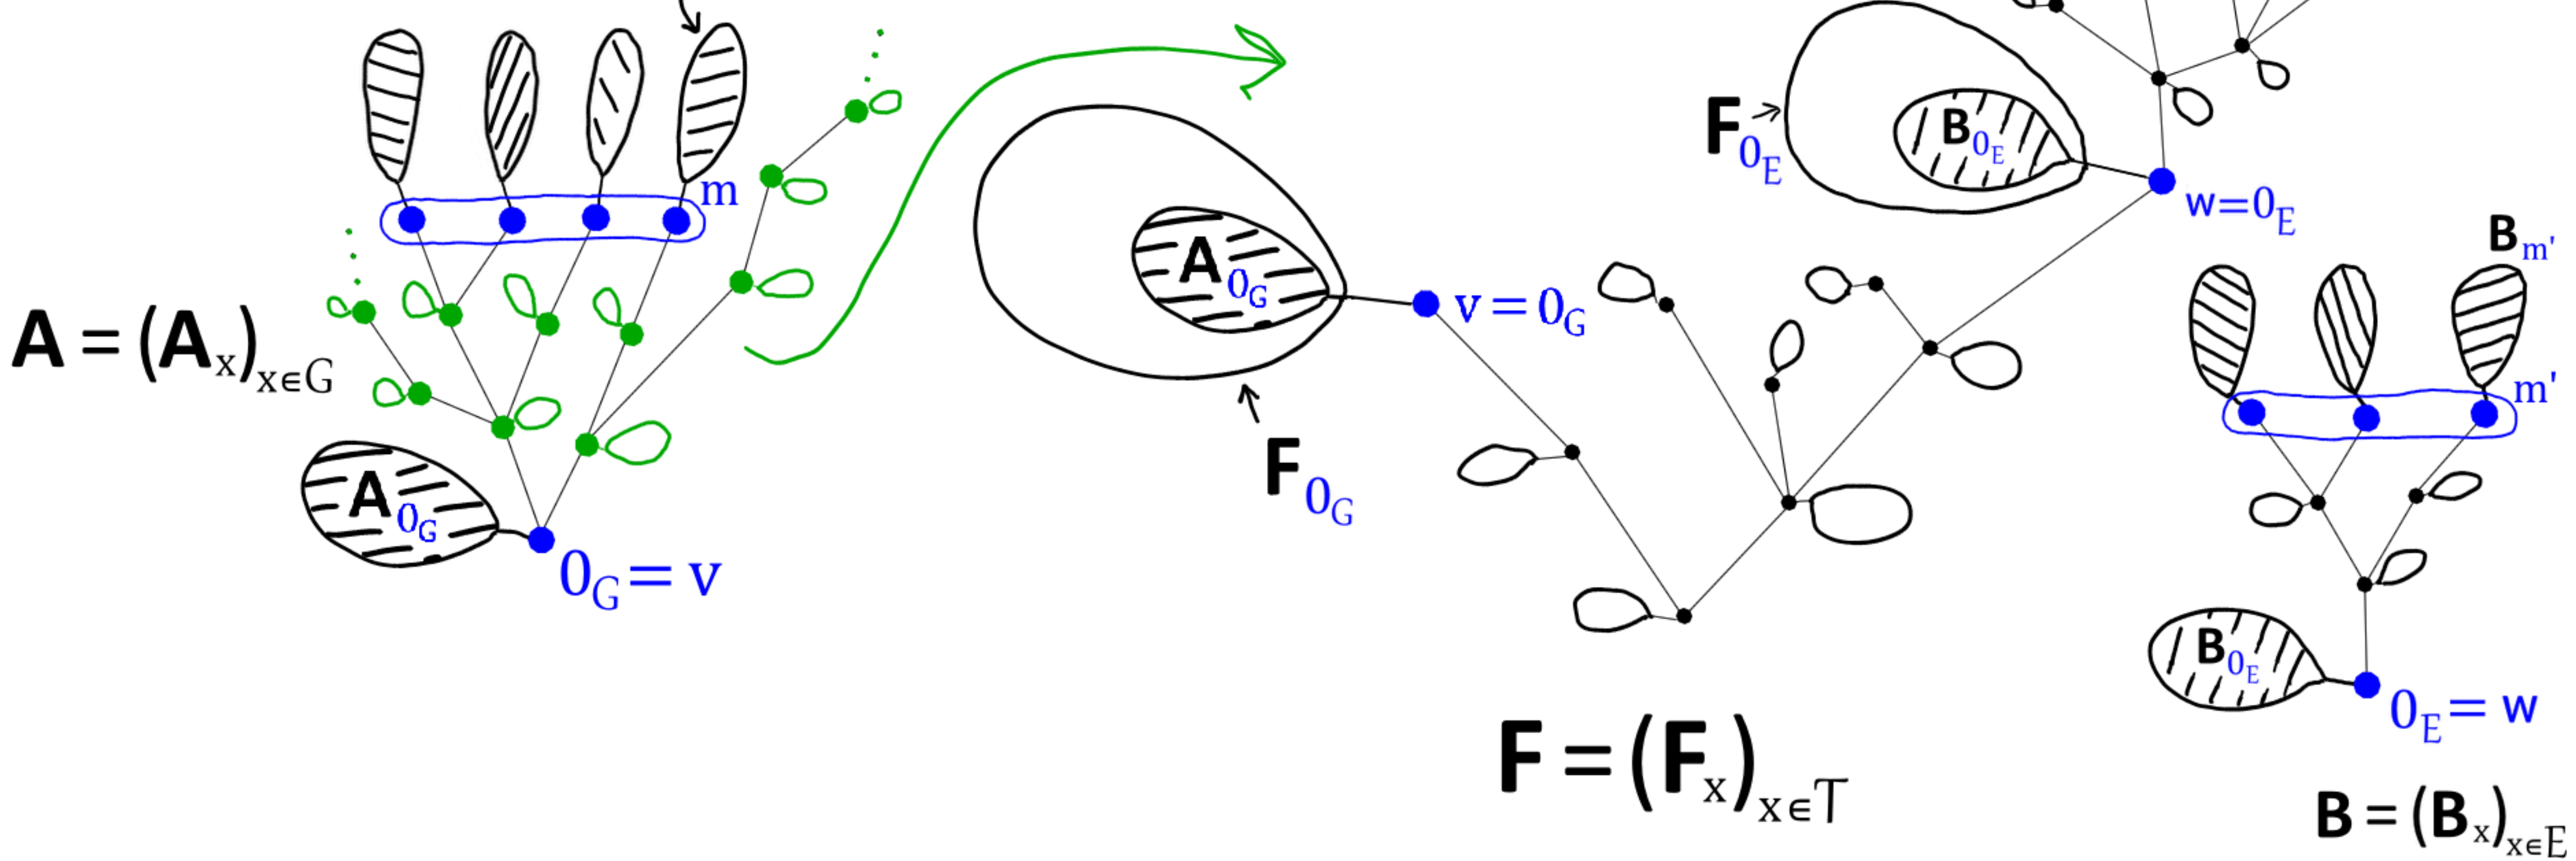



# FOLIAGE HYBRID OPERATION

We consider non-increasing foliage trees (i.e.,  $w > v \rightarrow \mathbf{F}_w \subseteq \mathbf{F}_v$ ).

**A** is a foliage graft for **F** iff

- (1)  $G$  is a graft for  $T$ ;
- (2)  $\mathbf{A}_{0_G} \subseteq \mathbf{F}_{0_G}$ ;
- (3)  $\forall m \in \max G \ [ \mathbf{A}_m = \mathbf{F}_m ]$ .

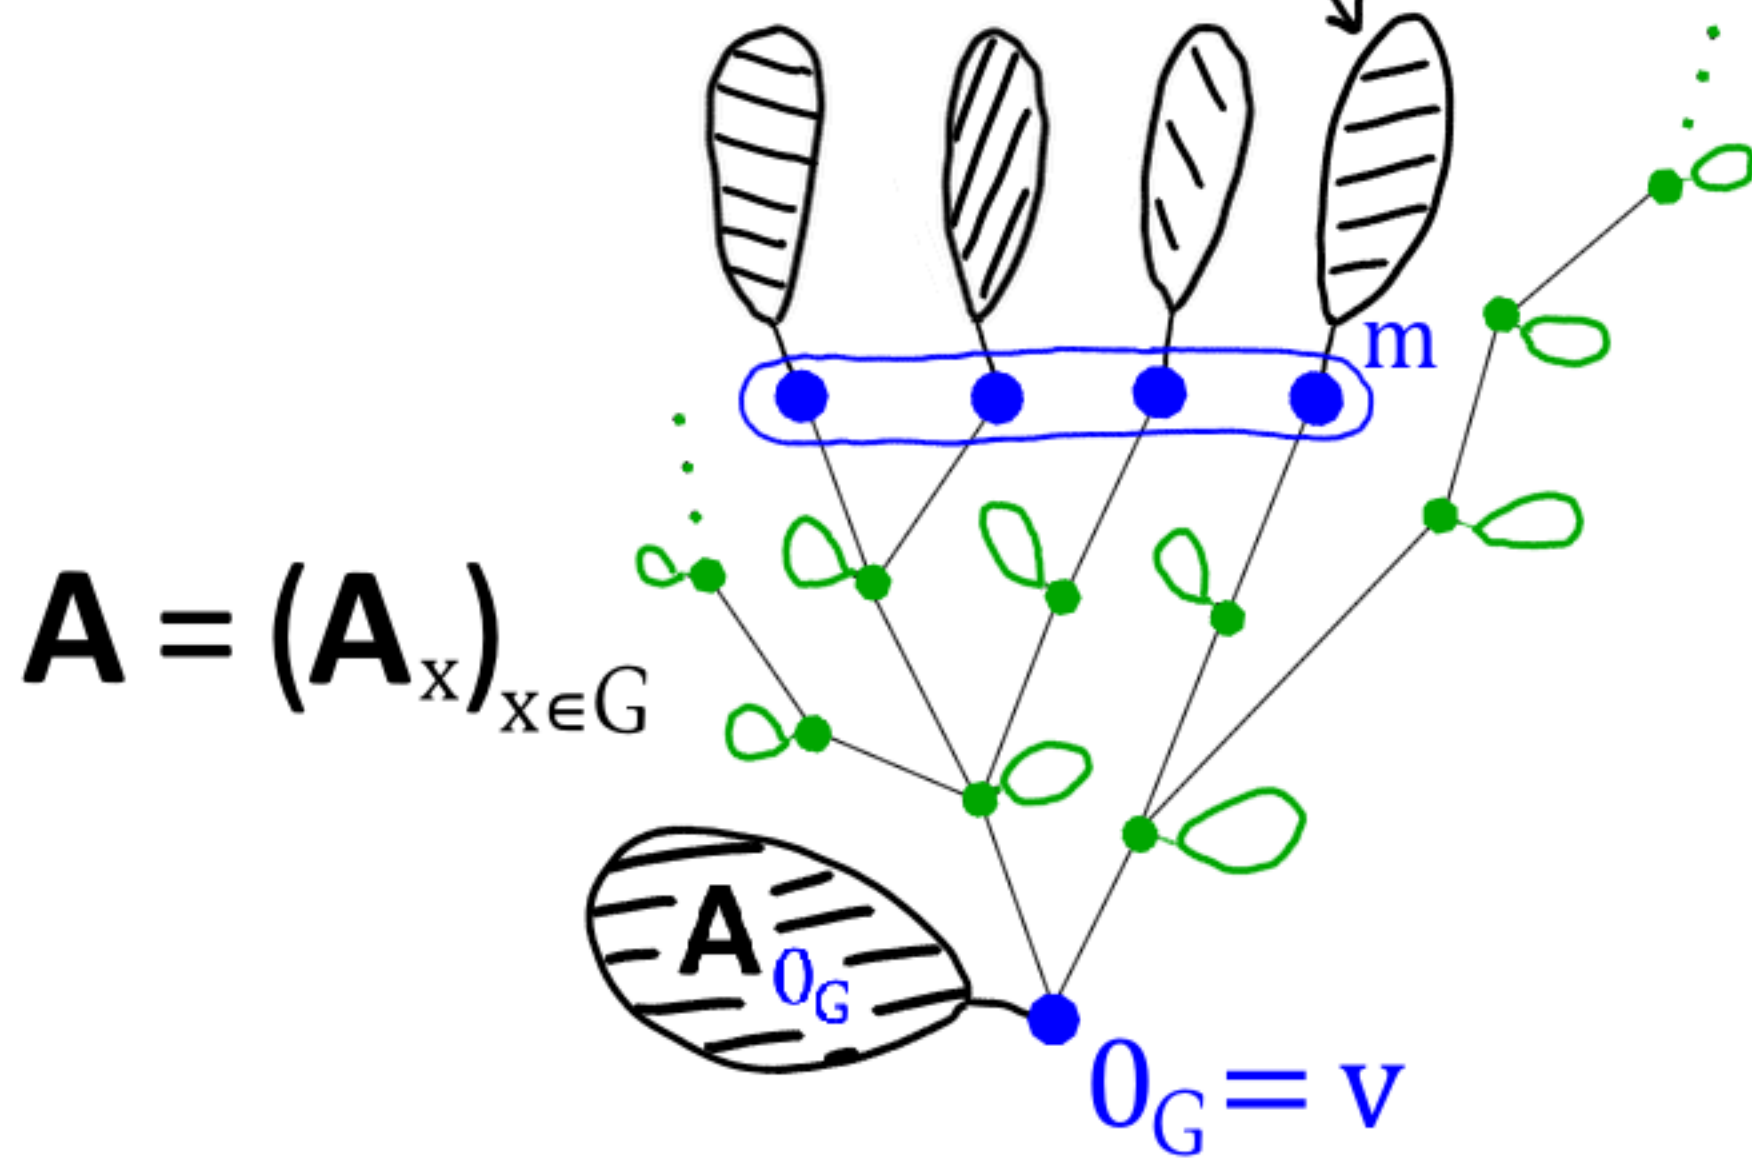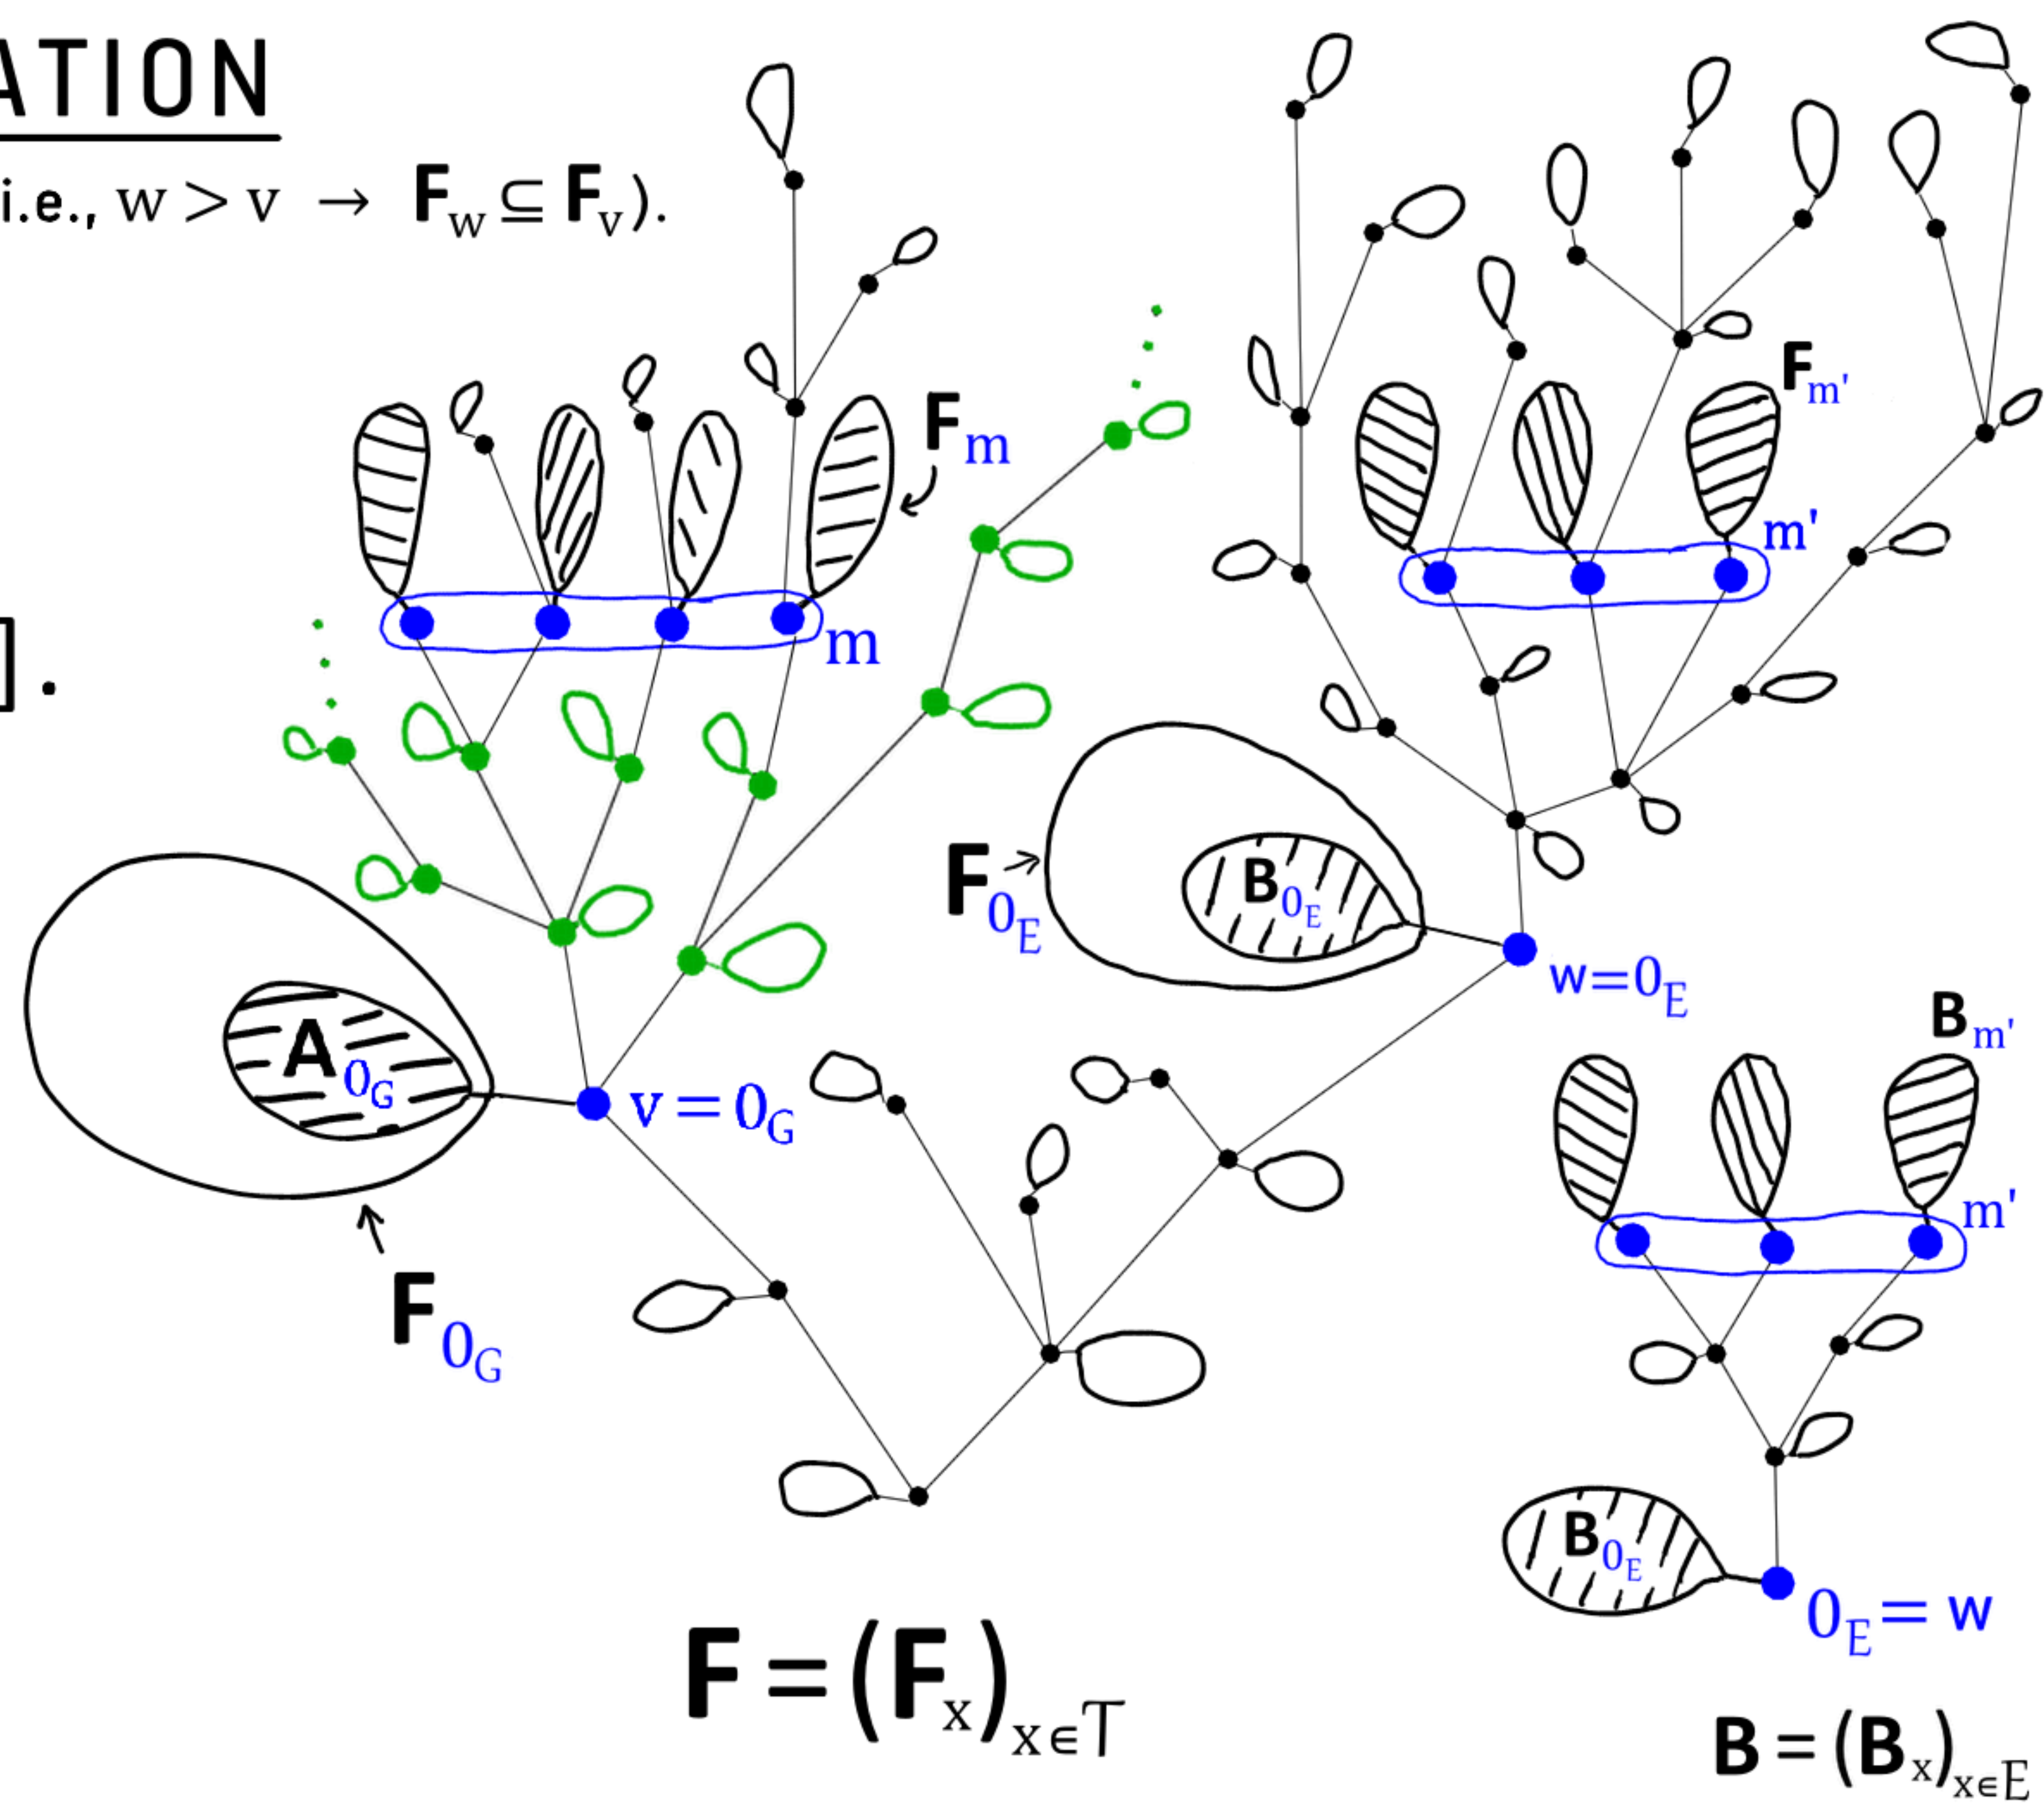



## FOLIAGE HYBRID OPERATION

We consider non-increasing foliage trees (i.e.,  $w > v \rightarrow \mathbf{F}_w \subseteq \mathbf{F}_v$ ).

**A** is a foliage graft for **F** iff

- (1)  $G$  is a graft for  $T$ ;
- (2)  $\mathbf{A}_{0_G} \subseteq \mathbf{F}_{0_G}$ ;
- (3)  $\forall m \in \max G \ [ \mathbf{A}_m = \mathbf{F}_m ]$ .

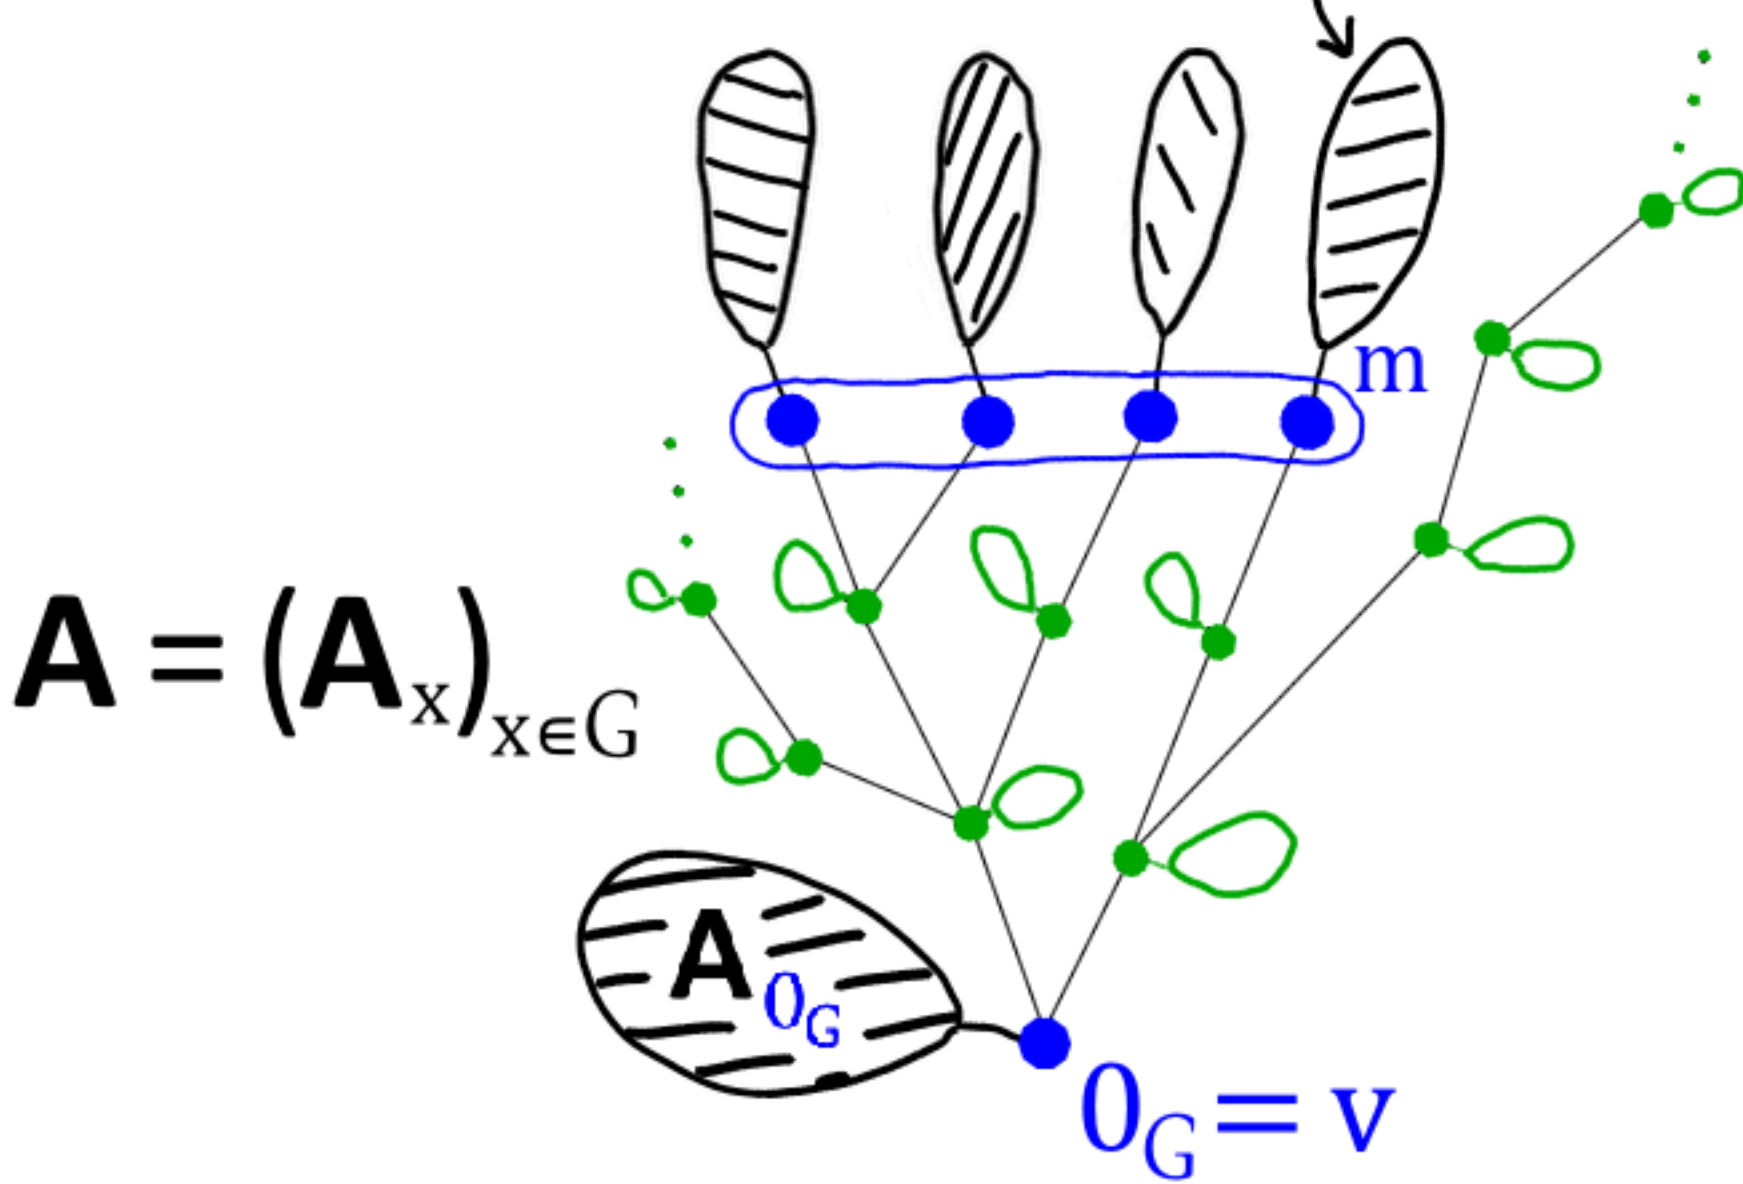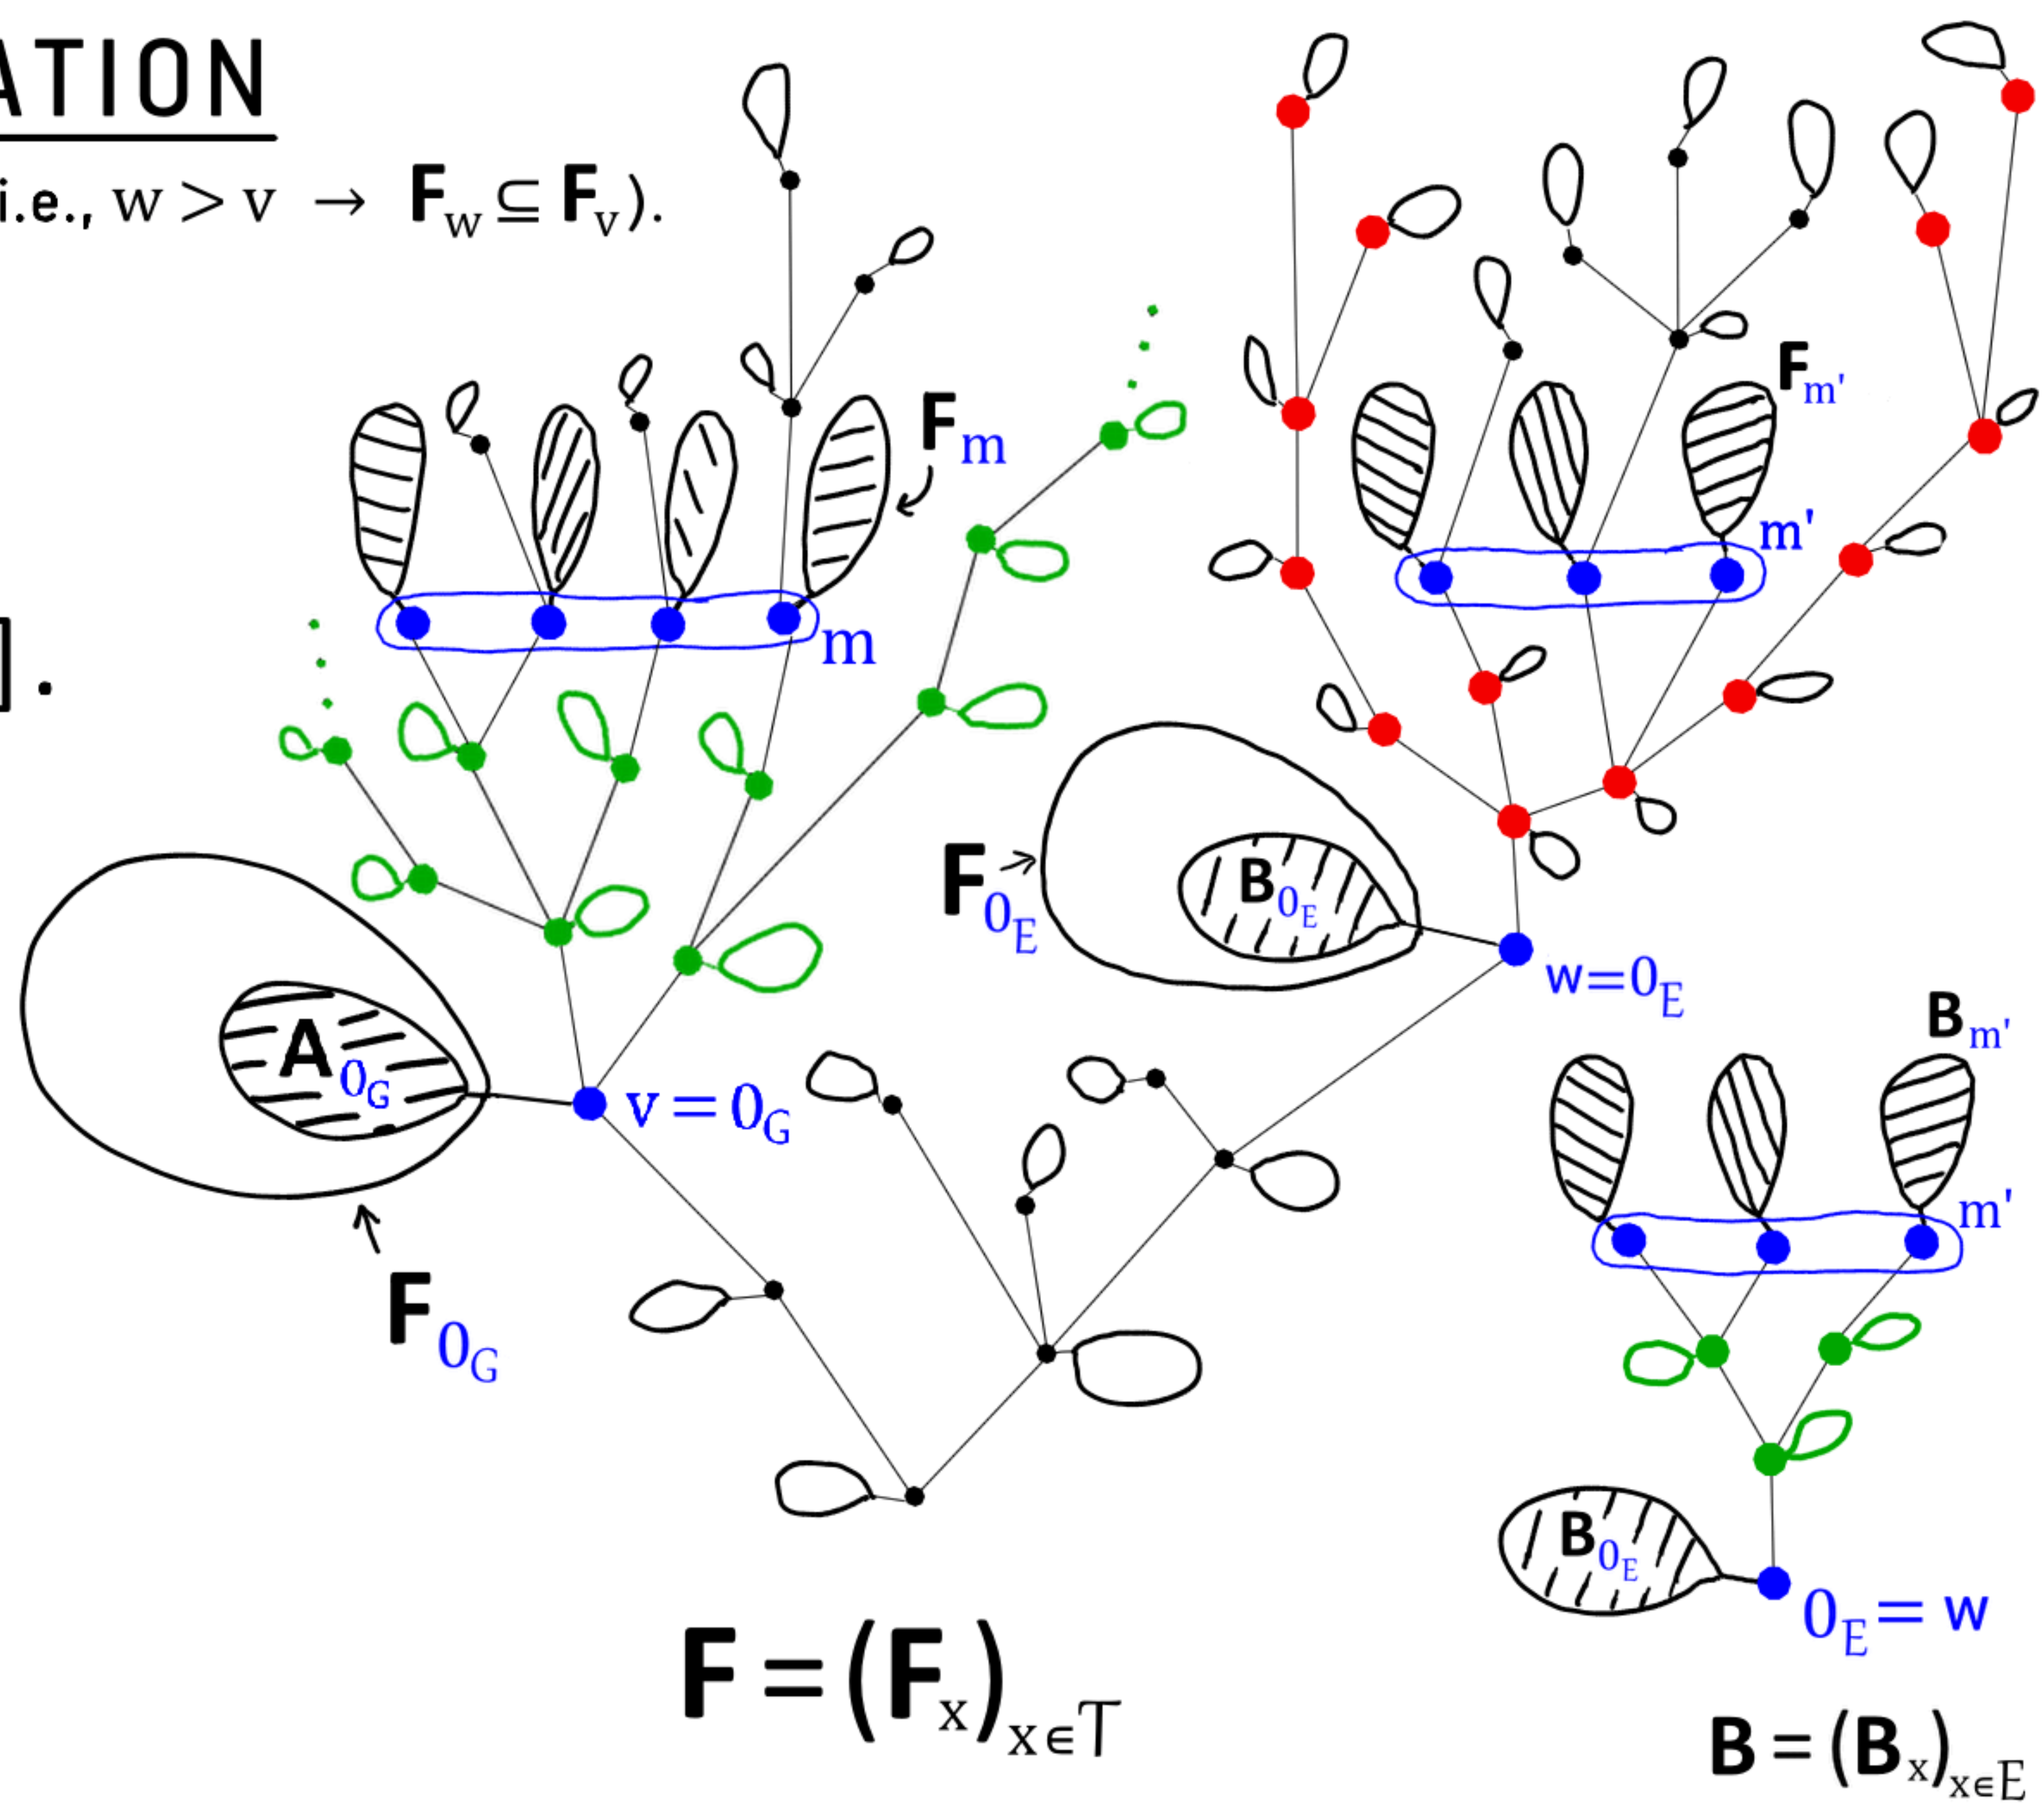



# FOLIAGE HYBRID OPERATION

We consider non-increasing foliage trees (i.e.,  $w > v \rightarrow \mathbf{F}_w \subseteq \mathbf{F}_v$ ).

**A** is a foliage graft for **F** iff

- (1)  $G$  is a graft for  $T$ ;
- (2)  $\mathbf{A}_{0_G} \subseteq \mathbf{F}_{0_G}$ ;
- (3)  $\forall m \in \max G \ [ \mathbf{A}_m = \mathbf{F}_m ]$ .

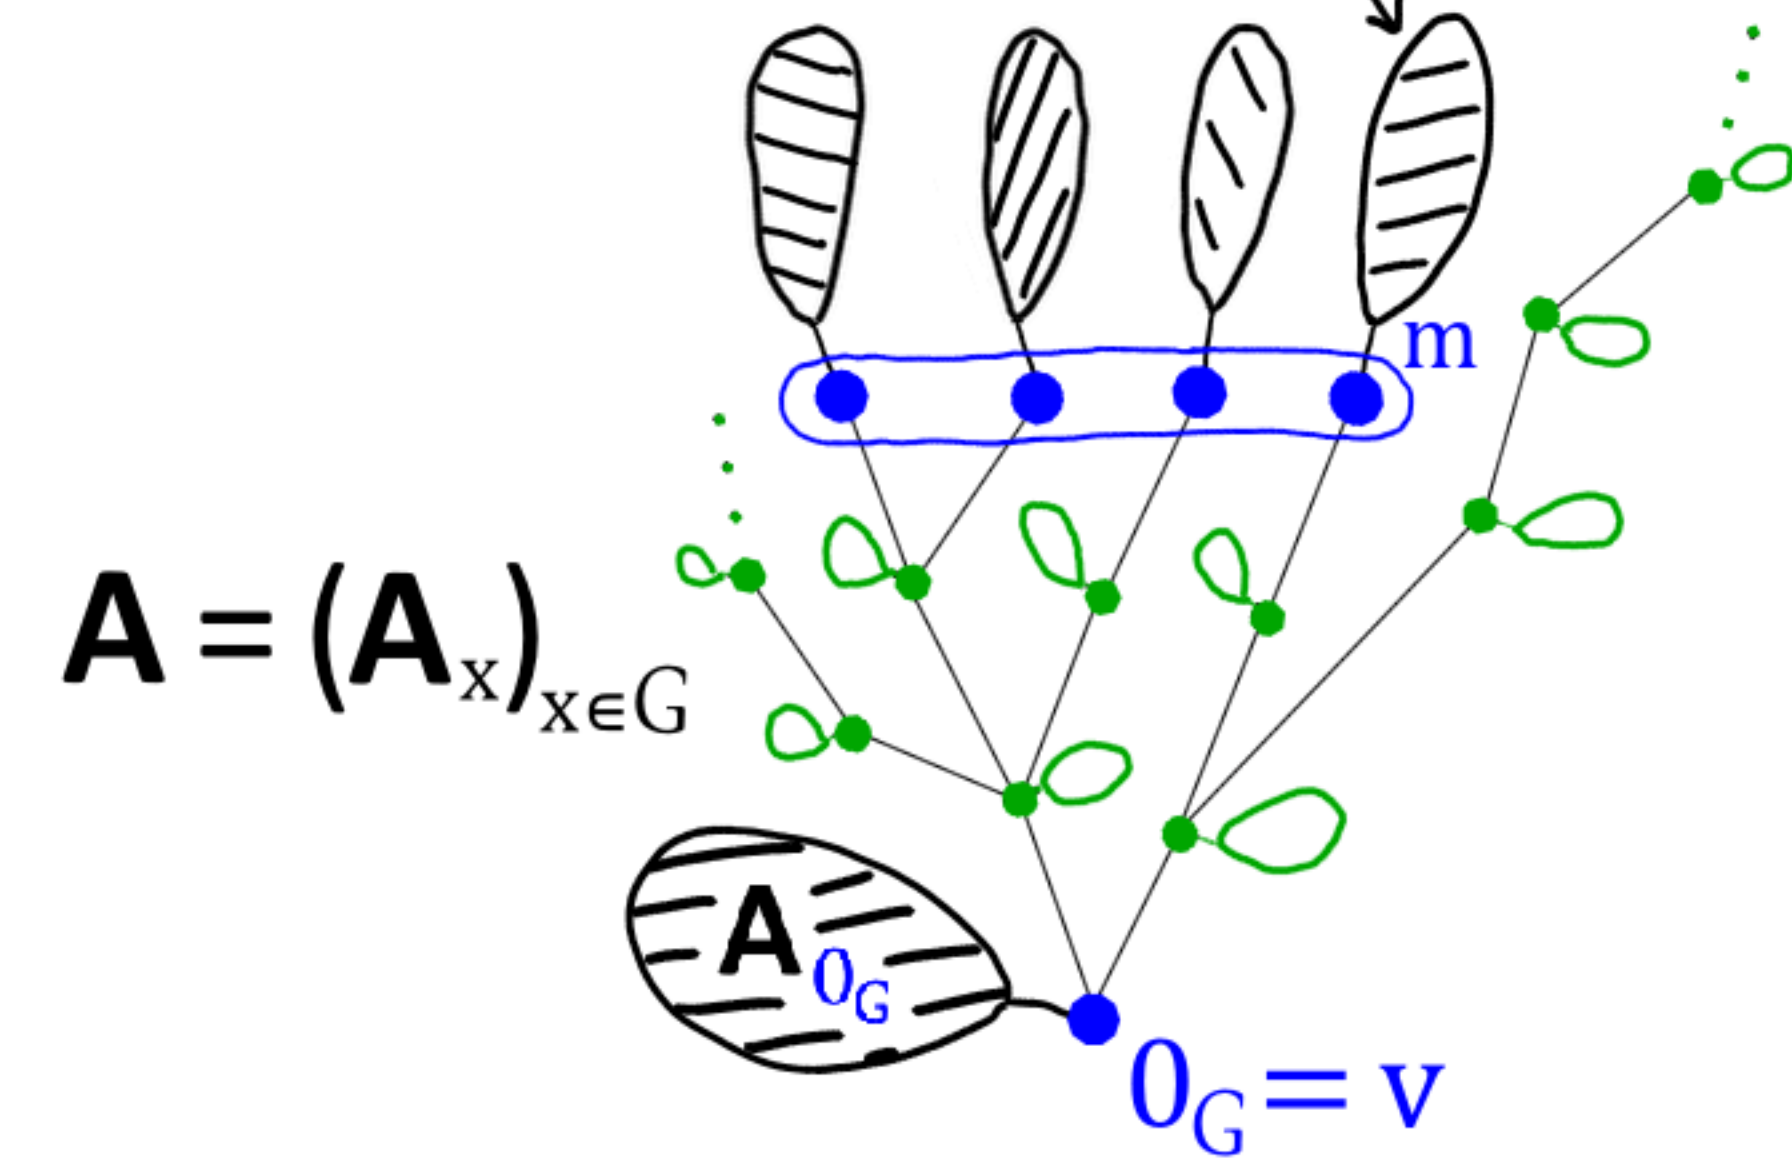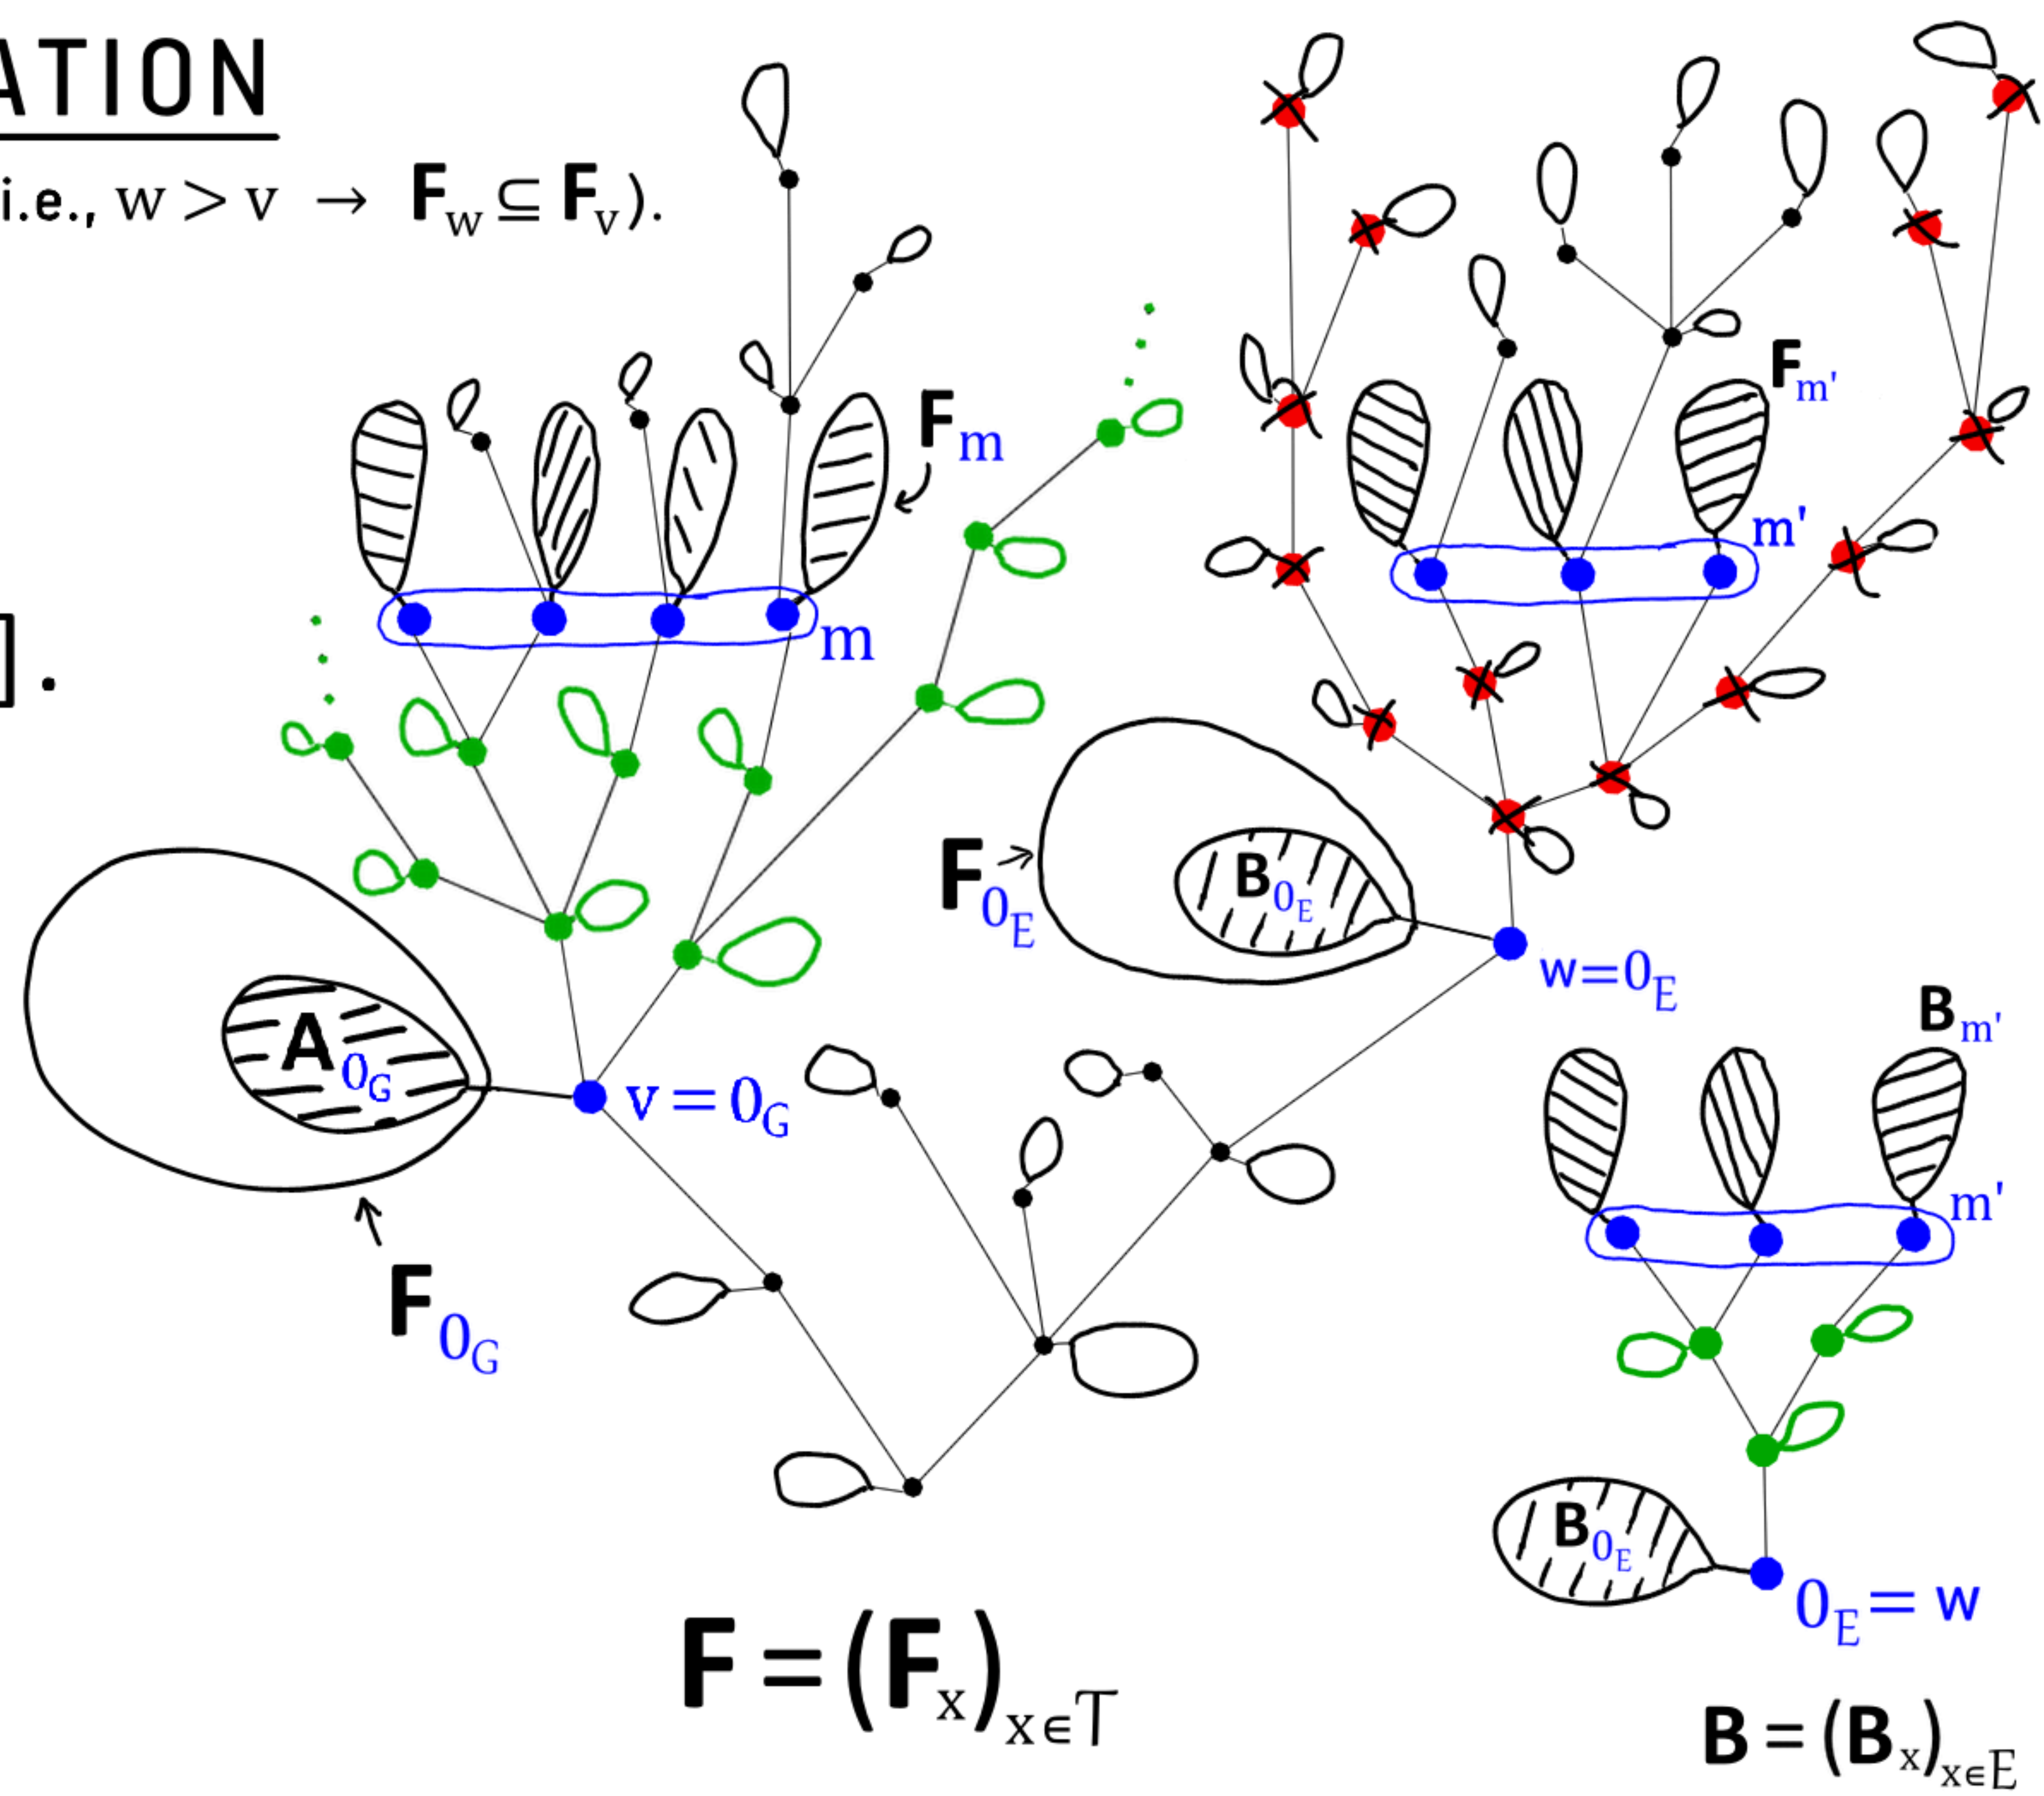



# FOLIAGE HYBRID OPERATION

We consider non-increasing foliage trees (i.e.,  $w > v \rightarrow \mathbf{F}_w \subseteq \mathbf{F}_v$ ).

**A** is a foliage graft for **F** iff

- (1)  $G$  is a graft for  $T$ ;
- (2)  $\mathbf{A}_{0_G} \subseteq \mathbf{F}_{0_G}$ ;
- (3)  $\forall m \in \max G \ [ \mathbf{A}_m = \mathbf{F}_m ]$ .

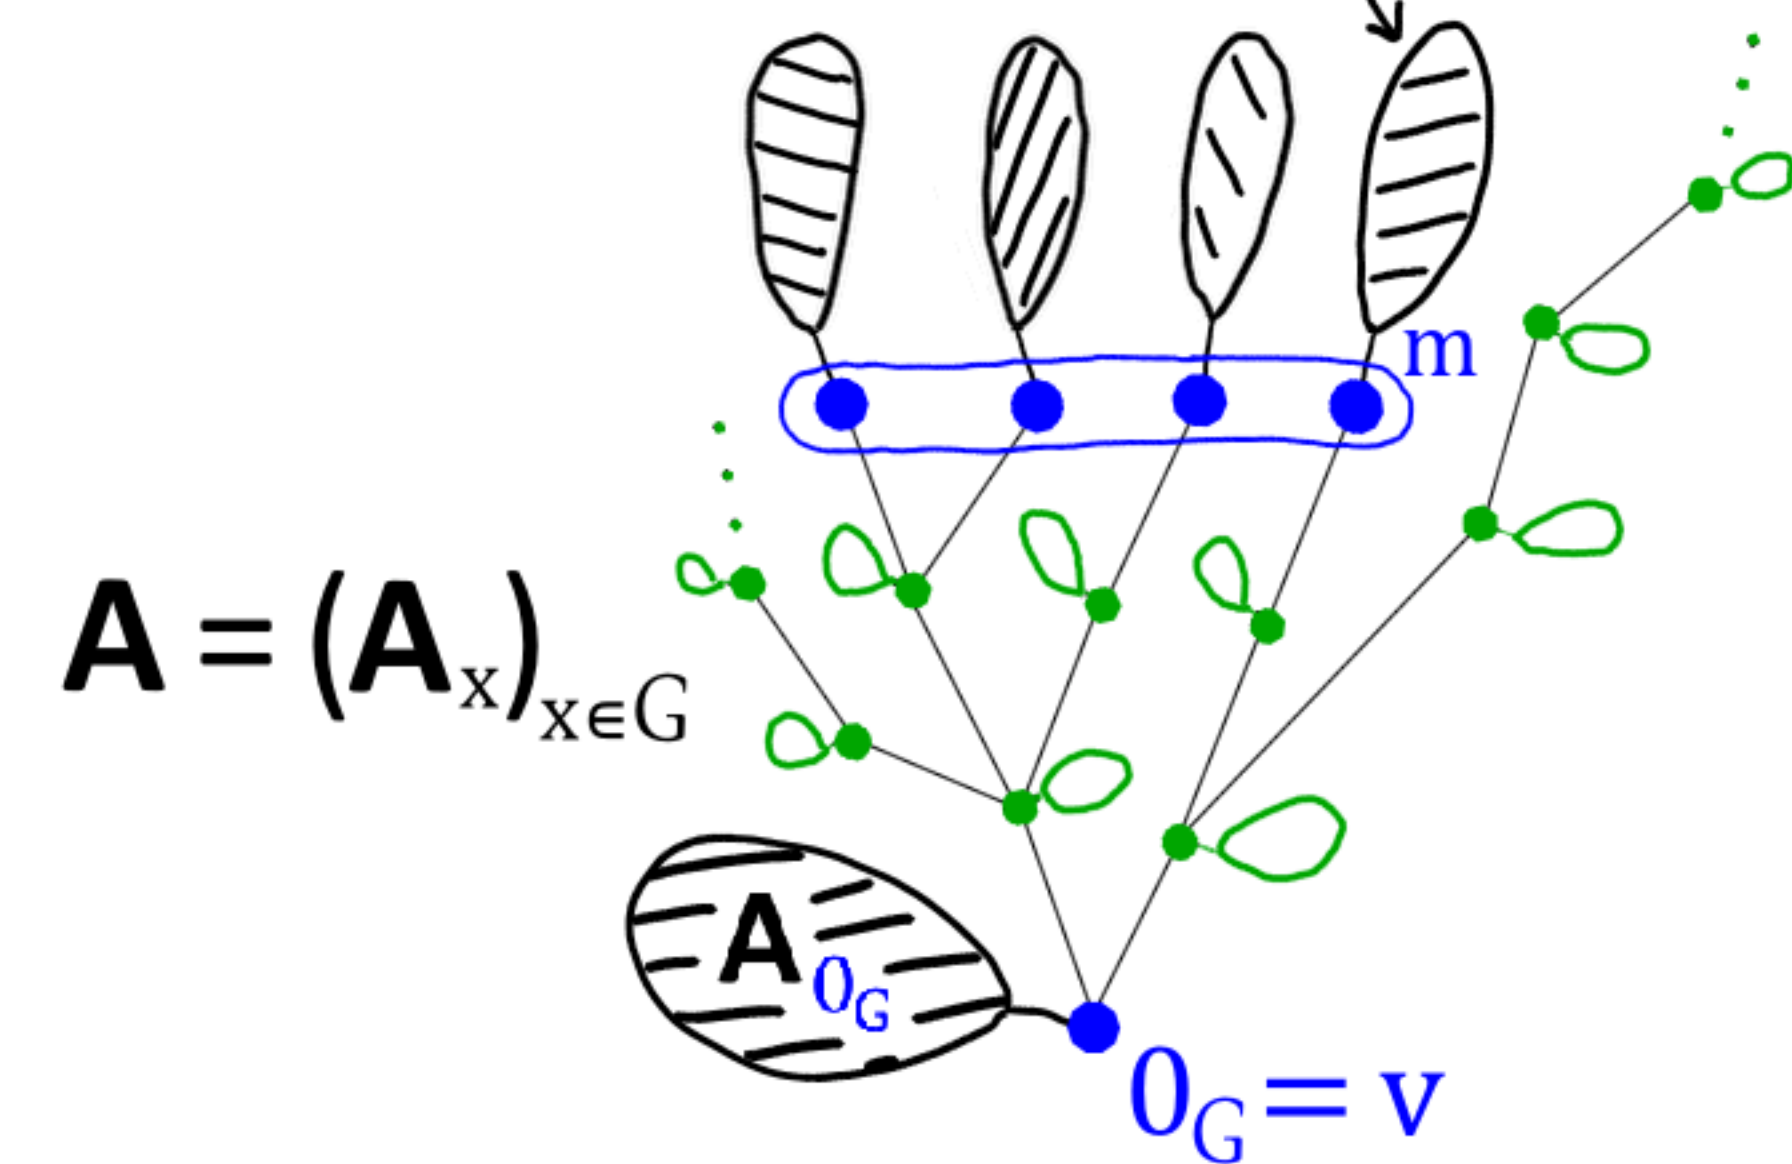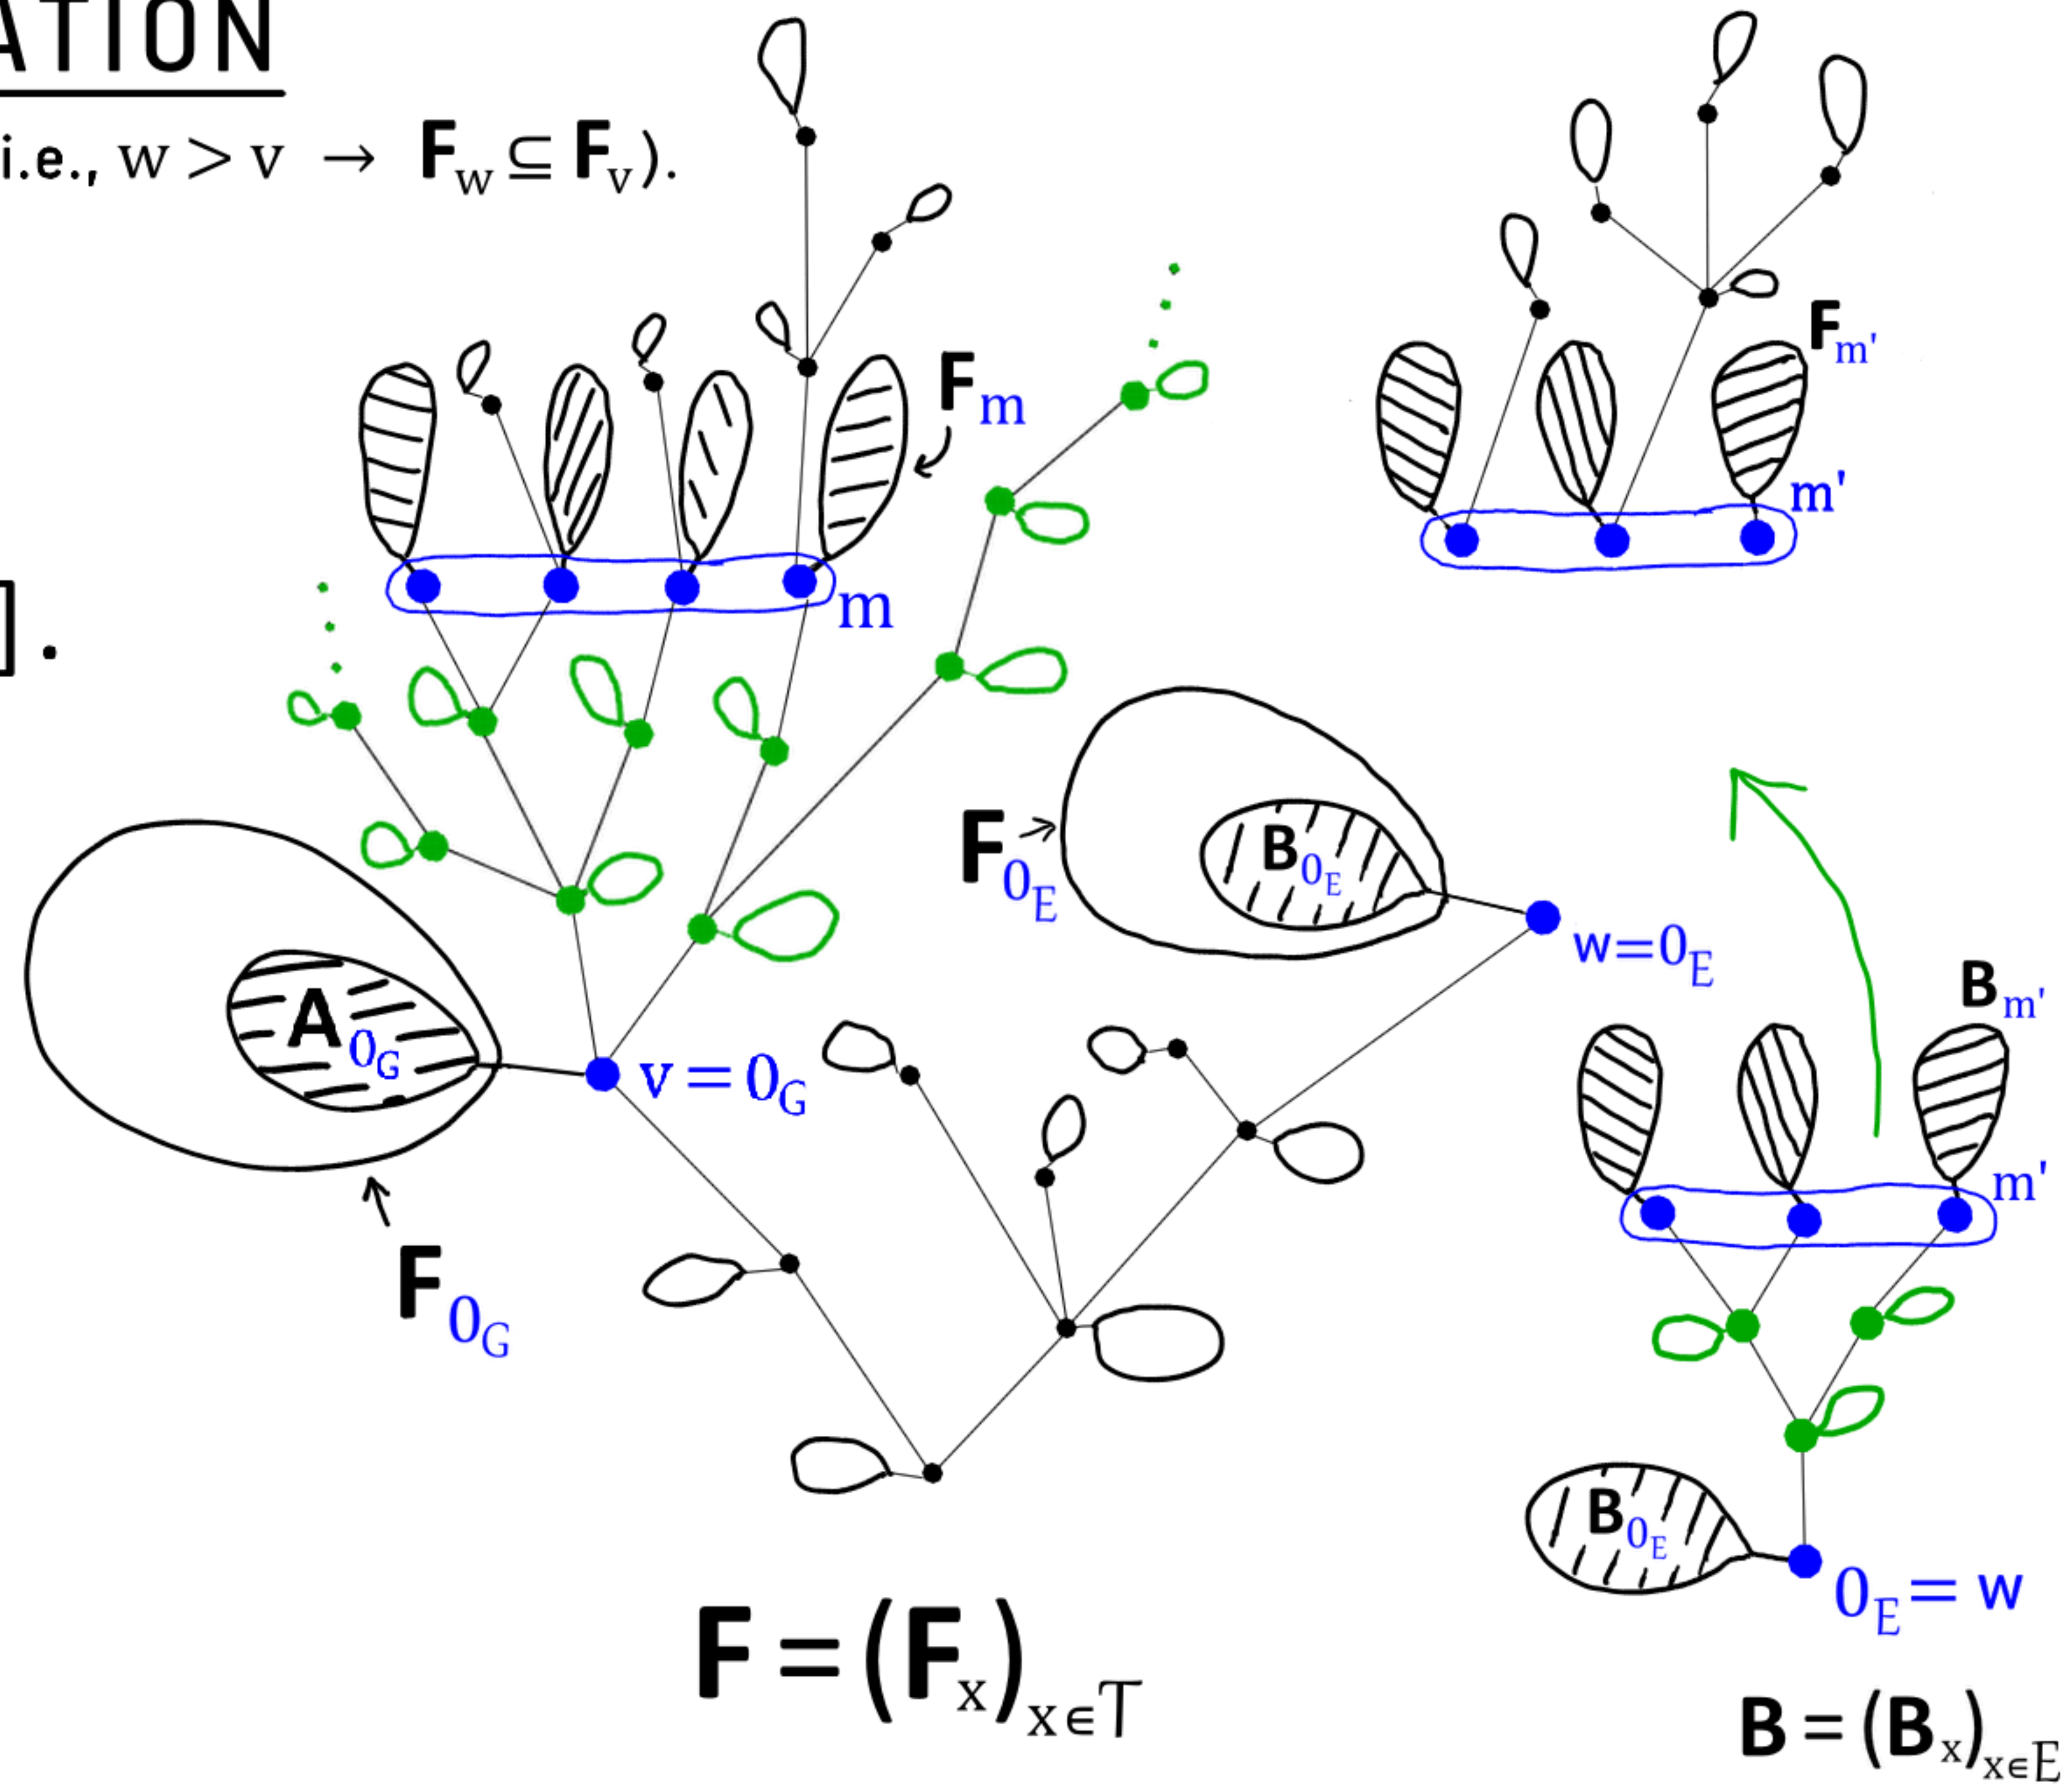



# FOLIAGE HYBRID OPERATION

We consider non-increasing foliage trees (i.e.,  $w > v \rightarrow \mathbf{F}_w \subseteq \mathbf{F}_v$ ).

**A** is a **foliage graft** for **F** iff

- (1)  $G$  is a graft for  $T$ ;
- (2)  $\mathbf{A}_{0_G} \subseteq \mathbf{F}_{0_G}$ ;
- (3)  $\forall m \in \max G \ [ \mathbf{A}_m = \mathbf{F}_m ]$ .

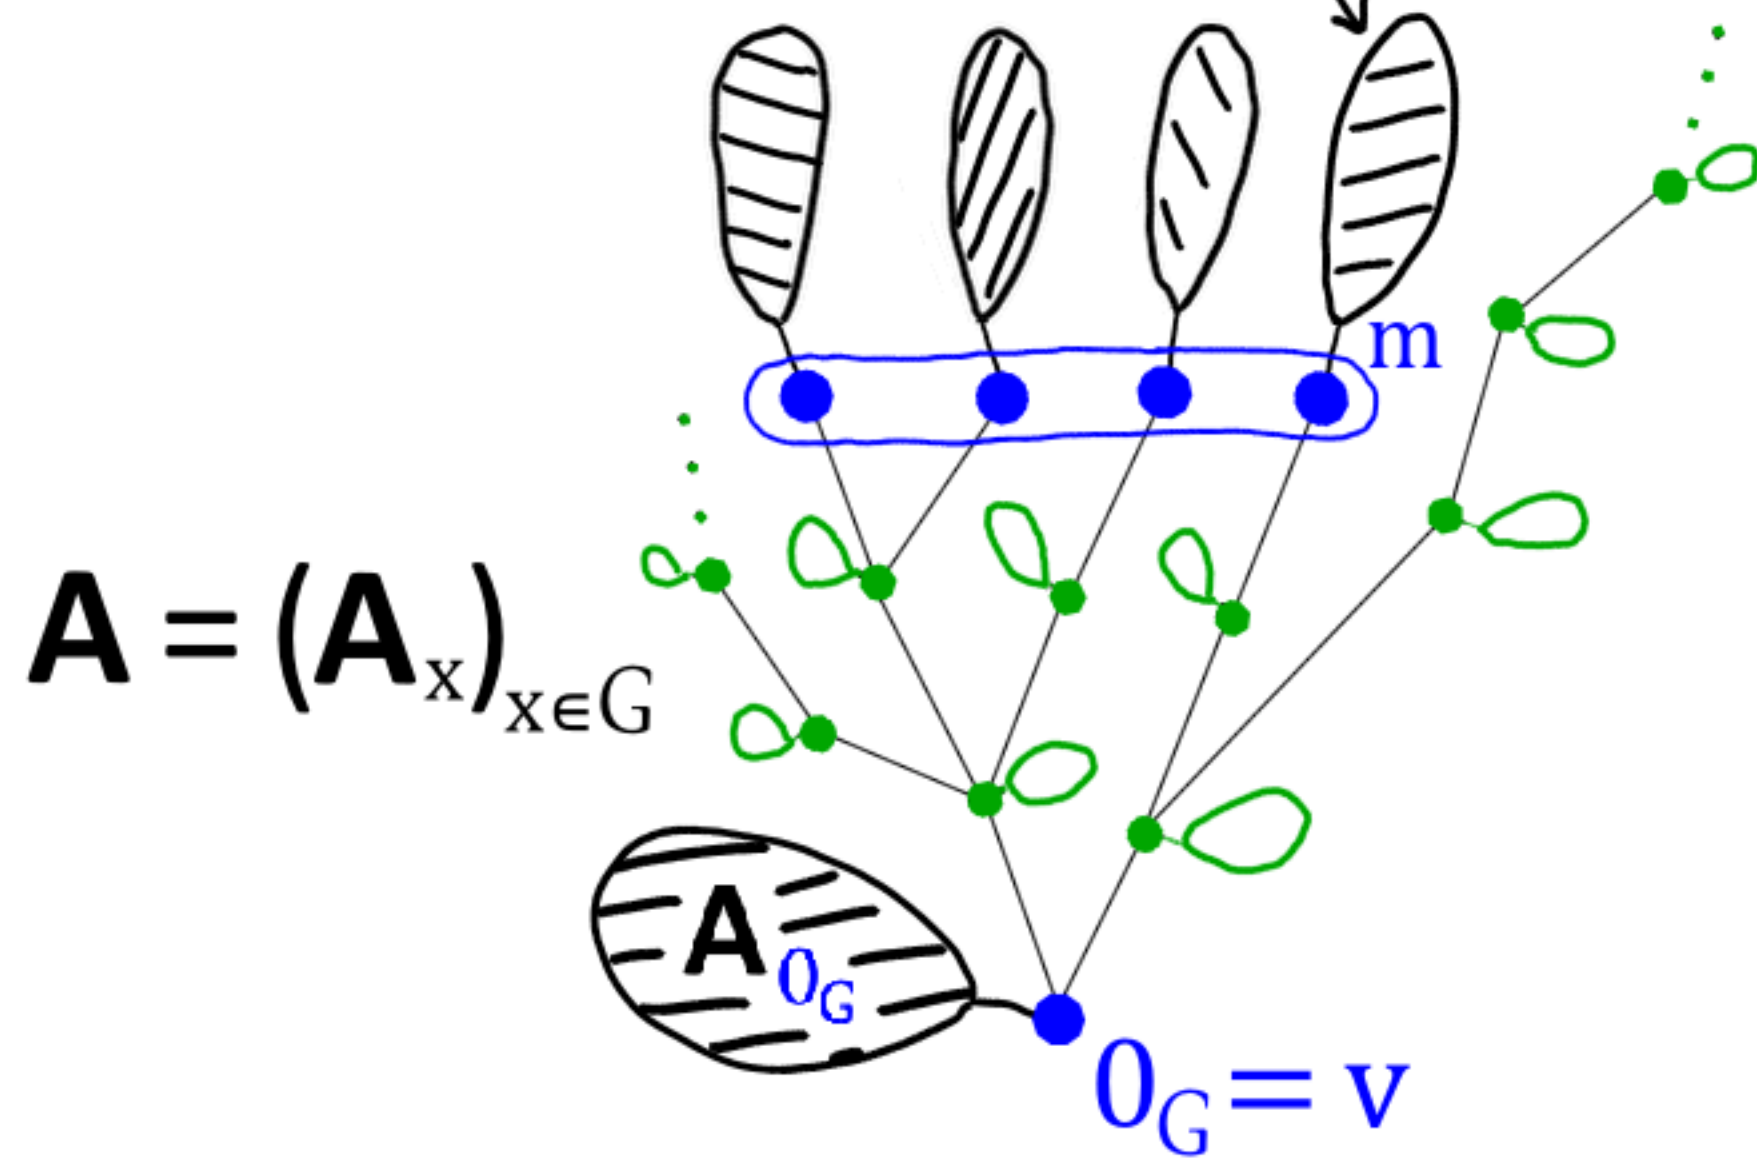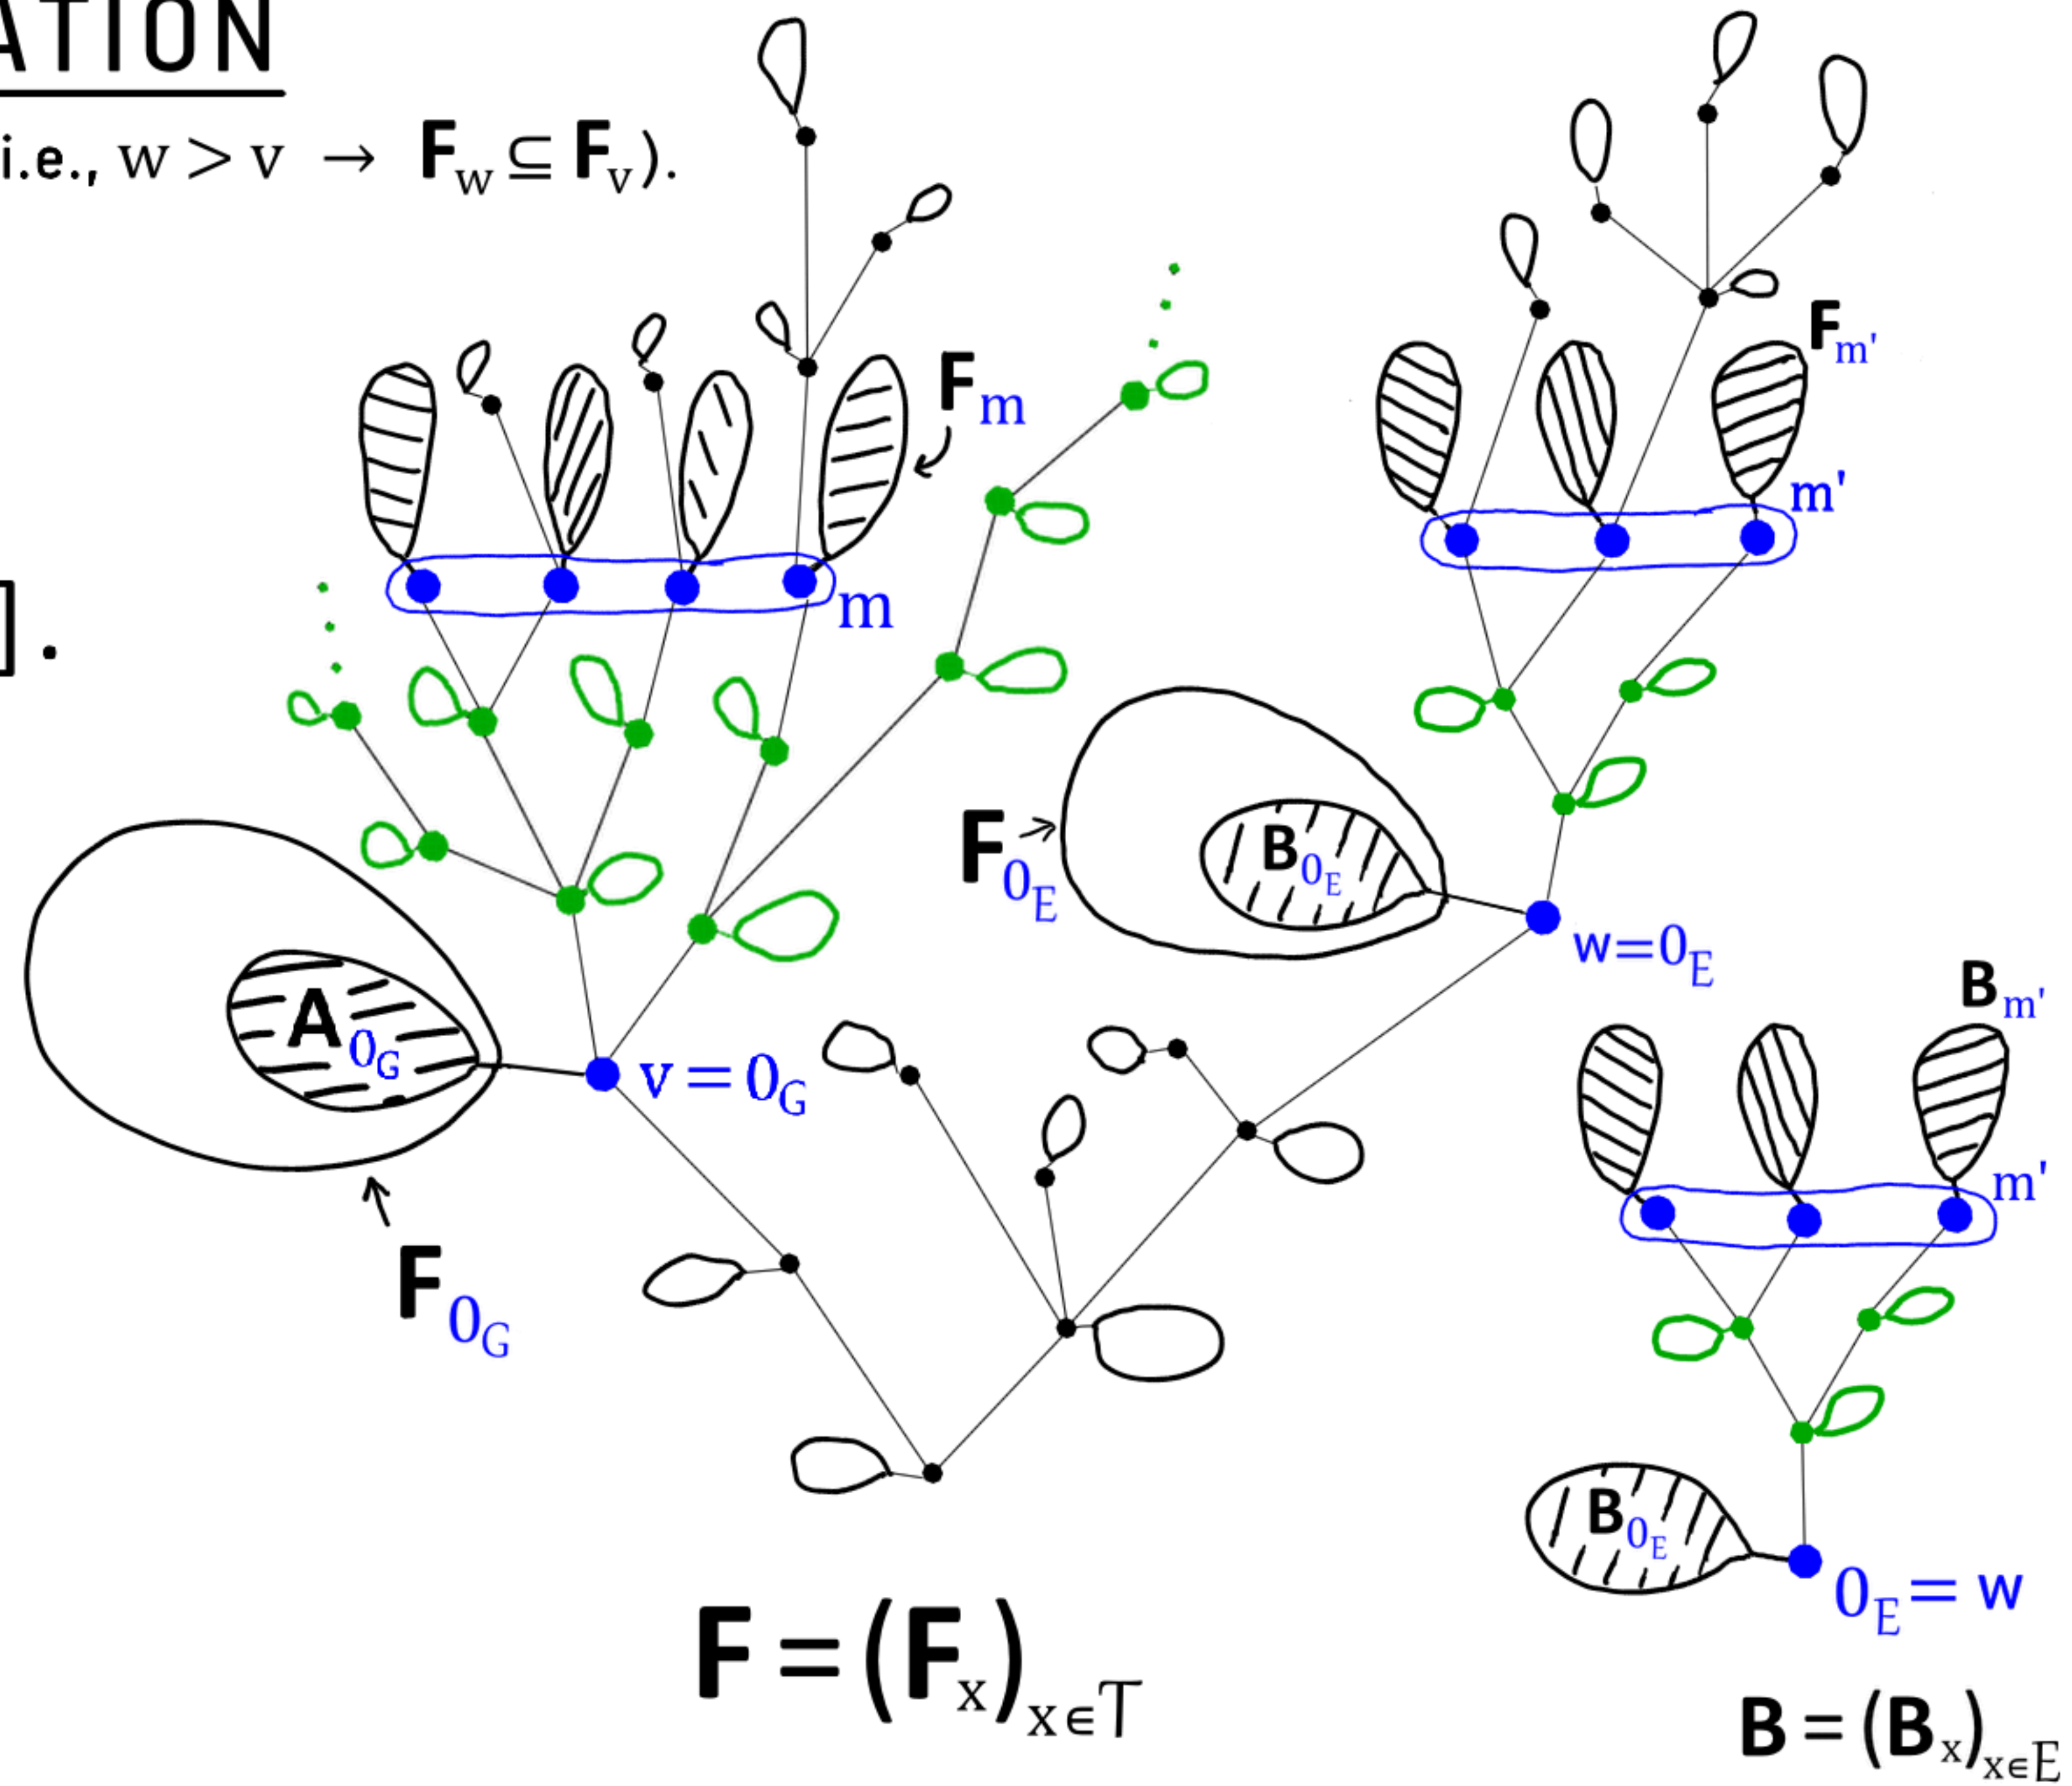



# FOLIAGE HYBRID OPERATION

We consider non-increasing foliage trees (i.e.,  $w > v \rightarrow \mathbf{F}_w \subseteq \mathbf{F}_v$ ).

**A** is a foliage graft for **F** iff

- (1)  $G$  is a graft for  $T$ ;
- (2)  $\mathbf{A}_{0_G} \subseteq \mathbf{F}_{0_G}$ ;
- (3)  $\forall m \in \max G \ [ \mathbf{A}_m = \mathbf{F}_m ]$ .

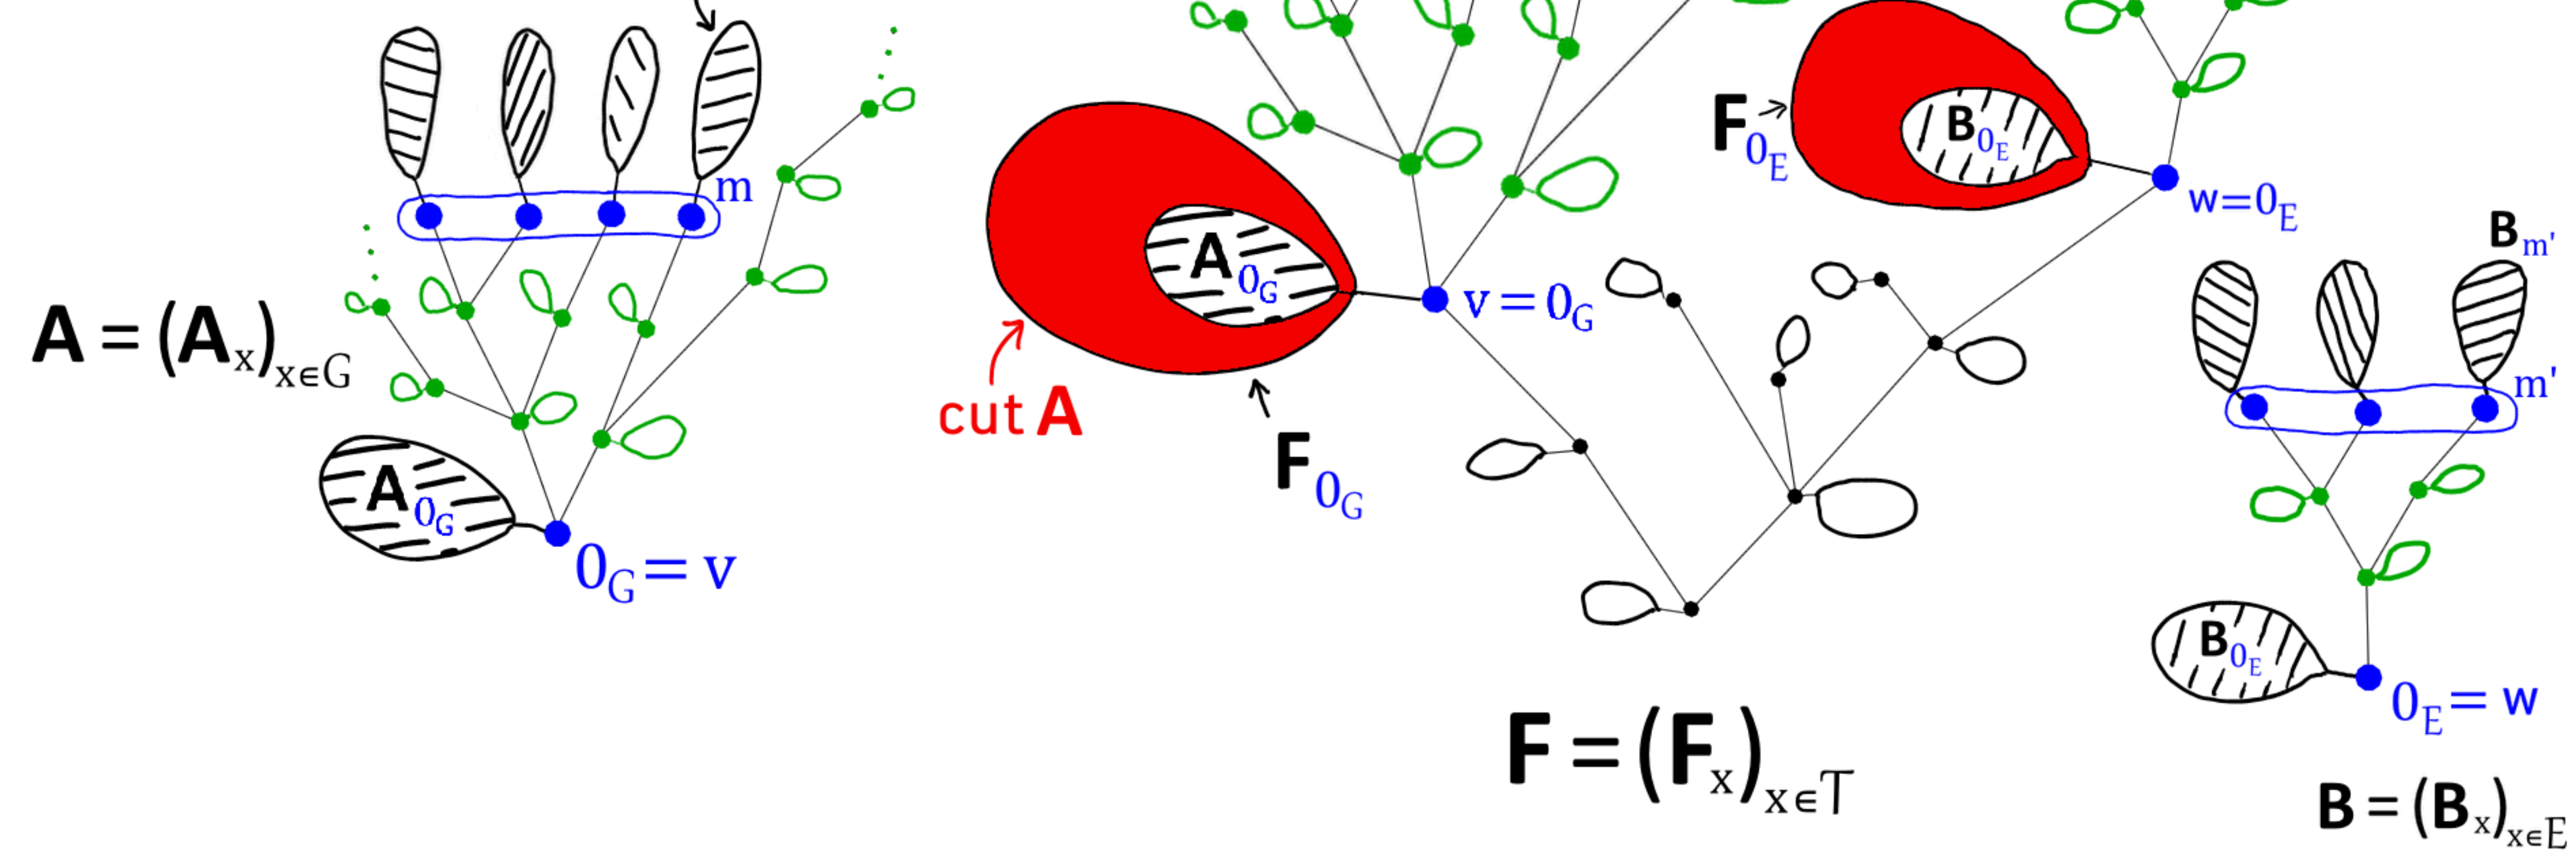



# FOLIAGE HYBRID OPERATION

We consider non-increasing foliage trees (i.e.,  $w > v \rightarrow \mathbf{F}_w \subseteq \mathbf{F}_v$ ).

**A** is a foliage graft for **F** iff

- (1)  $G$  is a graft for  $T$ ;
- (2)  $\mathbf{A}_{0_G} \subseteq \mathbf{F}_{0_G}$ ;
- (3)  $\forall m \in \max G \ [ \mathbf{A}_m = \mathbf{F}_m ]$ .

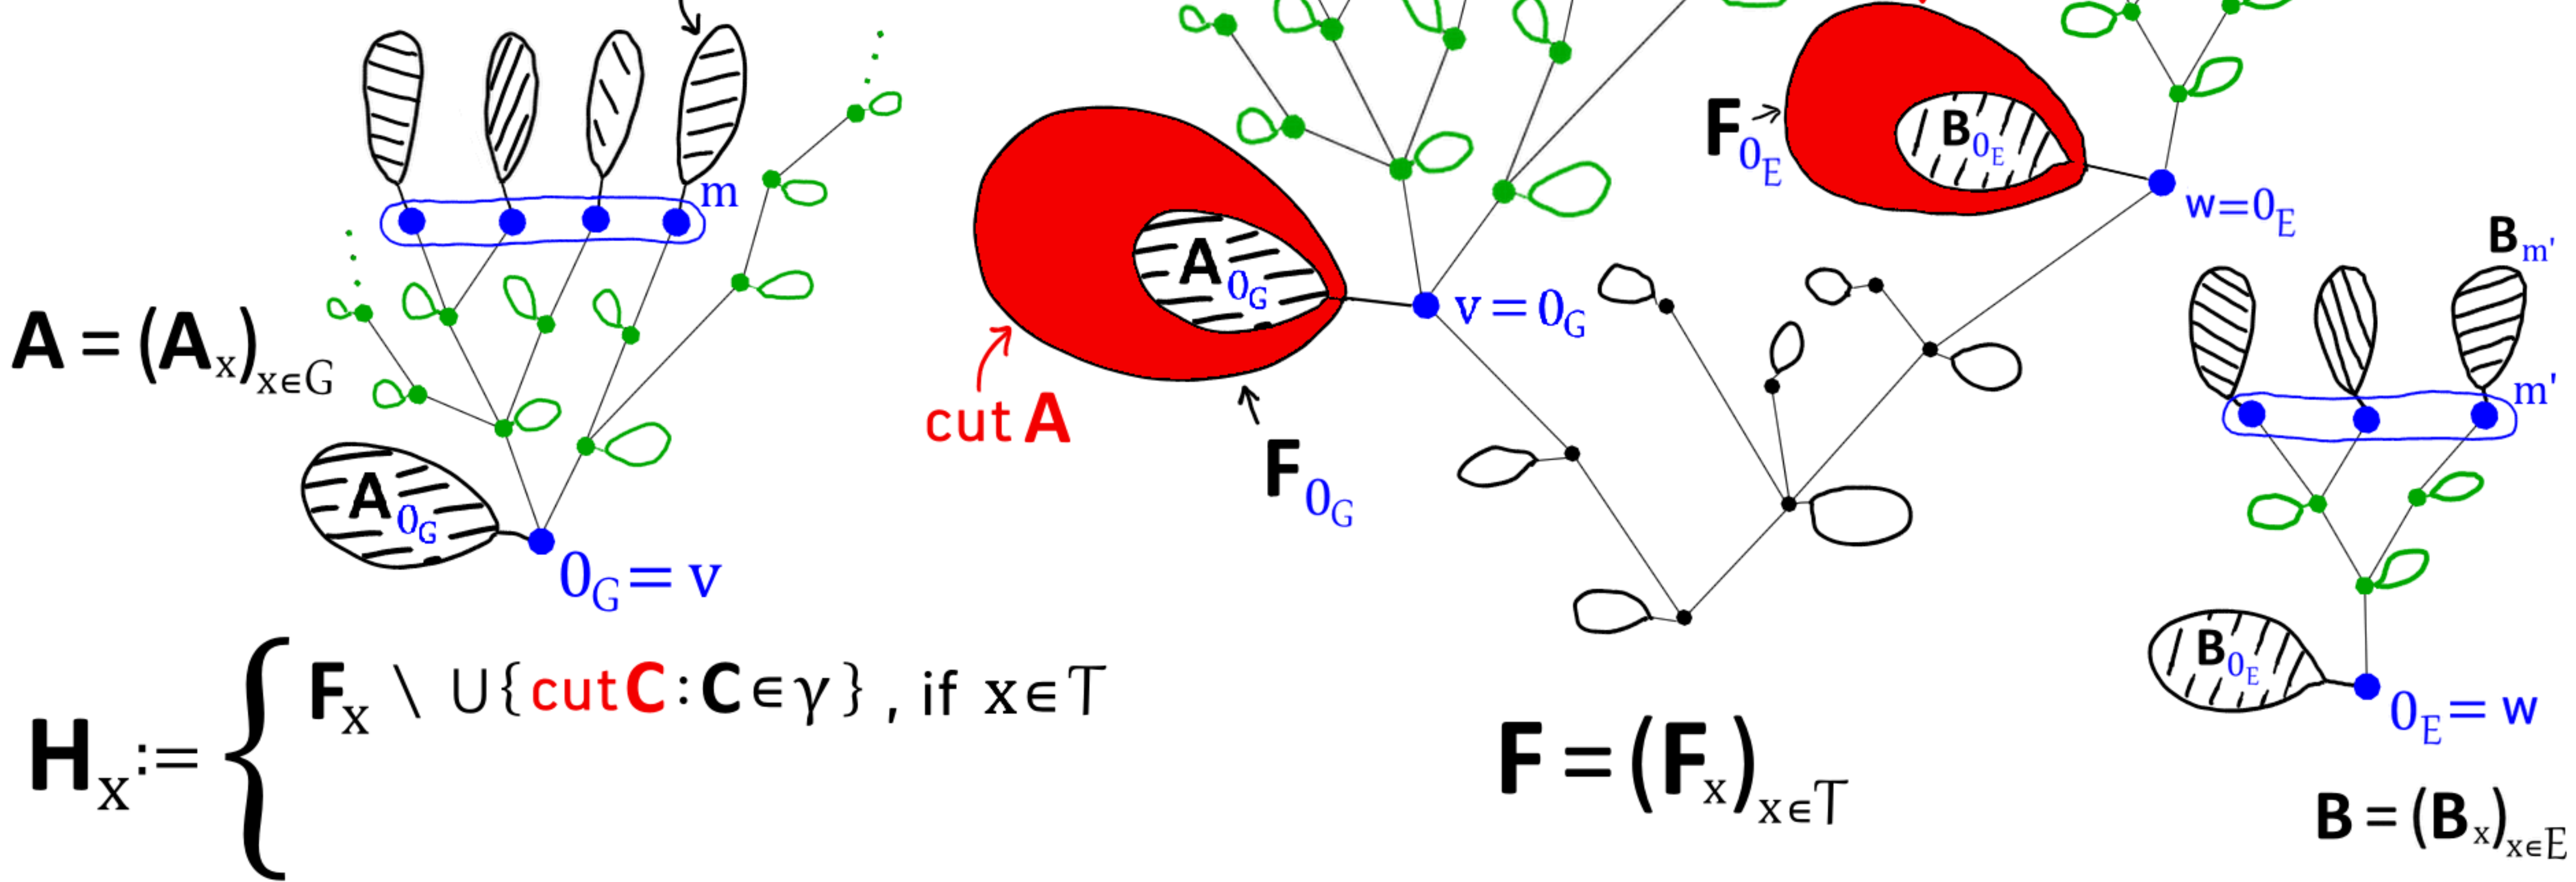



# FOLIAGE HYBRID OPERATION

We consider non-increasing foliage trees (i.e.,  $w > v \rightarrow \mathbf{F}_w \subseteq \mathbf{F}_v$ ).

**A** is a foliage graft for **F** iff

- (1)  $G$  is a graft for  $T$ ;
- (2)  $\mathbf{A}_{0_G} \subseteq \mathbf{F}_{0_G}$ ;
- (3)  $\forall m \in \max G \ [ \mathbf{A}_m = \mathbf{F}_m ]$ .

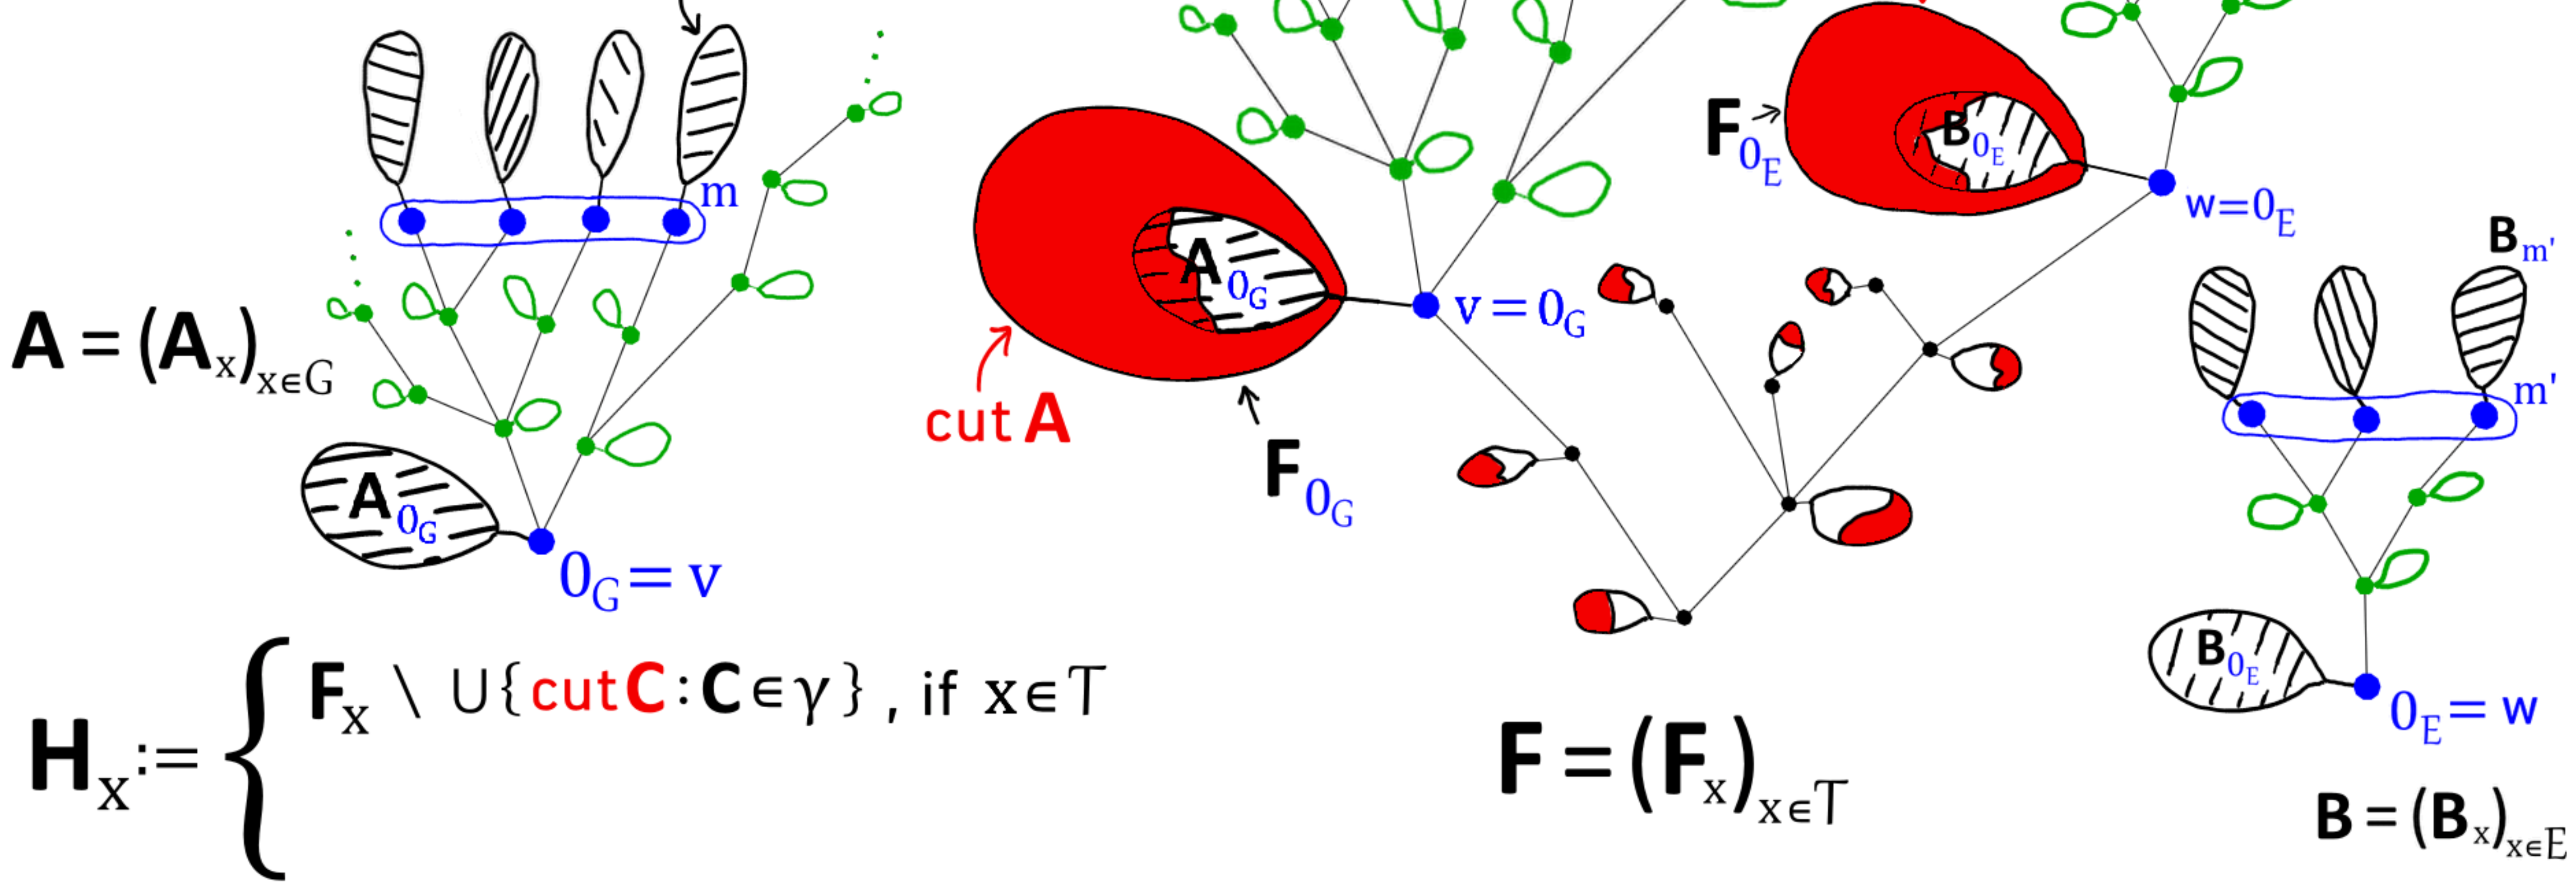



# FOLIAGE HYBRID OPERATION

We consider non-increasing foliage trees (i.e.,  $w > v \rightarrow \mathbf{F}_w \subseteq \mathbf{F}_v$ ).

**A** is a foliage graft for **F** iff

- (1) **G** is a graft for **T**;
- (2)  $\mathbf{A}_{0_G} \subseteq \mathbf{F}_{0_G}$ ;
- (3)  $\forall m \in \max G \ [ \mathbf{A}_m = \mathbf{F}_m ]$ .

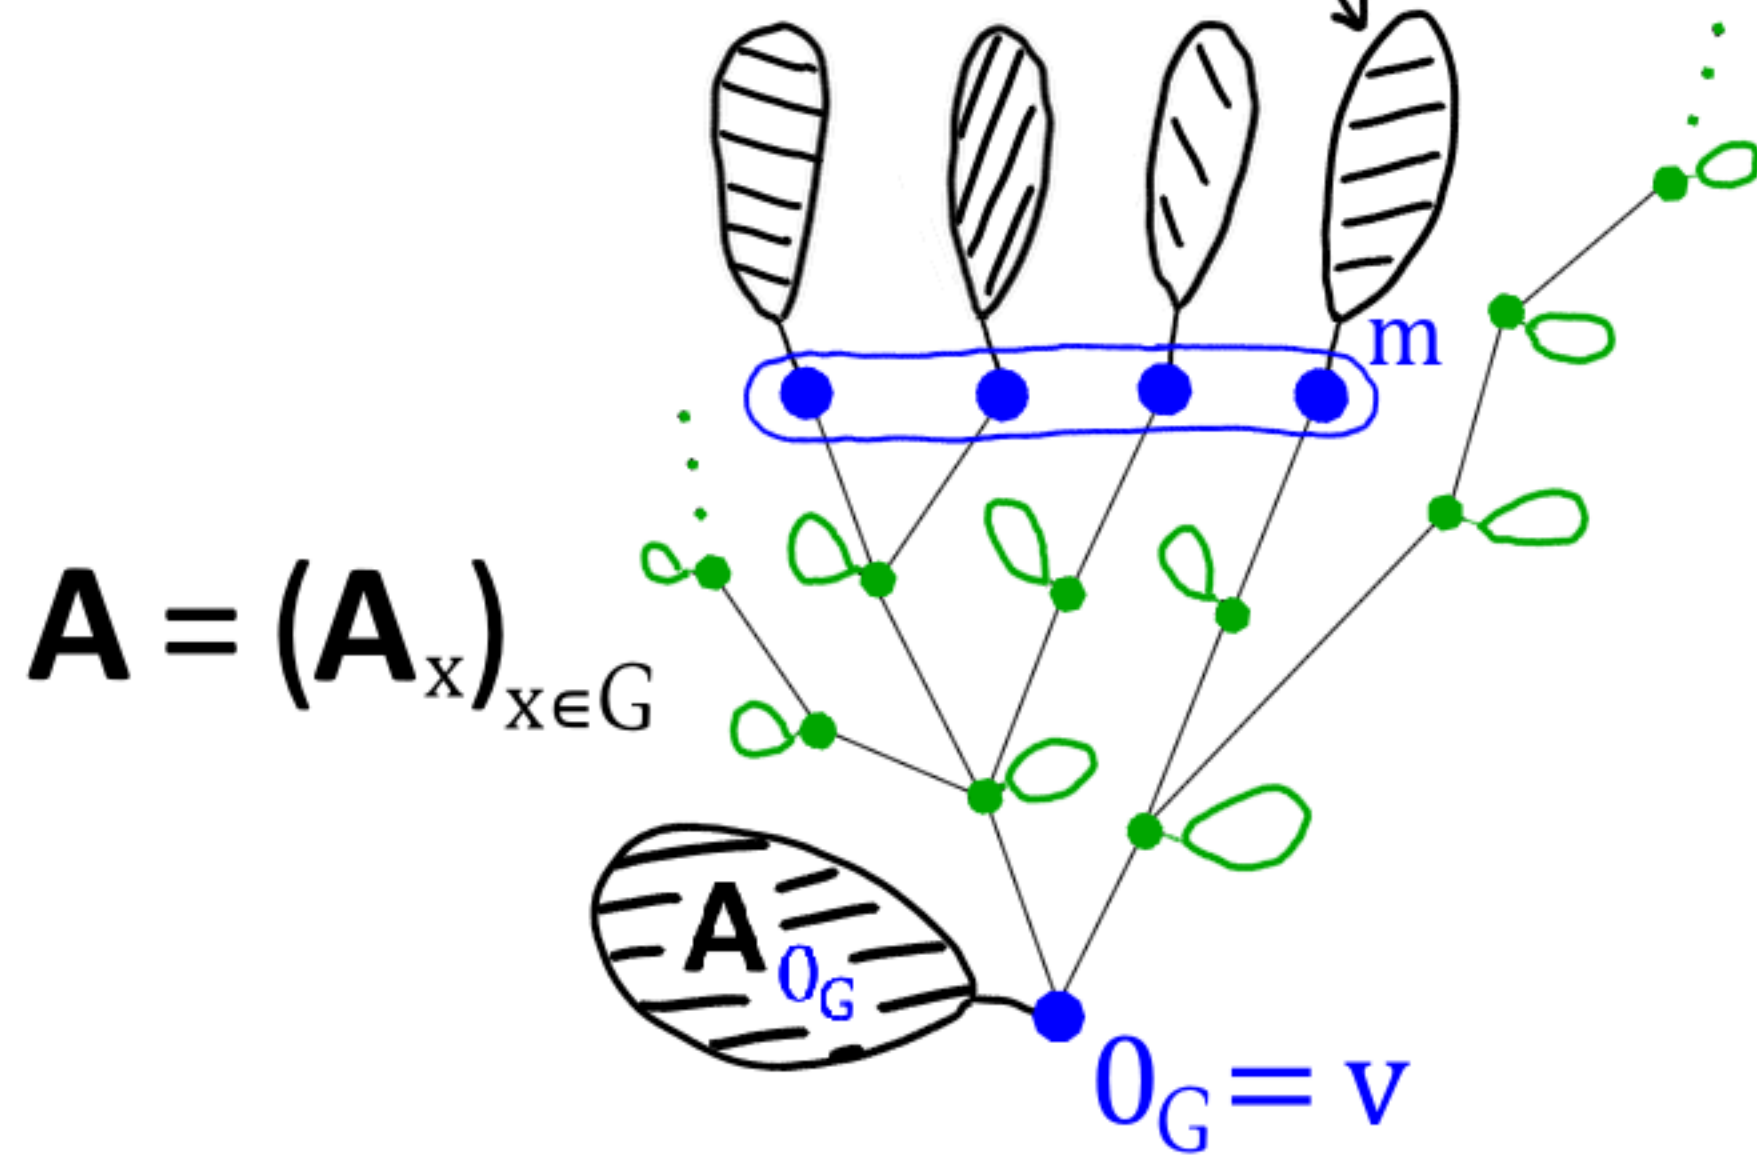

$$\mathbf{H}_x := \begin{cases} \mathbf{F}_x \setminus \cup \{ \text{cut } \mathbf{C} : \mathbf{C} \in \gamma \}, & \text{if } x \in T \end{cases}$$

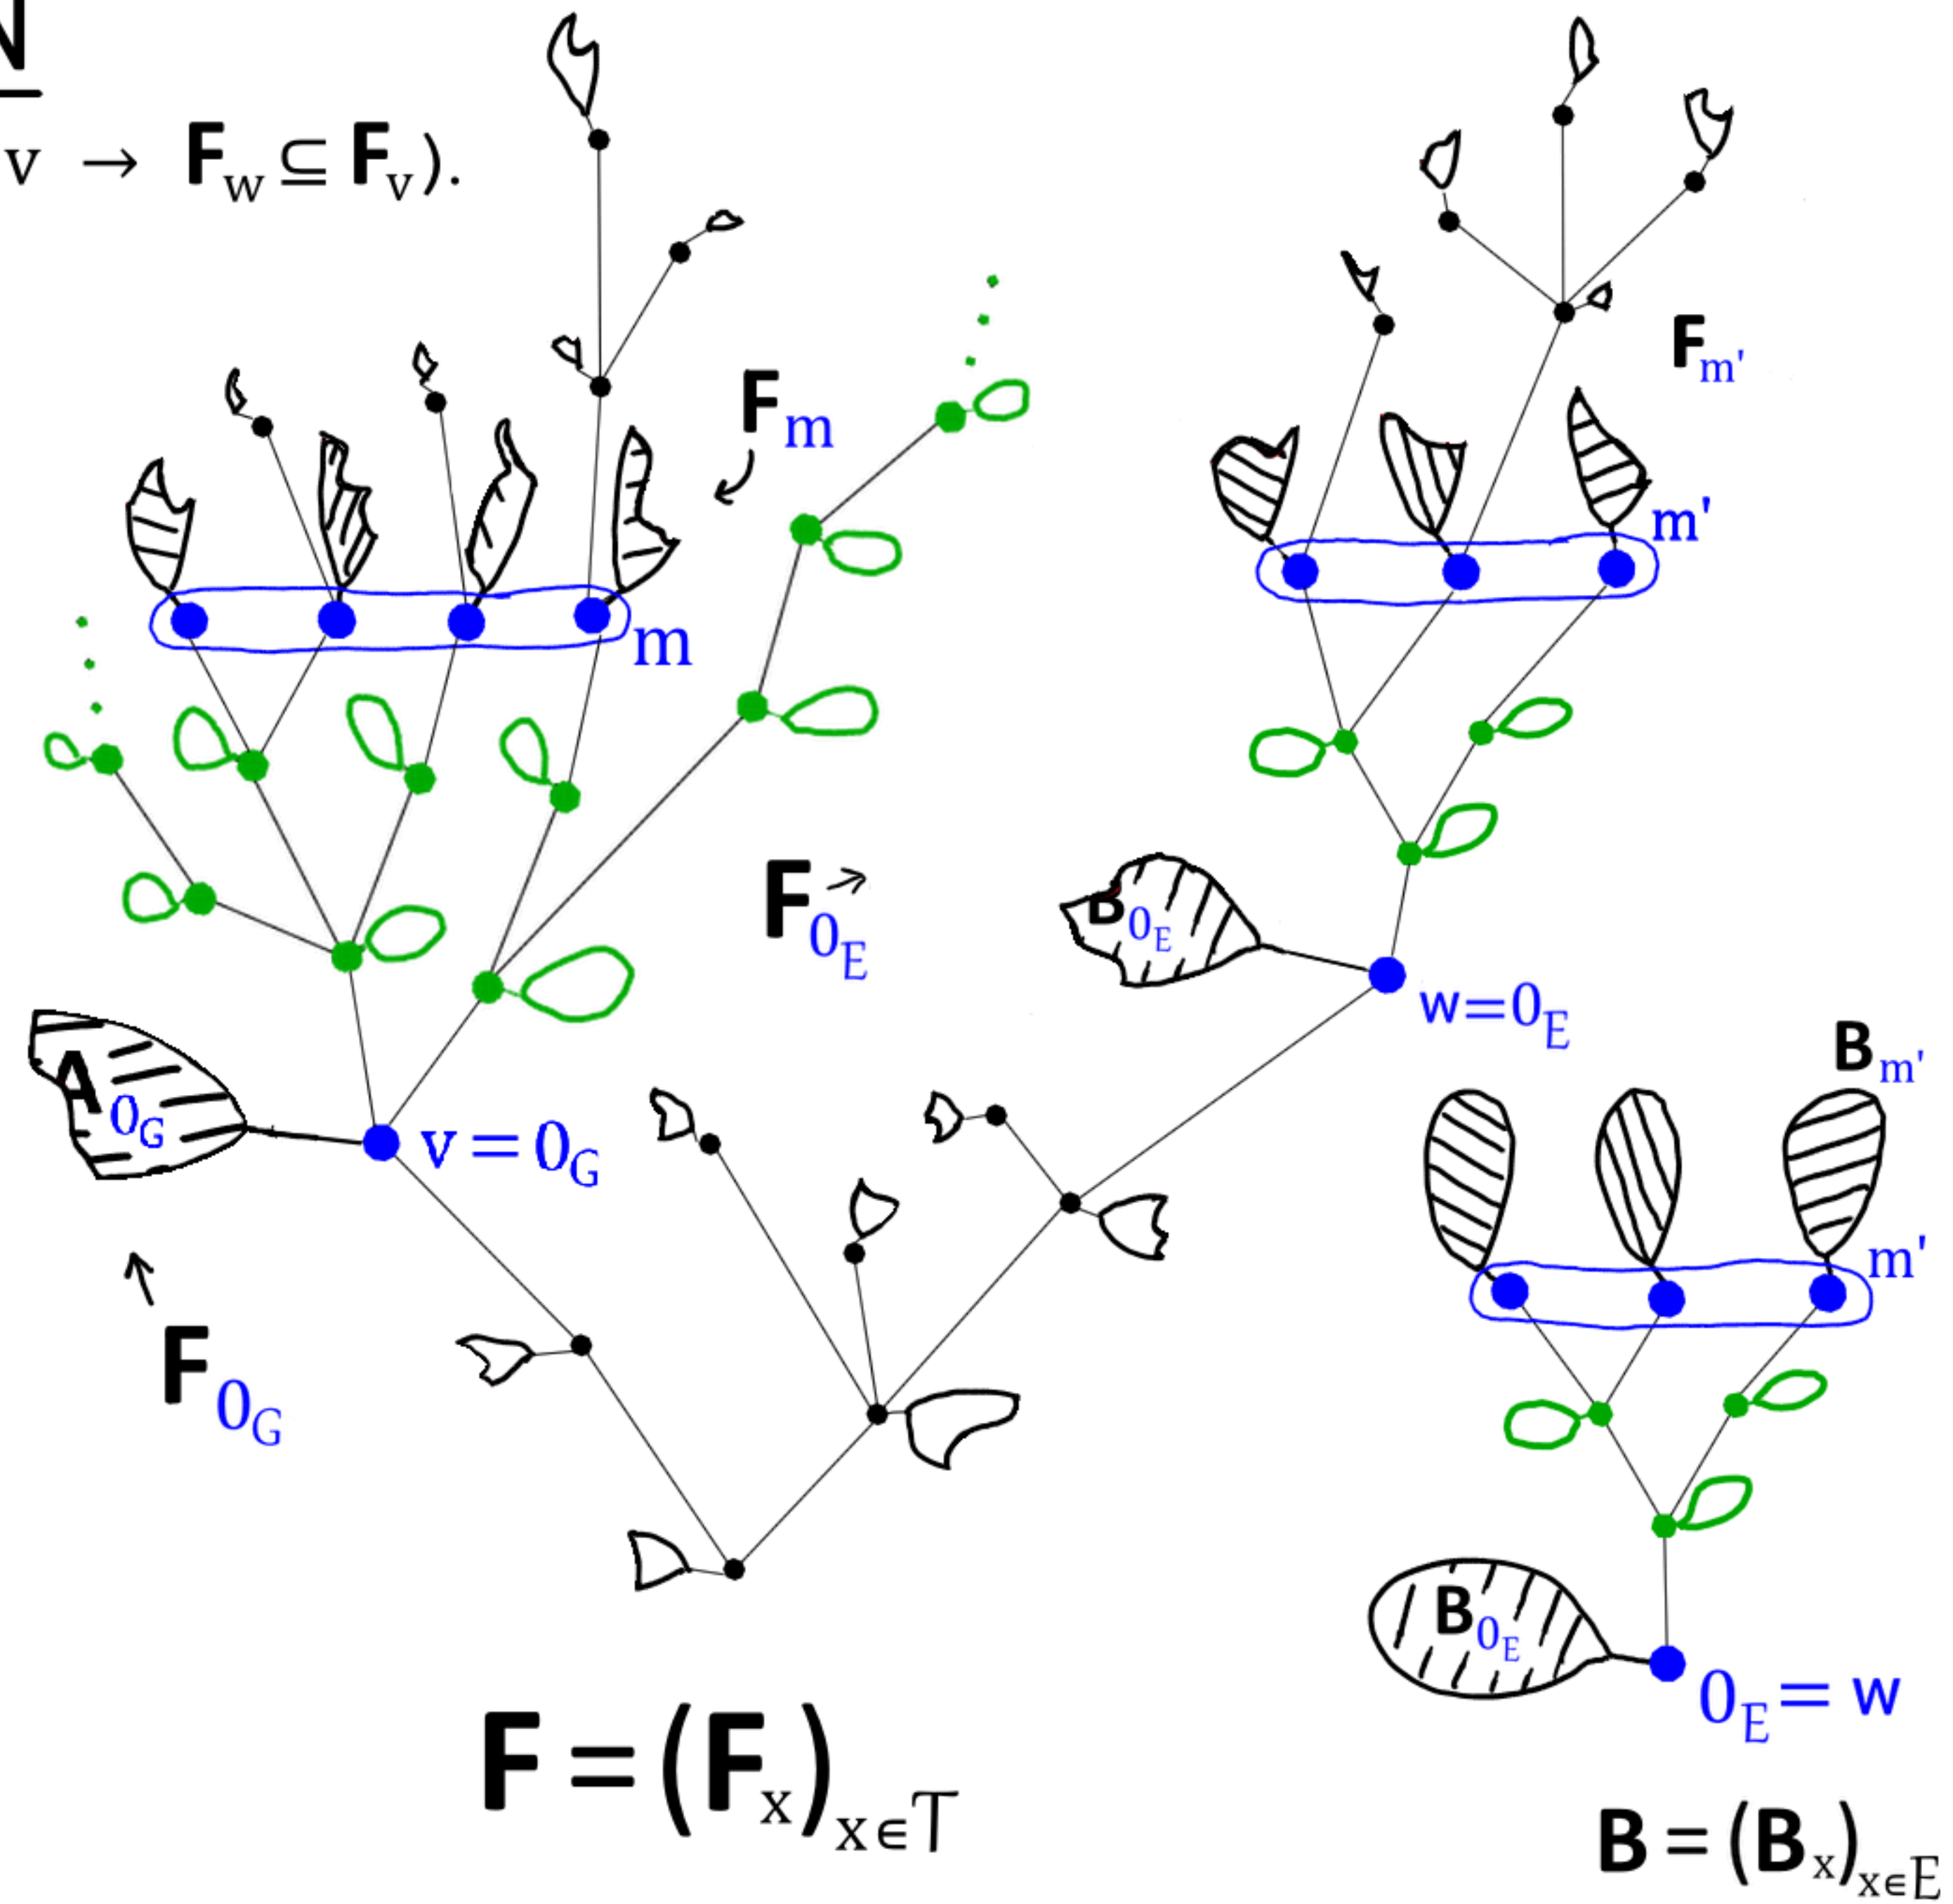



## FOLIAGE HYBRID OPERATION

We consider non-increasing foliage trees (i.e.,  $w > v \rightarrow \mathbf{F}_w \subseteq \mathbf{F}_v$ ).

**A** is a **foliage graft** for **F** iff

- (1)  $G$  is a graft for  $T$ ;
- (2)  $\mathbf{A}_{0_G} \subseteq \mathbf{F}_{0_G}$ ;
- (3)  $\forall m \in \max G \ [ \mathbf{A}_m = \mathbf{F}_m ]$ .

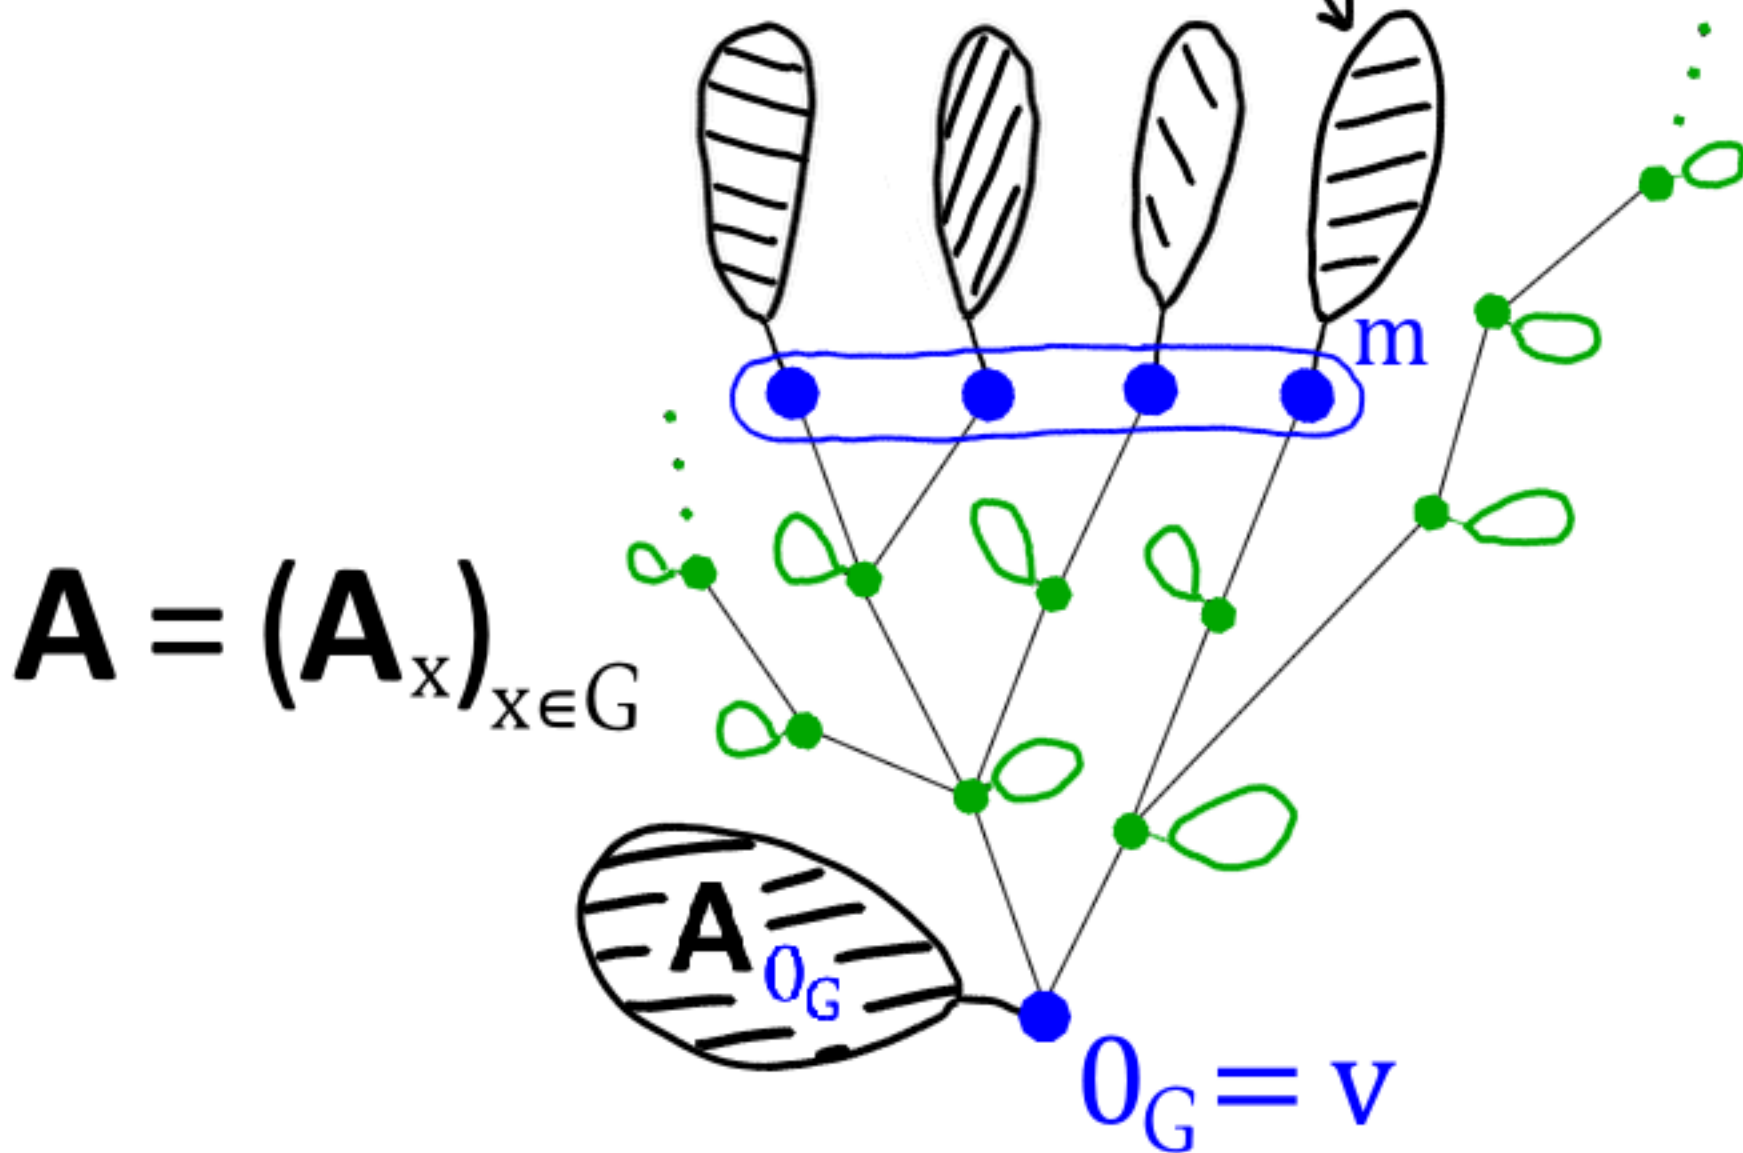

$$\mathbf{H}_x := \begin{cases} \mathbf{F}_x \setminus \cup \{\text{cut } \mathbf{C} : \mathbf{C} \in \gamma\}, & \text{if } x \in T \\ \mathbf{D}_x \setminus \cup \{\text{cut } \mathbf{C} : \mathbf{C} \in \gamma\}, & \text{if } x \in \text{implant } \mathbf{D} \end{cases}$$

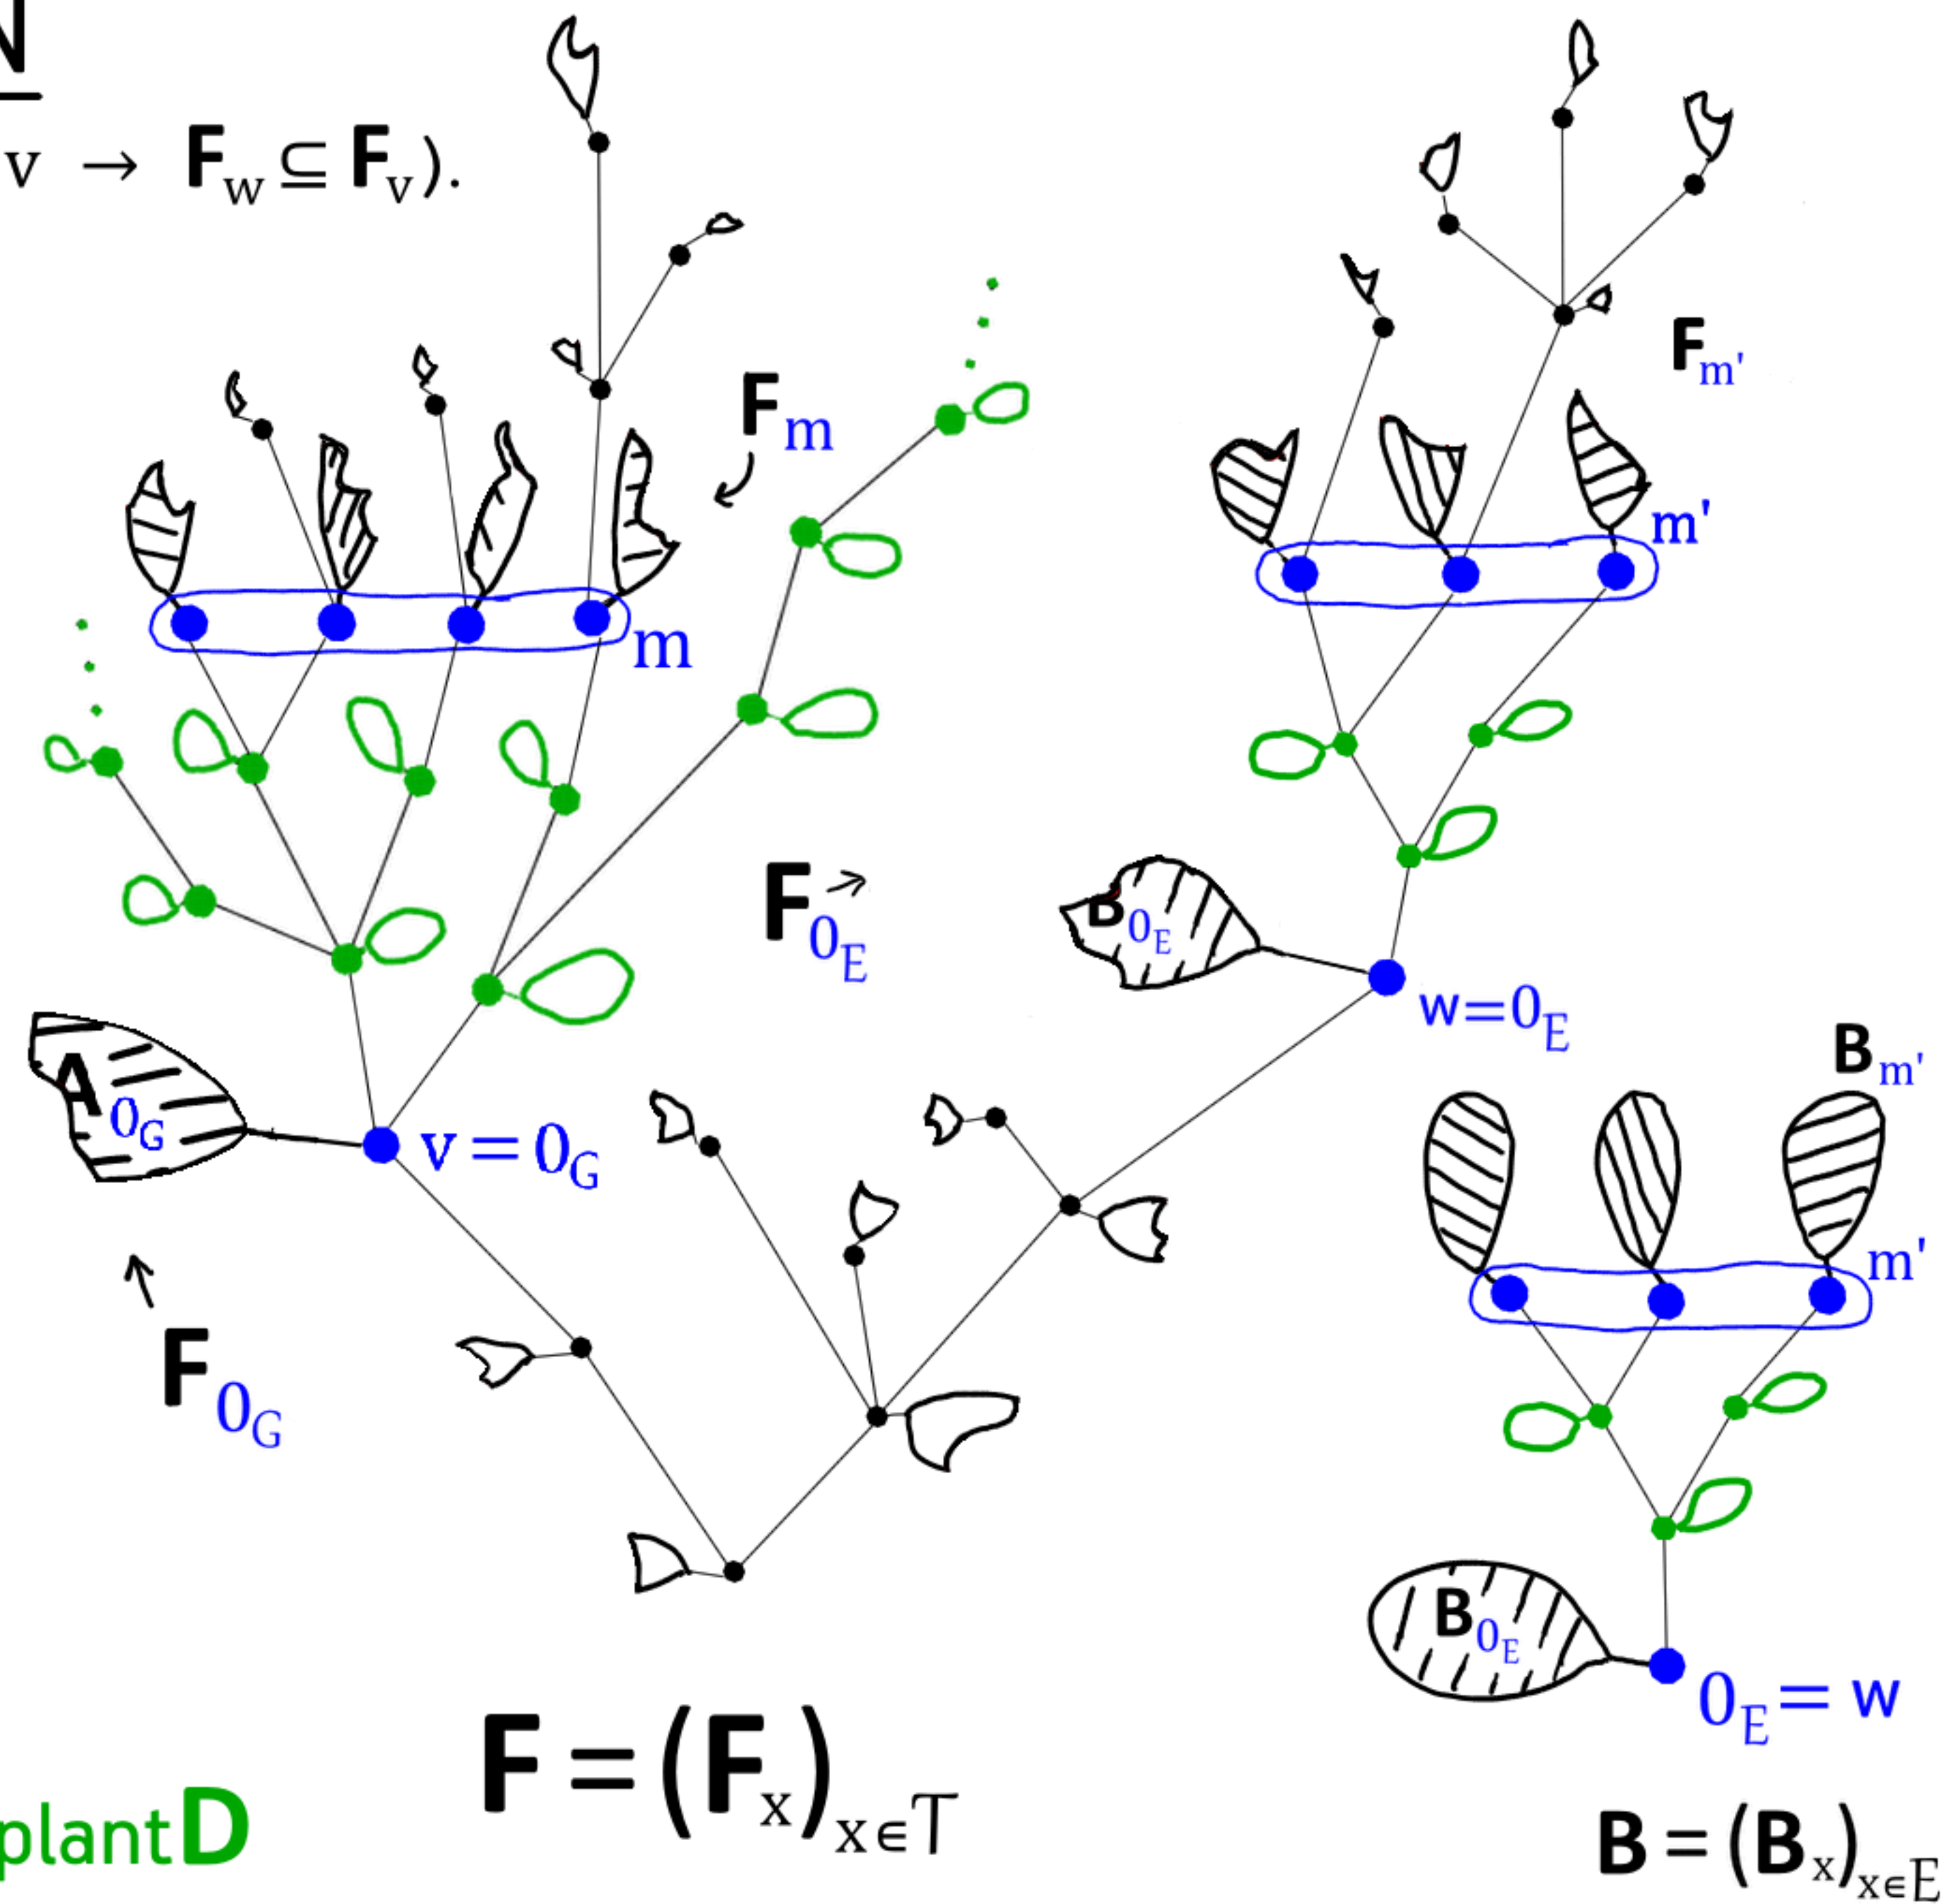



# FOLIAGE HYBRID OPERATION

We consider non-increasing foliage trees (i.e.,  $w > v \rightarrow \mathbf{F}_w \subseteq \mathbf{F}_v$ ).

**A** is a foliage graft for **F** iff

- (1) **G** is a graft for **T**;
- (2)  $\mathbf{A}_{0_G} \subseteq \mathbf{F}_{0_G}$ ;
- (3)  $\forall m \in \max G \ [ \mathbf{A}_m = \mathbf{F}_m ]$ .

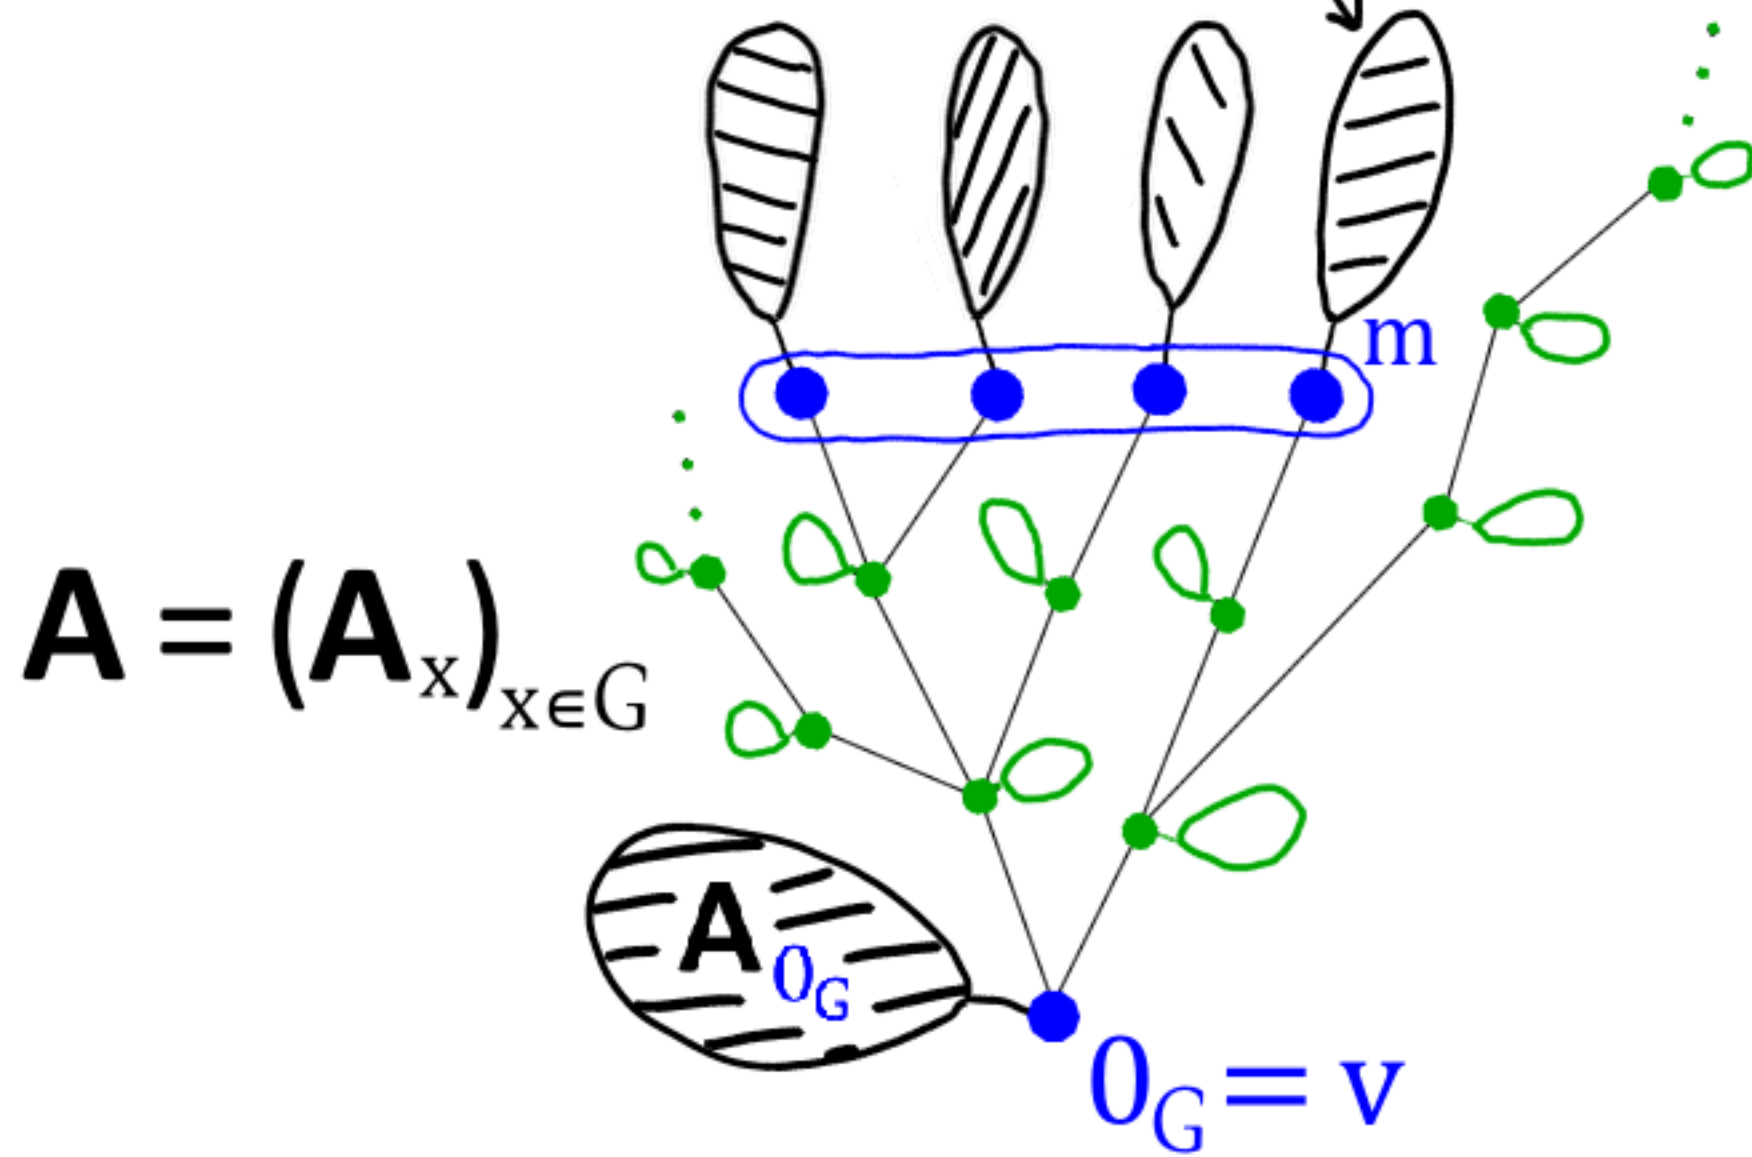

$$\mathbf{H}_x := \begin{cases} \mathbf{F}_x \setminus \cup \{ \text{cut } \mathbf{C} : \mathbf{C} \in \gamma \}, & \text{if } x \in T \\ \mathbf{D}_x \setminus \cup \{ \text{cut } \mathbf{C} : \mathbf{C} \in \gamma \}, & \text{if } x \in \text{implant } \mathbf{D} \end{cases}$$

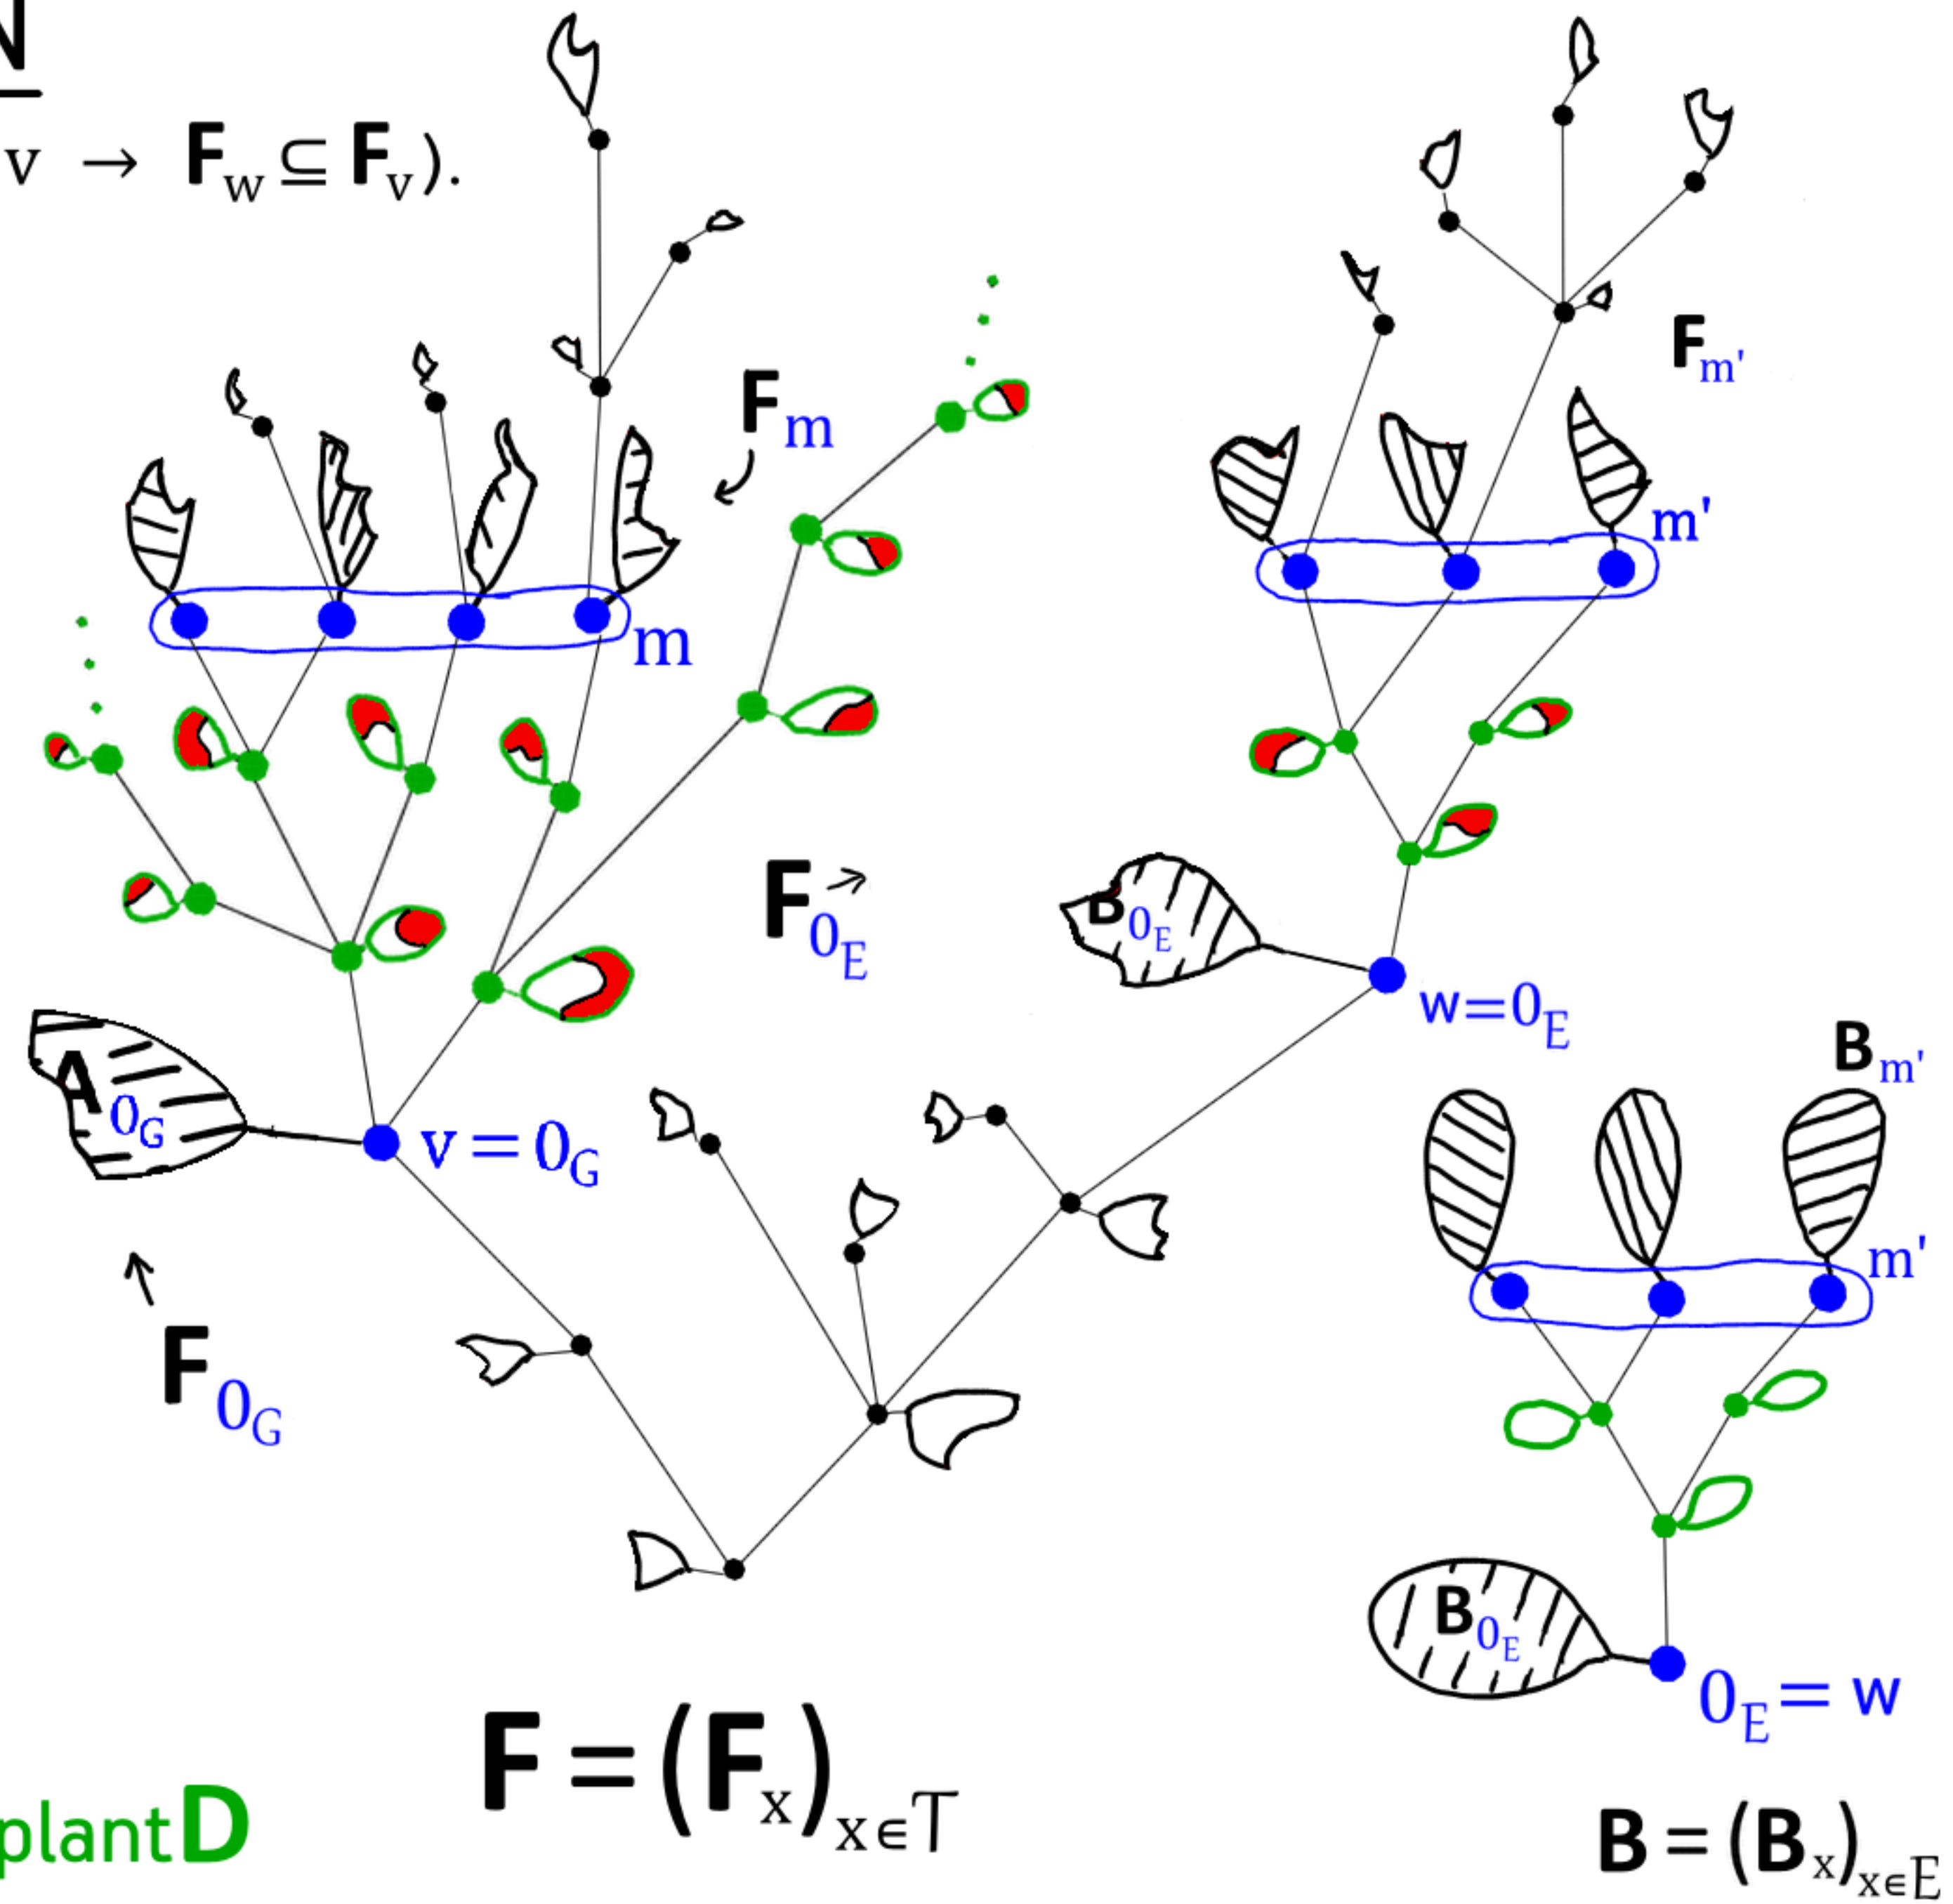



# FOLIAGE HYBRID OPERATION

We consider non-increasing foliage trees (i.e.,  $w > v \rightarrow \mathbf{F}_w \subseteq \mathbf{F}_v$ ).

**A** is a **foliage graft** for **F** iff

- (1)  $G$  is a graft for  $T$ ;
- (2)  $\mathbf{A}_{0_G} \subseteq \mathbf{F}_{0_G}$ ;
- (3)  $\forall m \in \max G \ [ \mathbf{A}_m = \mathbf{F}_m ]$ .

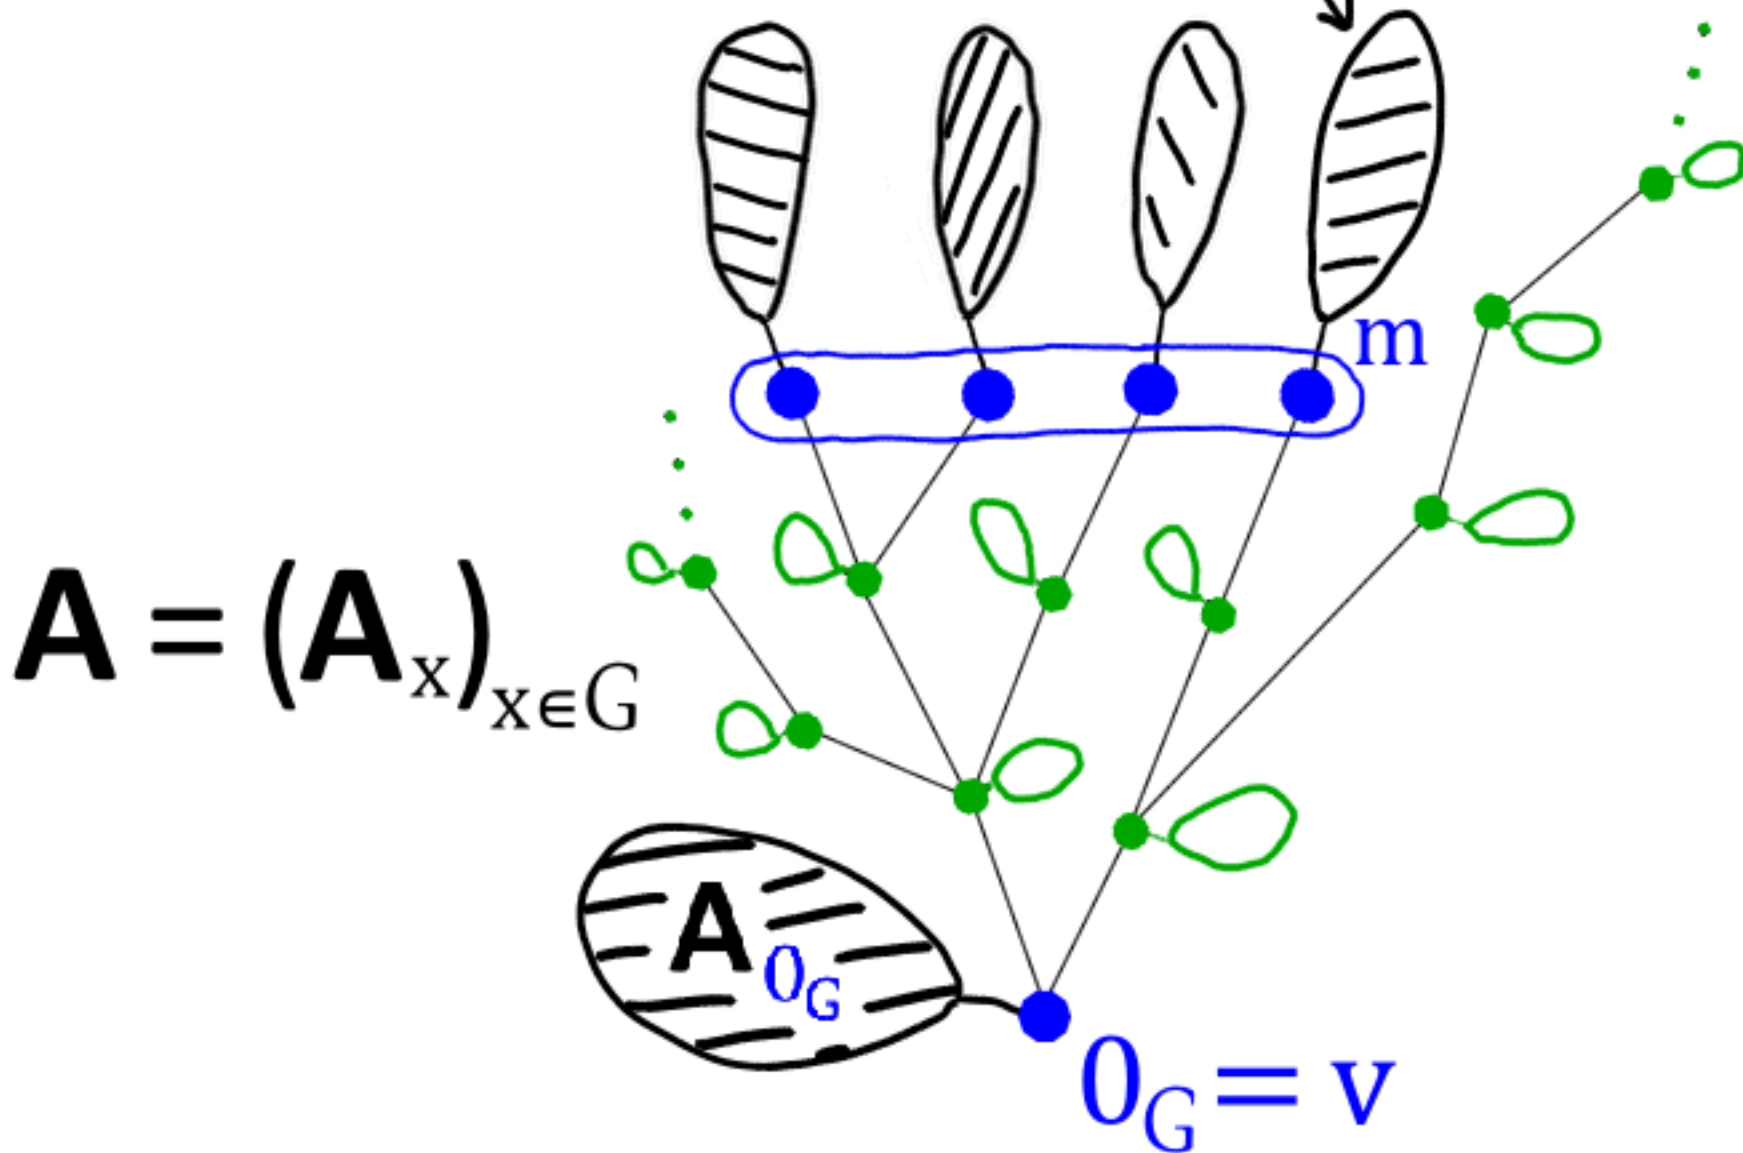

$$\mathbf{H}_x := \begin{cases} \mathbf{F}_x \setminus \cup \{\text{cut } \mathbf{C} : \mathbf{C} \in \gamma\}, & \text{if } x \in T \\ \mathbf{D}_x \setminus \cup \{\text{cut } \mathbf{C} : \mathbf{C} \in \gamma\}, & \text{if } x \in \text{implant } \mathbf{D} \end{cases}$$

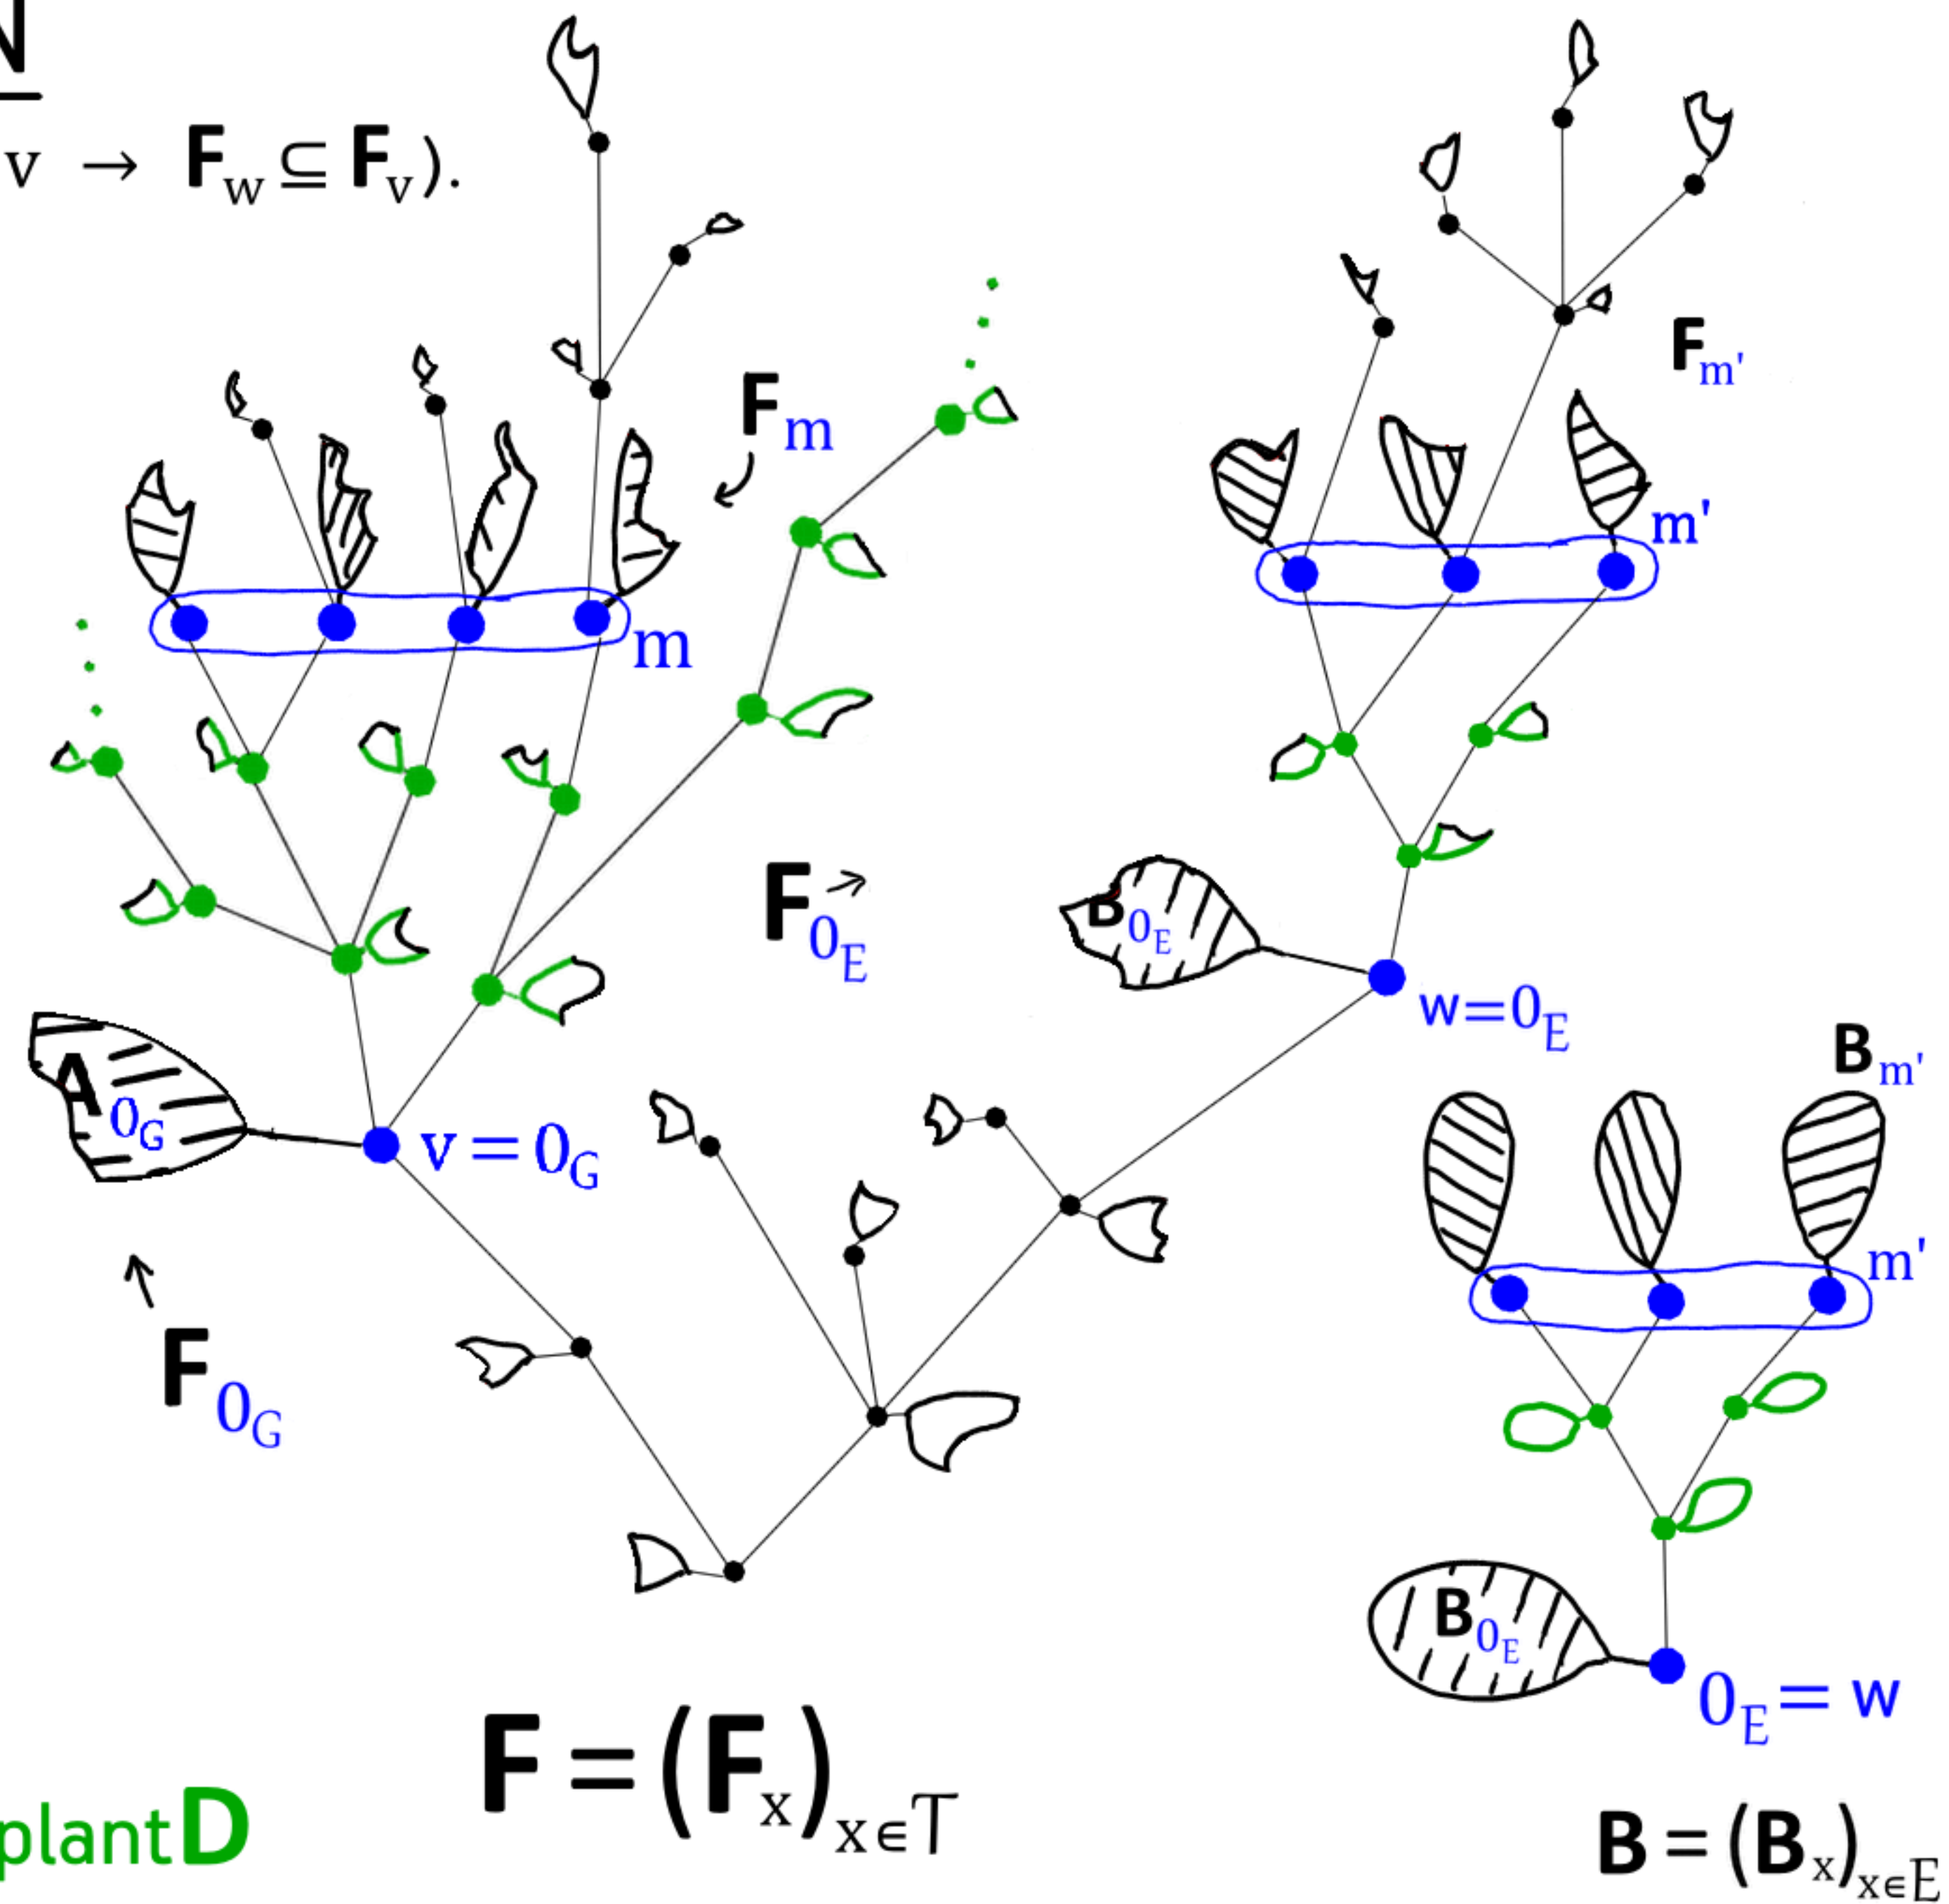

# FOLIAGE HYBRID OPERATION

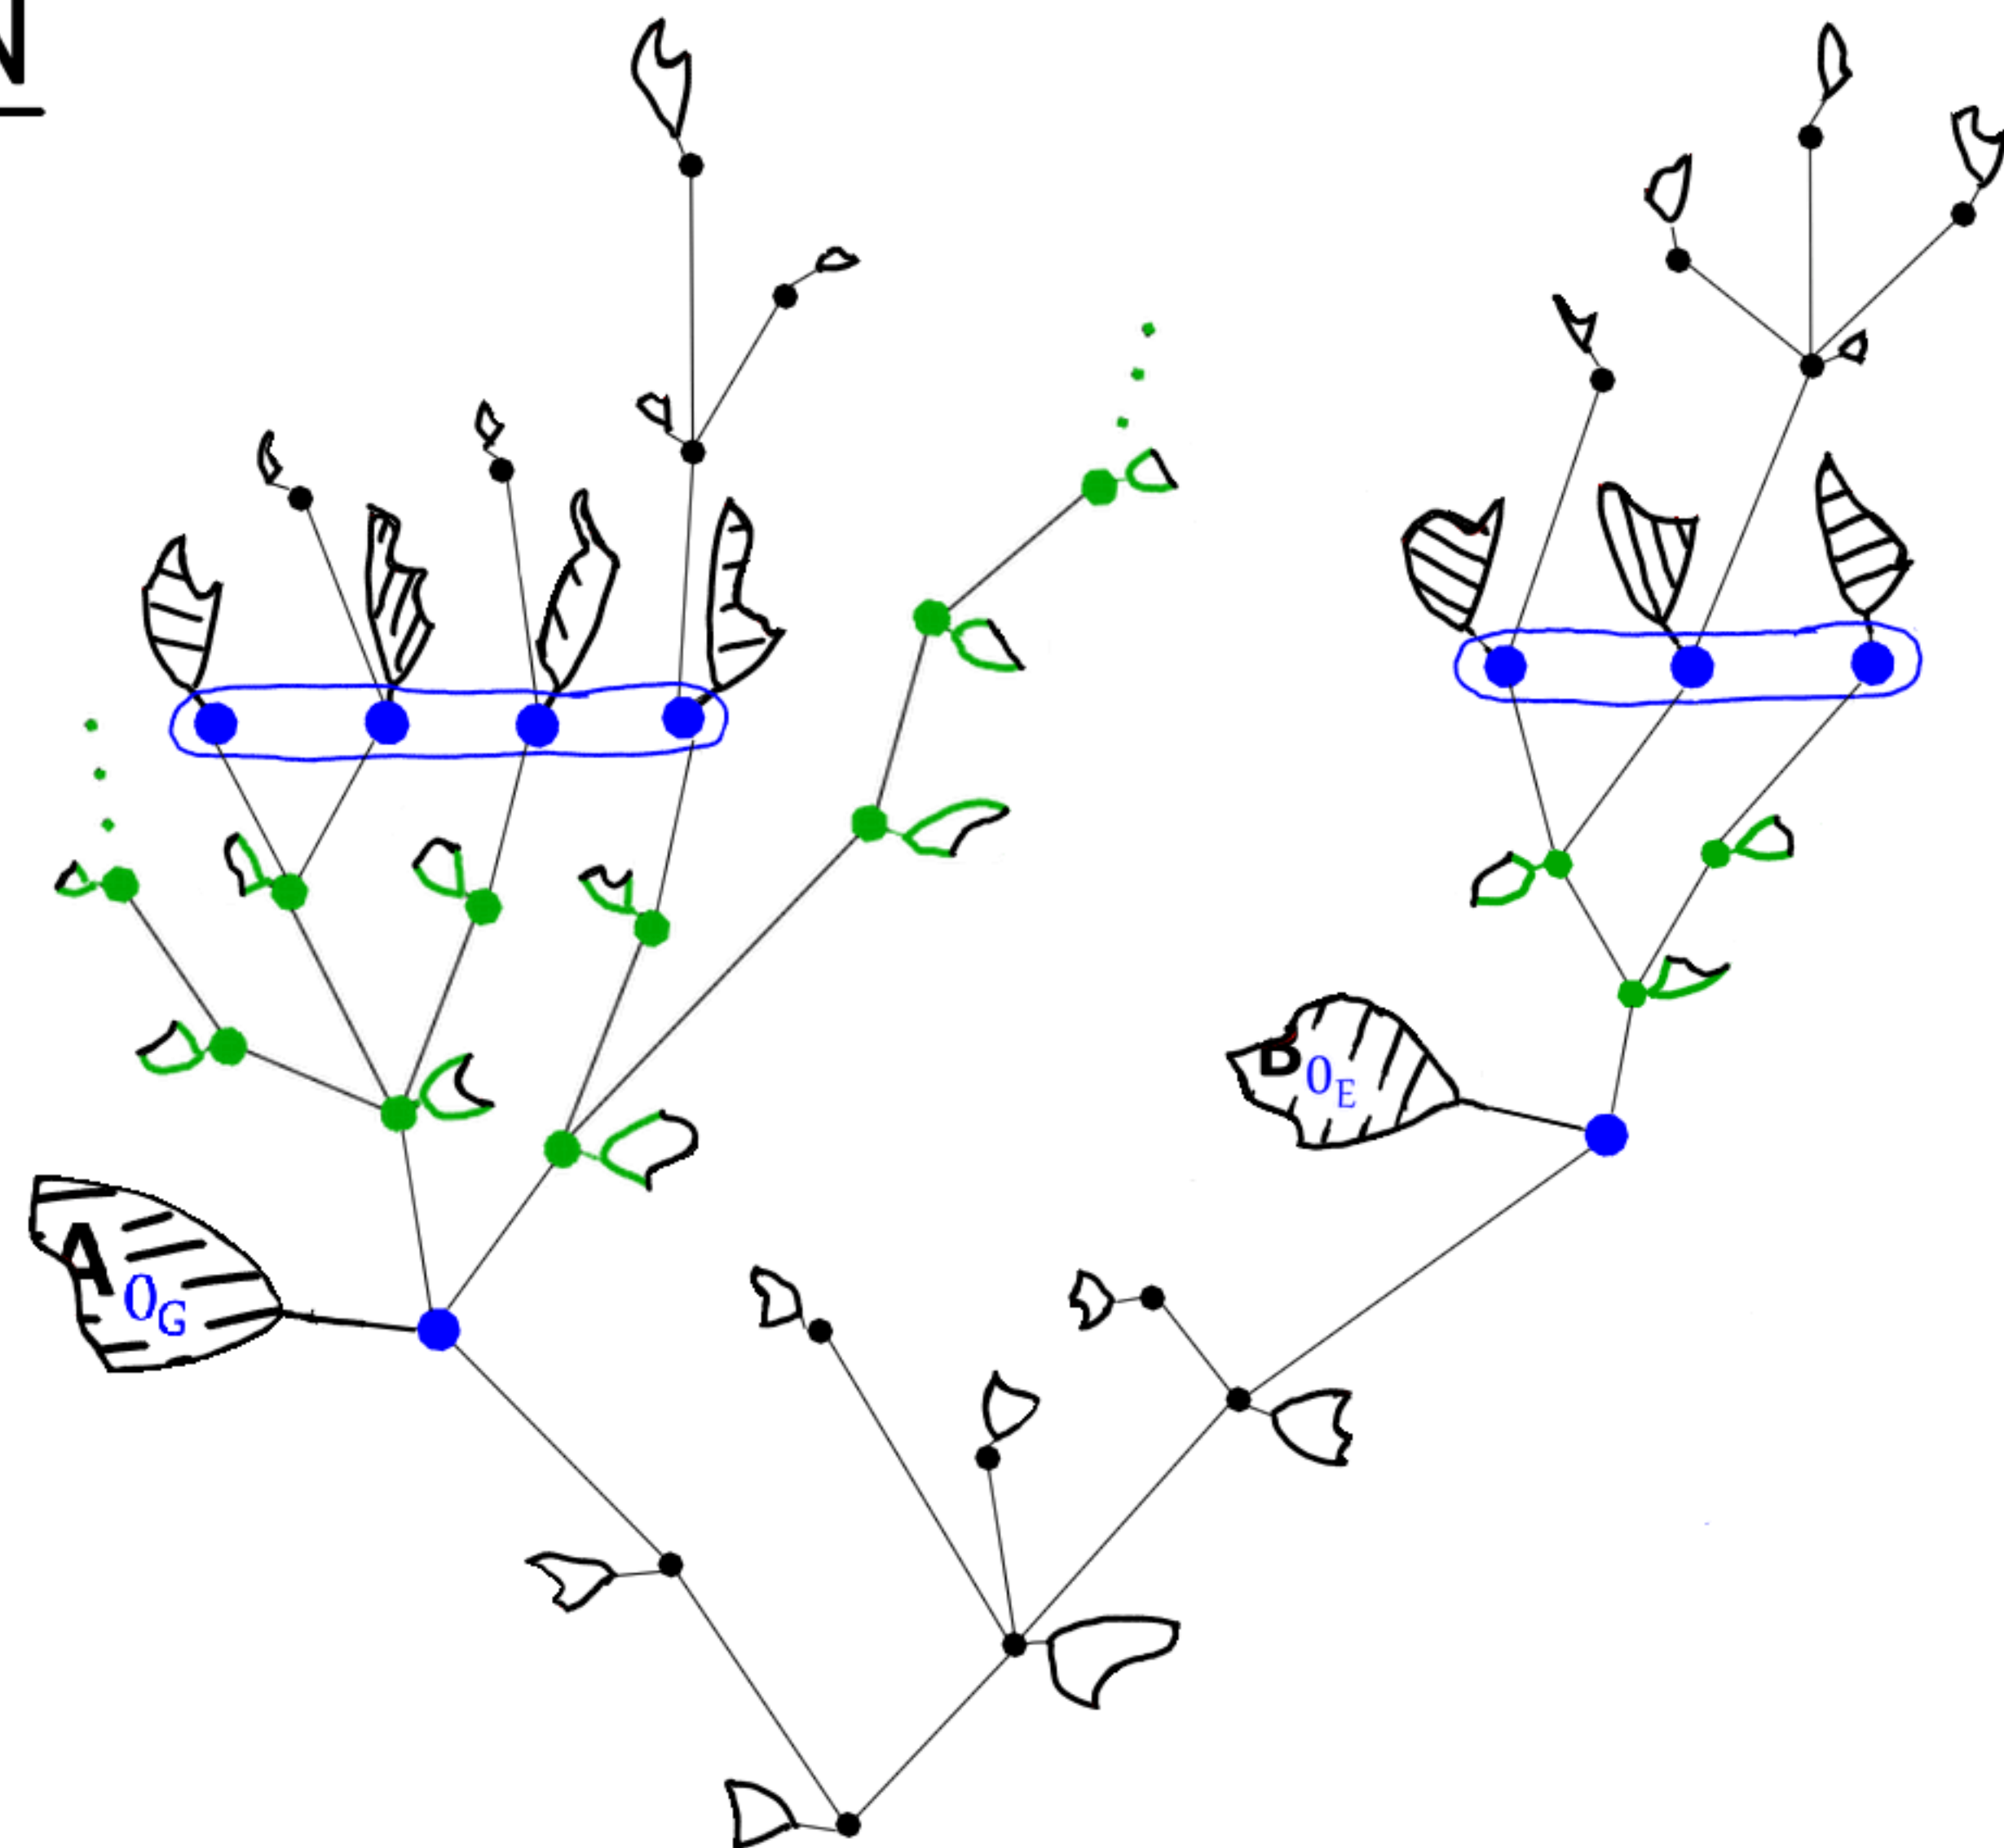



# FOLIAGE HYBRID OPERATION

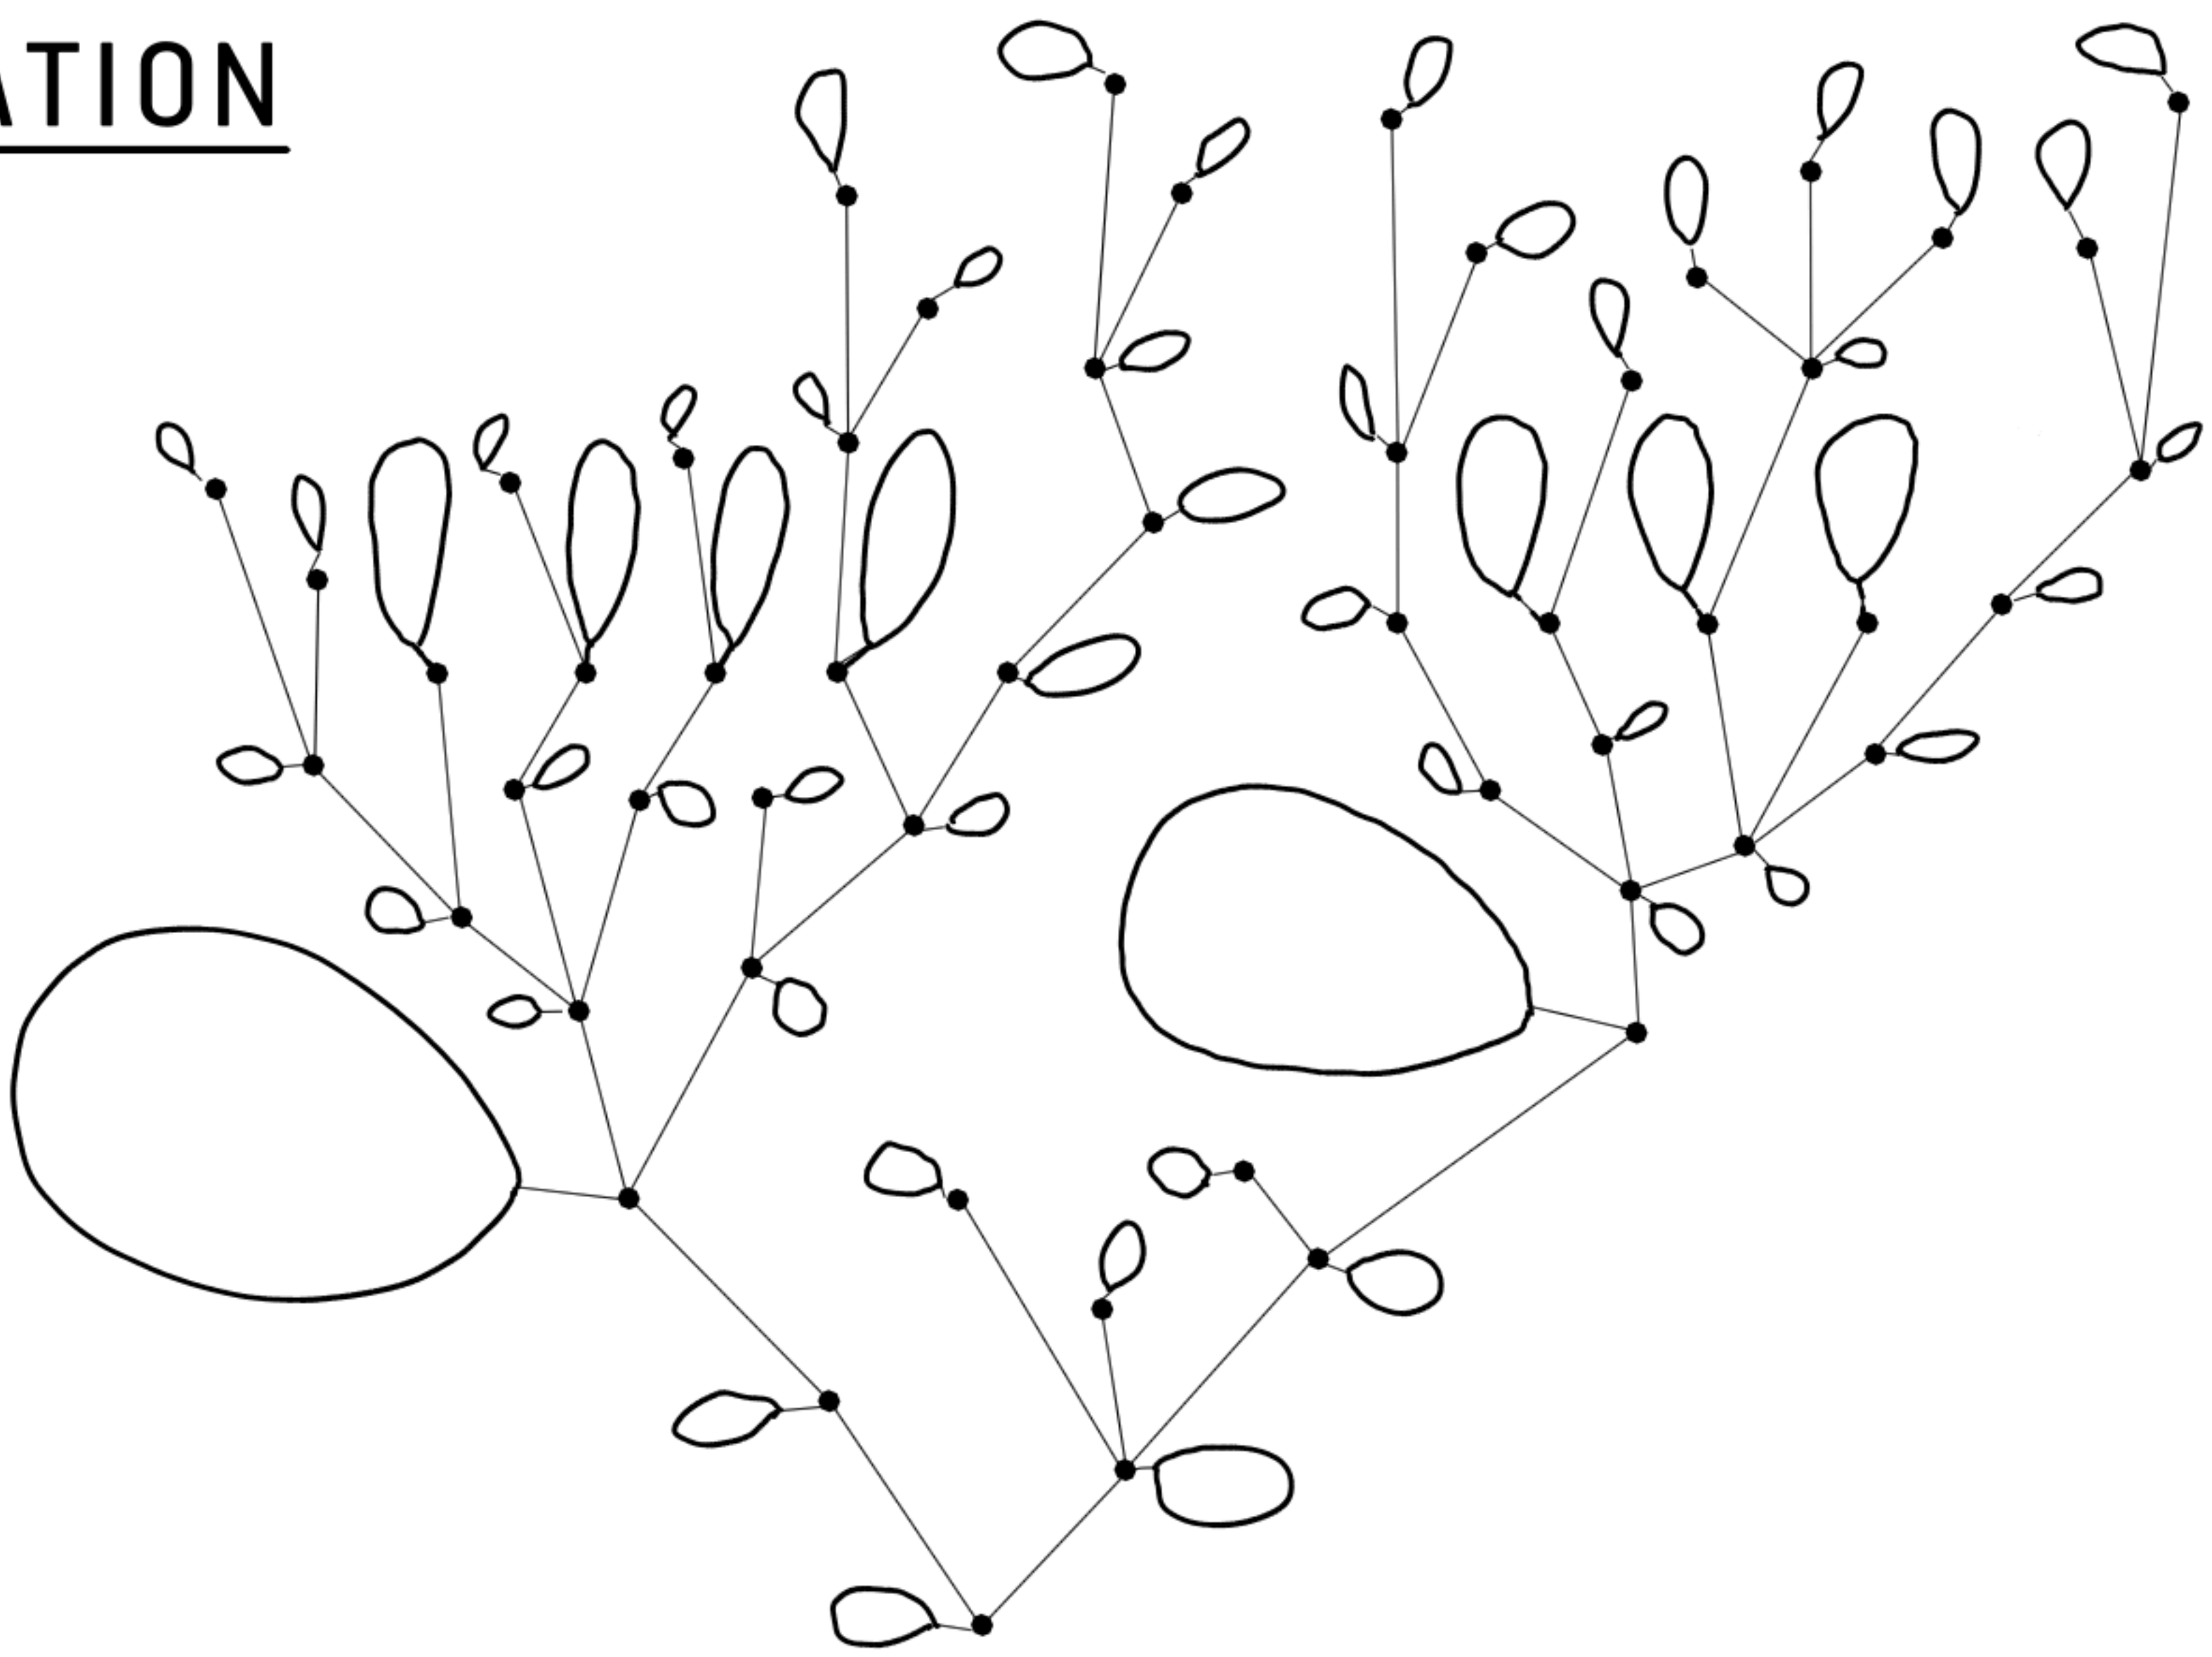

# FOLIAGE HYBRID OPERATION

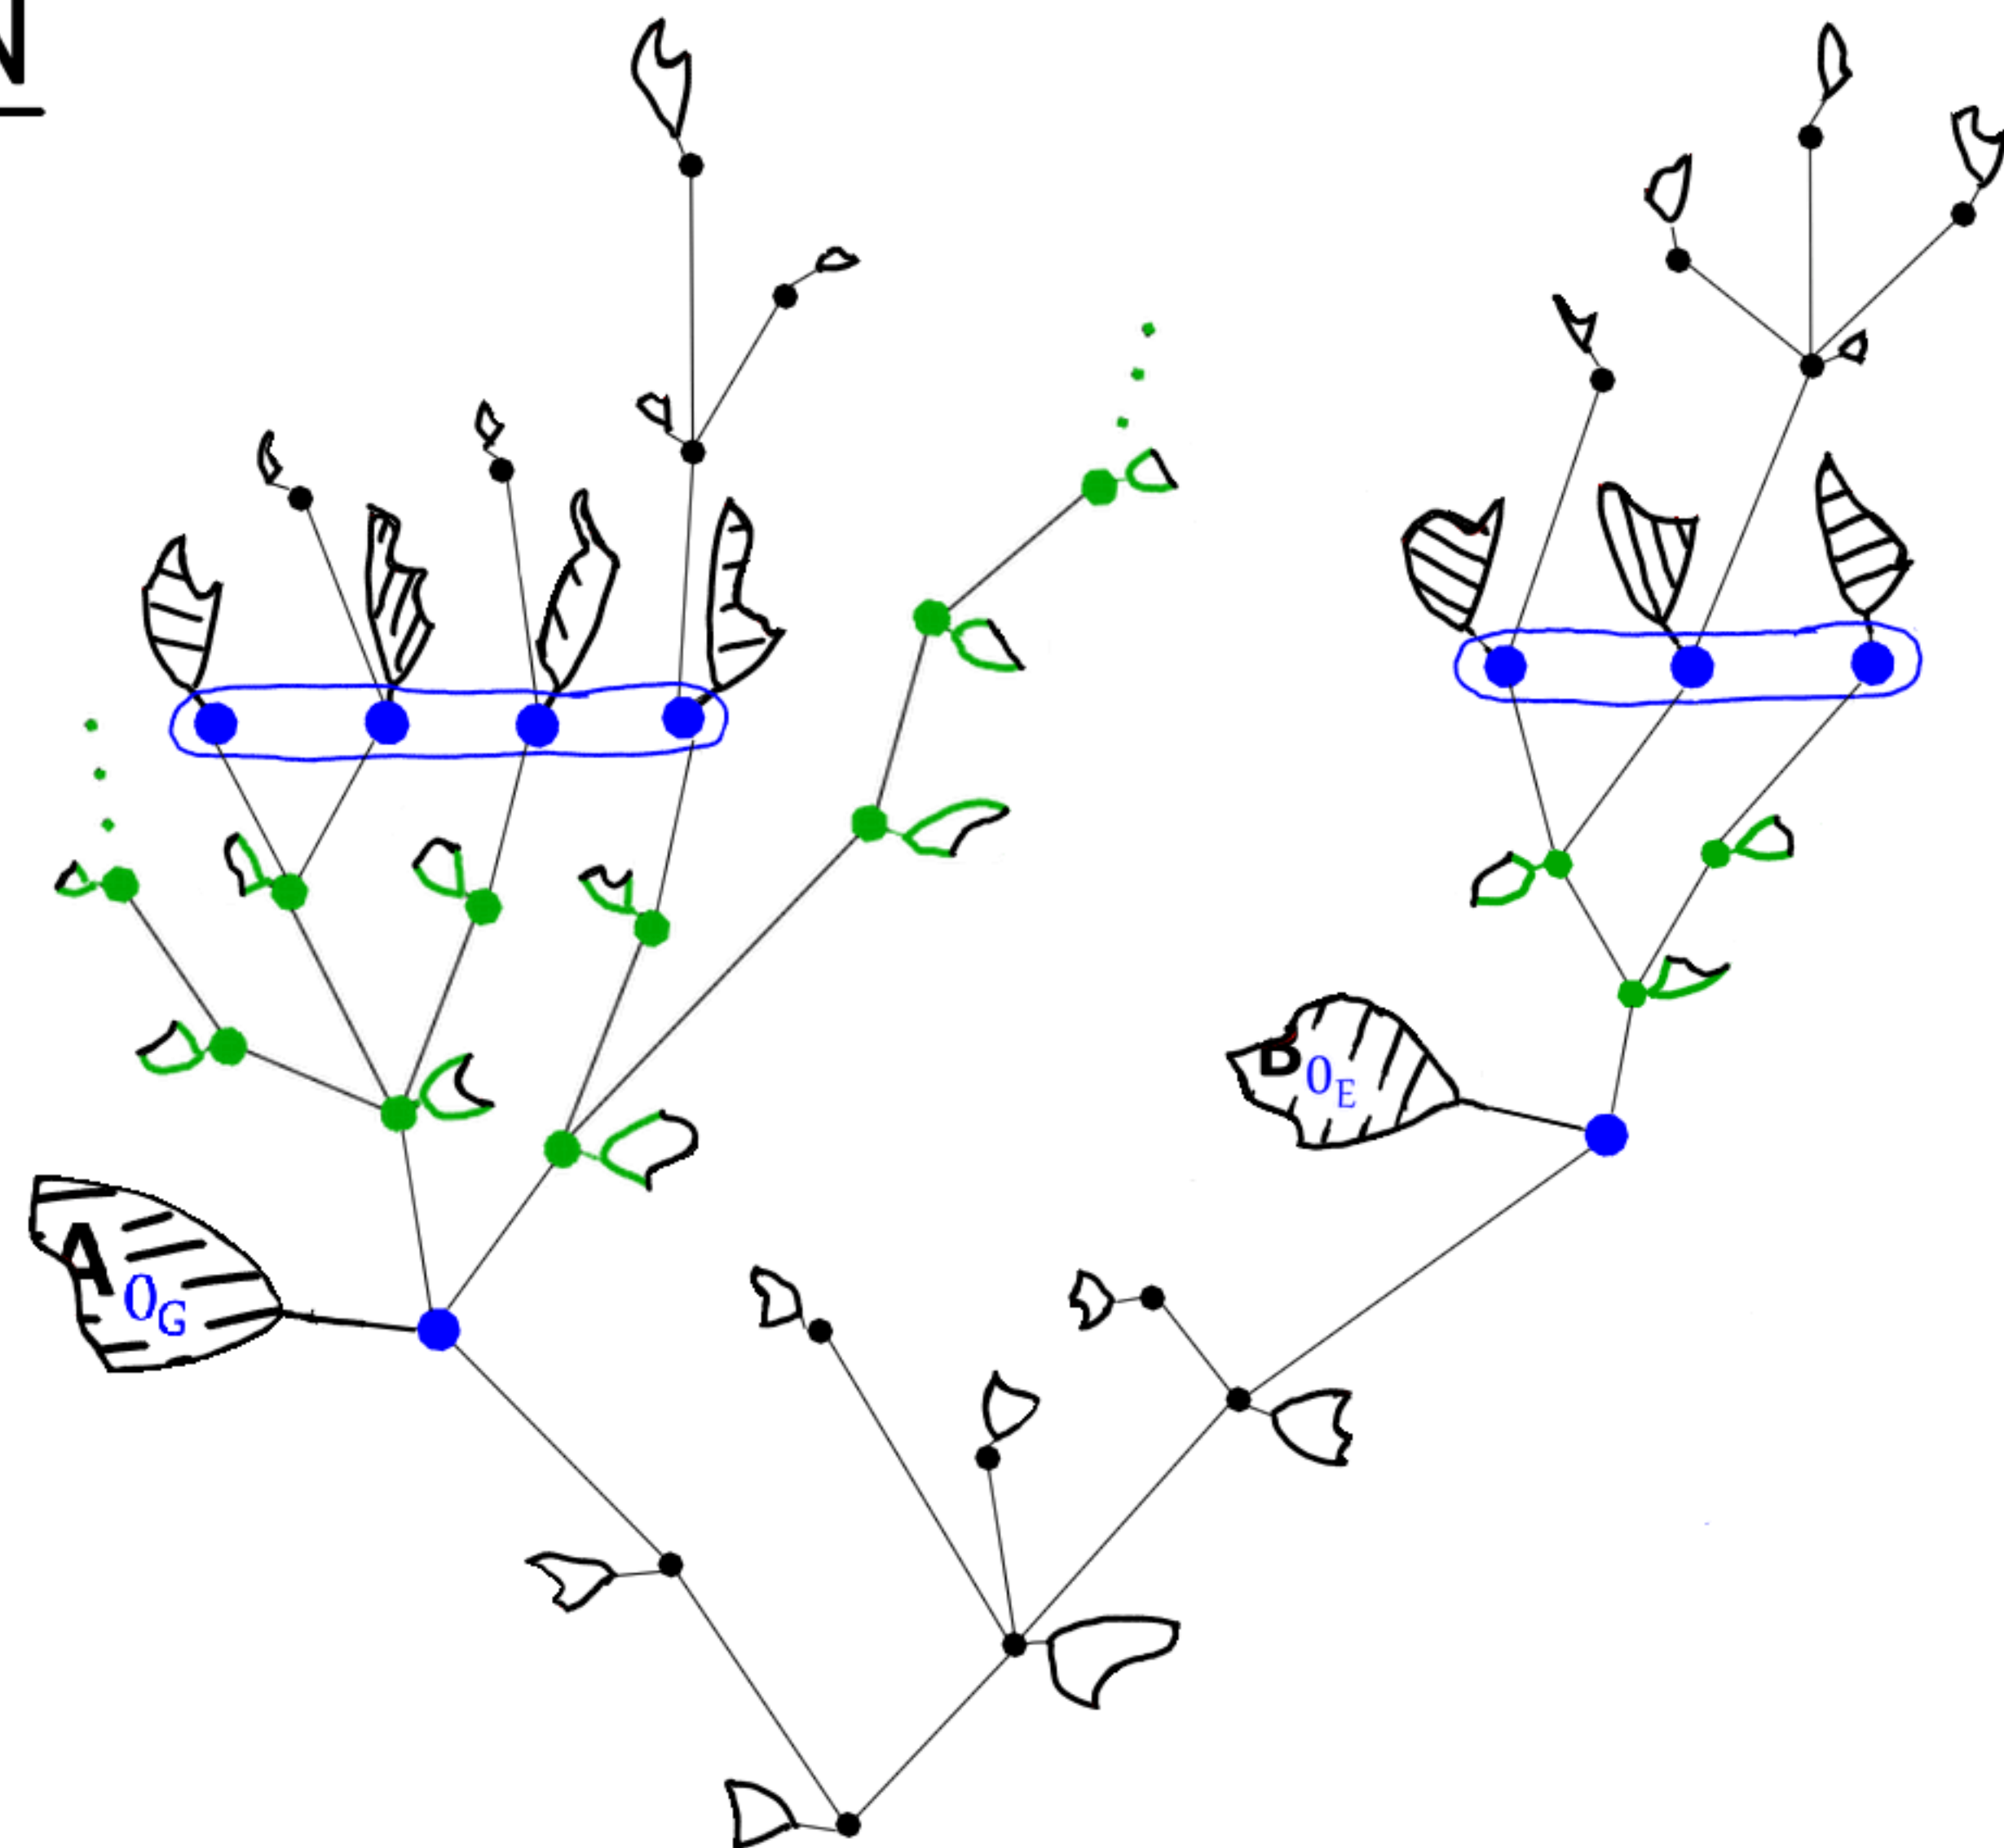



Mikhail Patrakeev, *The complement of a  $\sigma$ -compact subset of a space with a  $\pi$ -tree also has a  $\pi$ -tree*, Topology and its Applications, the special issue dedicated to the 120th anniversary of P.S. Alexandroff, accepted for publication in 2016. Preprint: <https://arxiv.org/abs/1512.02458>
